# Supplementary material for: Playable Video Generation
Source: arXiv:2101.12195 source file (2021-01-28)
Supplement: Supplementary file 1 [file bair_breakout_action_unrolls.tex]

\begin{table*}
    \centering
    
    \resizebox{\linewidth}{!}{

    \setlength\tabcolsep{0.5pt}
    \footnotesize

    \begin{tabular}{l@{\hskip 0.7mm}ccccccc}
         
         & Action 1 & Action 2 & Action 3 & Action 4 & Action 5 & Action 6 & Action 7 \\
         
         \rotatebox{90}{\setlength{\thickmuskip}{0mu}\hspace{6mm}$t=6$\hspace{11.5mm}$t=4$\hspace{11.5mm}$t=2$\hspace{11.5mm}$t=0$} &
         \setlength{\fboxsep}{0pt}\fbox{\includegraphics[trim=2 0 0 2,clip,width=0.2\columnwidth]{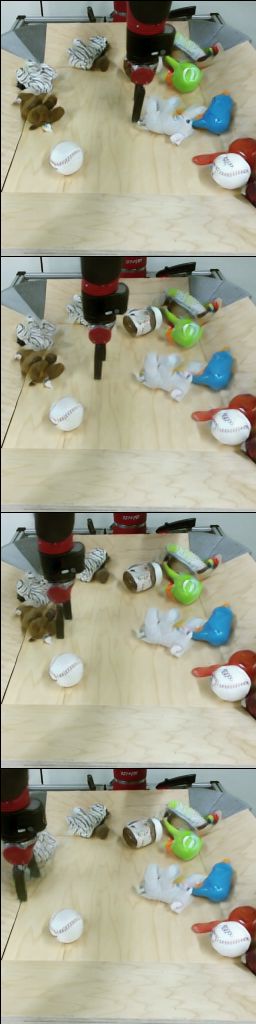}} &
         \setlength{\fboxsep}{0pt}\fbox{\includegraphics[trim=2 0 0 2,clip,width=0.2\columnwidth]{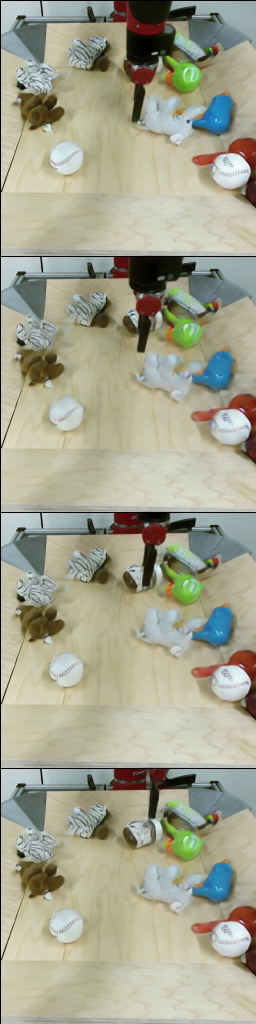}} &
         \setlength{\fboxsep}{0pt}\fbox{\includegraphics[trim=2 0 0 2,clip,width=0.2\columnwidth]{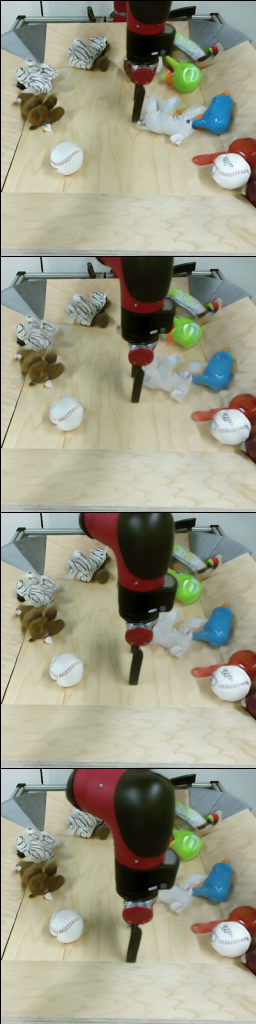}} &
         \setlength{\fboxsep}{0pt}\fbox{\includegraphics[trim=2 0 0 2,clip,width=0.2\columnwidth]{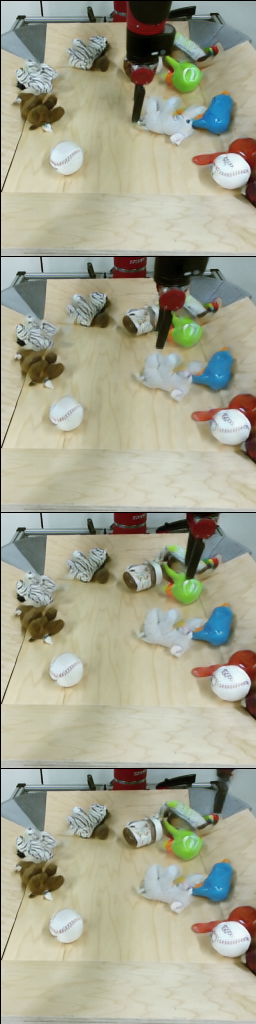}} &
         \setlength{\fboxsep}{0pt}\fbox{\includegraphics[trim=2 0 0 2,clip,width=0.2\columnwidth]{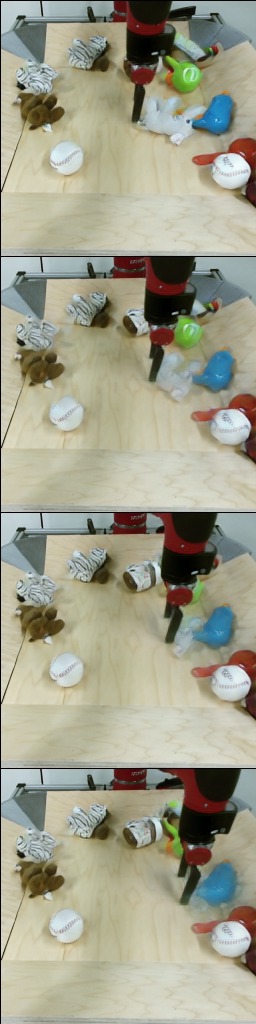}} &
         \setlength{\fboxsep}{0pt}\fbox{\includegraphics[trim=2 0 0 2,clip,width=0.2\columnwidth]{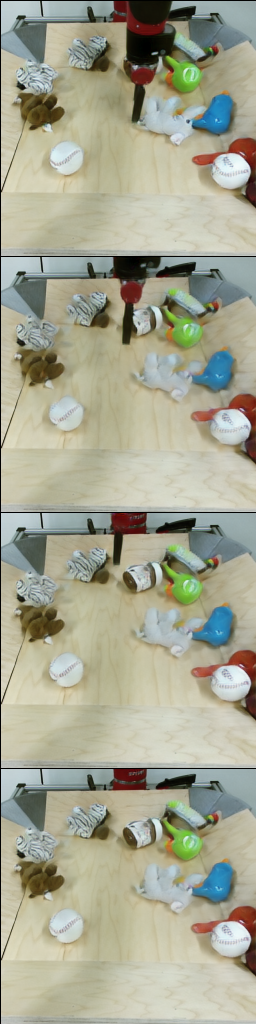}} &
         \setlength{\fboxsep}{0pt}\fbox{\includegraphics[trim=2 0 0 2,clip,width=0.2\columnwidth]{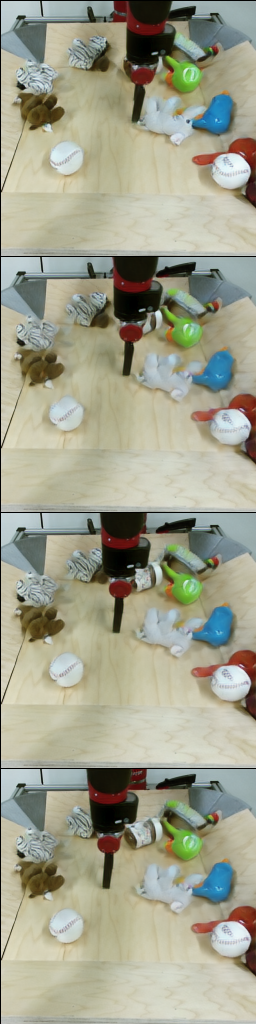}} \\

    \end{tabular}
    \quad
    \begin{tabular}{l@{\hskip 0.7mm}ccc}
     
         & Action 1 & Action 2 & Action 3 \\
         
         \rotatebox{90}{\setlength{\thickmuskip}{0mu}\hspace{6mm}$t=6$\hspace{11.5mm}$t=4$\hspace{11.5mm}$t=2$\hspace{11.5mm}$t=0$}
         &
         \setlength{\fboxsep}{0pt}\fbox{\includegraphics[width=0.2\columnwidth]{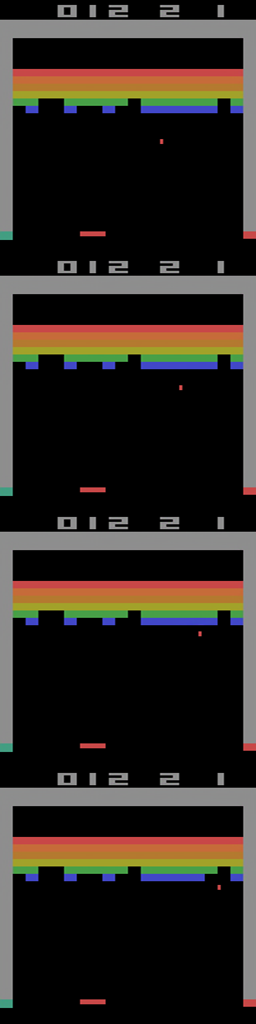}} &
         \setlength{\fboxsep}{0pt}\fbox{\includegraphics[width=0.2\columnwidth]{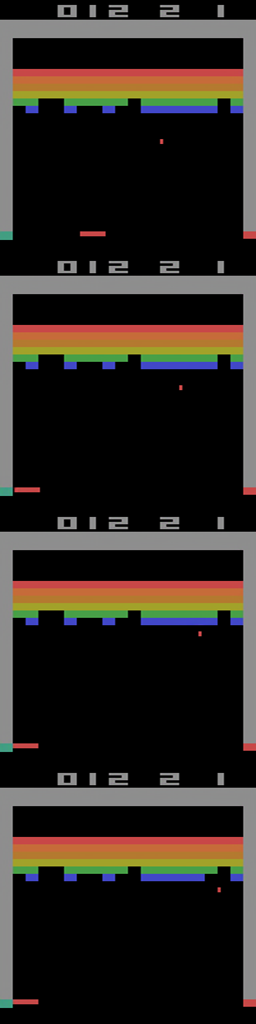}} &
         \setlength{\fboxsep}{0pt}\fbox{\includegraphics[width=0.2\columnwidth]{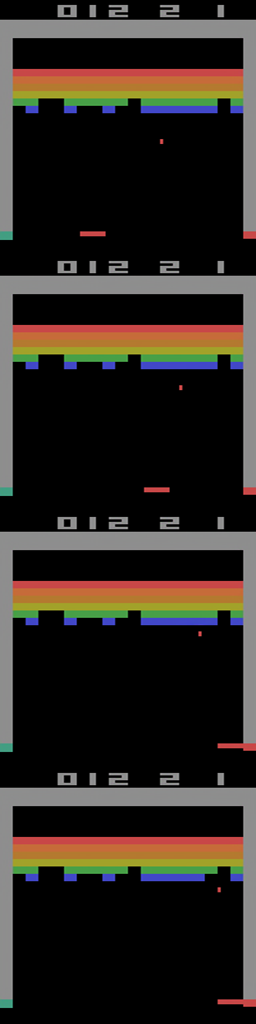}} \\
         
         %& \includegraphics[trim=65 85 52 80,clip,width=0.2\columnwidth]{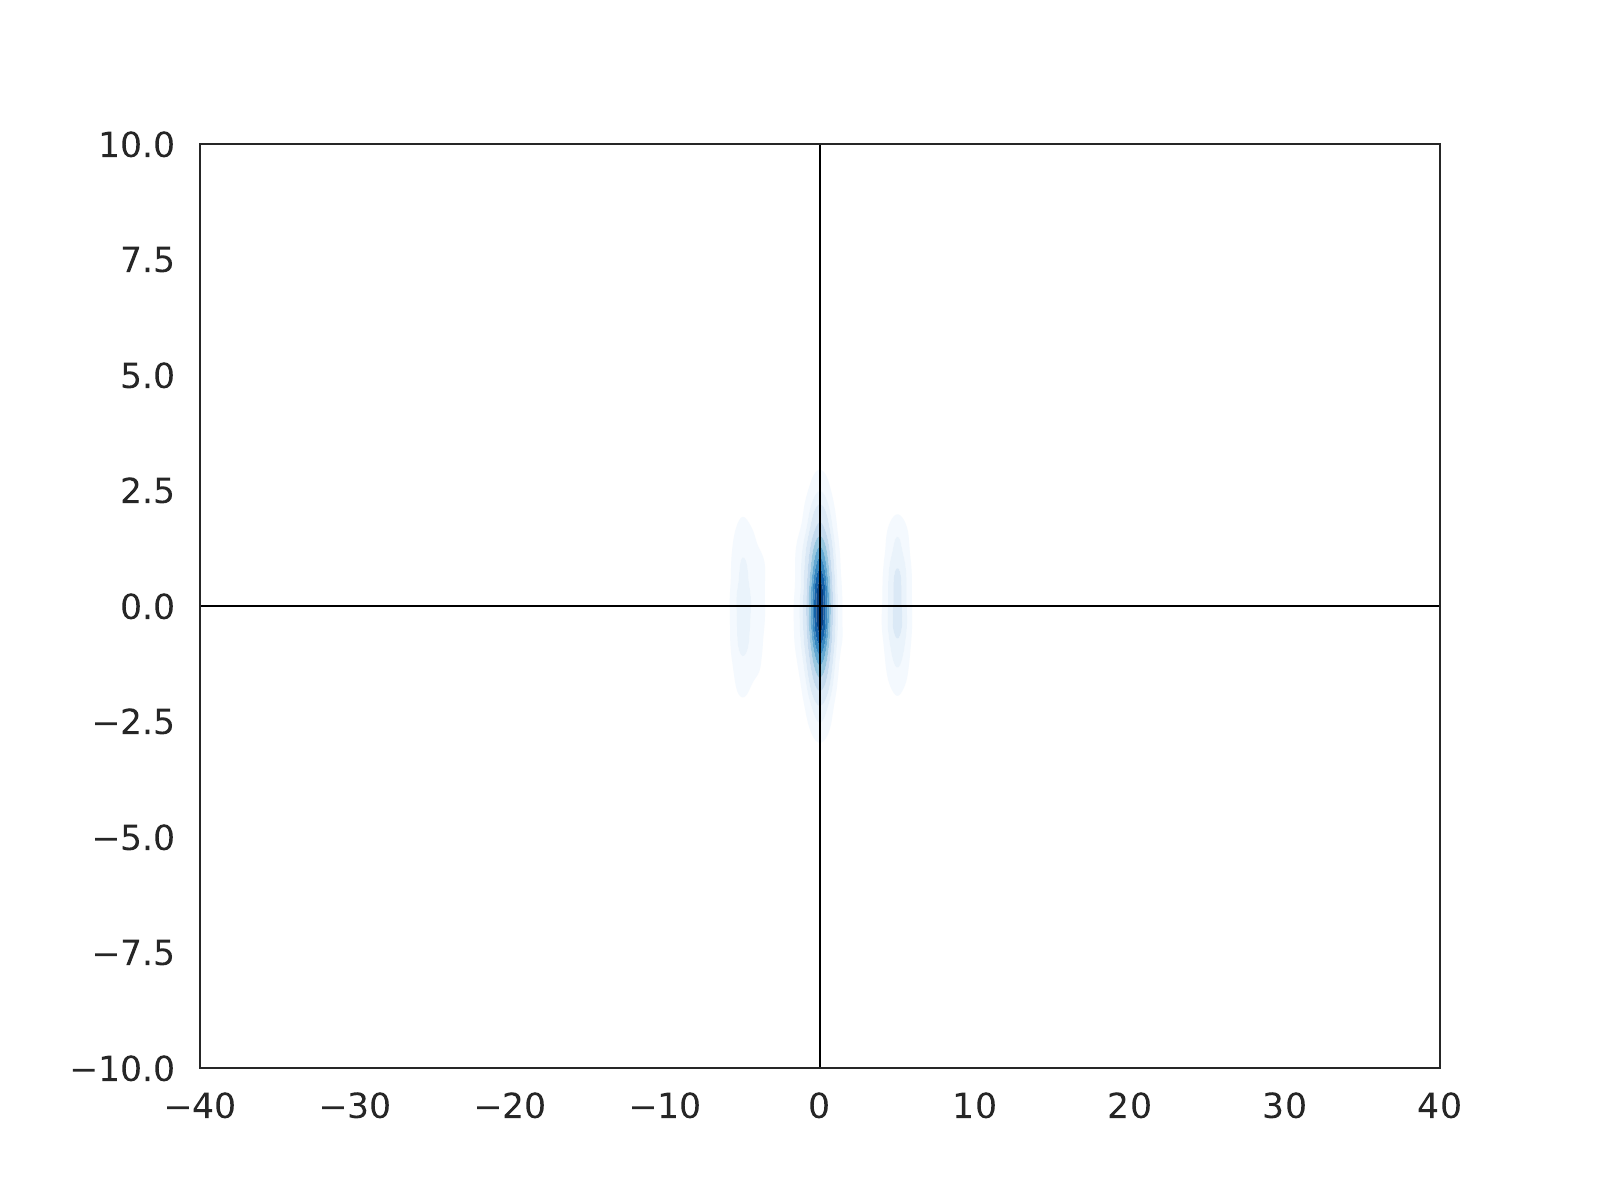} &
         %\includegraphics[trim=65 85 52 80,clip,width=0.2\columnwidth]{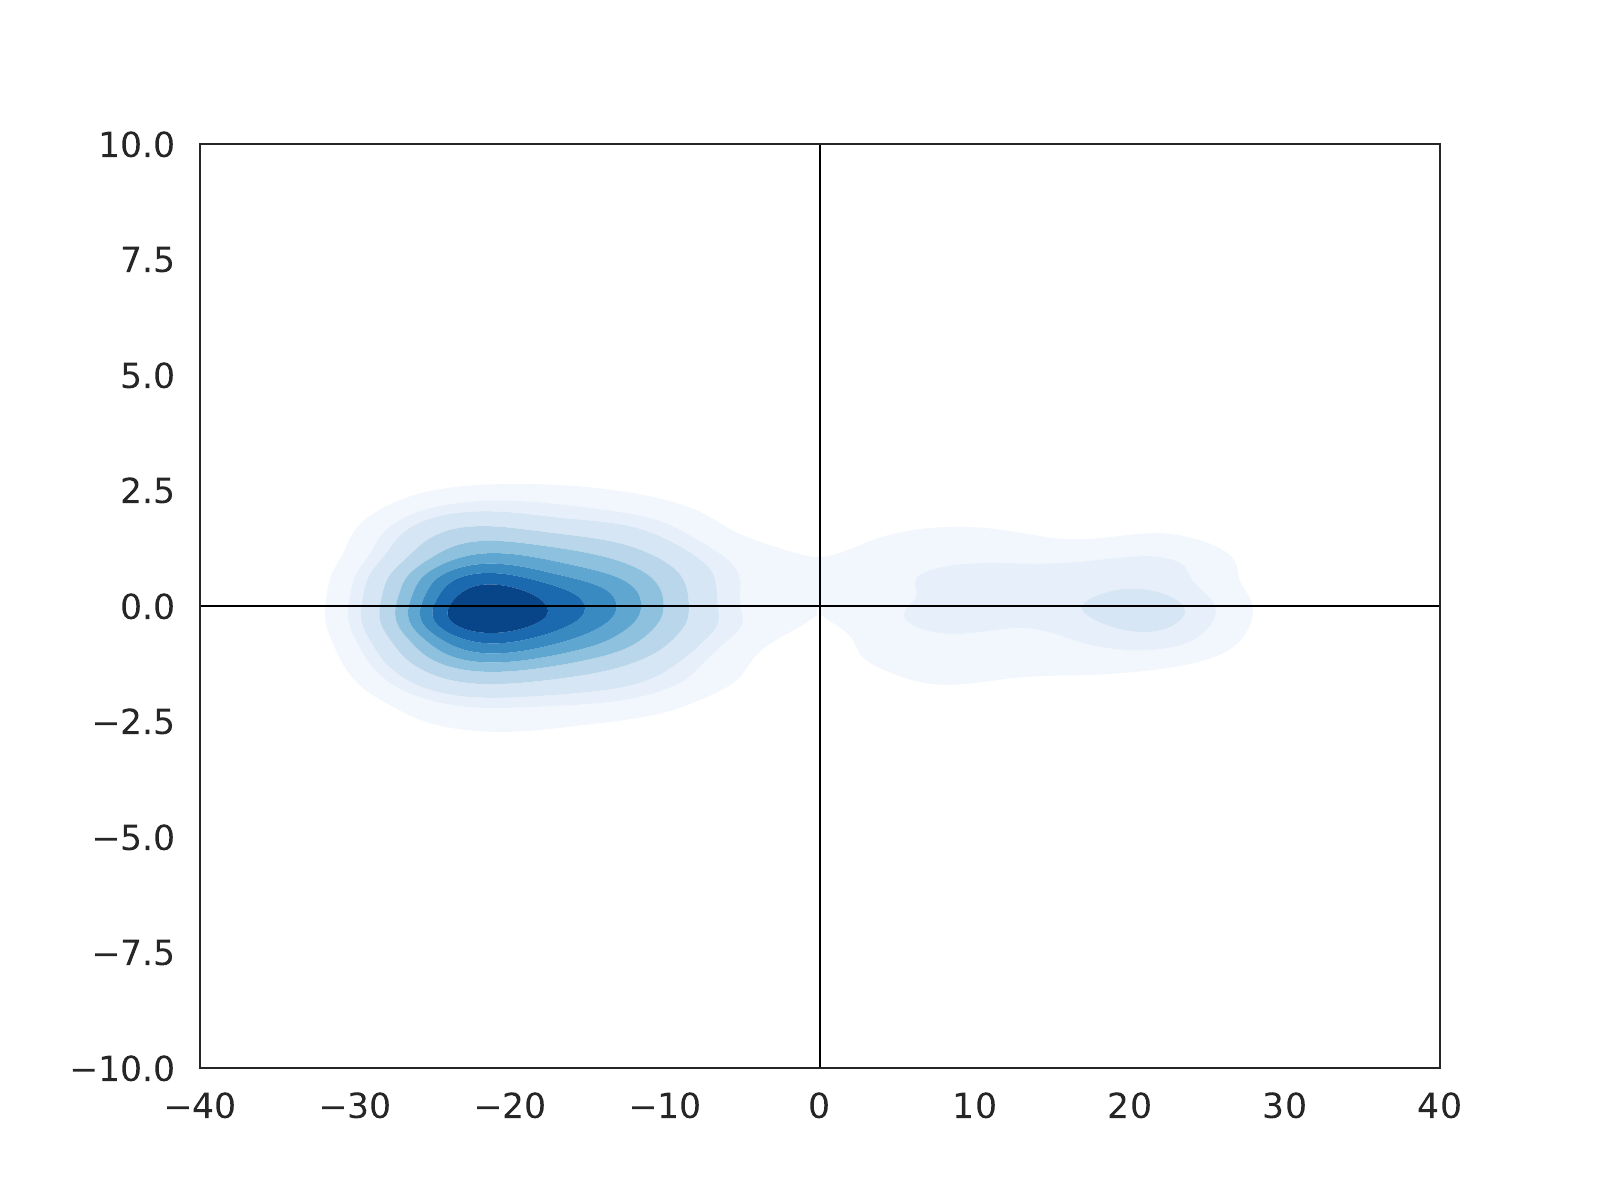} &
         %\includegraphics[trim=65 85 52 80,clip,width=0.2\columnwidth]{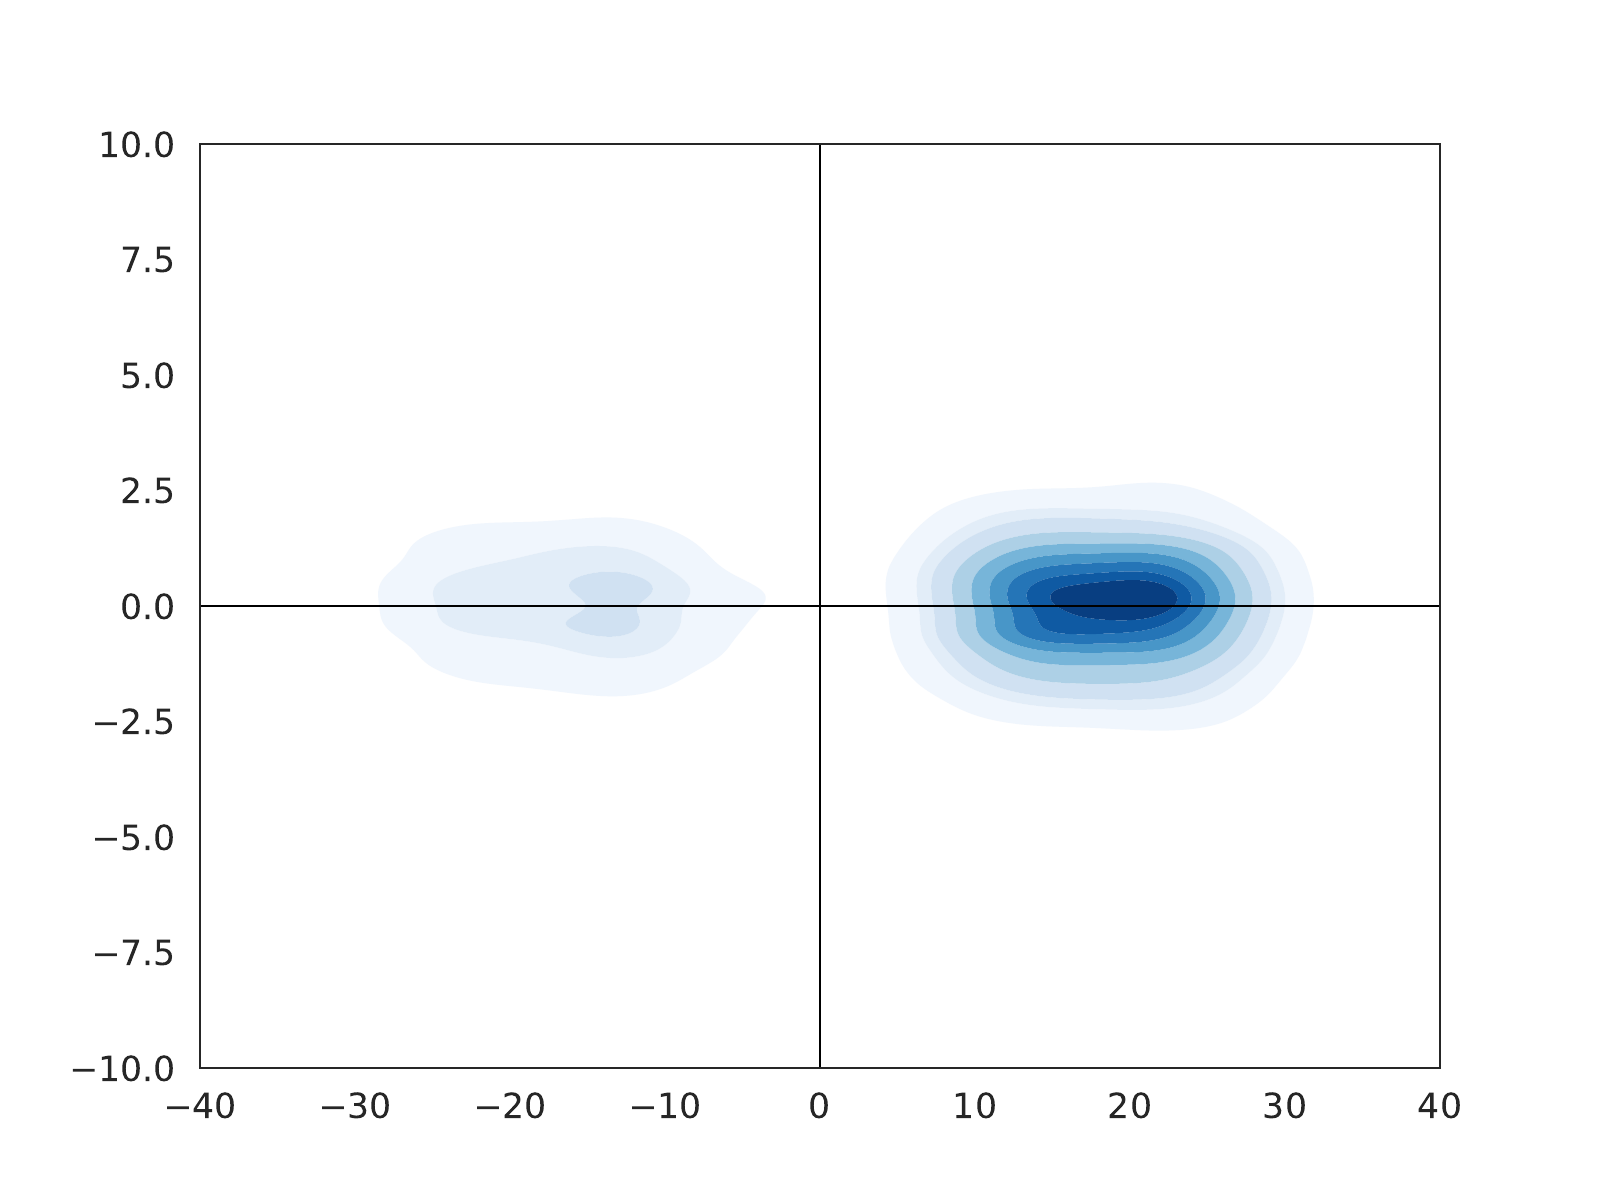} \\
         
    \end{tabular}
    }
    \captionof{figure}{Videos generated by \methodname~on the \emph{BAIR} (left) and on the \emph{Atari Breakout} (right) datasets. We generate a sequence for each learned action by repeatedly inputting the current action starting from the same initial frame. In all datasets, the model learns actions that correspond to movement on each axis. Additional videos are shown in the corresponding section of the \href{run:./main.html}{main.html} page.}
    \label{fig:bair_breakout_action_unrolls}

\end{table*}
