# Supplementary material for: Playable Video Generation
Source: arXiv:2101.12195 source file (2021-01-28)
Supplement: Supplementary file 2 [file tennis_action_unrolls.tex]

\begin{table*}
    \centering
    
    \resizebox{\linewidth}{!}{
    \setlength\tabcolsep{0.5pt}
    \scriptsize
    \begin{tabular}{l@{\hskip 0.7mm}ccccccc}
         
         & Action 1 & Action 2 & Action 3 & Action 4 & Action 5 & Action 6 & Action 7 \\
         
         \rotatebox{90}{\setlength{\thickmuskip}{0mu}\resizebox{30mm}{!}{\hspace{2mm}$t=8$\hspace{4mm}$t=6$\hspace{4mm}$t=4$\hspace{4mm}$t=2$\hspace{4mm}$t=0$}} &
         \setlength{\fboxsep}{0pt}\fbox{\includegraphics[width=0.2\columnwidth]{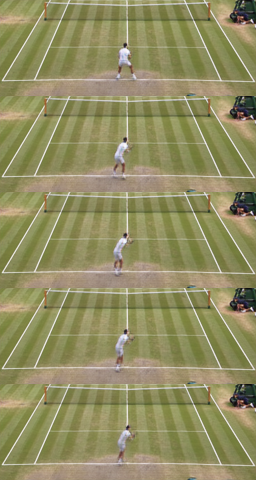}} & \setlength{\fboxsep}{0pt}\fbox{\includegraphics[width=0.2\columnwidth]{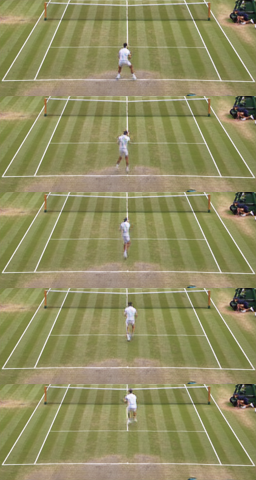}} & \setlength{\fboxsep}{0pt}\fbox{\includegraphics[width=0.2\columnwidth]{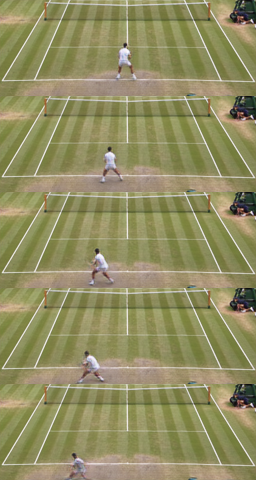}} & \setlength{\fboxsep}{0pt}\fbox{\includegraphics[width=0.2\columnwidth]{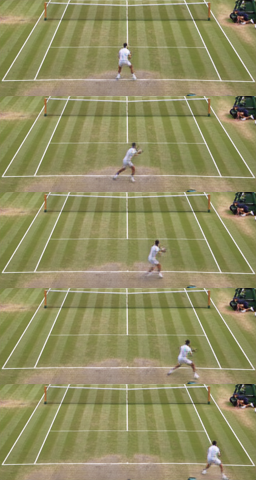}} & \setlength{\fboxsep}{0pt}\fbox{\includegraphics[width=0.2\columnwidth]{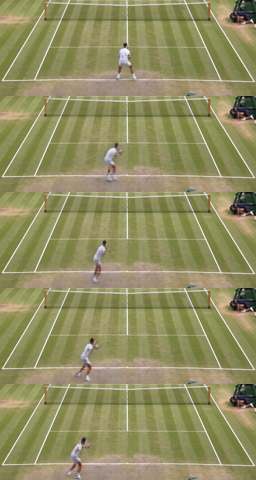}} & \setlength{\fboxsep}{0pt}\fbox{\includegraphics[width=0.2\columnwidth]{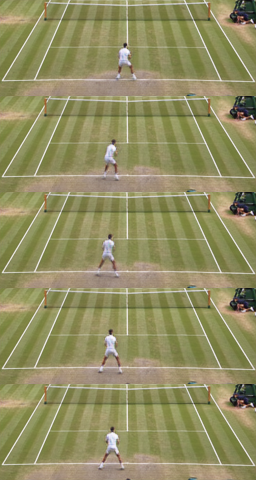}} & \setlength{\fboxsep}{0pt}\fbox{\includegraphics[width=0.2\columnwidth]{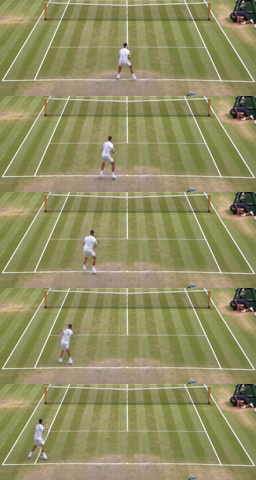}} \\
         
         %& \includegraphics[trim=62 85 49 80,clip,width=0.2\columnwidth]{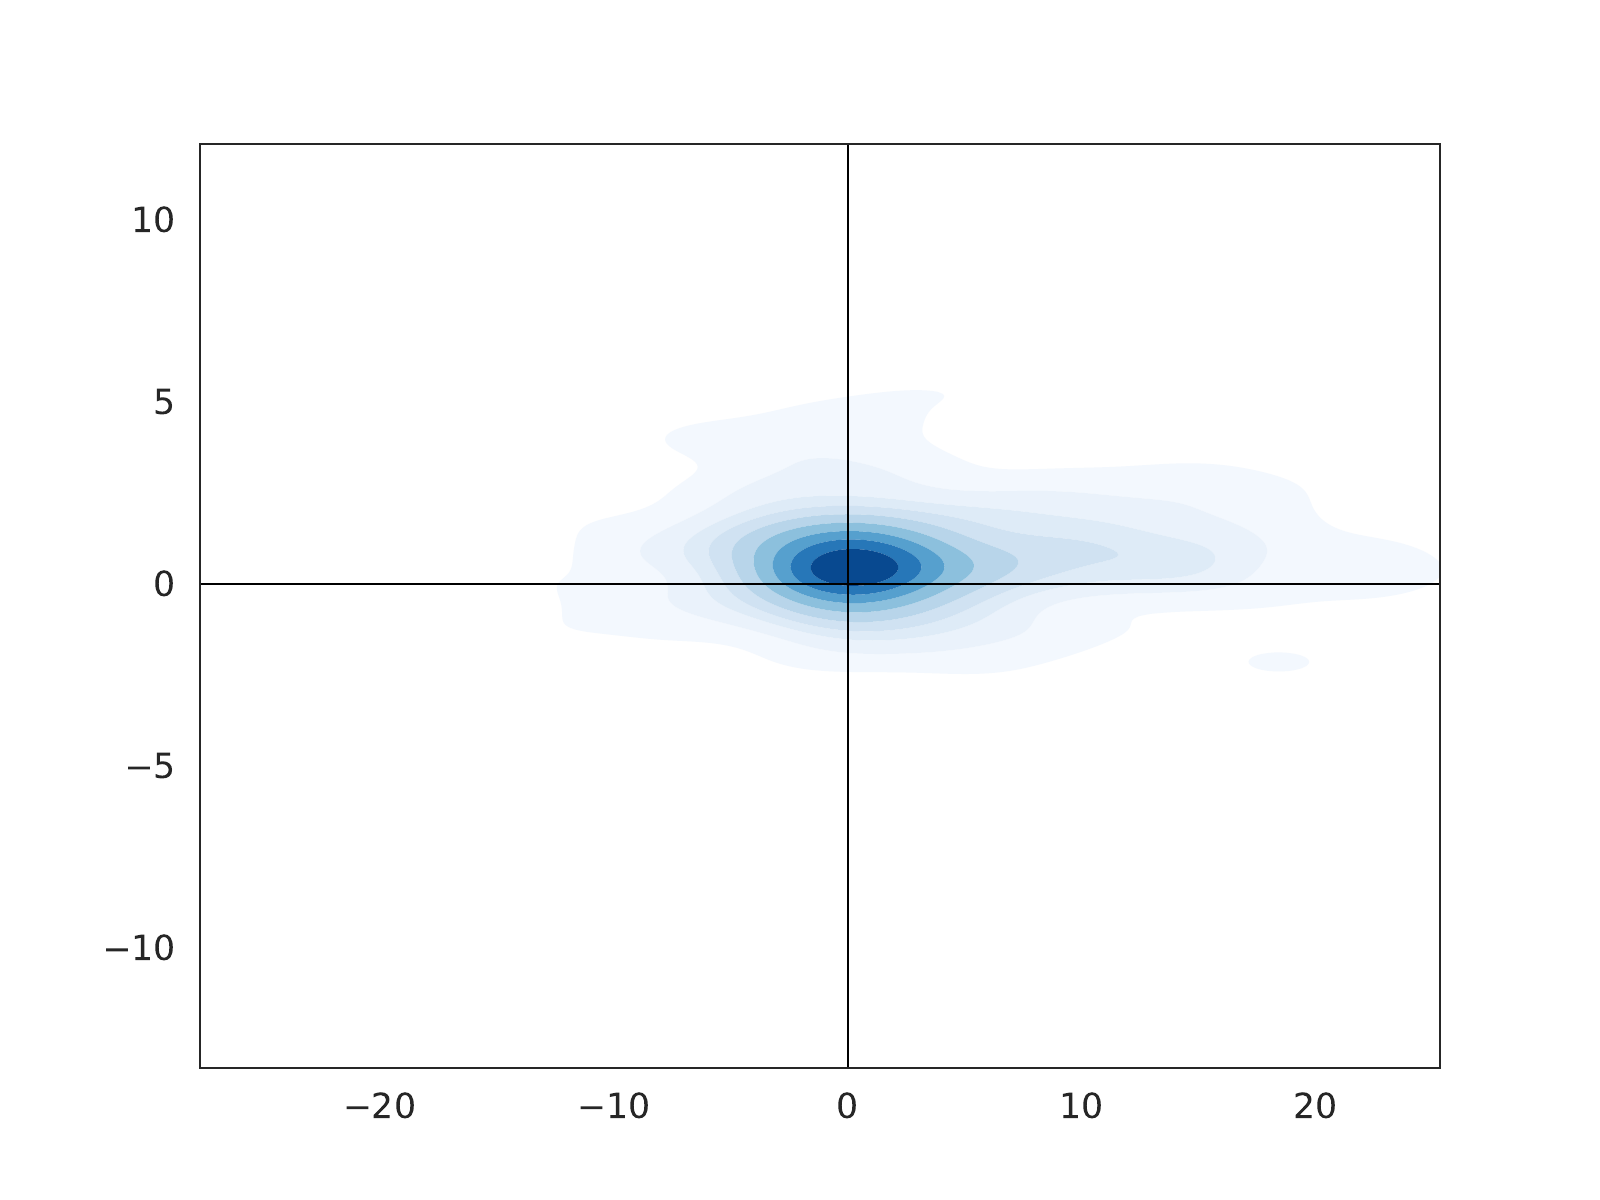} &
         %\includegraphics[trim=62 85 49 80,clip,width=0.2\columnwidth]{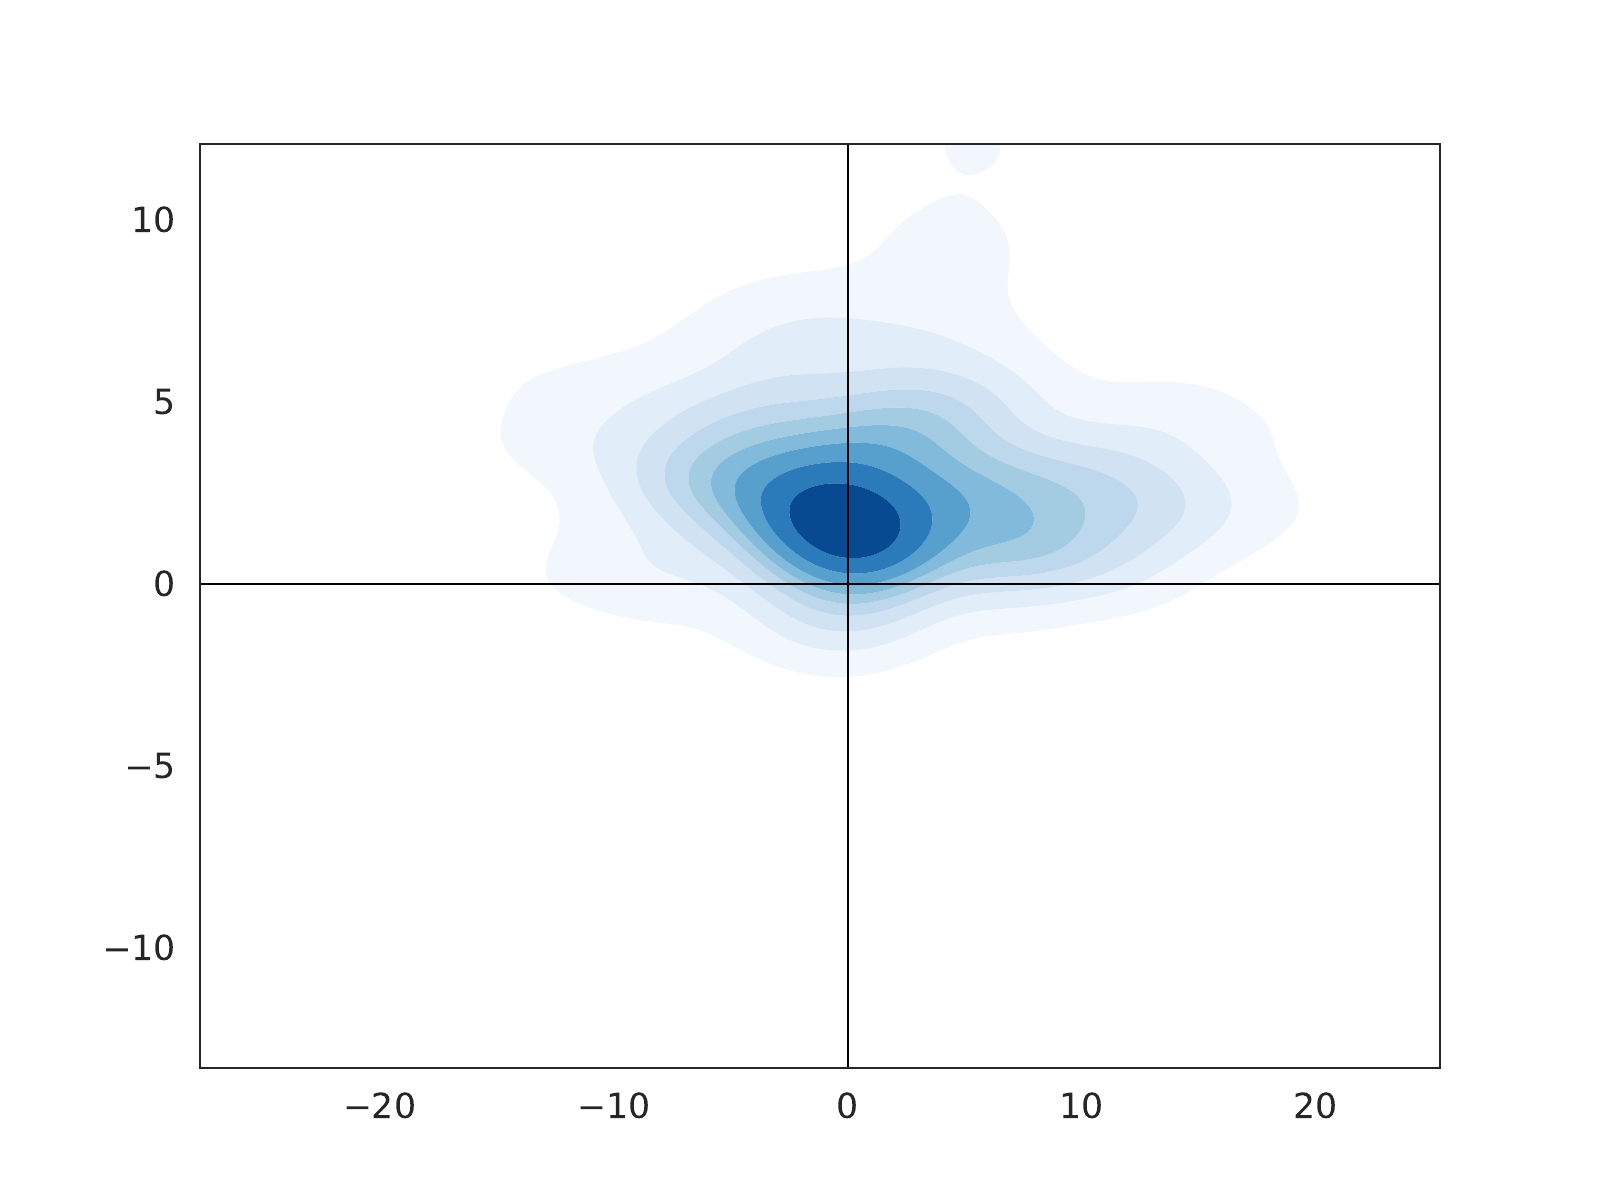} &
         %\includegraphics[trim=62 85 49 80,clip,width=0.2\columnwidth]{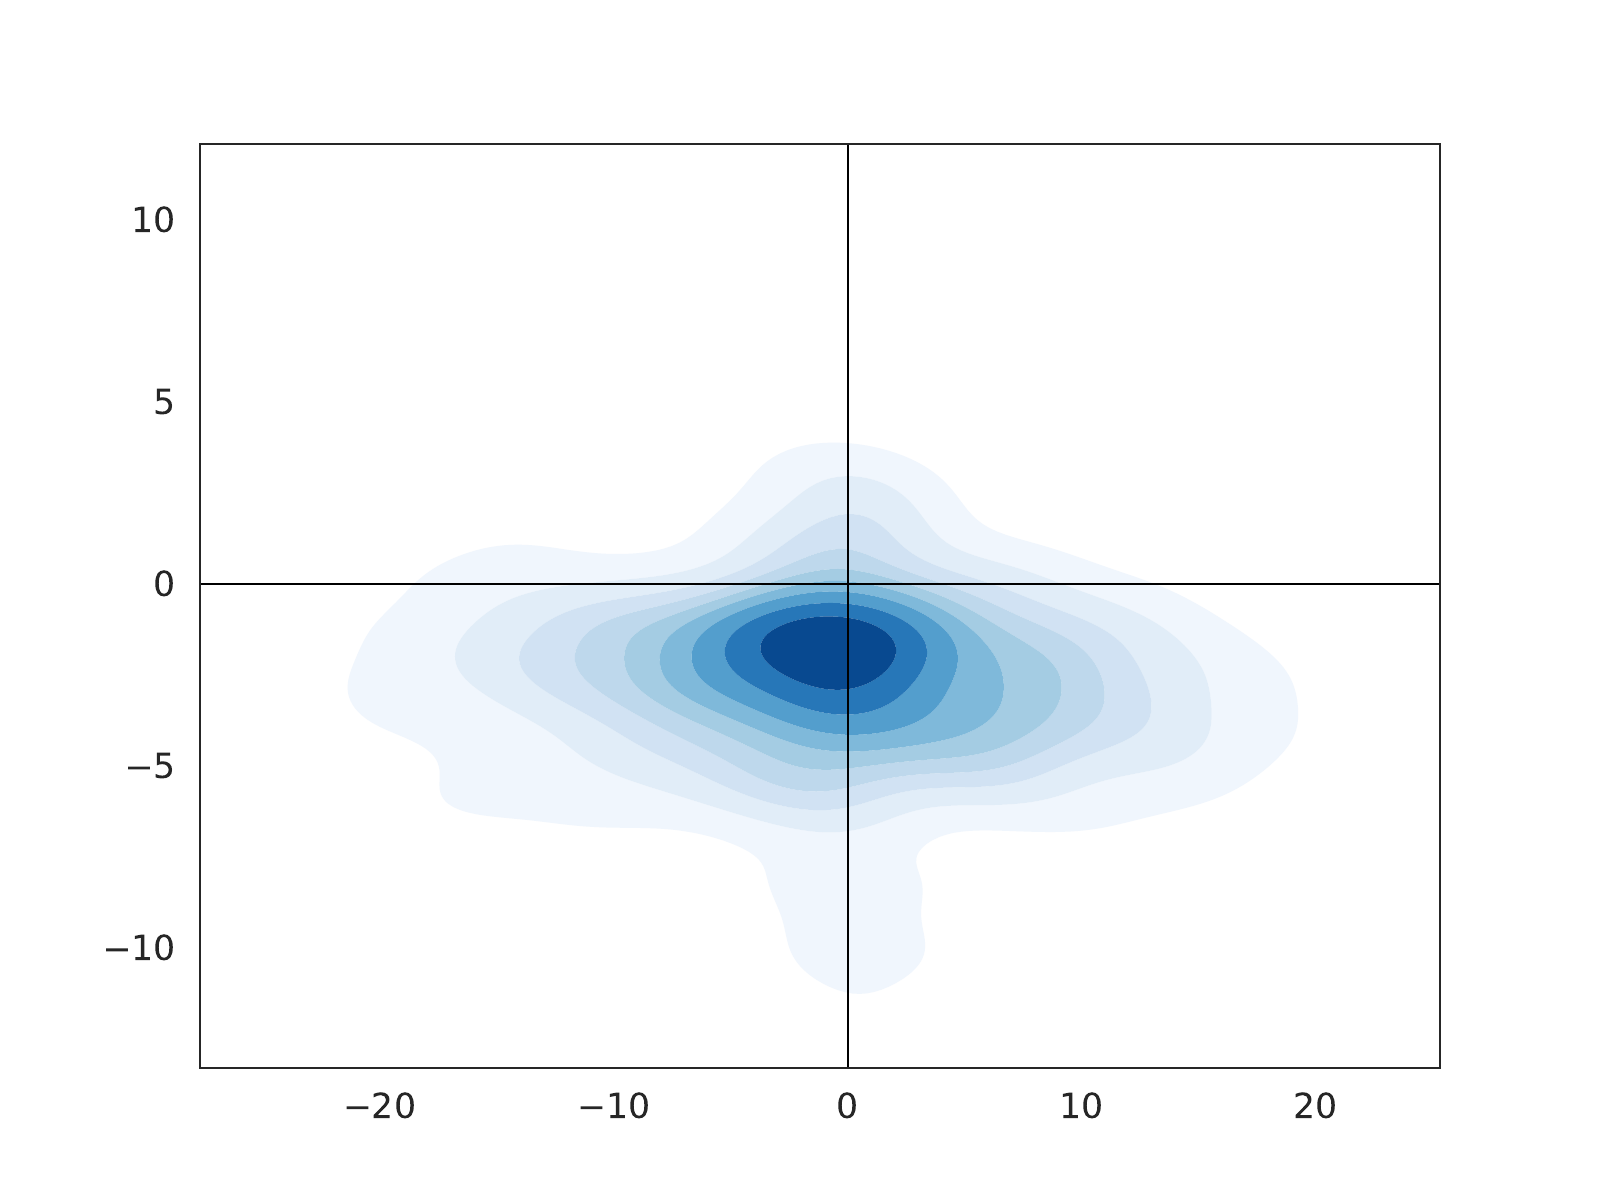} &
         %\includegraphics[trim=62 85 49 80,clip,width=0.2\columnwidth]{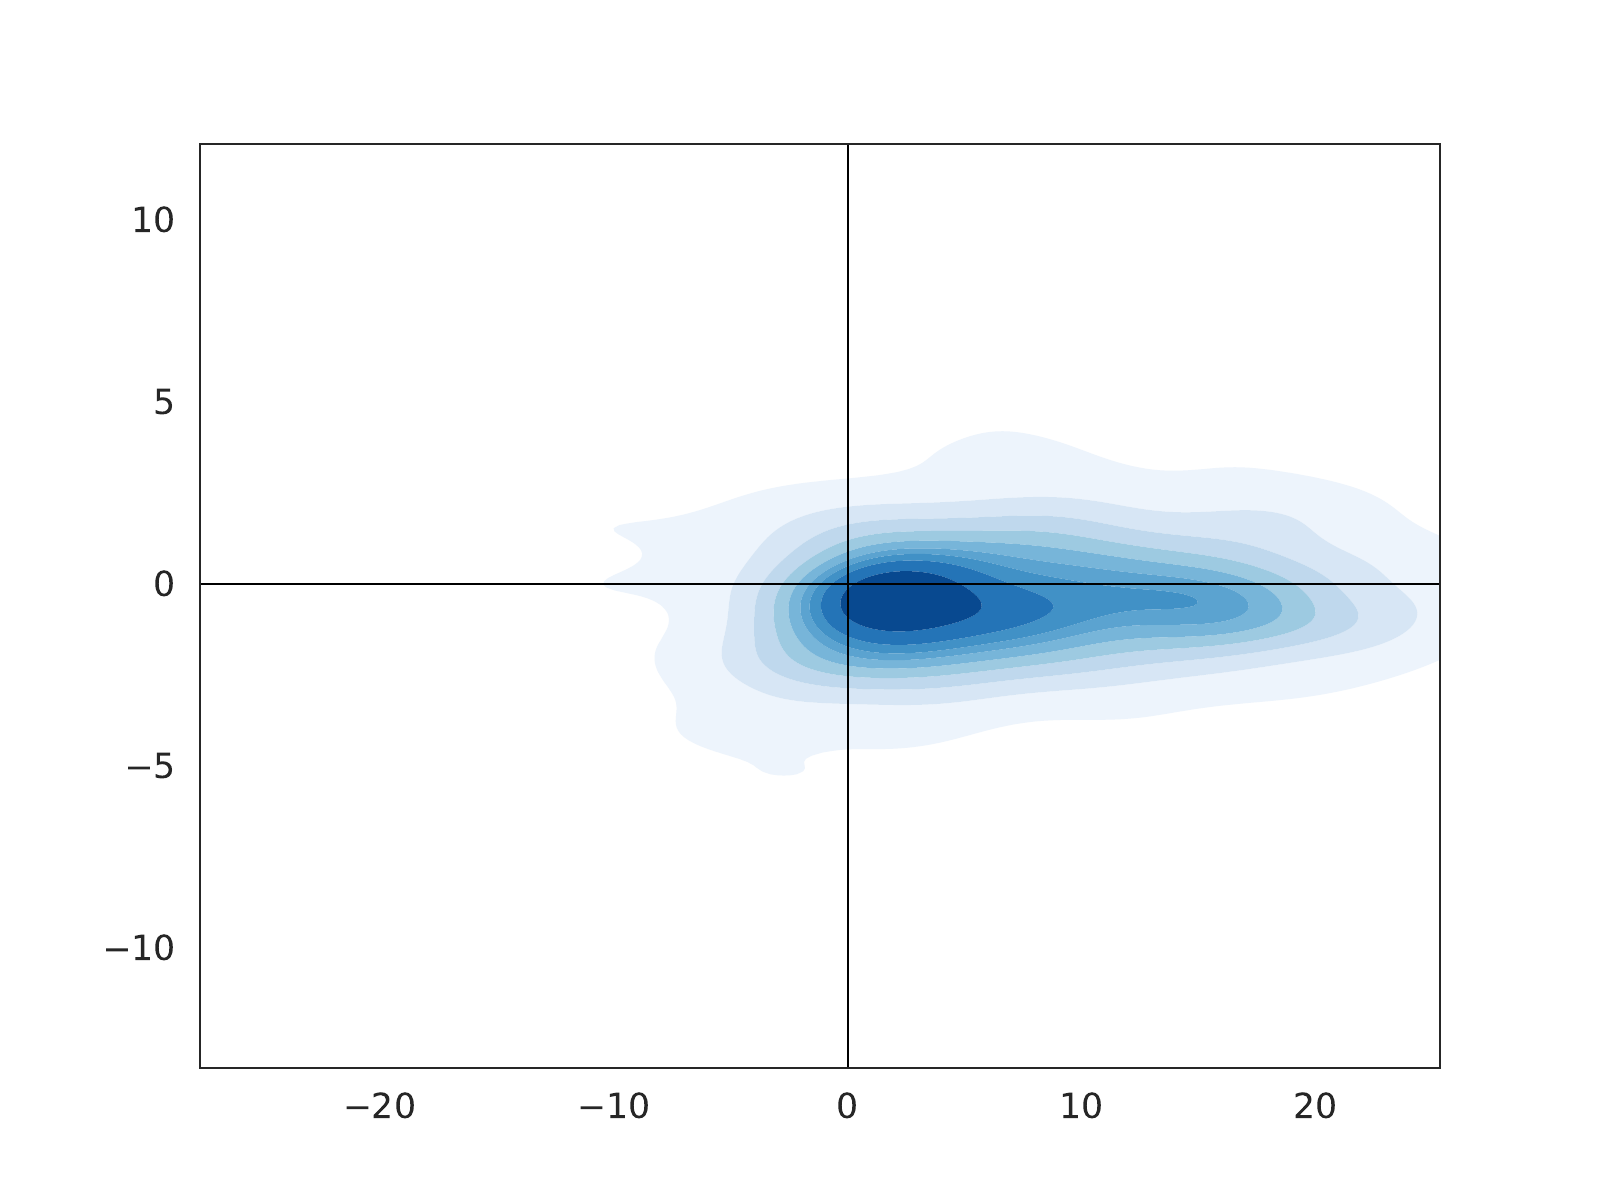} &
         %\includegraphics[trim=62 85 49 80,clip,width=0.2\columnwidth]{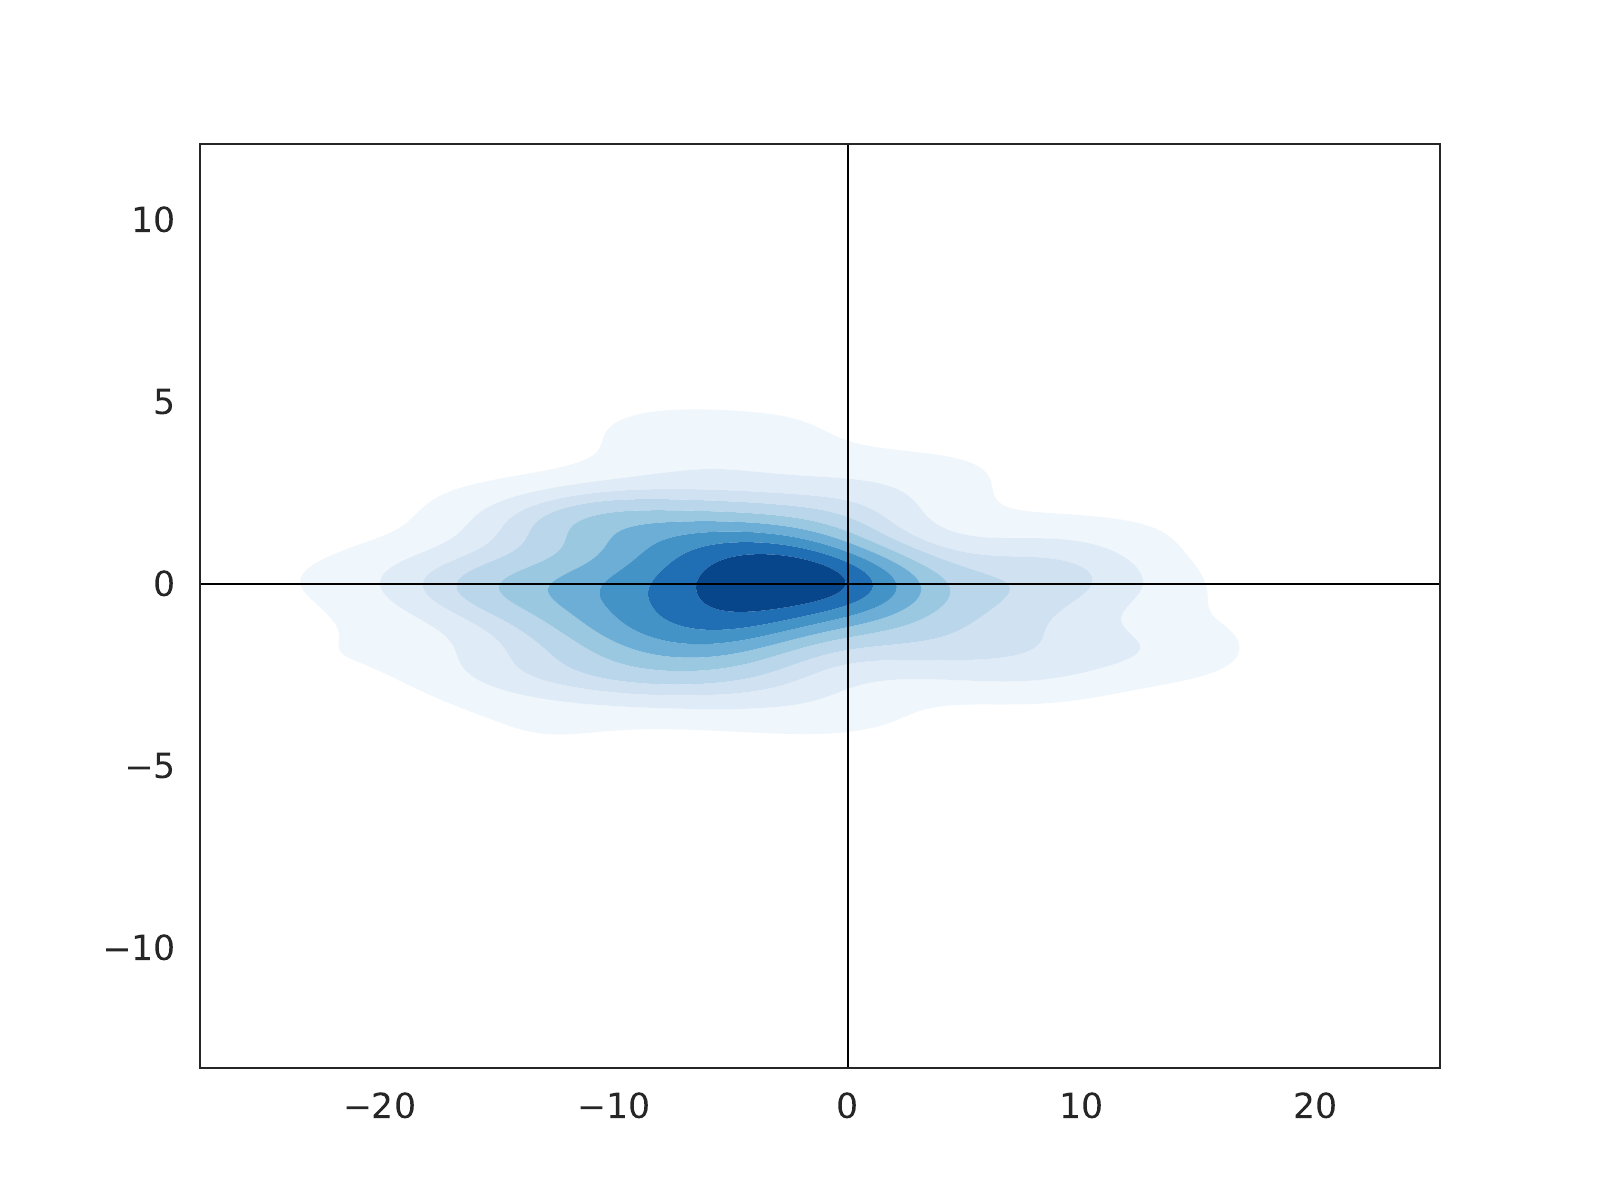} &
         %\includegraphics[trim=62 85 49 80,clip,width=0.2\columnwidth]{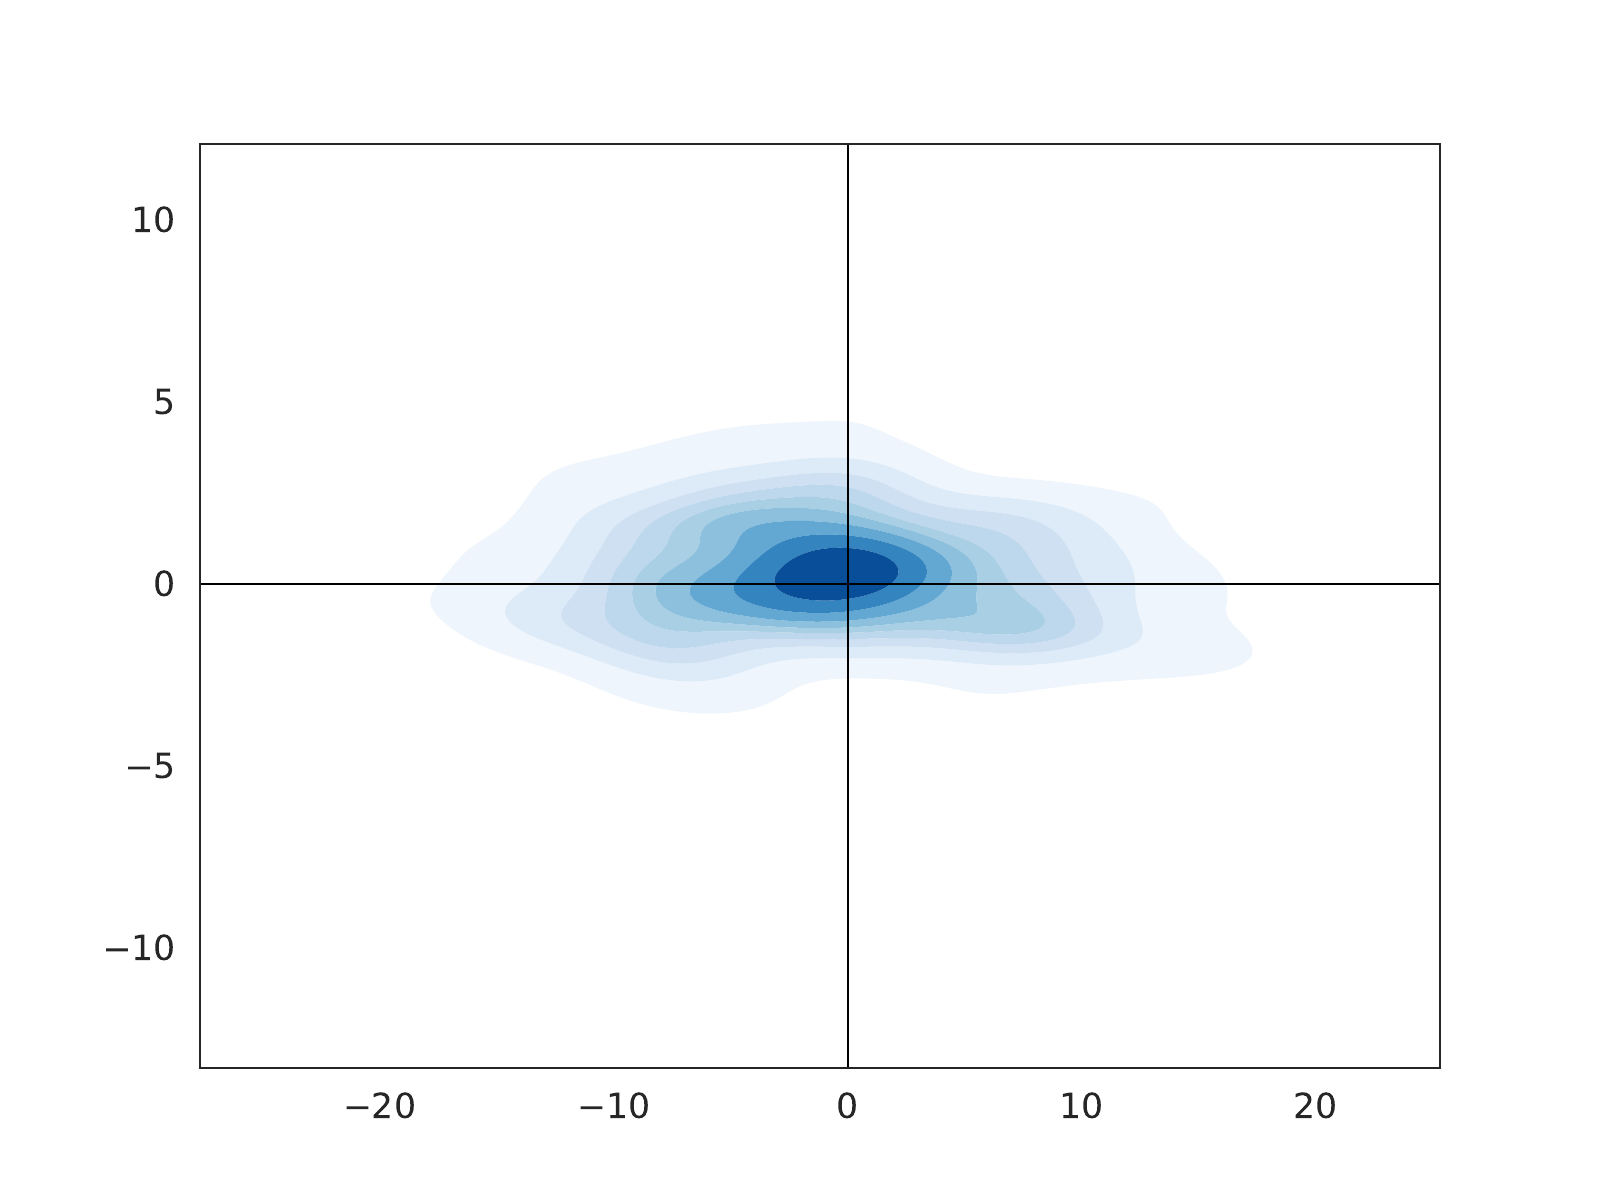} &
         %\includegraphics[trim=62 85 49 80,clip,width=0.2\columnwidth]{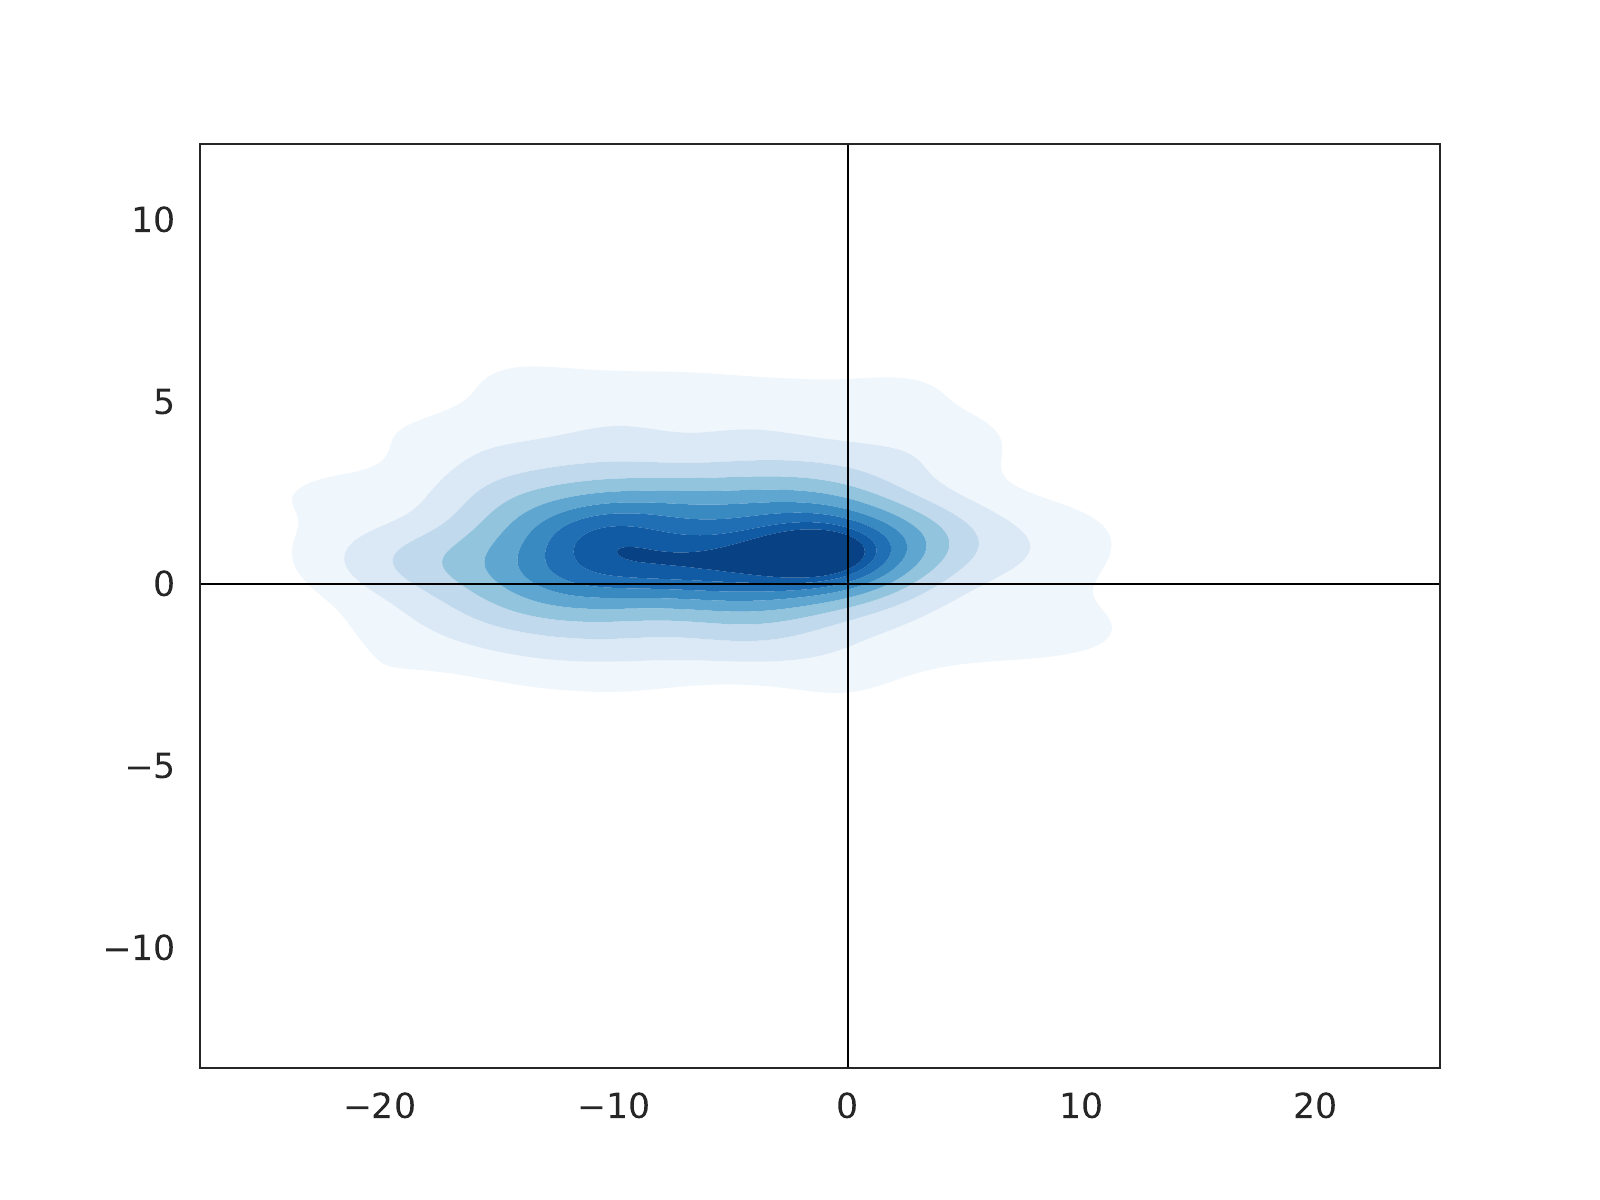} \\

    \end{tabular}
    }
    \captionof{figure}{Videos generated by \methodname~on the \emph{Tennis} dataset. We generate a sequence for each learned action by repeatedly inputting the current action starting from the same initial frame. The model learns actions that correspond horizontal (Act. 4 and Act. 7) and vertical player movement (Act. 2 and Act. 3), no movement (Act. 6), and ball hitting (Act. 1, Act. 5). Additional videos are shown in the corresponding section of the \href{run:./main.html}{main.html} page.}
    \label{fig:tennis_action_unrolls}
\end{table*}
