# Supplementary material for: Playable Video Generation
Source: arXiv:2101.12195 source file (2021-01-28)
Supplement: Supplementary file 4 [file breakout_reconstruction_0.tex]

\begin{table*}
    \centering
    
    \resizebox{0.8\linewidth}{!}{
    \setlength\tabcolsep{0pt}
    \footnotesize
    
    \begin{tabular}{l@{\hskip 1mm}ccccccccccc}
         & $t=1$ & $t=4$ & $t=7$ & $t=10$ & $t=13$ & $t=16$ & $t=19$ & $t=22$ & $t=25$ & $t=28$ & $t=30$  \\
         \rotatebox{90}{\hspace{5.5mm}Original} &
         \includegraphics[width=0.2\columnwidth]{supplementary_resources/breakout/original/0/00000.png} & 
         \includegraphics[width=0.2\columnwidth]{supplementary_resources/breakout/original/0/00003.png} & 
         \includegraphics[width=0.2\columnwidth]{supplementary_resources/breakout/original/0/00006.png} & 
         \includegraphics[width=0.2\columnwidth]{supplementary_resources/breakout/original/0/00009.png} & 
         \includegraphics[width=0.2\columnwidth]{supplementary_resources/breakout/original/0/00012.png} & 
         \includegraphics[width=0.2\columnwidth]{supplementary_resources/breakout/original/0/00015.png} & 
         \includegraphics[width=0.2\columnwidth]{supplementary_resources/breakout/original/0/00018.png} & 
         \includegraphics[width=0.2\columnwidth]{supplementary_resources/breakout/original/0/00021.png} & 
         \includegraphics[width=0.2\columnwidth]{supplementary_resources/breakout/original/0/00024.png} & 
         \includegraphics[width=0.2\columnwidth]{supplementary_resources/breakout/original/0/00027.png} & 
         \includegraphics[width=0.2\columnwidth]{supplementary_resources/breakout/original/0/00031.png} \\
         
         \rotatebox{90}{\hspace{2mm}MoCoGAN \cite{tulyakov2018moco}} &
         \includegraphics[width=0.2\columnwidth]{supplementary_resources/breakout/moco/0/00000.png} & 
         \includegraphics[width=0.2\columnwidth]{supplementary_resources/breakout/moco/0/00003.png} & 
         \includegraphics[width=0.2\columnwidth]{supplementary_resources/breakout/moco/0/00006.png} & 
         \includegraphics[width=0.2\columnwidth]{supplementary_resources/breakout/moco/0/00009.png} & 
         \includegraphics[width=0.2\columnwidth]{supplementary_resources/breakout/moco/0/00012.png} & 
         \includegraphics[width=0.2\columnwidth]{supplementary_resources/breakout/moco/0/00015.png} & 
         \includegraphics[width=0.2\columnwidth]{supplementary_resources/breakout/moco/0/00018.png} & 
         \includegraphics[width=0.2\columnwidth]{supplementary_resources/breakout/moco/0/00021.png} & 
         \includegraphics[width=0.2\columnwidth]{supplementary_resources/breakout/moco/0/00024.png} & 
         \includegraphics[width=0.2\columnwidth]{supplementary_resources/breakout/moco/0/00027.png} & 
         \includegraphics[width=0.2\columnwidth]{supplementary_resources/breakout/moco/0/00031.png} \\
         
         \rotatebox{90}{\hspace{3mm}MoCoGAN+} &
         \includegraphics[width=0.2\columnwidth]{supplementary_resources/breakout/moco_plus/0/00000.png} & 
         \includegraphics[width=0.2\columnwidth]{supplementary_resources/breakout/moco_plus/0/00003.png} & 
         \includegraphics[width=0.2\columnwidth]{supplementary_resources/breakout/moco_plus/0/00006.png} & 
         \includegraphics[width=0.2\columnwidth]{supplementary_resources/breakout/moco_plus/0/00009.png} & 
         \includegraphics[width=0.2\columnwidth]{supplementary_resources/breakout/moco_plus/0/00012.png} & 
         \includegraphics[width=0.2\columnwidth]{supplementary_resources/breakout/moco_plus/0/00015.png} & 
         \includegraphics[width=0.2\columnwidth]{supplementary_resources/breakout/moco_plus/0/00018.png} & 
         \includegraphics[width=0.2\columnwidth]{supplementary_resources/breakout/moco_plus/0/00021.png} & 
         \includegraphics[width=0.2\columnwidth]{supplementary_resources/breakout/moco_plus/0/00024.png} & 
         \includegraphics[width=0.2\columnwidth]{supplementary_resources/breakout/moco_plus/0/00027.png} & 
         \includegraphics[width=0.2\columnwidth]{supplementary_resources/breakout/moco_plus/0/00031.png} \\
         
         \rotatebox{90}{\hspace{5mm}SAVP \cite{lee2018savp}} &
         \includegraphics[width=0.2\columnwidth]{supplementary_resources/breakout/savp/0/00000.png} & 
         \includegraphics[width=0.2\columnwidth]{supplementary_resources/breakout/savp/0/00003.png} & 
         \includegraphics[width=0.2\columnwidth]{supplementary_resources/breakout/savp/0/00006.png} & 
         \includegraphics[width=0.2\columnwidth]{supplementary_resources/breakout/savp/0/00009.png} & 
         \includegraphics[width=0.2\columnwidth]{supplementary_resources/breakout/savp/0/00012.png} & 
         \includegraphics[width=0.2\columnwidth]{supplementary_resources/breakout/savp/0/00015.png} & 
         \includegraphics[width=0.2\columnwidth]{supplementary_resources/breakout/savp/0/00018.png} & 
         \includegraphics[width=0.2\columnwidth]{supplementary_resources/breakout/savp/0/00021.png} & 
         \includegraphics[width=0.2\columnwidth]{supplementary_resources/breakout/savp/0/00024.png} & 
         \includegraphics[width=0.2\columnwidth]{supplementary_resources/breakout/savp/0/00027.png} & 
         \includegraphics[width=0.2\columnwidth]{supplementary_resources/breakout/savp/0/00031.png} \\
         
         \rotatebox{90}{\hspace{6mm}SAVP+} &
         \includegraphics[width=0.2\columnwidth]{supplementary_resources/breakout/savp_plus/0/00000.png} & 
         \includegraphics[width=0.2\columnwidth]{supplementary_resources/breakout/savp_plus/0/00003.png} & 
         \includegraphics[width=0.2\columnwidth]{supplementary_resources/breakout/savp_plus/0/00006.png} & 
         \includegraphics[width=0.2\columnwidth]{supplementary_resources/breakout/savp_plus/0/00009.png} & 
         \includegraphics[width=0.2\columnwidth]{supplementary_resources/breakout/savp_plus/0/00012.png} & 
         \includegraphics[width=0.2\columnwidth]{supplementary_resources/breakout/savp_plus/0/00015.png} & 
         \includegraphics[width=0.2\columnwidth]{supplementary_resources/breakout/savp_plus/0/00018.png} & 
         \includegraphics[width=0.2\columnwidth]{supplementary_resources/breakout/savp_plus/0/00021.png} & 
         \includegraphics[width=0.2\columnwidth]{supplementary_resources/breakout/savp_plus/0/00024.png} & 
         \includegraphics[width=0.2\columnwidth]{supplementary_resources/breakout/savp_plus/0/00027.png} & 
         \includegraphics[width=0.2\columnwidth]{supplementary_resources/breakout/savp_plus/0/00031.png} \\
         
         \rotatebox{90}{\hspace{7.5mm}Ours} &
         \includegraphics[width=0.2\columnwidth]{supplementary_resources/breakout/ours/0/00000.png} & 
         \includegraphics[width=0.2\columnwidth]{supplementary_resources/breakout/ours/0/00003.png} & 
         \includegraphics[width=0.2\columnwidth]{supplementary_resources/breakout/ours/0/00006.png} & 
         \includegraphics[width=0.2\columnwidth]{supplementary_resources/breakout/ours/0/00009.png} & 
         \includegraphics[width=0.2\columnwidth]{supplementary_resources/breakout/ours/0/00012.png} & 
         \includegraphics[width=0.2\columnwidth]{supplementary_resources/breakout/ours/0/00015.png} & 
         \includegraphics[width=0.2\columnwidth]{supplementary_resources/breakout/ours/0/00018.png} & 
         \includegraphics[width=0.2\columnwidth]{supplementary_resources/breakout/ours/0/00021.png} & 
         \includegraphics[width=0.2\columnwidth]{supplementary_resources/breakout/ours/0/00024.png} & 
         \includegraphics[width=0.2\columnwidth]{supplementary_resources/breakout/ours/0/00027.png} & 
         \includegraphics[width=0.2\columnwidth]{supplementary_resources/breakout/ours/0/00031.png} \\

    \end{tabular}
    }
    \captionof{figure}{Reconstructed sequences on the \emph{Atari Breakout} dataset using the learned, discrete actions extracted from the original sequence as inputs.}
    \label{fig:breakout_reconstruction_0}
\end{table*}
