# Supplementary material for: Playable Video Generation
Source: arXiv:2101.12195 source file (2021-01-28)
Supplement: Supplementary file 7 [file bair_density_plots.tex]

\begin{table*}
    \centering
    
    \resizebox{\linewidth}{!}{
    \setlength\tabcolsep{0pt}
    \tiny
    
    \begin{tabular}{l@{\hskip 0.7mm}ccccccc}
         & Action 1 & Action 2 & Action 3 & Action 4 & Action 5 & Action 6 & Action 7  \\

         \rotatebox{90}{\hspace{0mm}\scalebox{1}{MoCoGAN \cite{tulyakov2018moco}}} &
         \includegraphics[trim=60 80 60 80,clip,width=0.2\columnwidth]{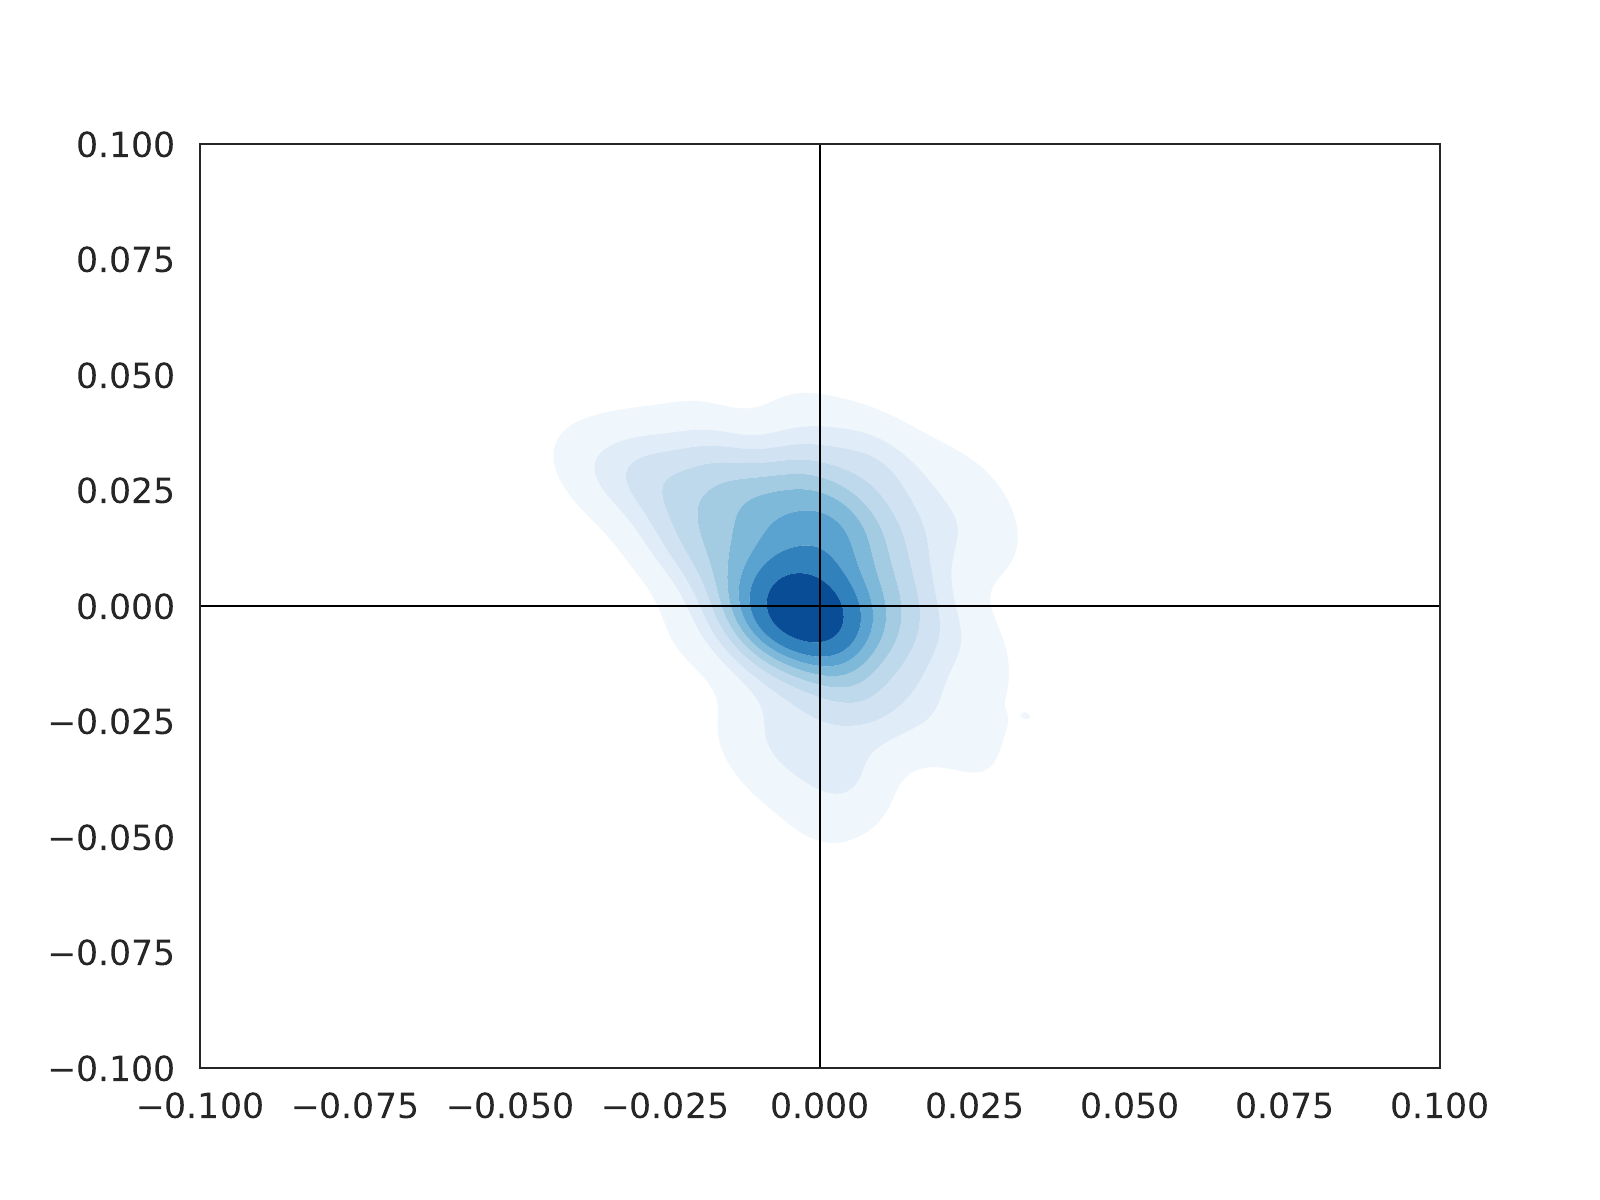} &
         \includegraphics[trim=60 80 60 80,clip,width=0.2\columnwidth]{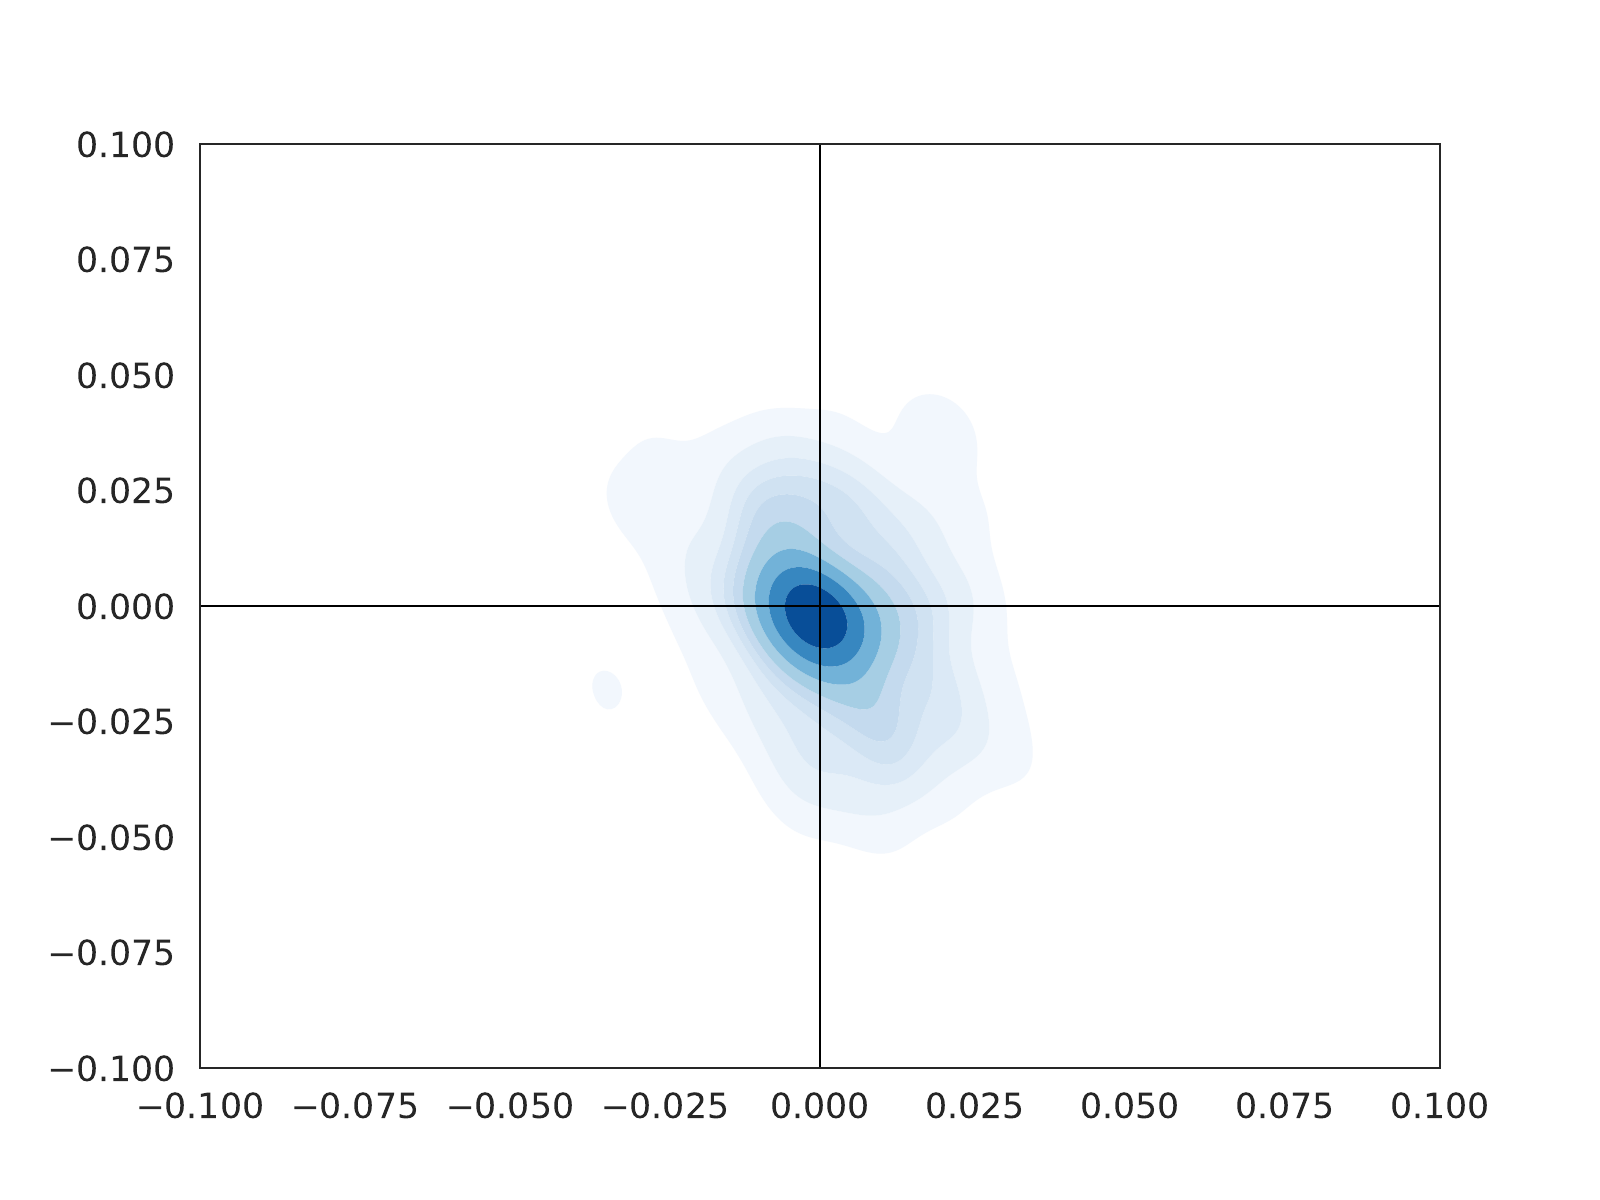} &
         \includegraphics[trim=60 80 60 80,clip,width=0.2\columnwidth]{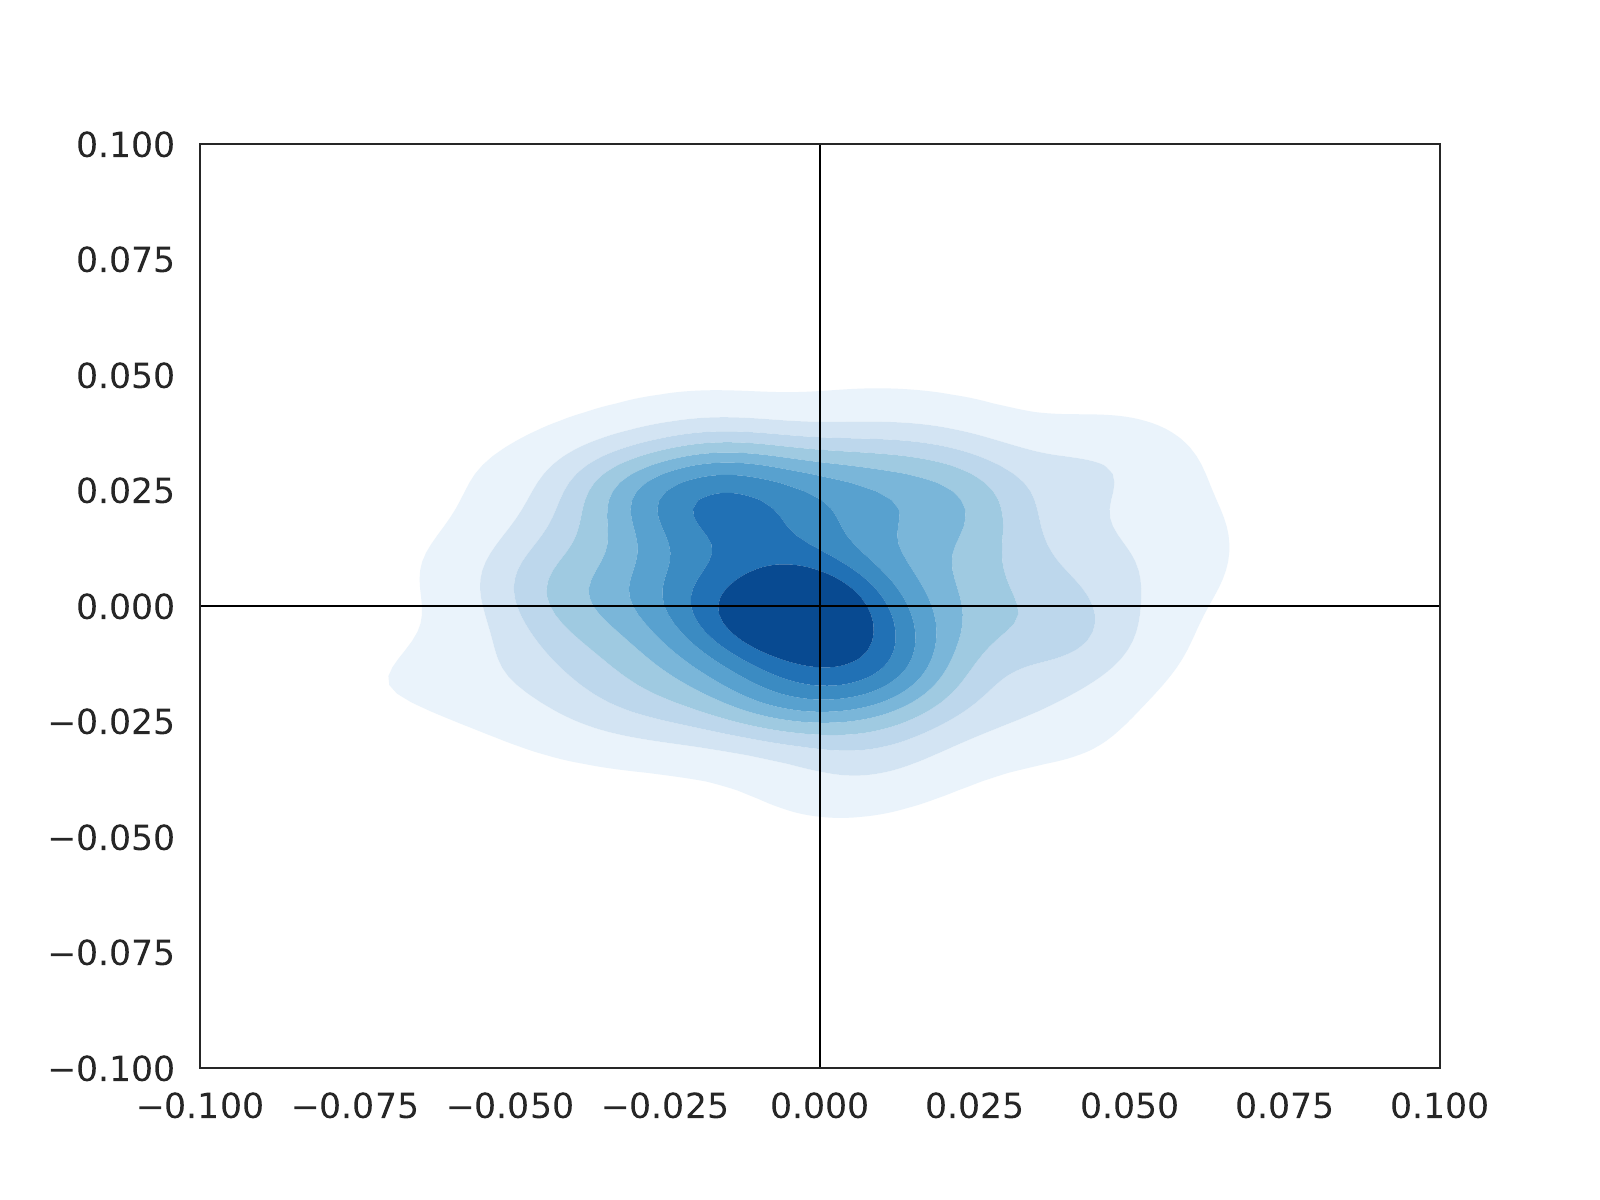} &
         \includegraphics[trim=60 80 60 80,clip,width=0.2\columnwidth]{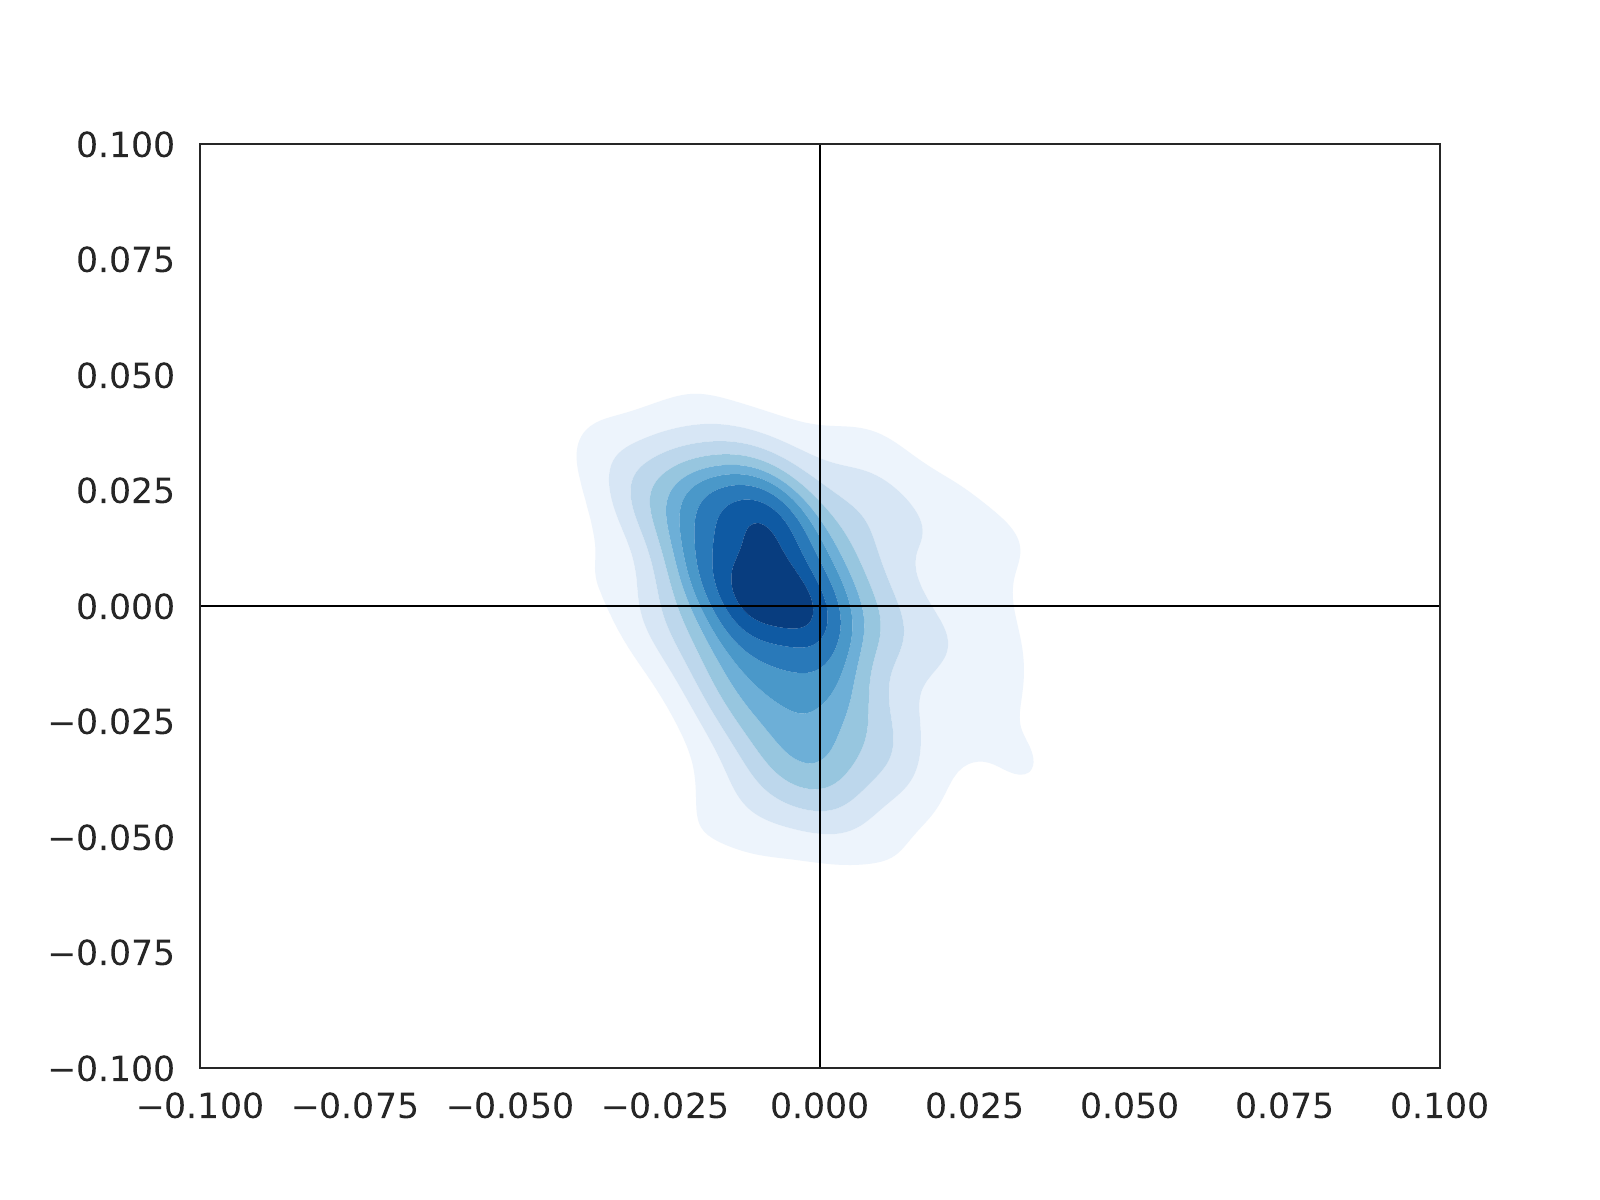} &
         \includegraphics[trim=60 80 60 80,clip,width=0.2\columnwidth]{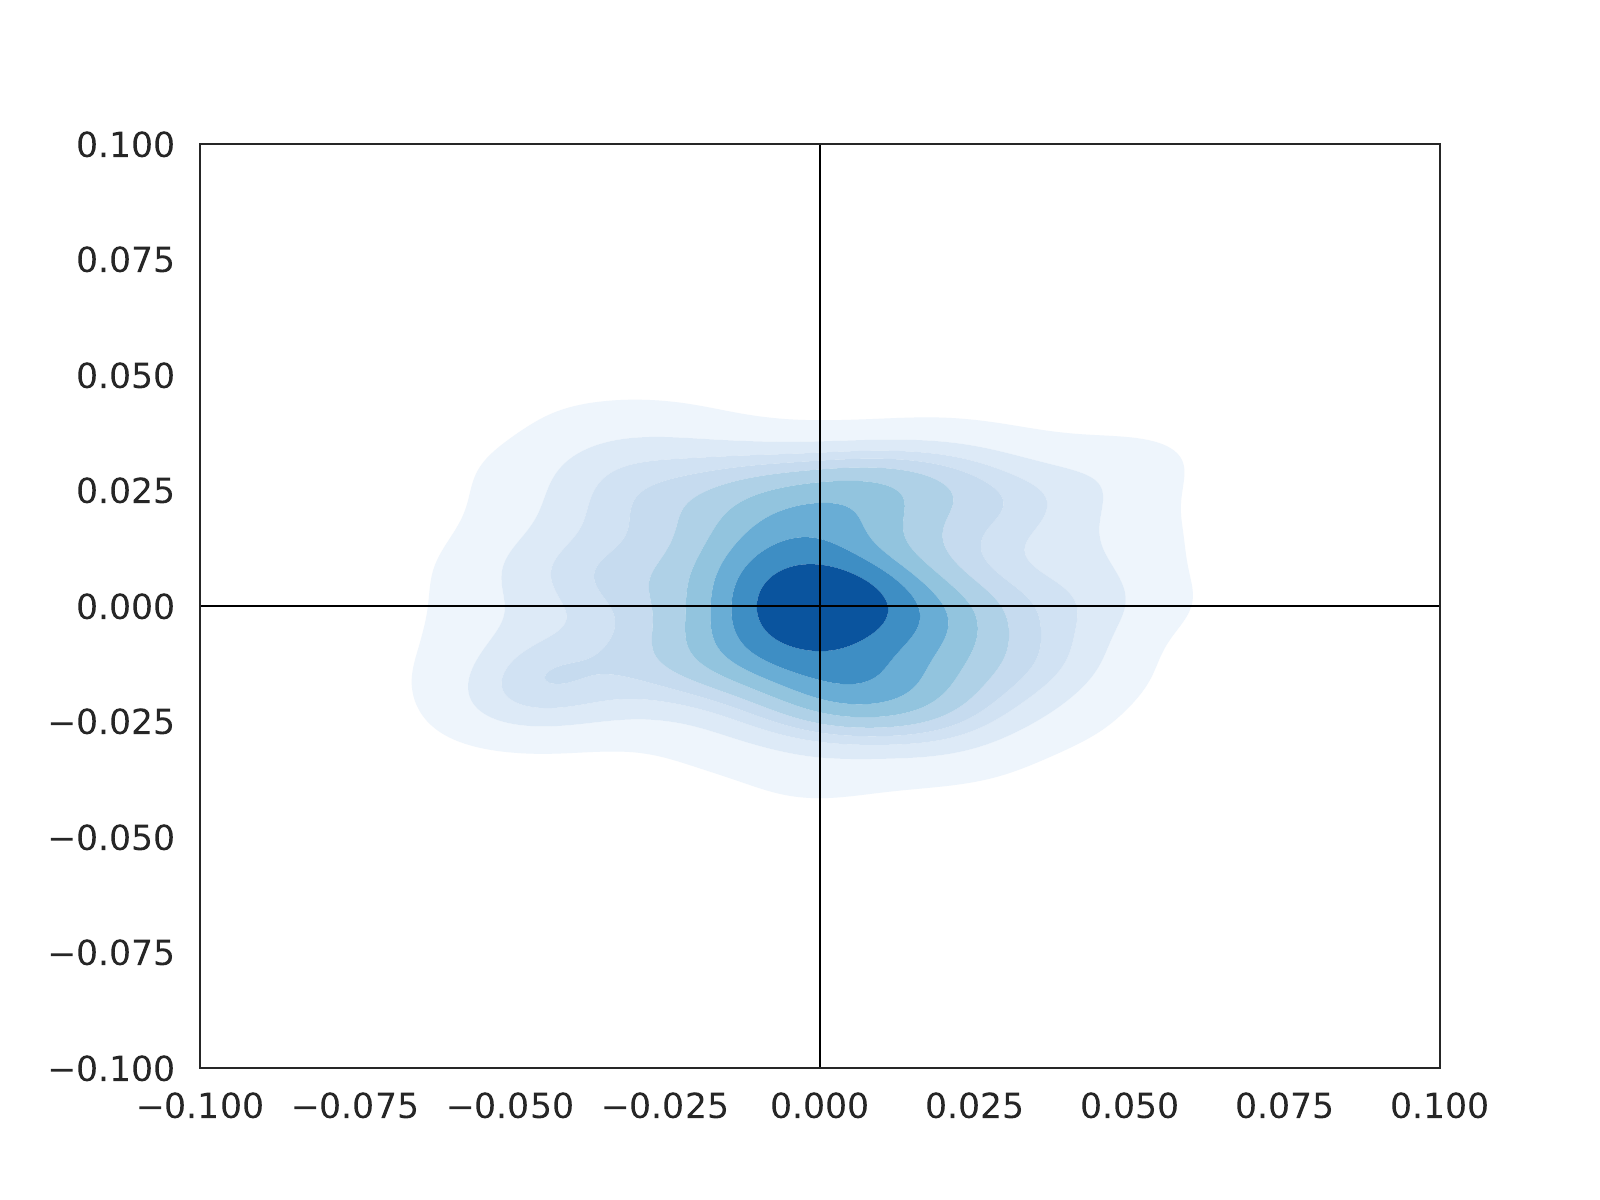} &
         \includegraphics[trim=60 80 60 80,clip,width=0.2\columnwidth]{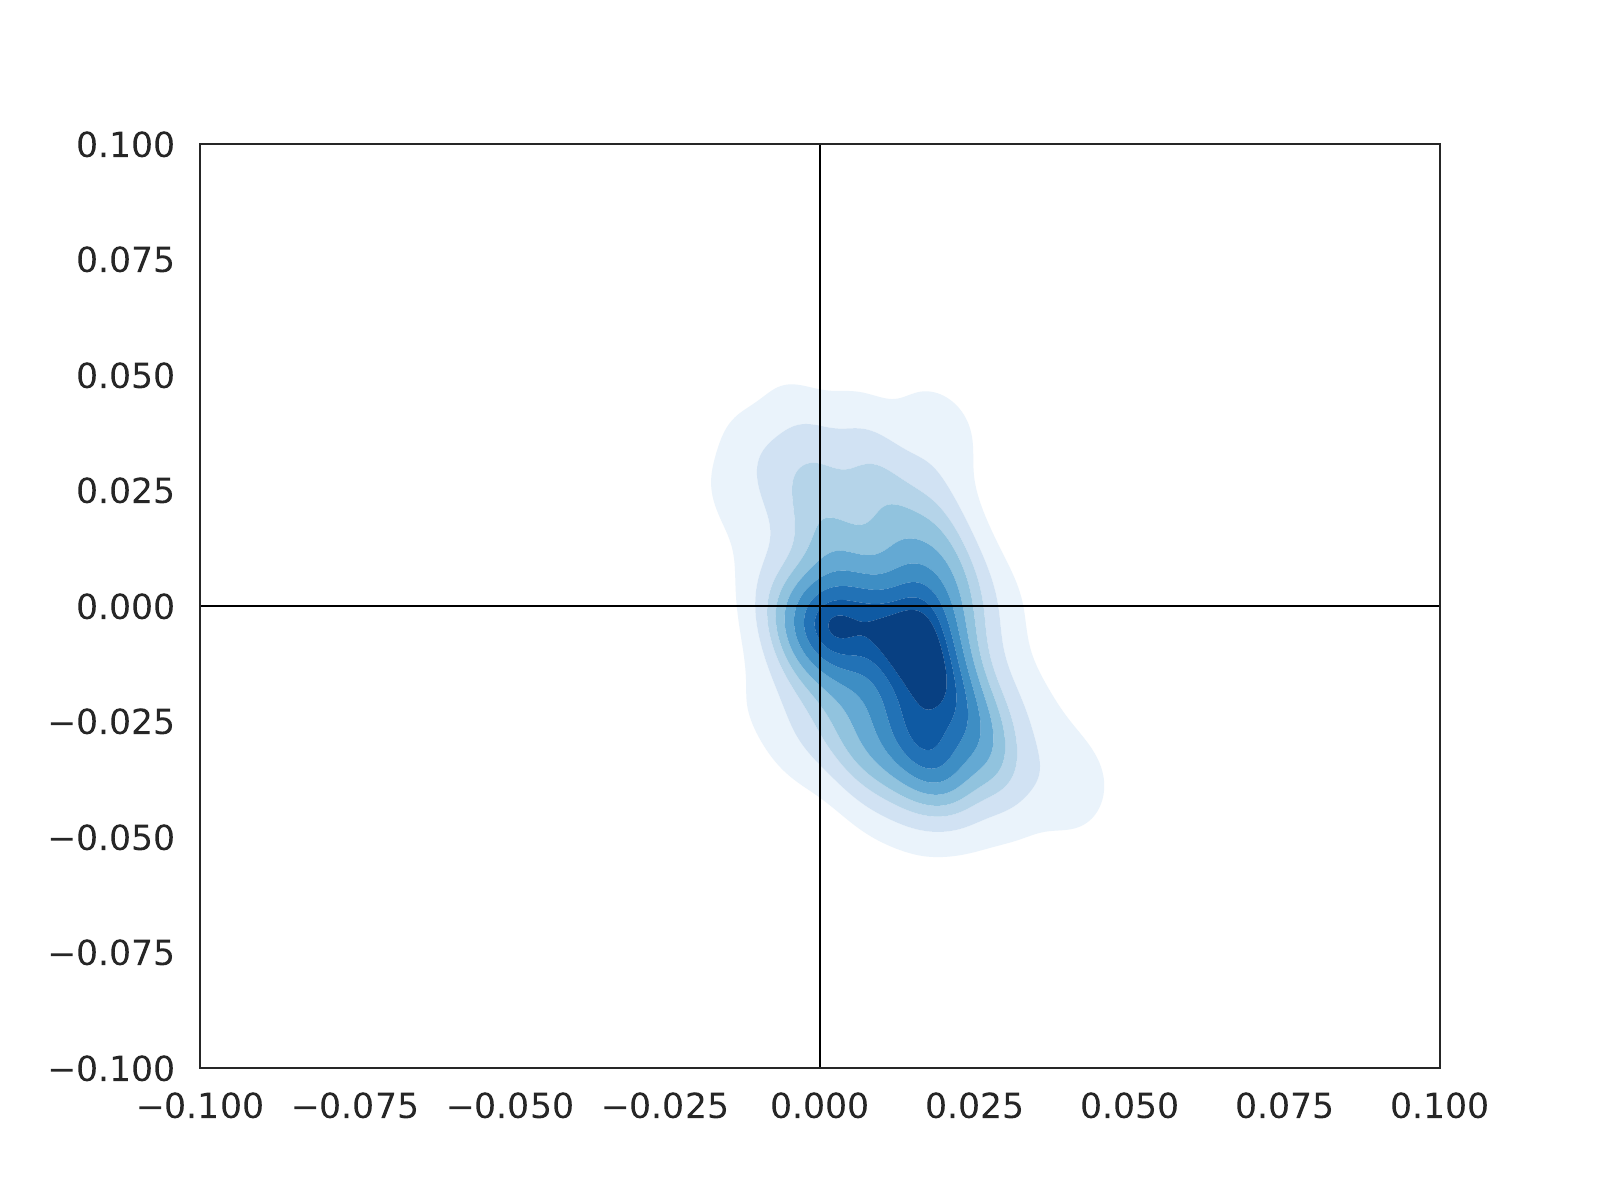} &
         \includegraphics[trim=60 80 60 80,clip,width=0.2\columnwidth]{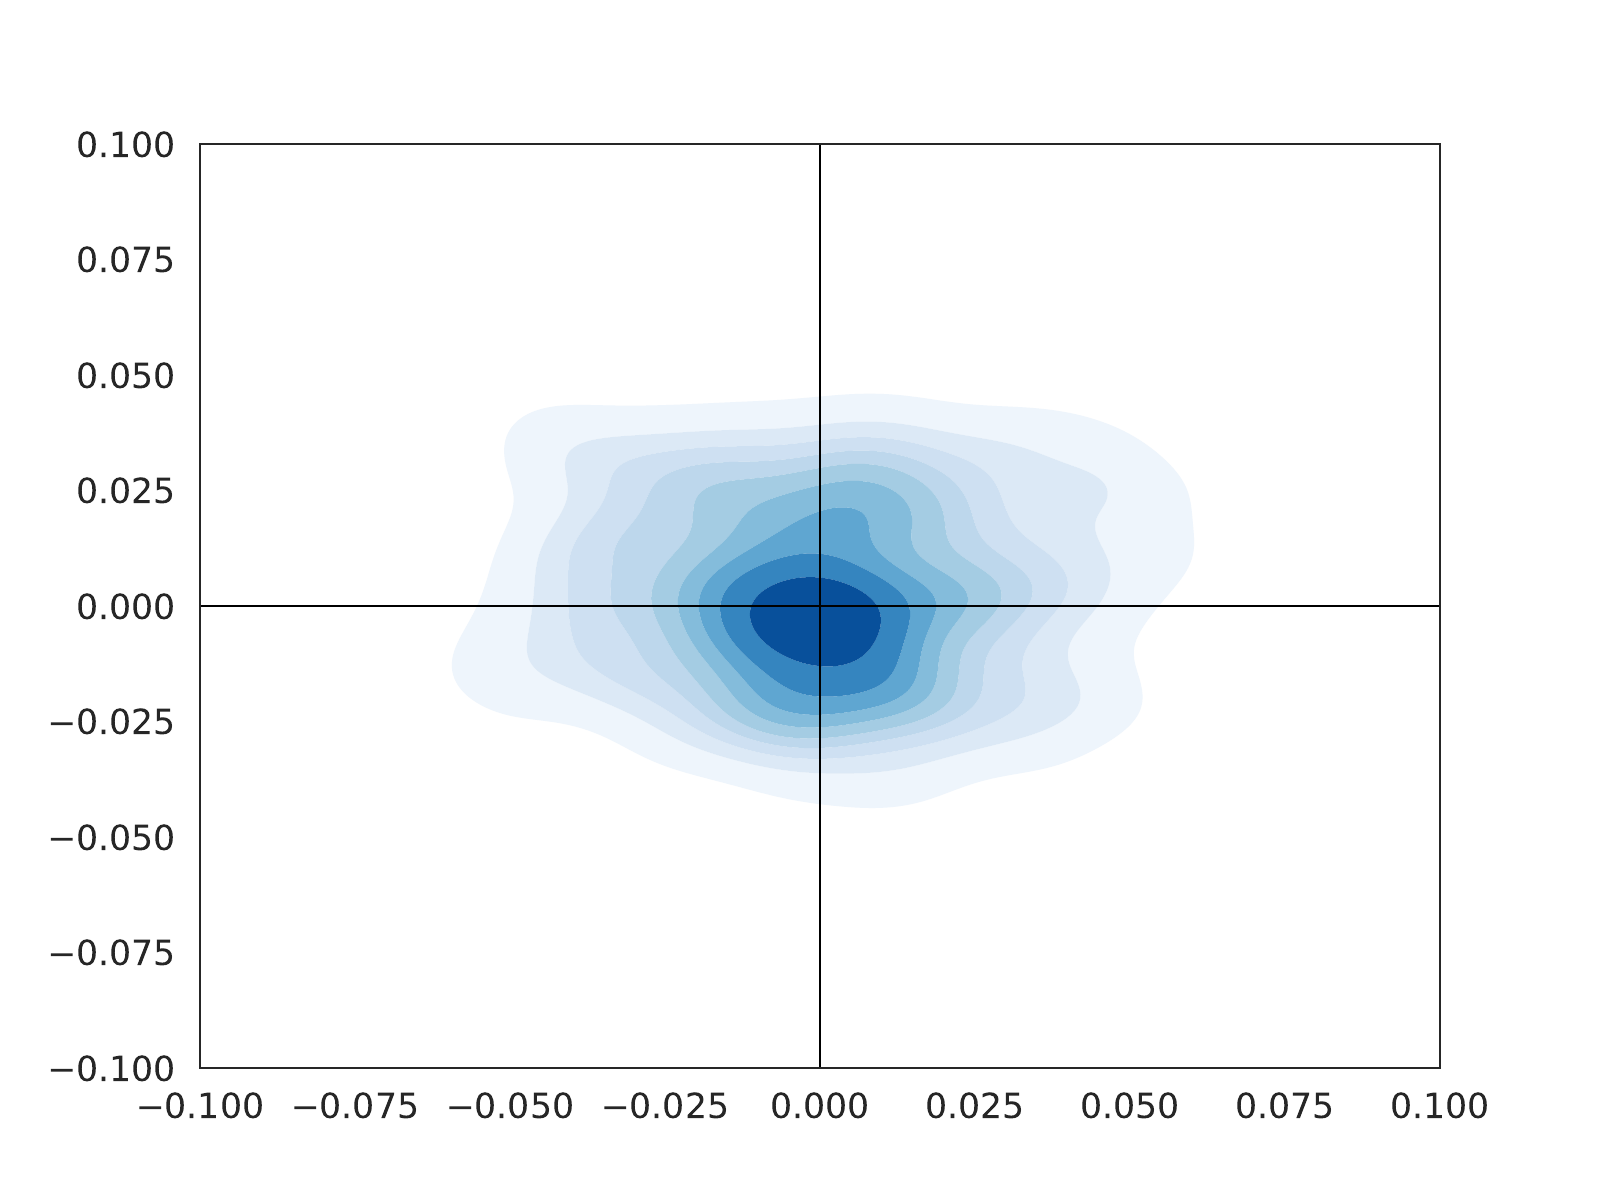} \\
         
         \rotatebox{90}{\hspace{0mm}\scalebox{1}{MoCoGAN+}} &
         \includegraphics[trim=60 80 60 80,clip,width=0.2\columnwidth]{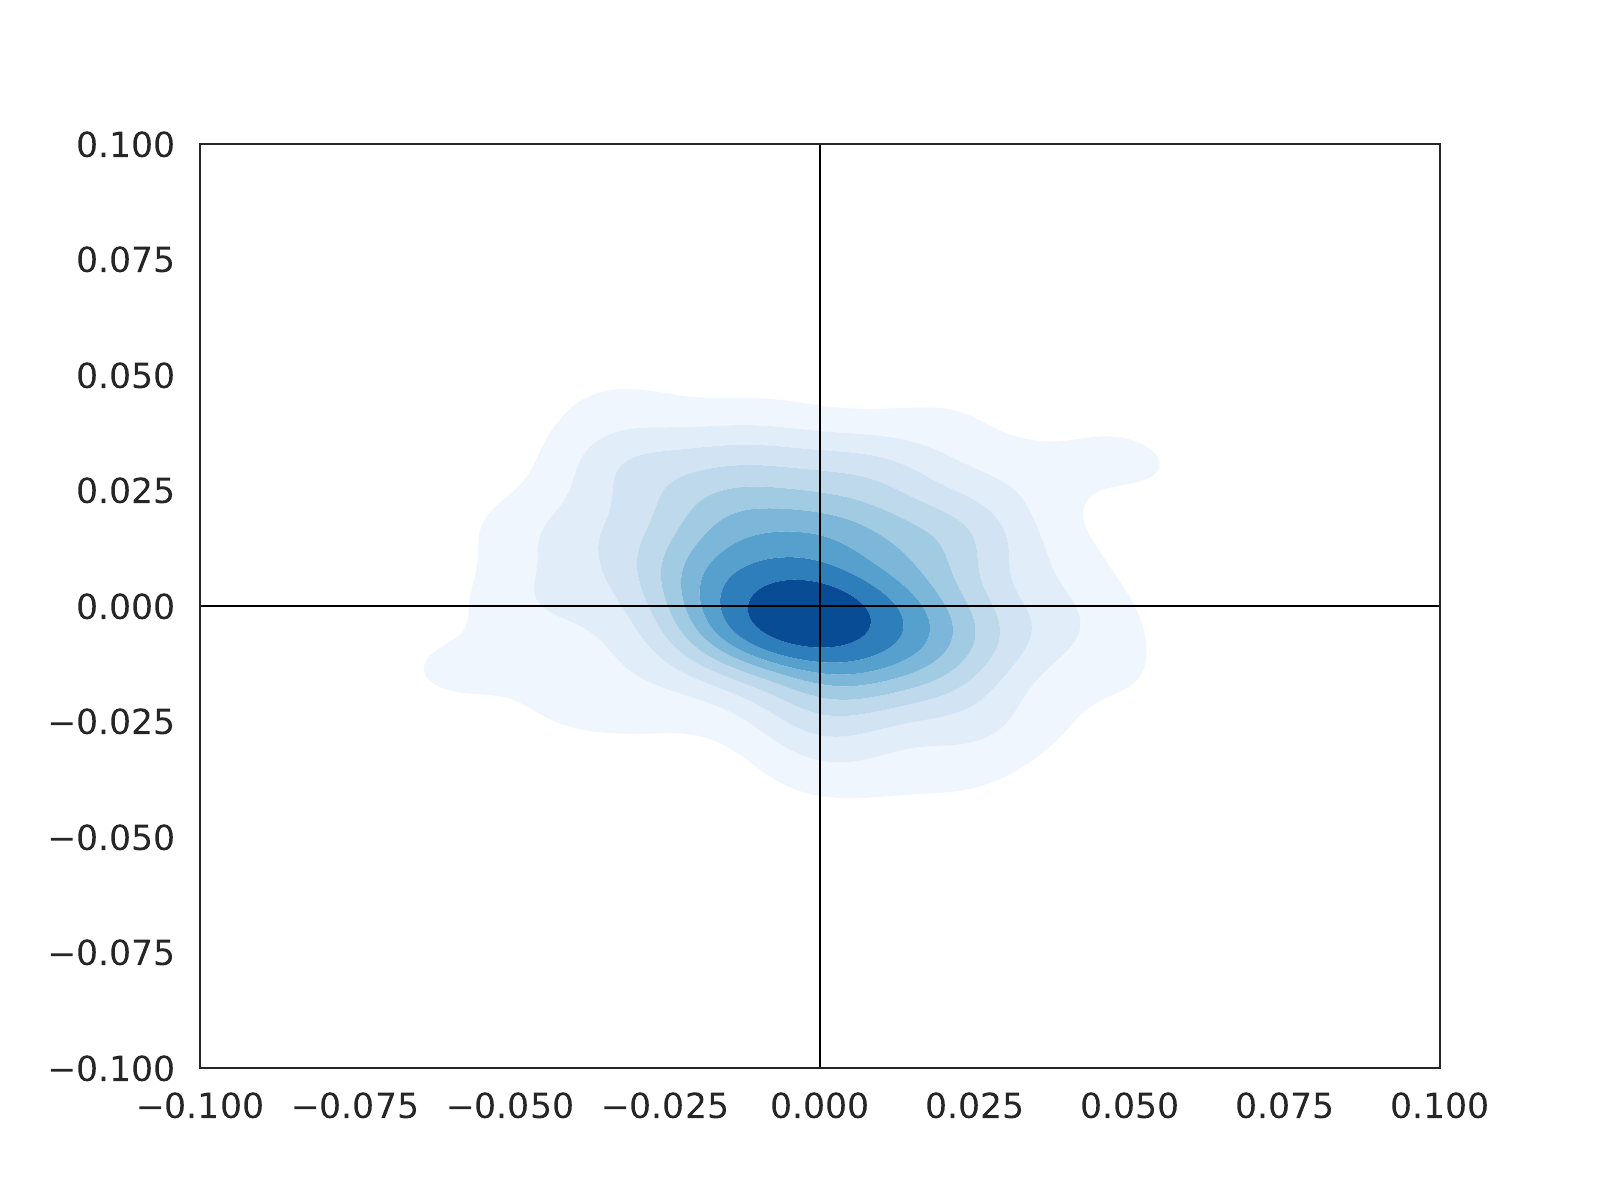} &
         \includegraphics[trim=60 80 60 80,clip,width=0.2\columnwidth]{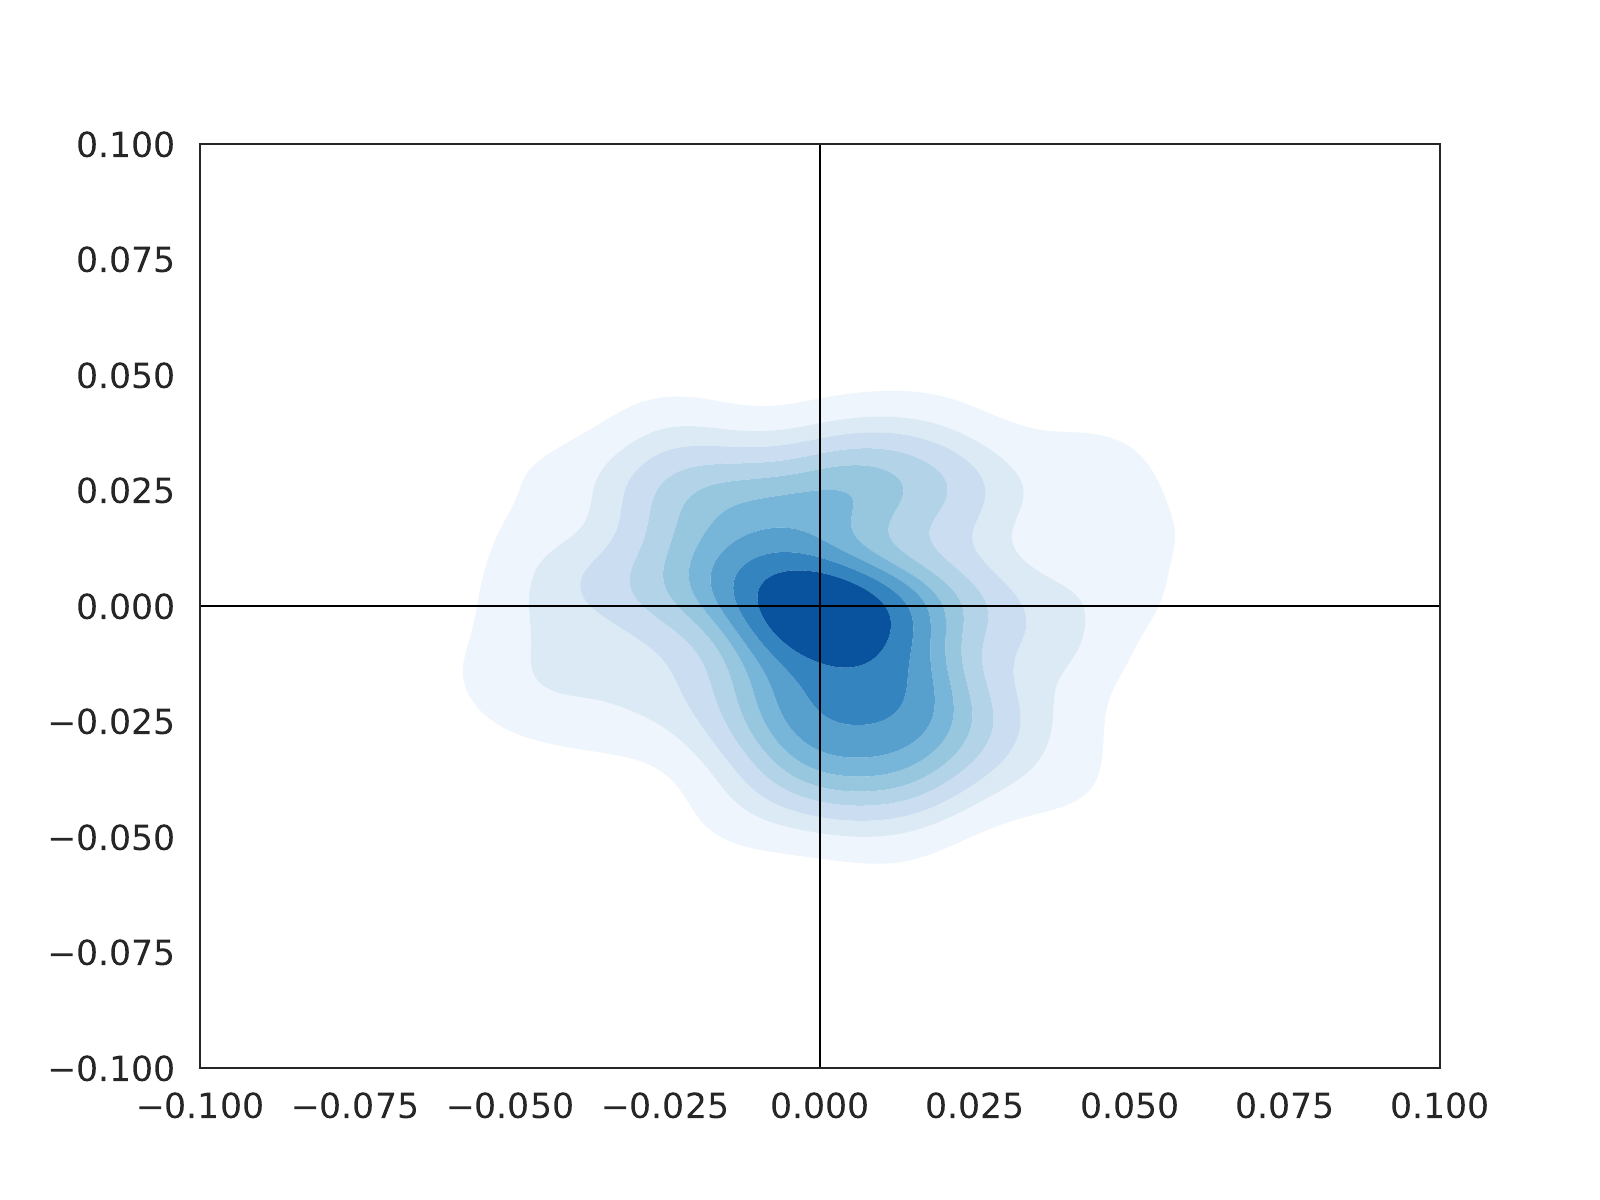} &
         \includegraphics[trim=60 80 60 80,clip,width=0.2\columnwidth]{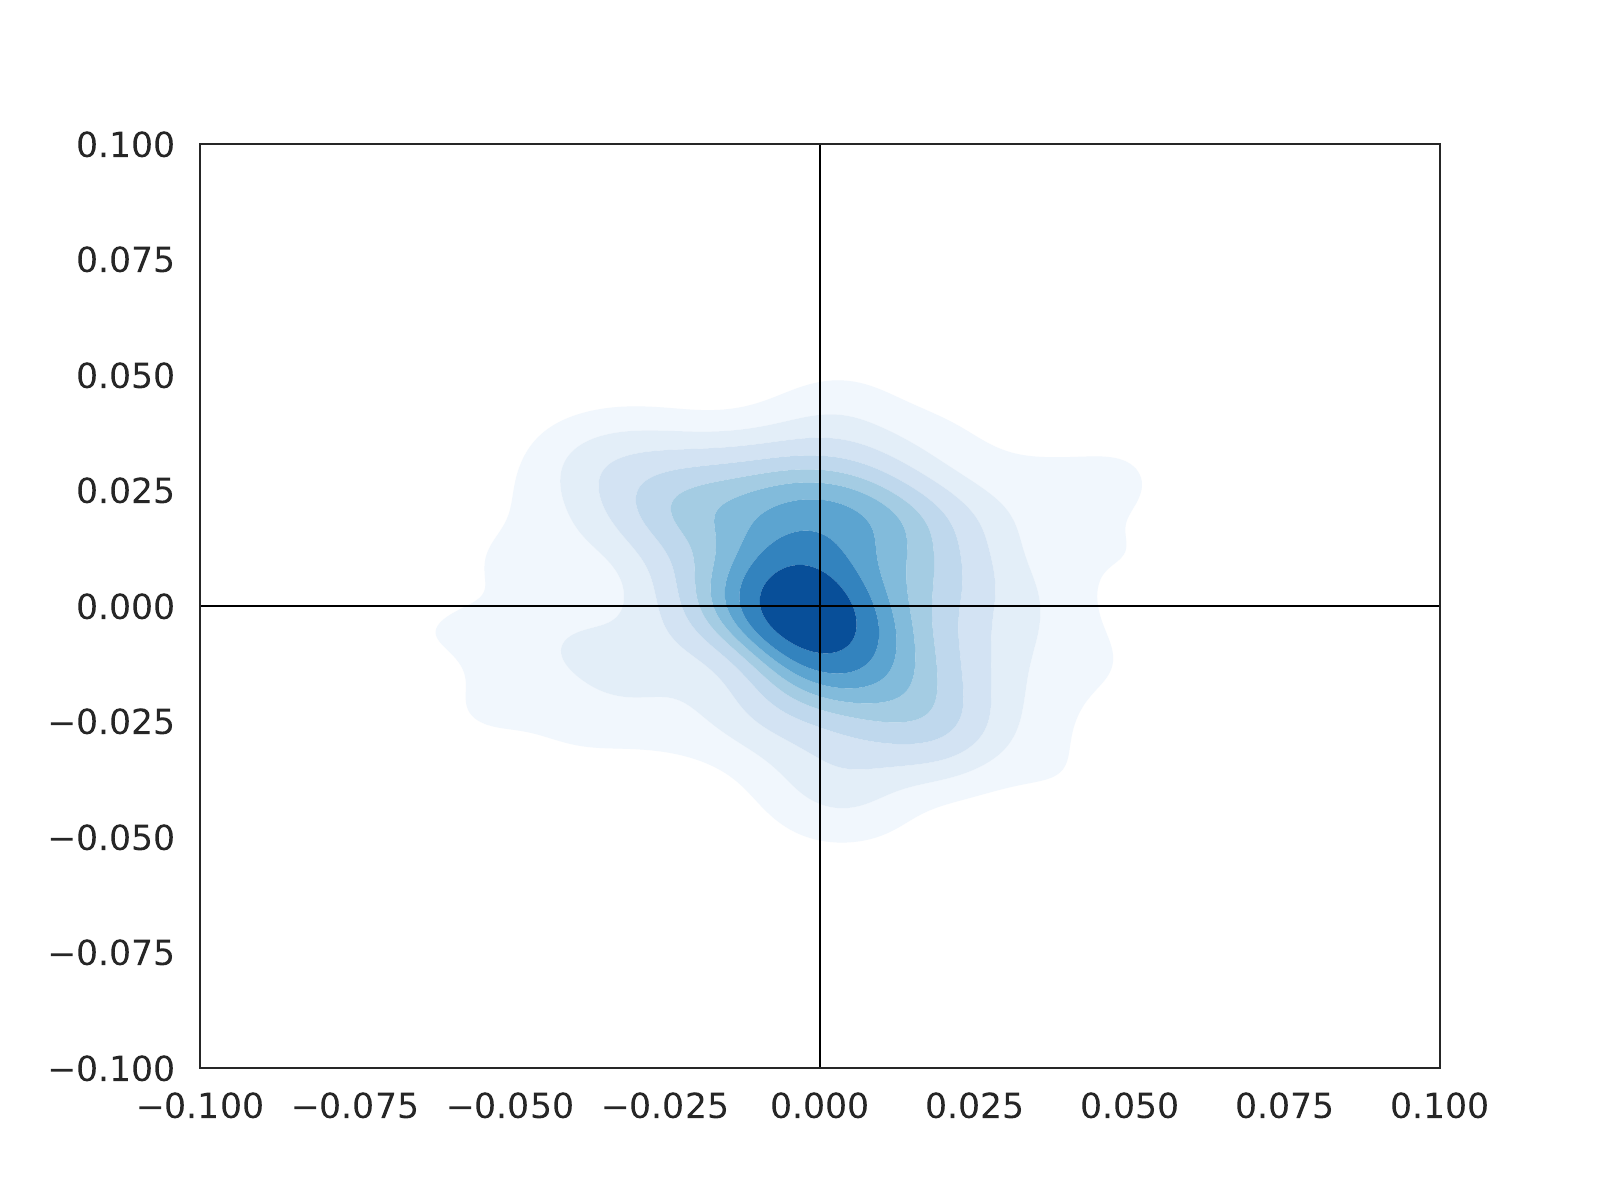} &
         \includegraphics[trim=60 80 60 80,clip,width=0.2\columnwidth]{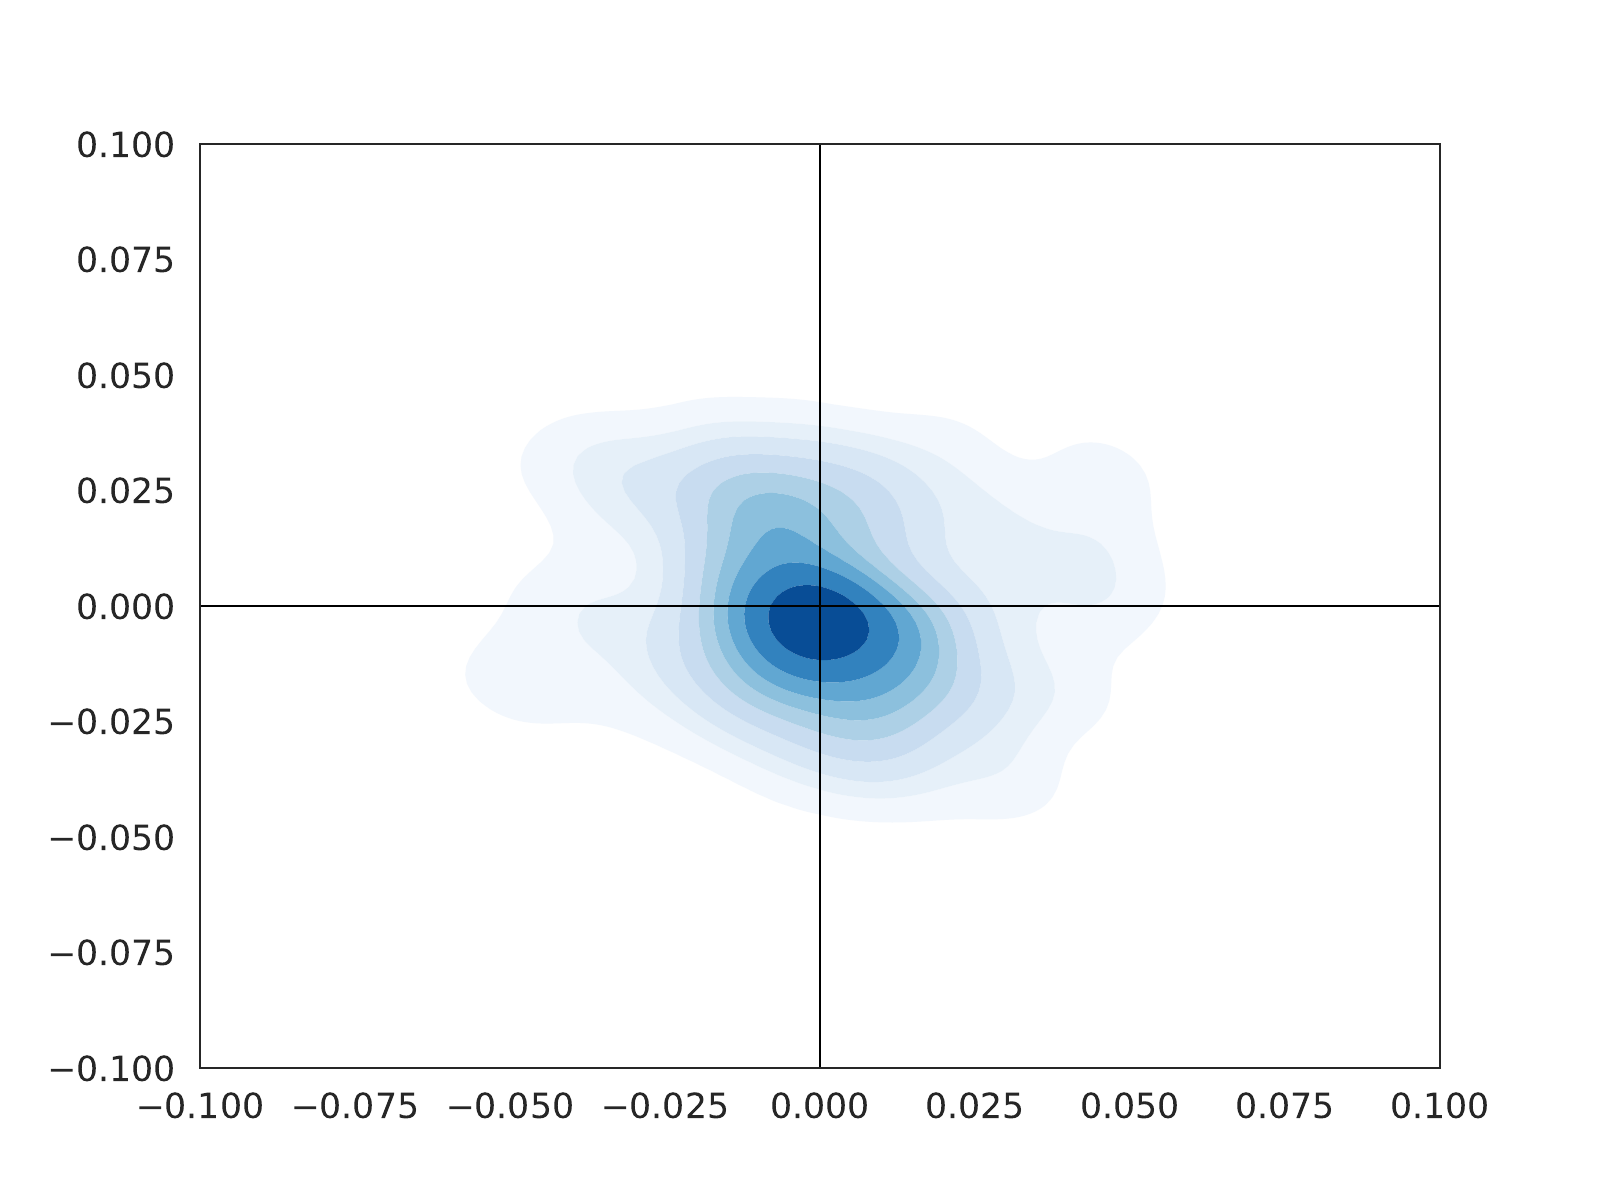} &
         \includegraphics[trim=60 80 60 80,clip,width=0.2\columnwidth]{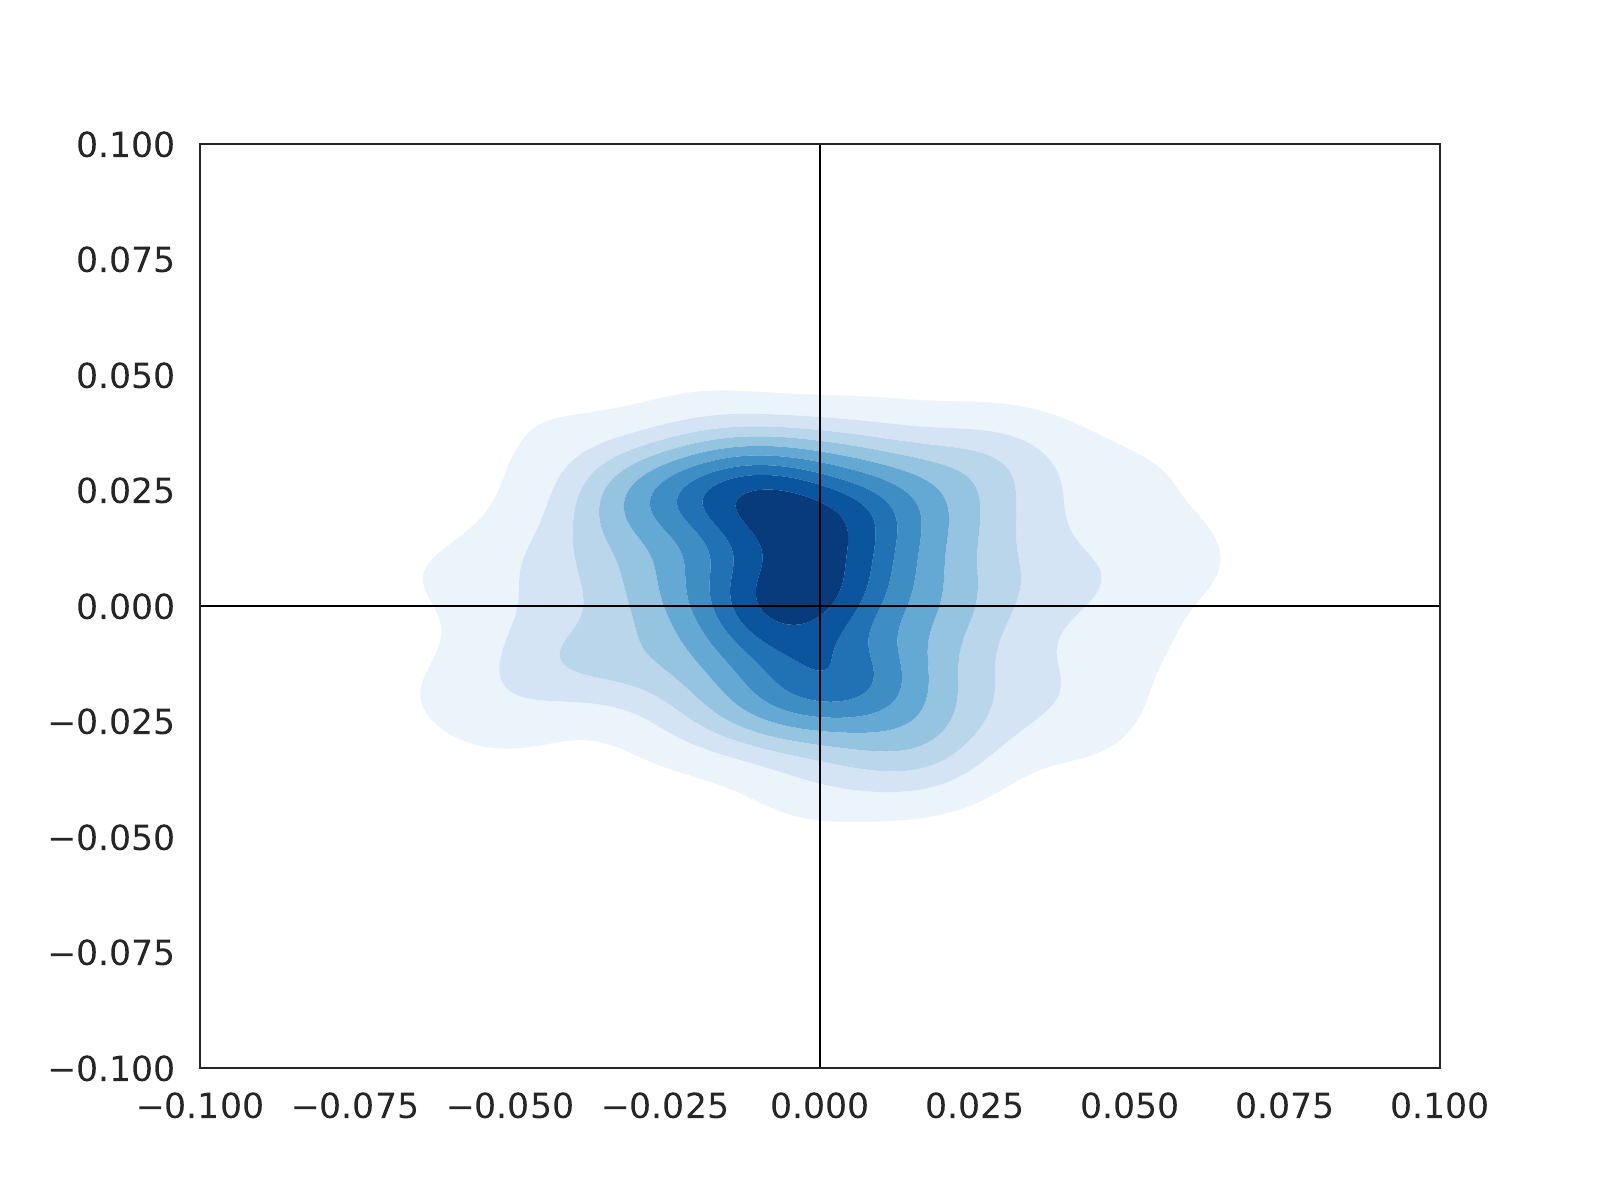} &
         \includegraphics[trim=60 80 60 80,clip,width=0.2\columnwidth]{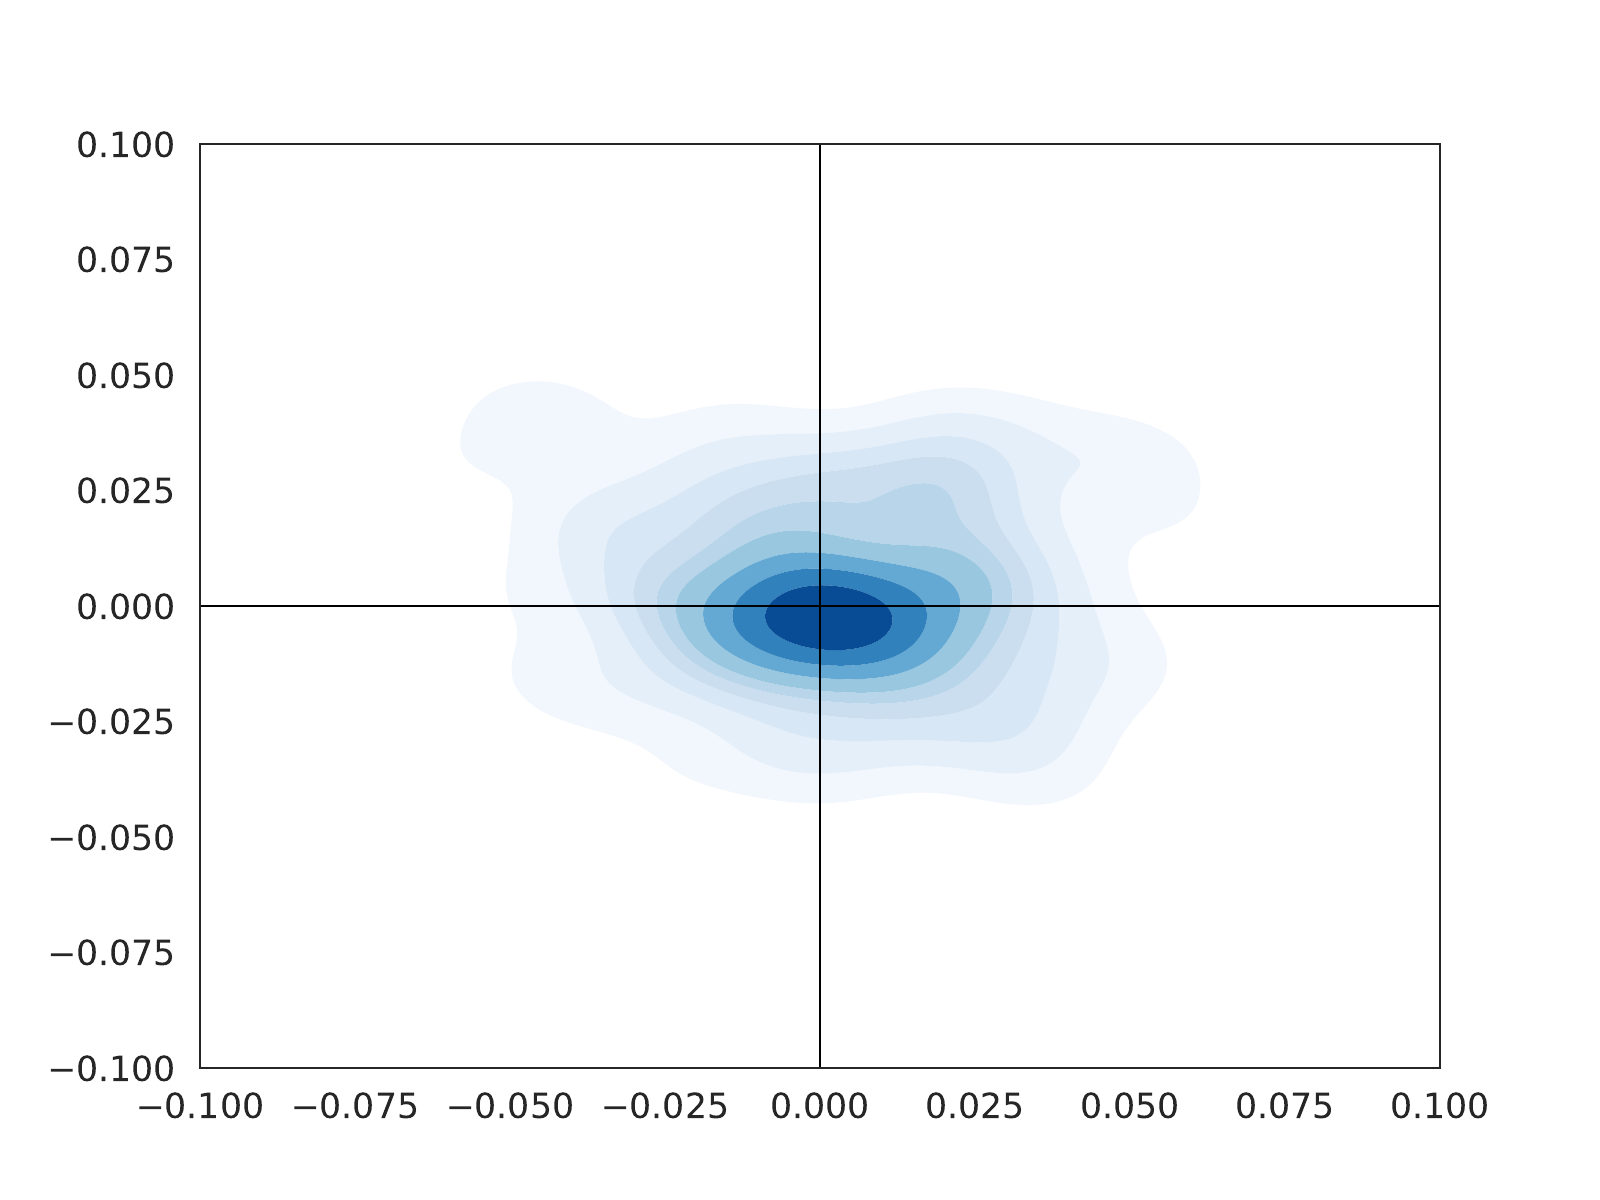} &
         \includegraphics[trim=60 80 60 80,clip,width=0.2\columnwidth]{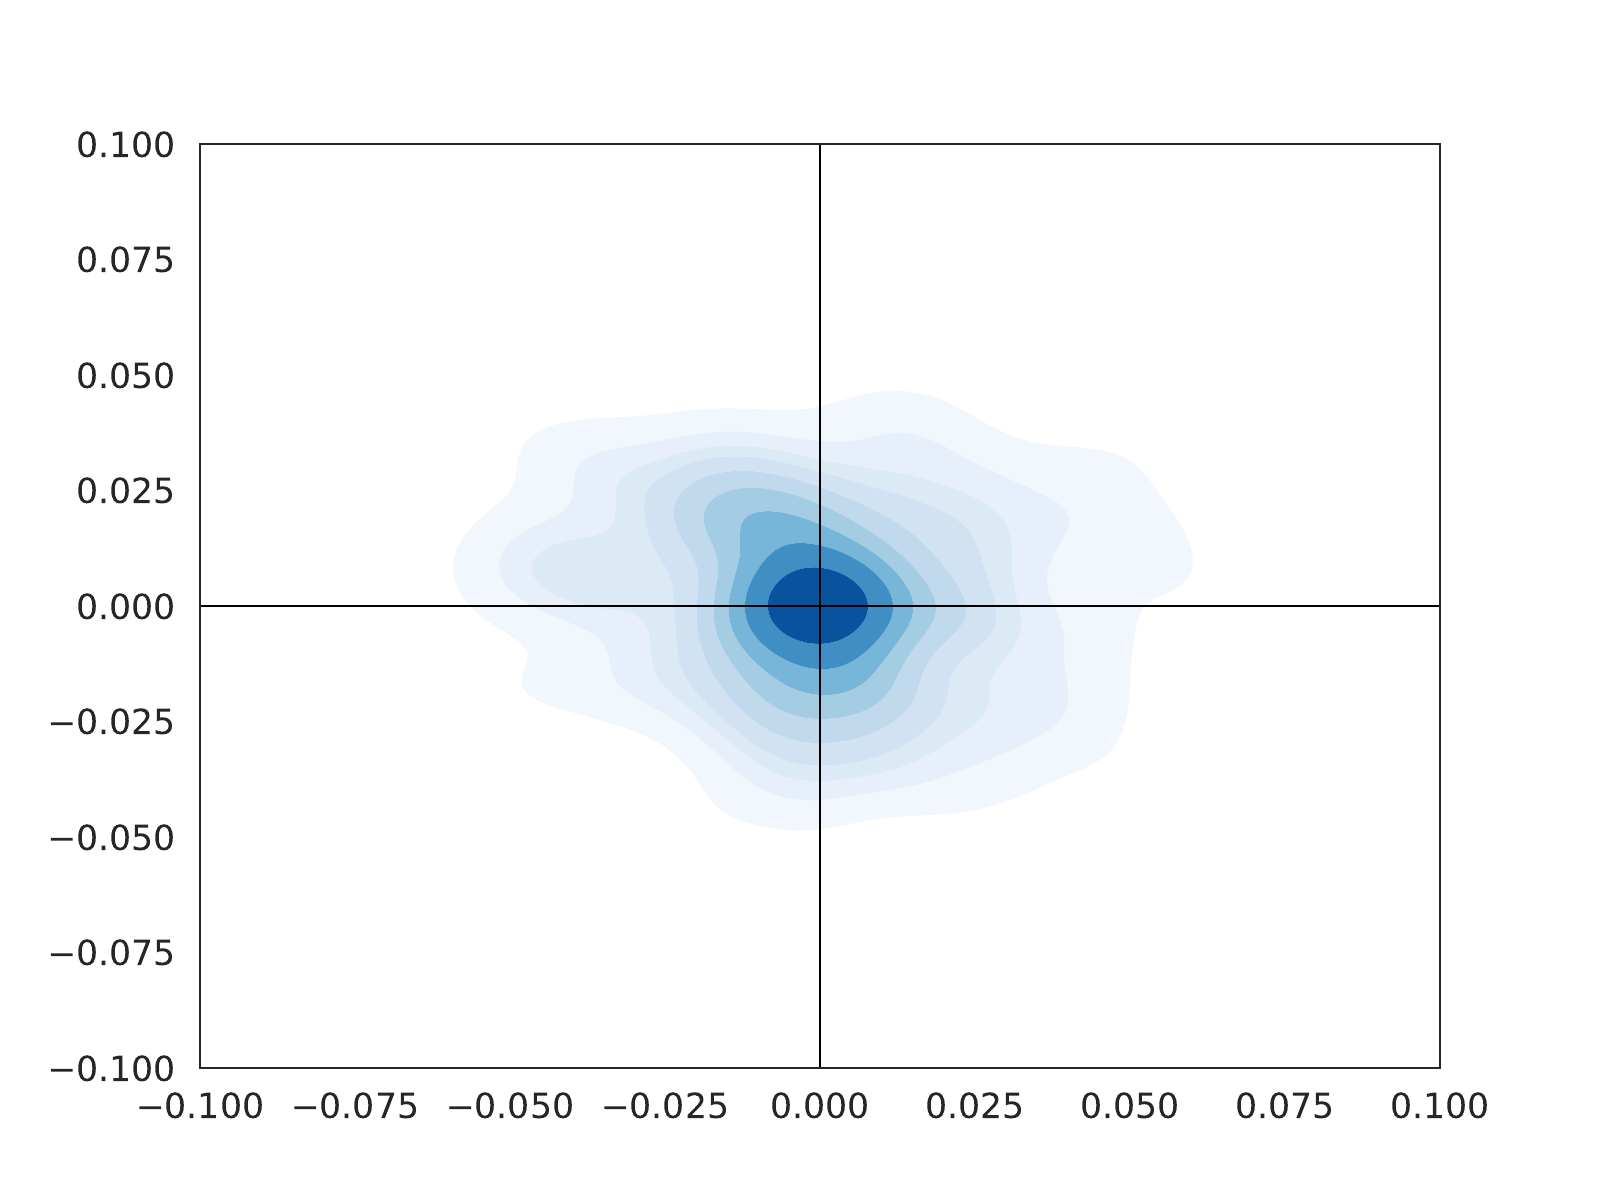} \\
         
         \rotatebox{90}{\hspace{1.8mm}SAVP\cite{lee2018savp}} &
         \includegraphics[trim=60 80 60 80,clip,width=0.2\columnwidth]{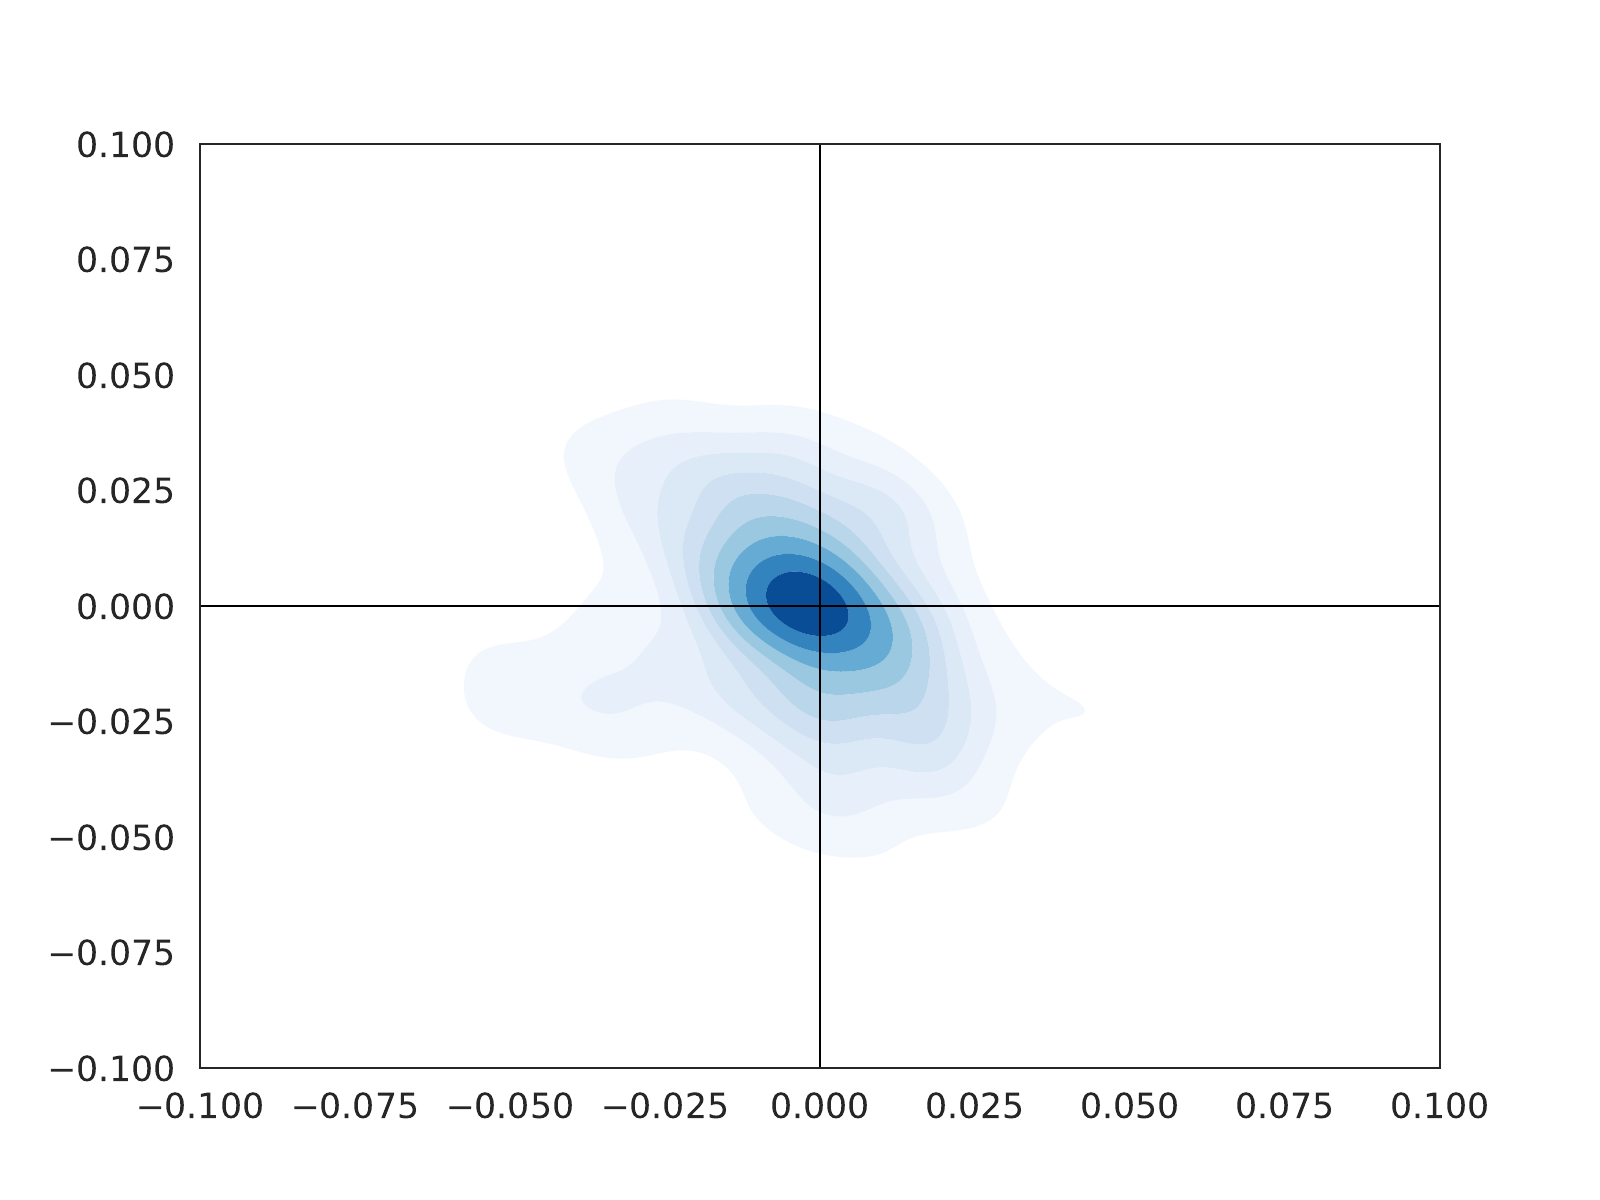} &
         \includegraphics[trim=60 80 60 80,clip,width=0.2\columnwidth]{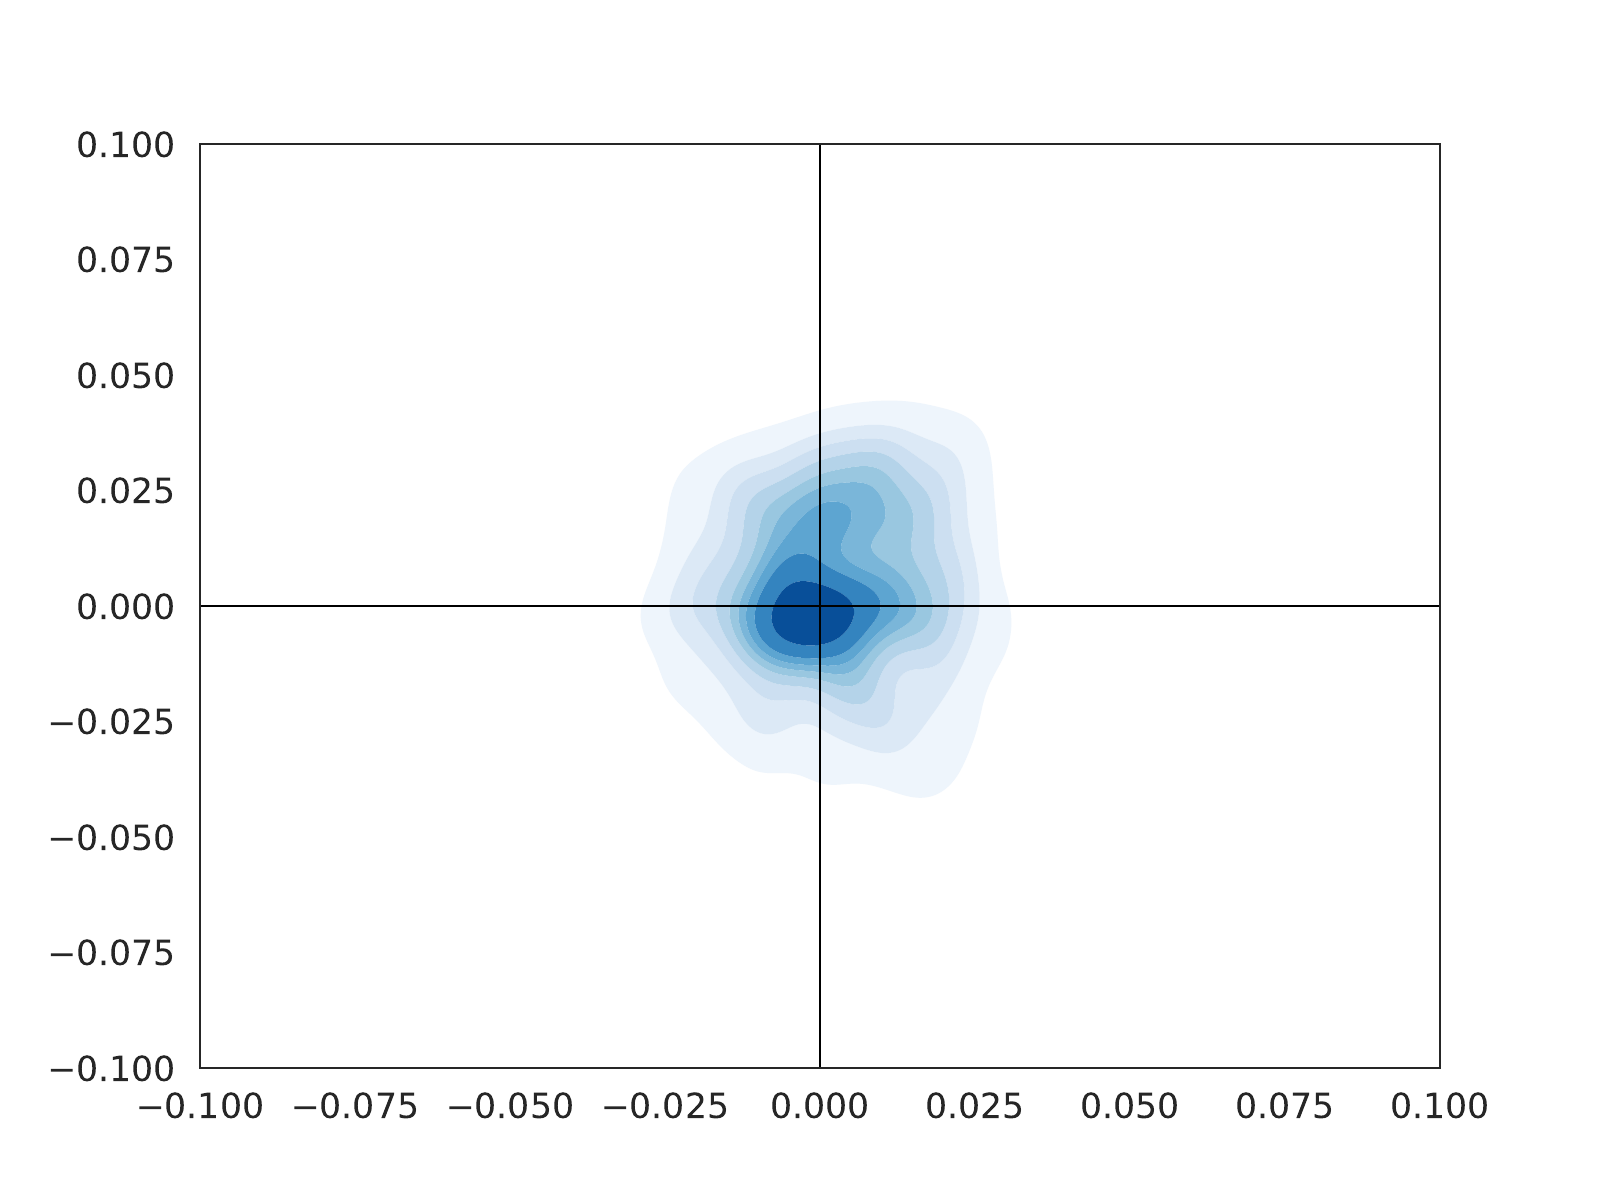} &
         \includegraphics[trim=60 80 60 80,clip,width=0.2\columnwidth]{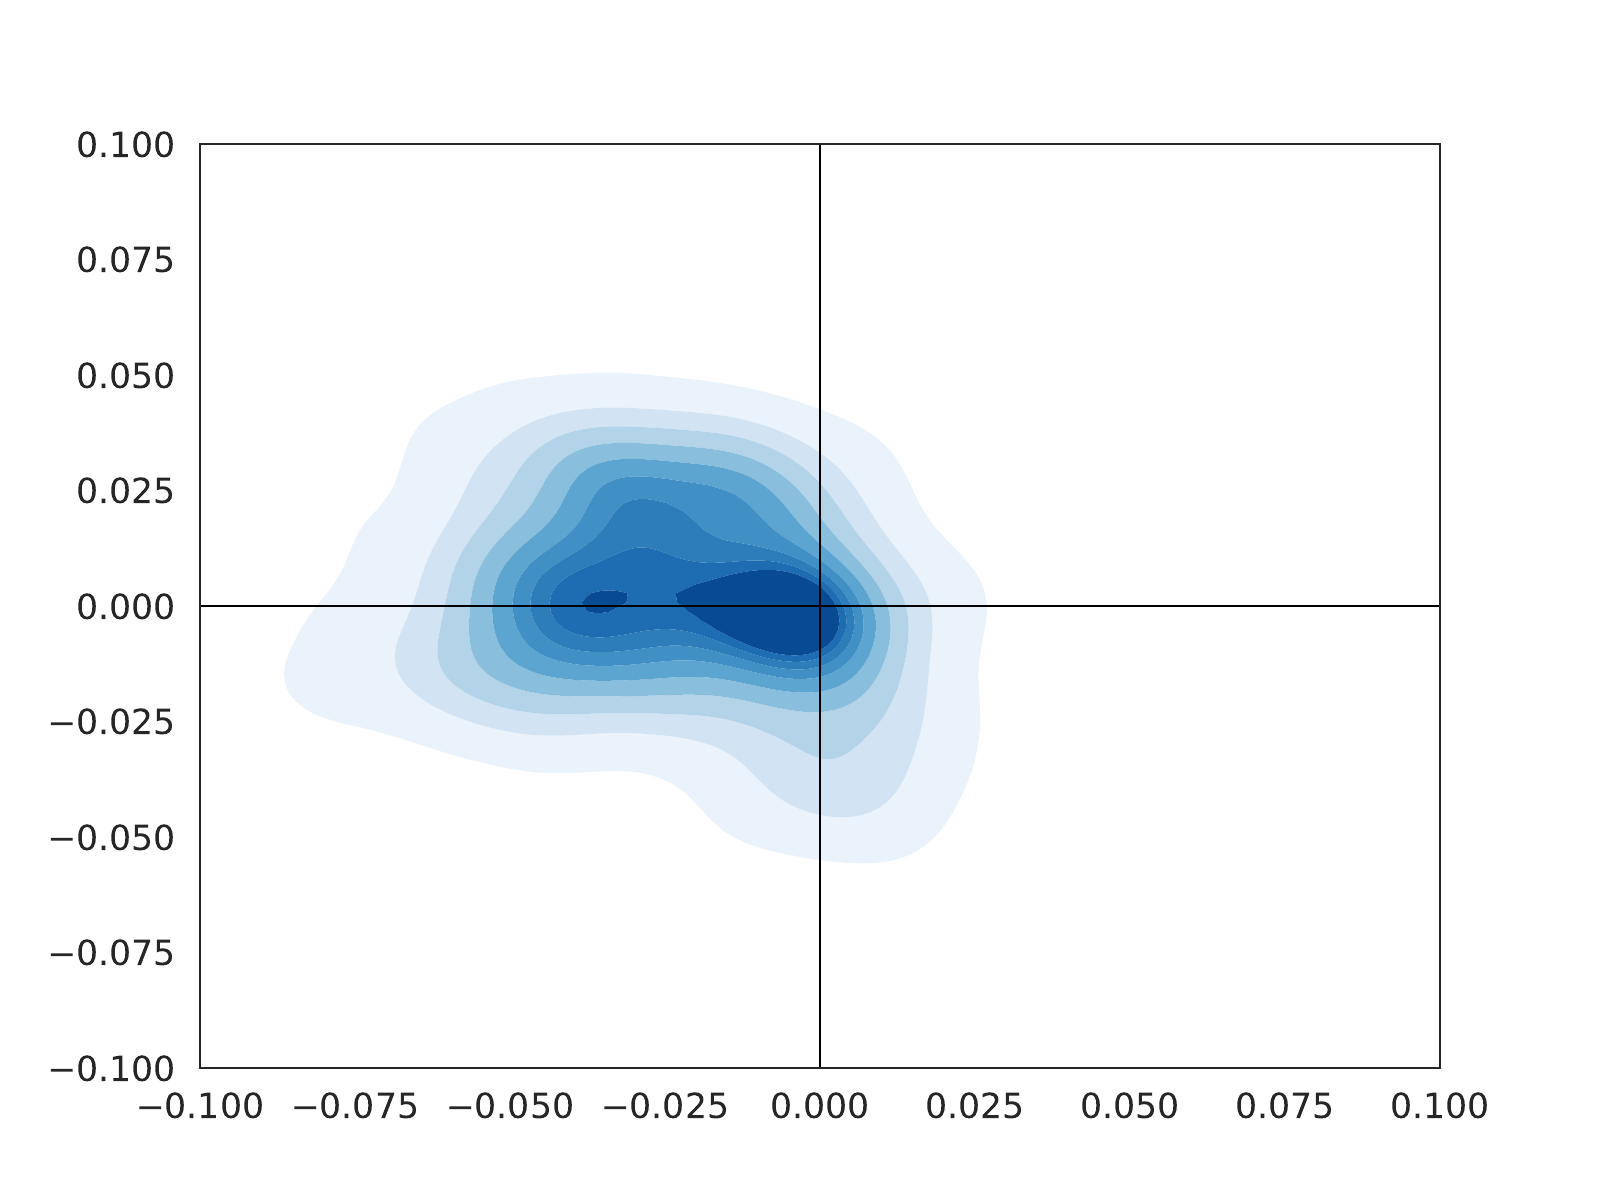} &
         \includegraphics[trim=60 80 60 80,clip,width=0.2\columnwidth]{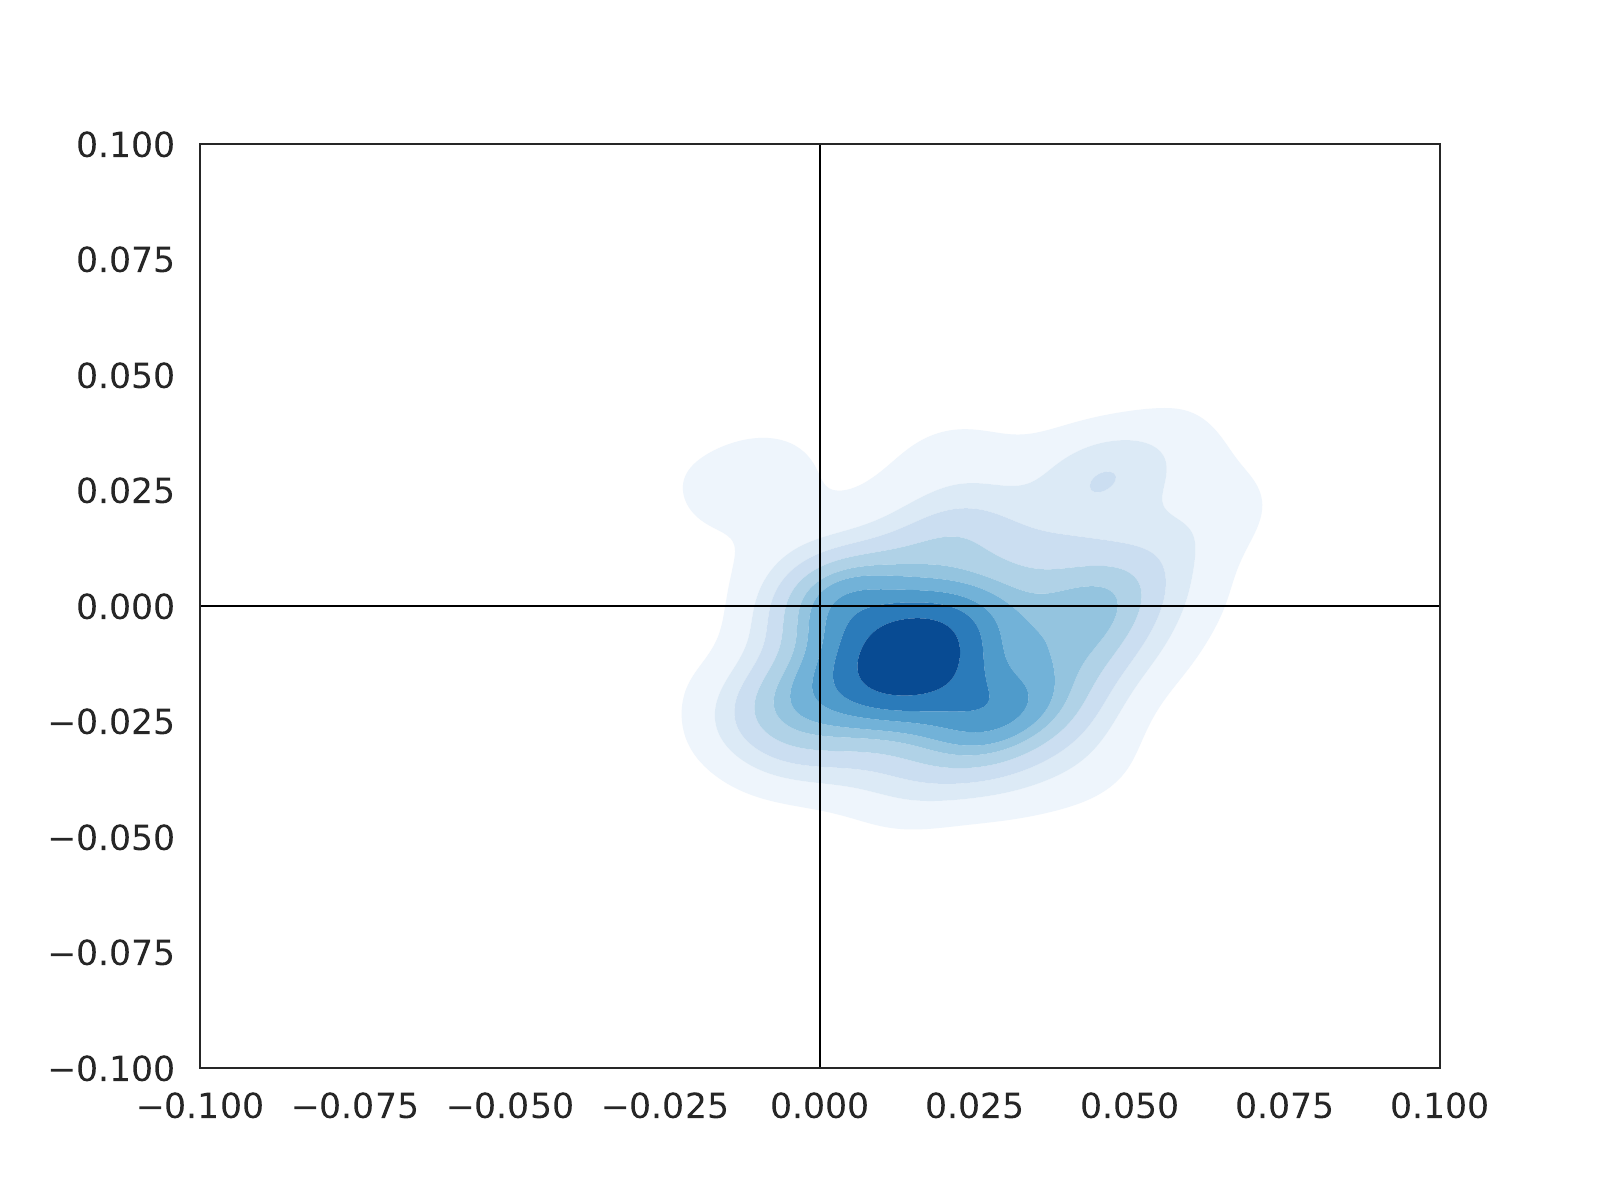} &
         \includegraphics[trim=60 80 60 80,clip,width=0.2\columnwidth]{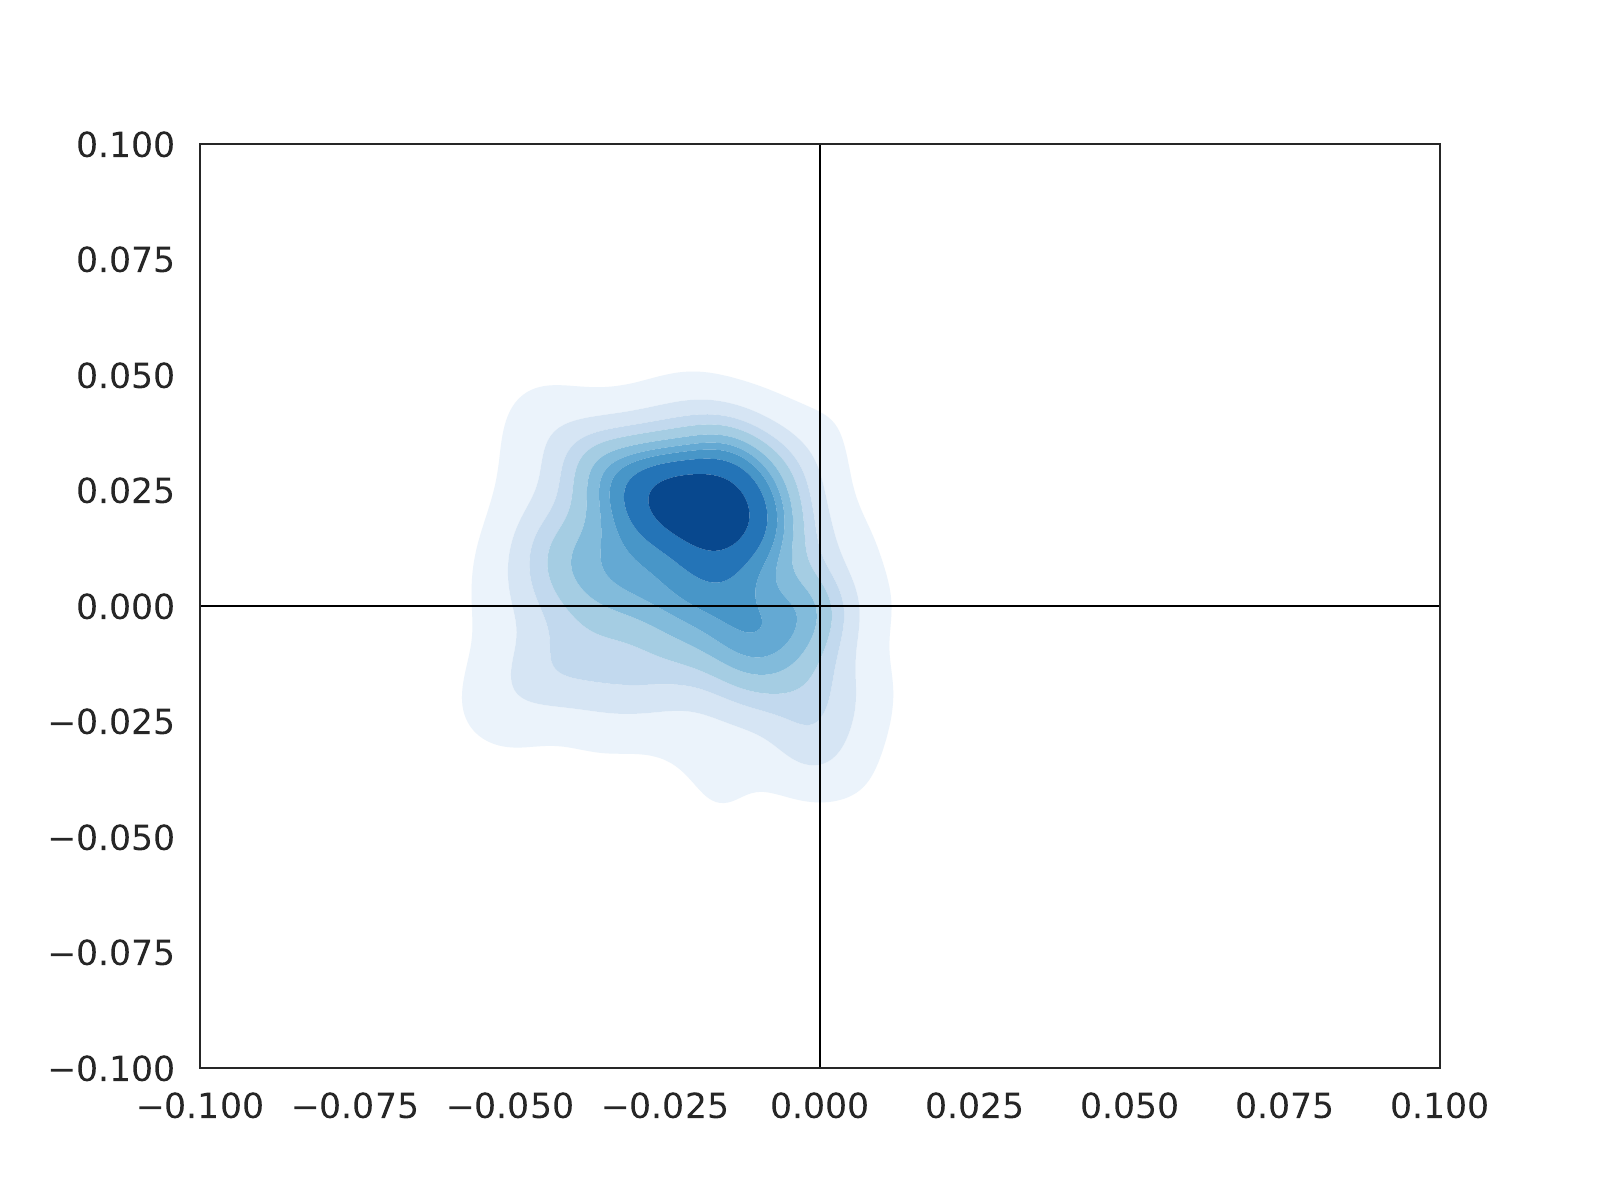} &
         \includegraphics[trim=60 80 60 80,clip,width=0.2\columnwidth]{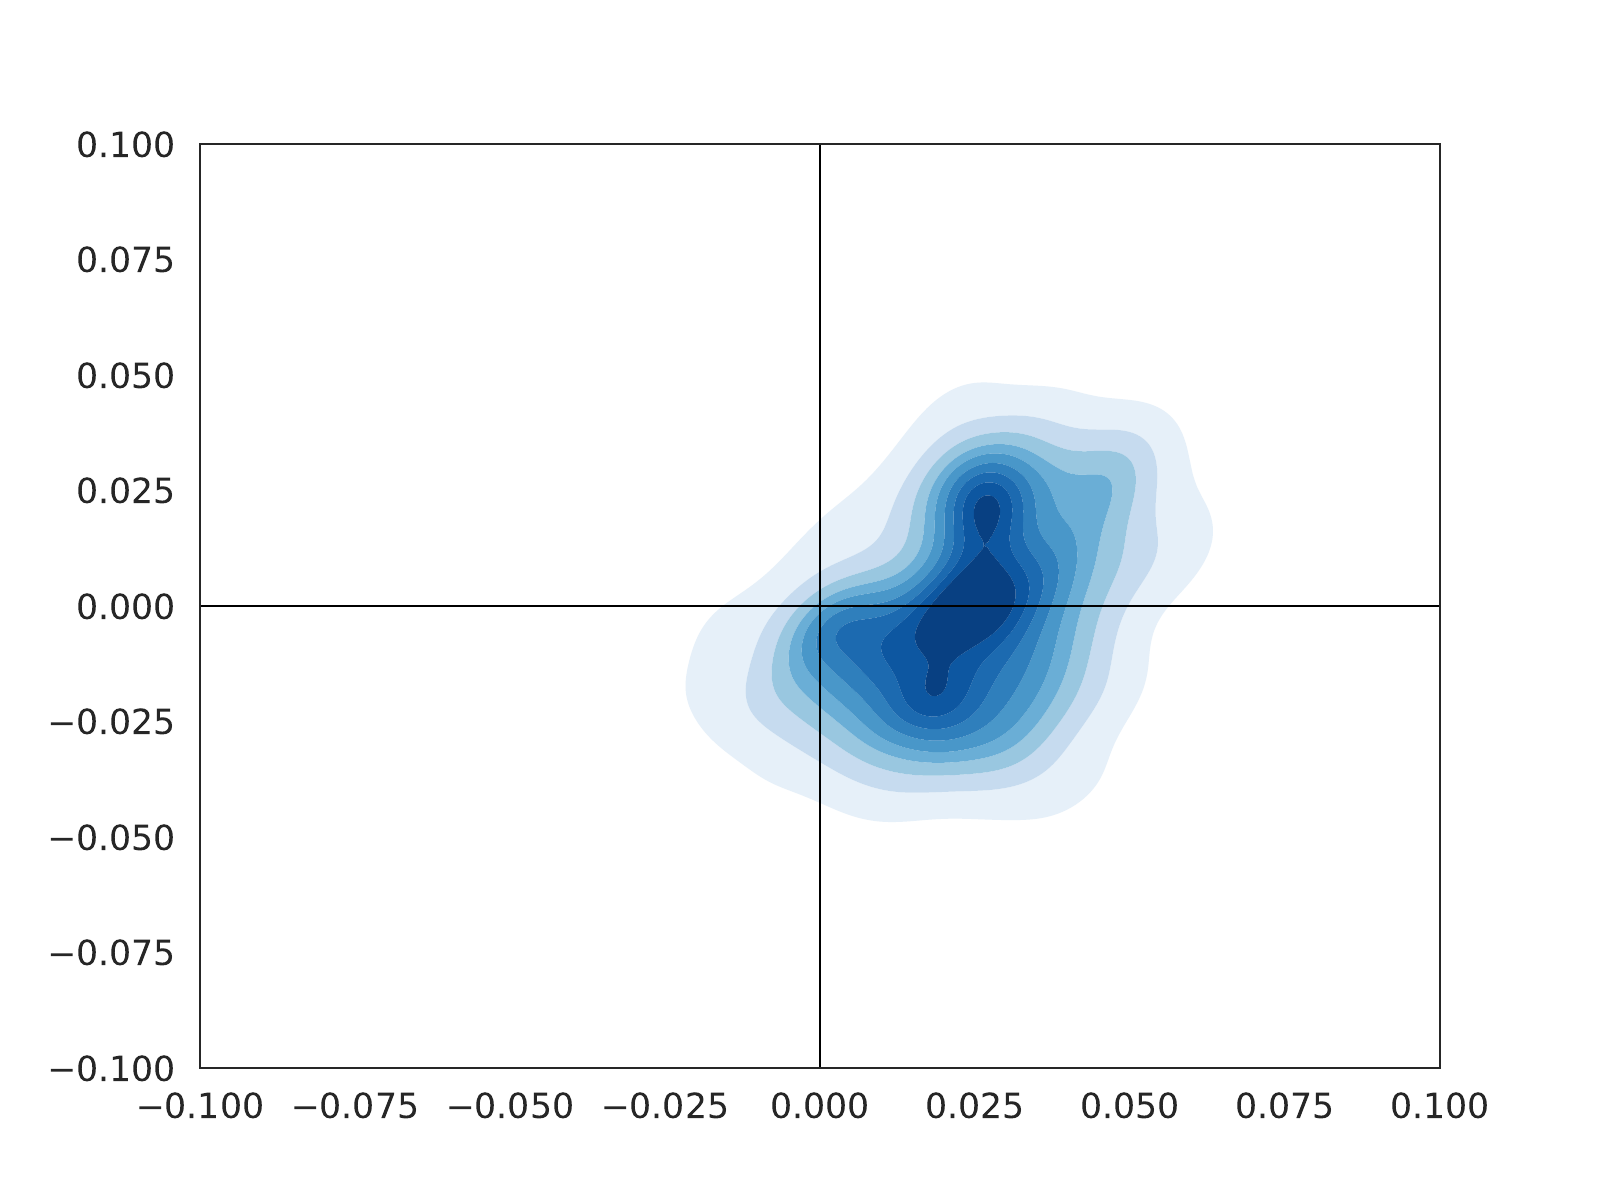} &
         \includegraphics[trim=60 80 60 80,clip,width=0.2\columnwidth]{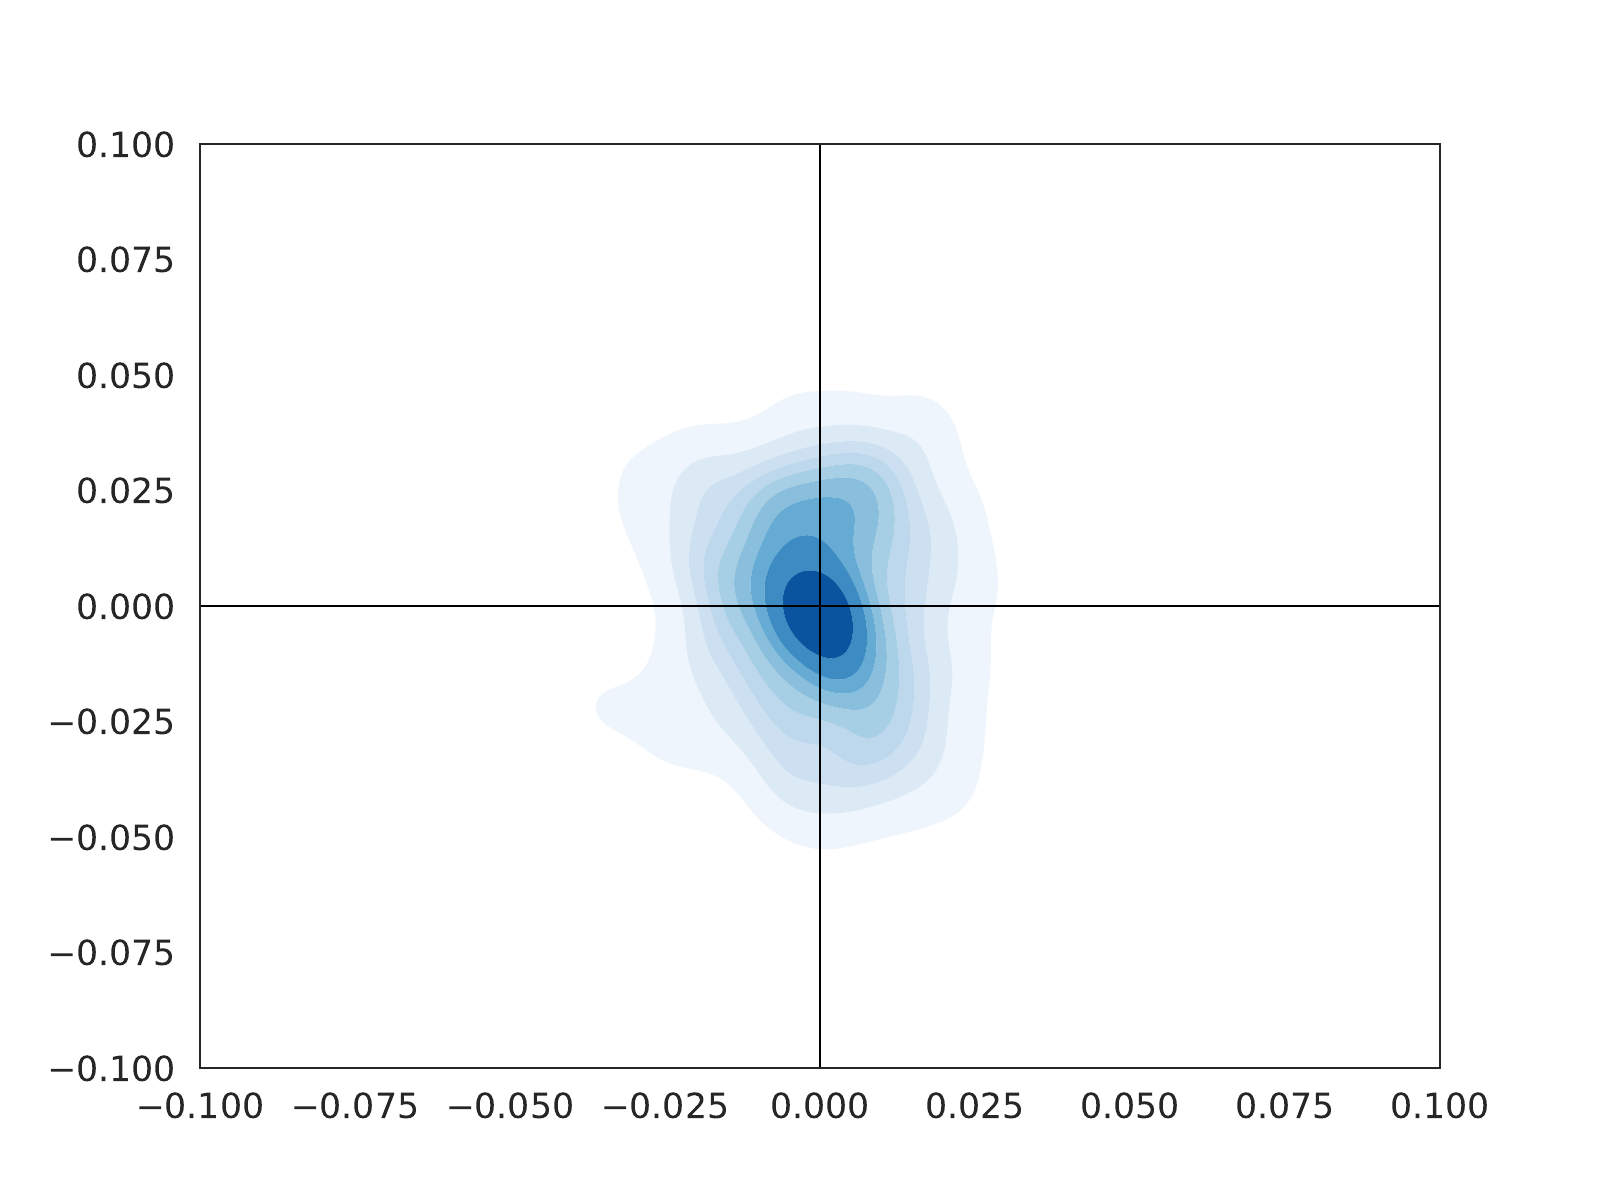} \\
         
         \rotatebox{90}{\hspace{2.5mm}SAVP+} &
         \includegraphics[trim=60 80 60 80,clip,width=0.2\columnwidth]{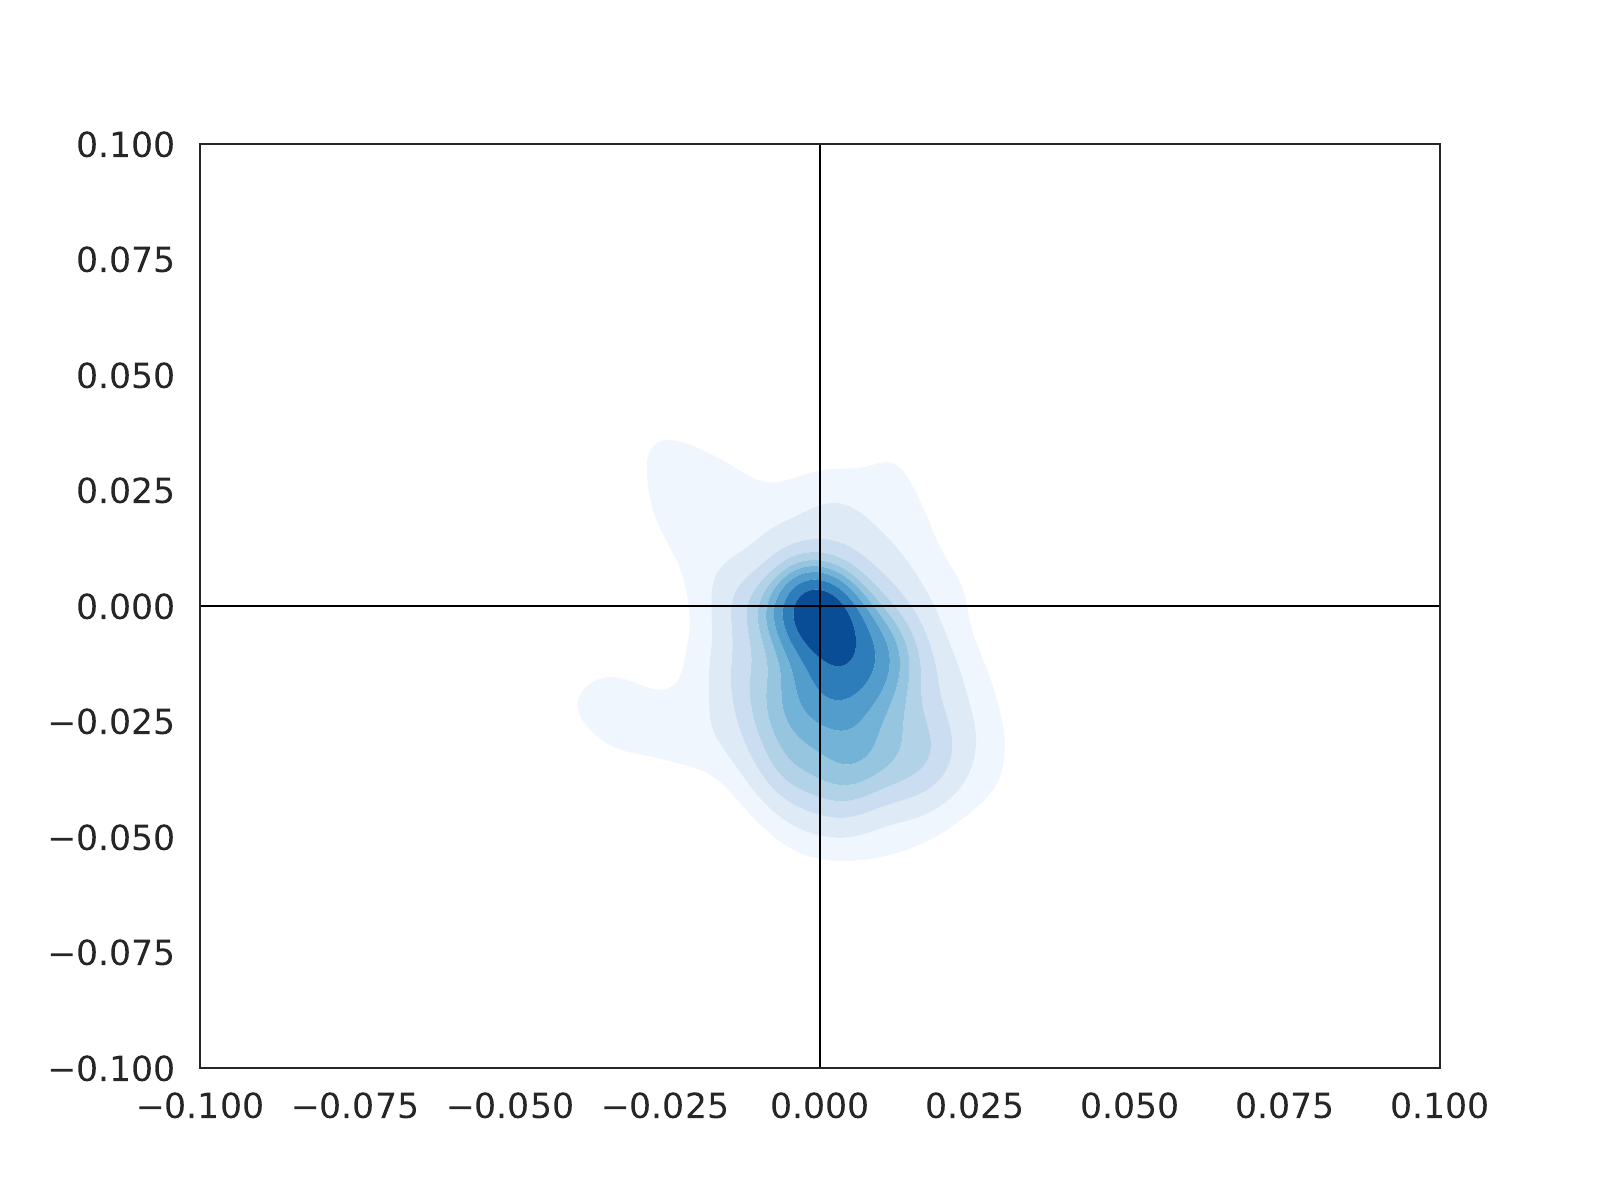} &
         \includegraphics[trim=60 80 60 80,clip,width=0.2\columnwidth]{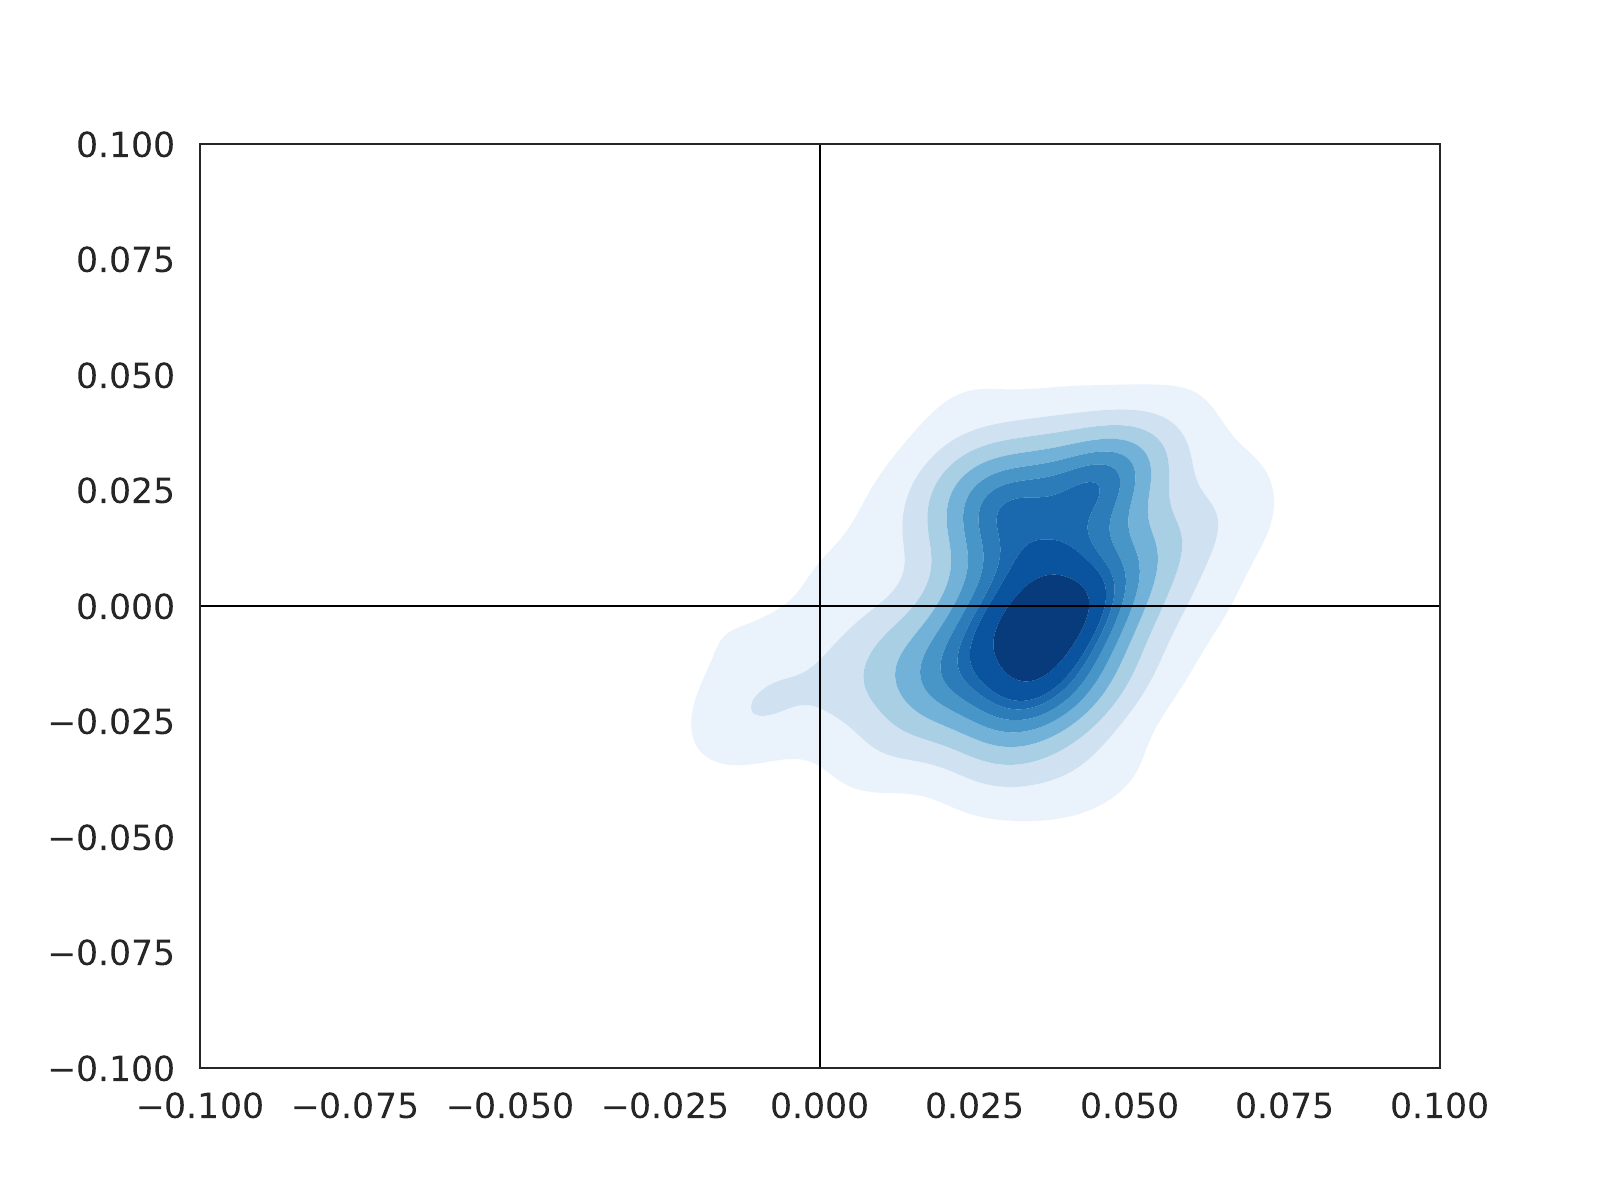} &
         \includegraphics[trim=60 80 60 80,clip,width=0.2\columnwidth]{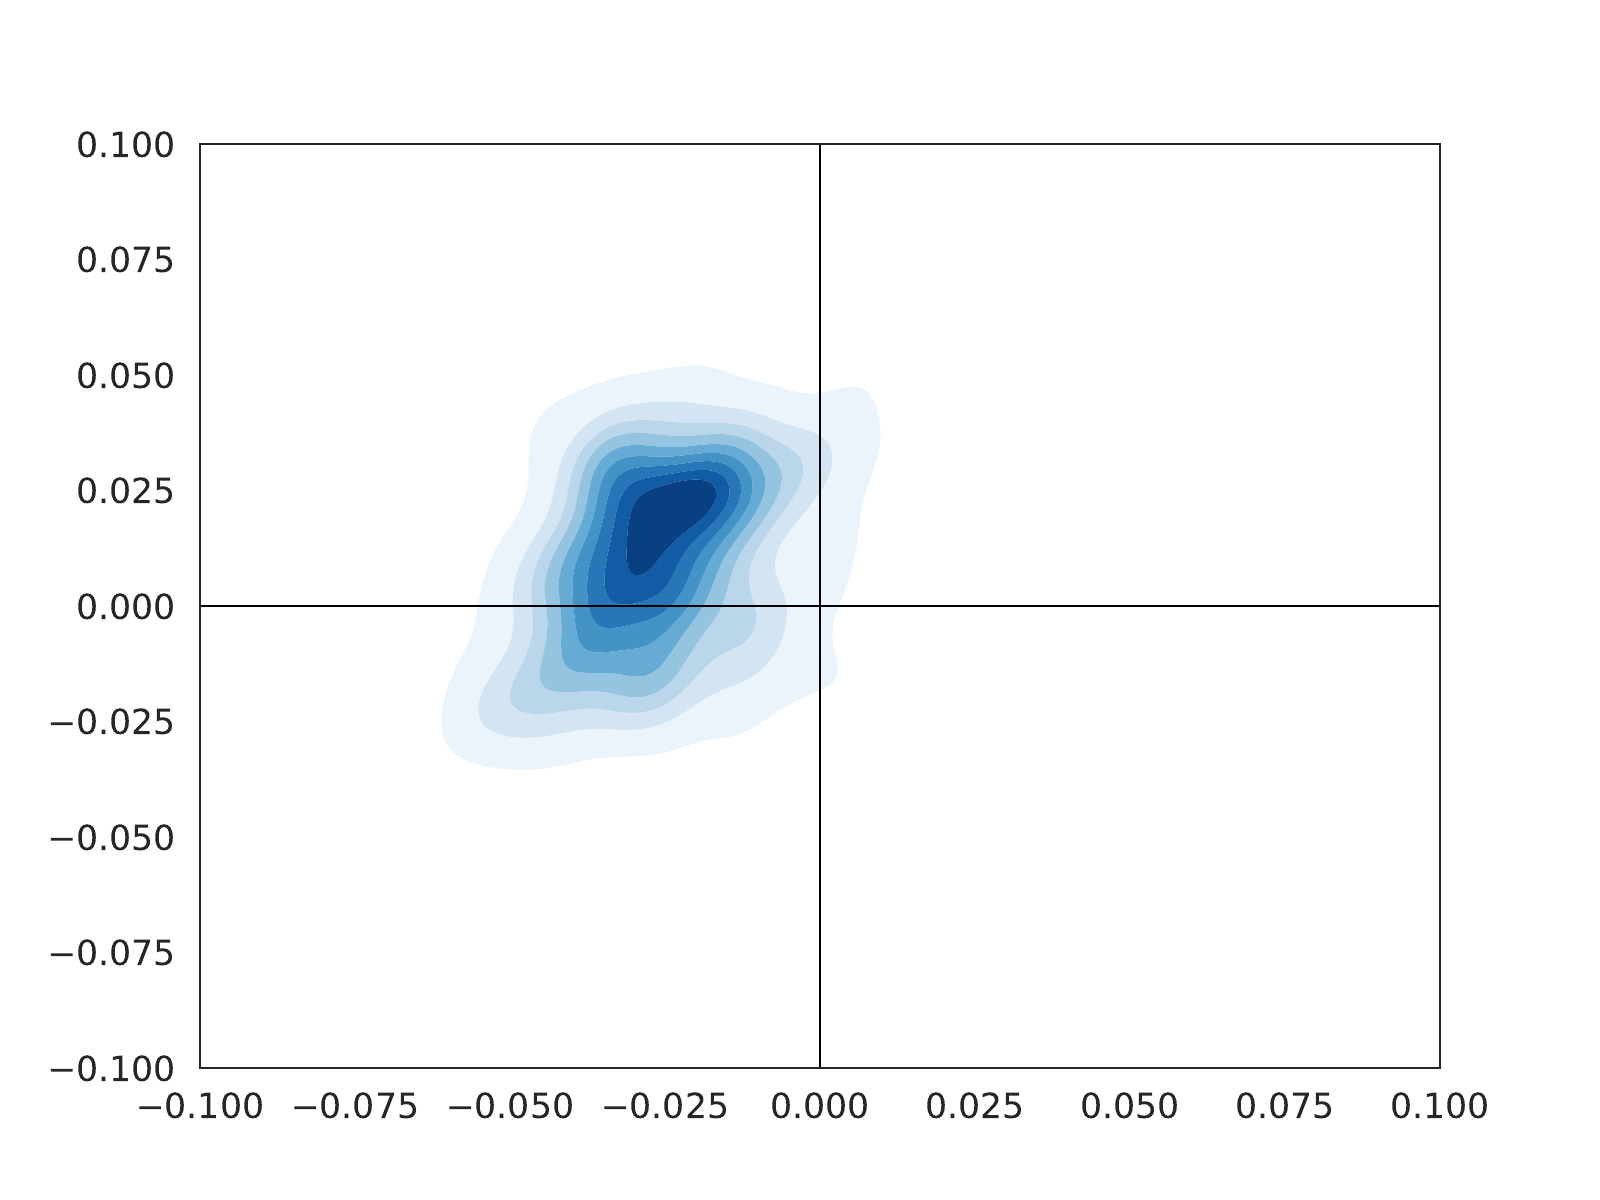} &
         \includegraphics[trim=60 80 60 80,clip,width=0.2\columnwidth]{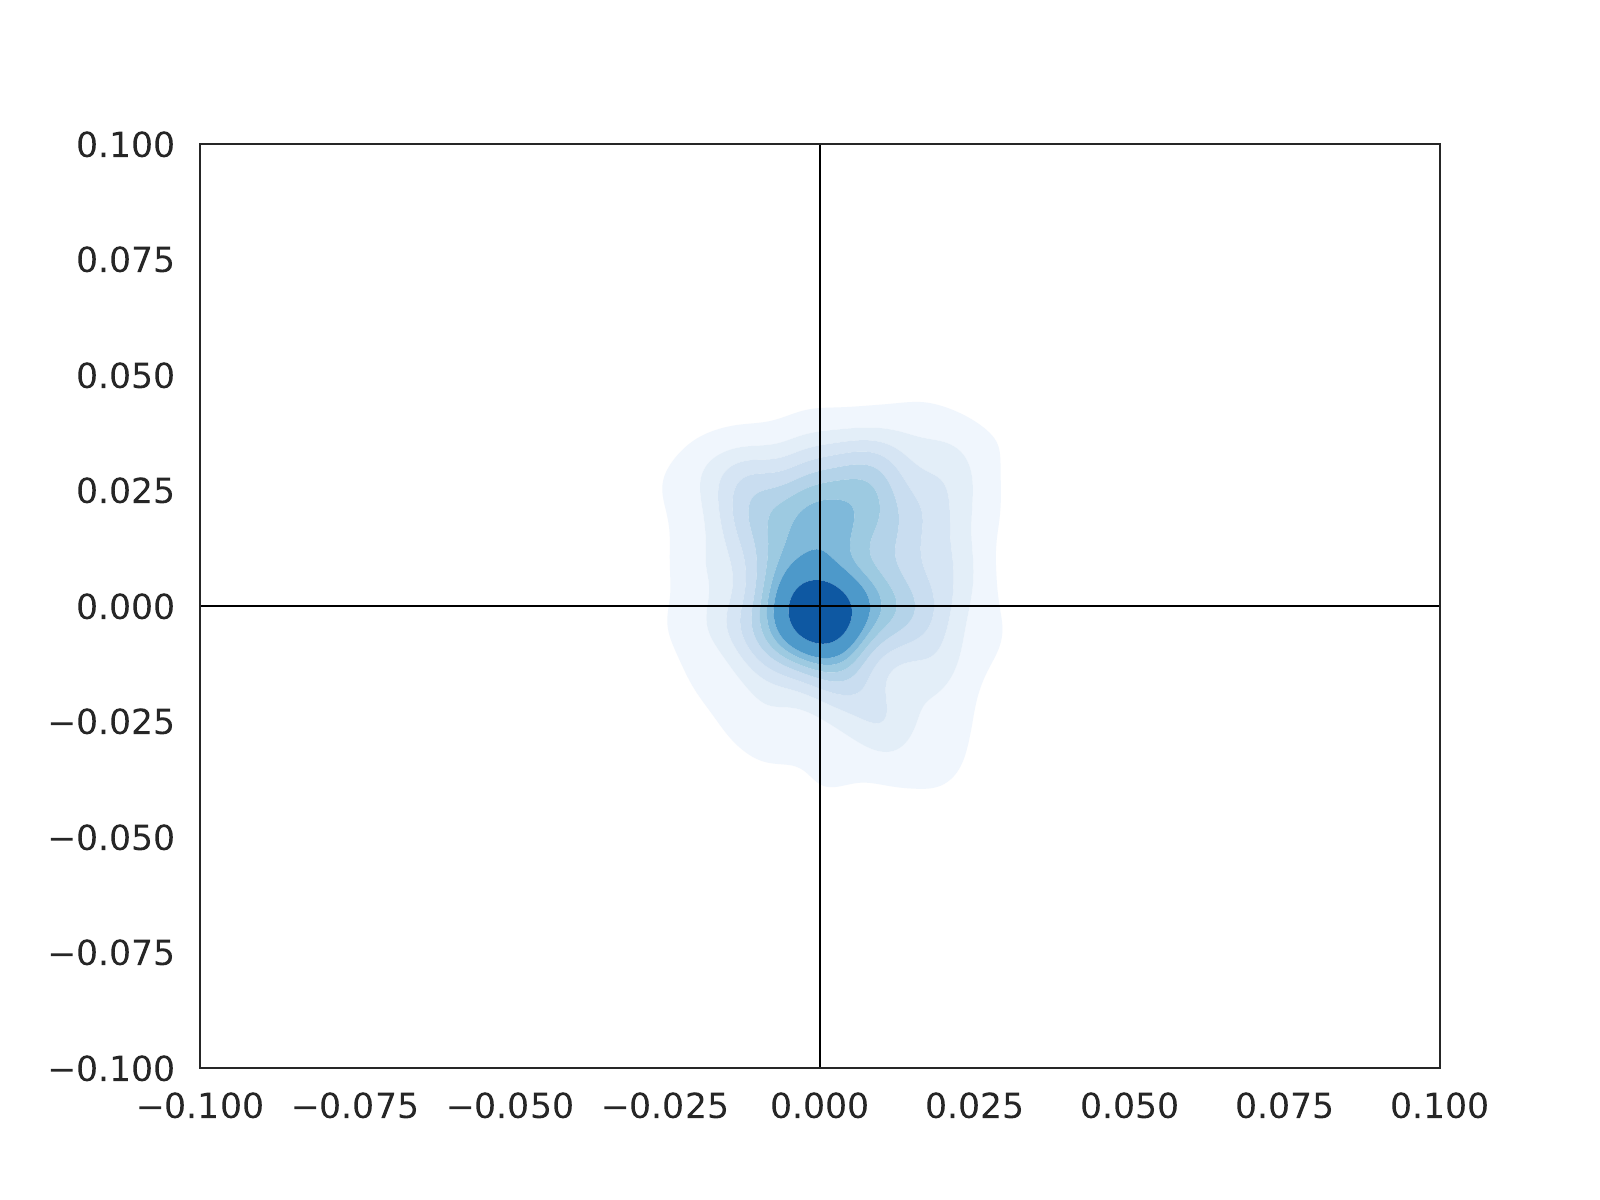} &
         \includegraphics[trim=60 80 60 80,clip,width=0.2\columnwidth]{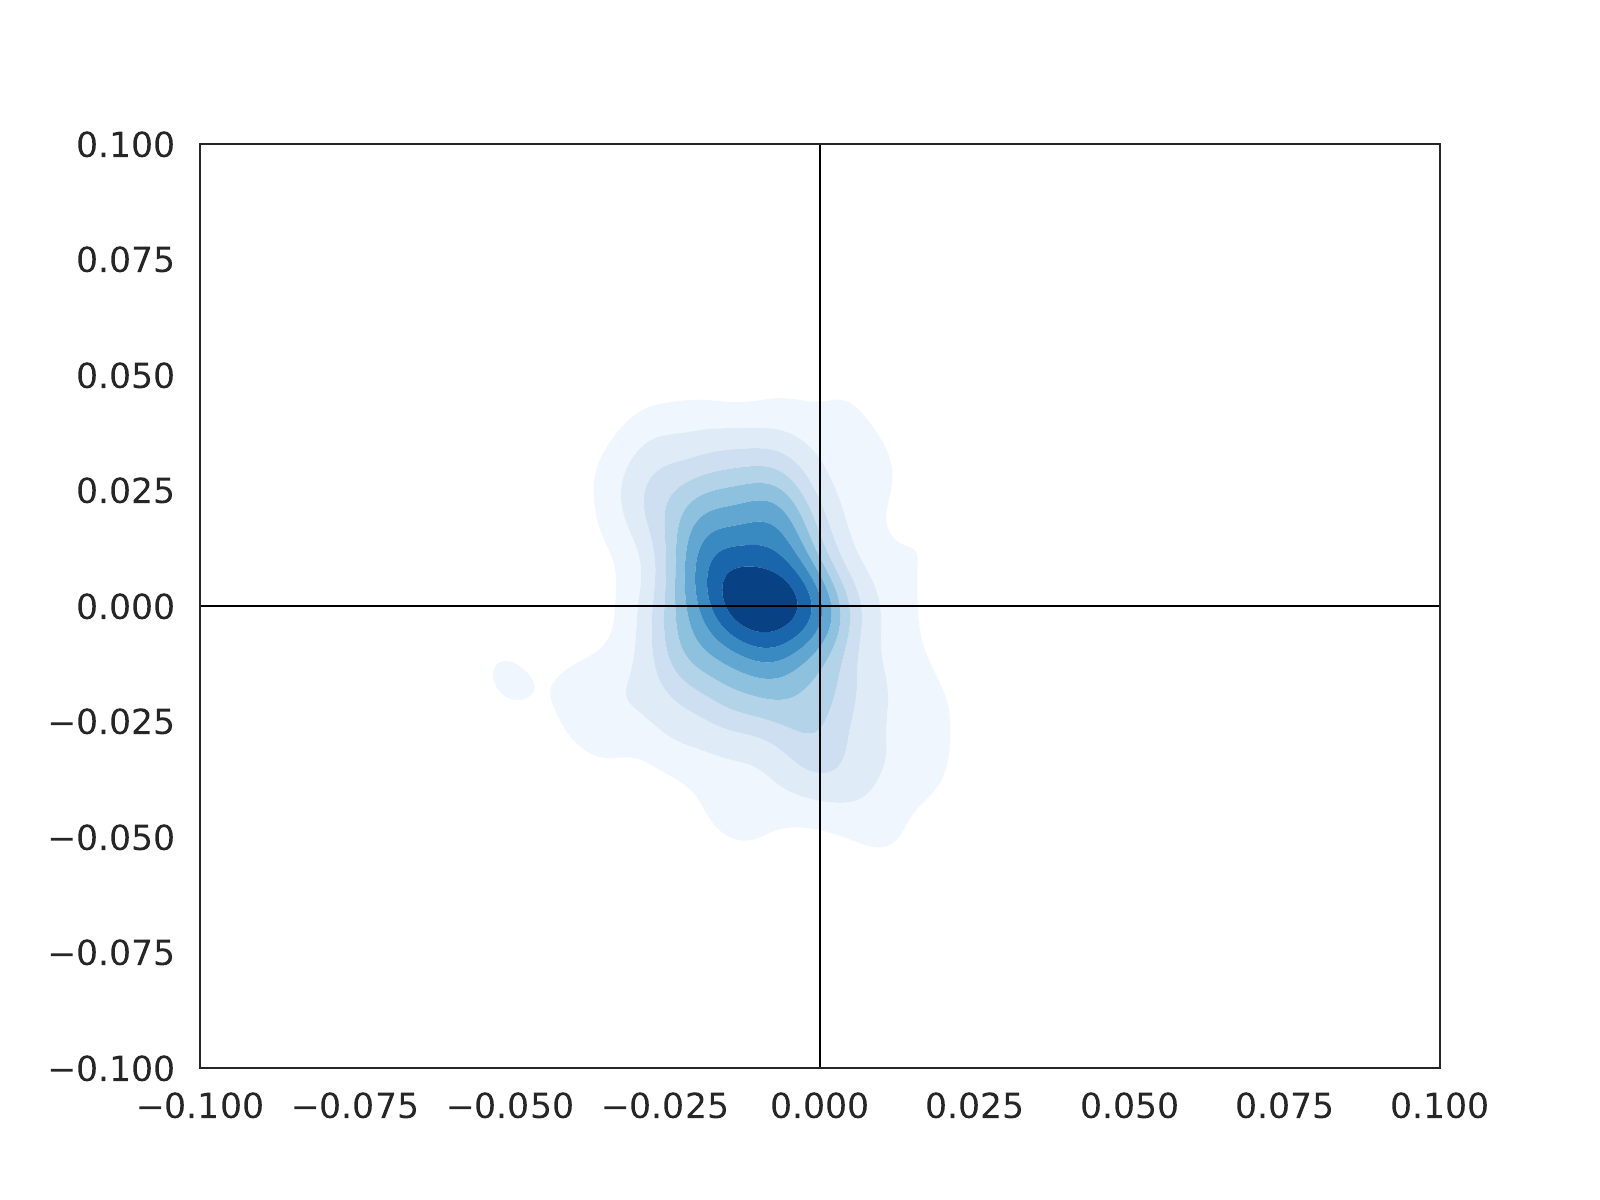} &
         \includegraphics[trim=60 80 60 80,clip,width=0.2\columnwidth]{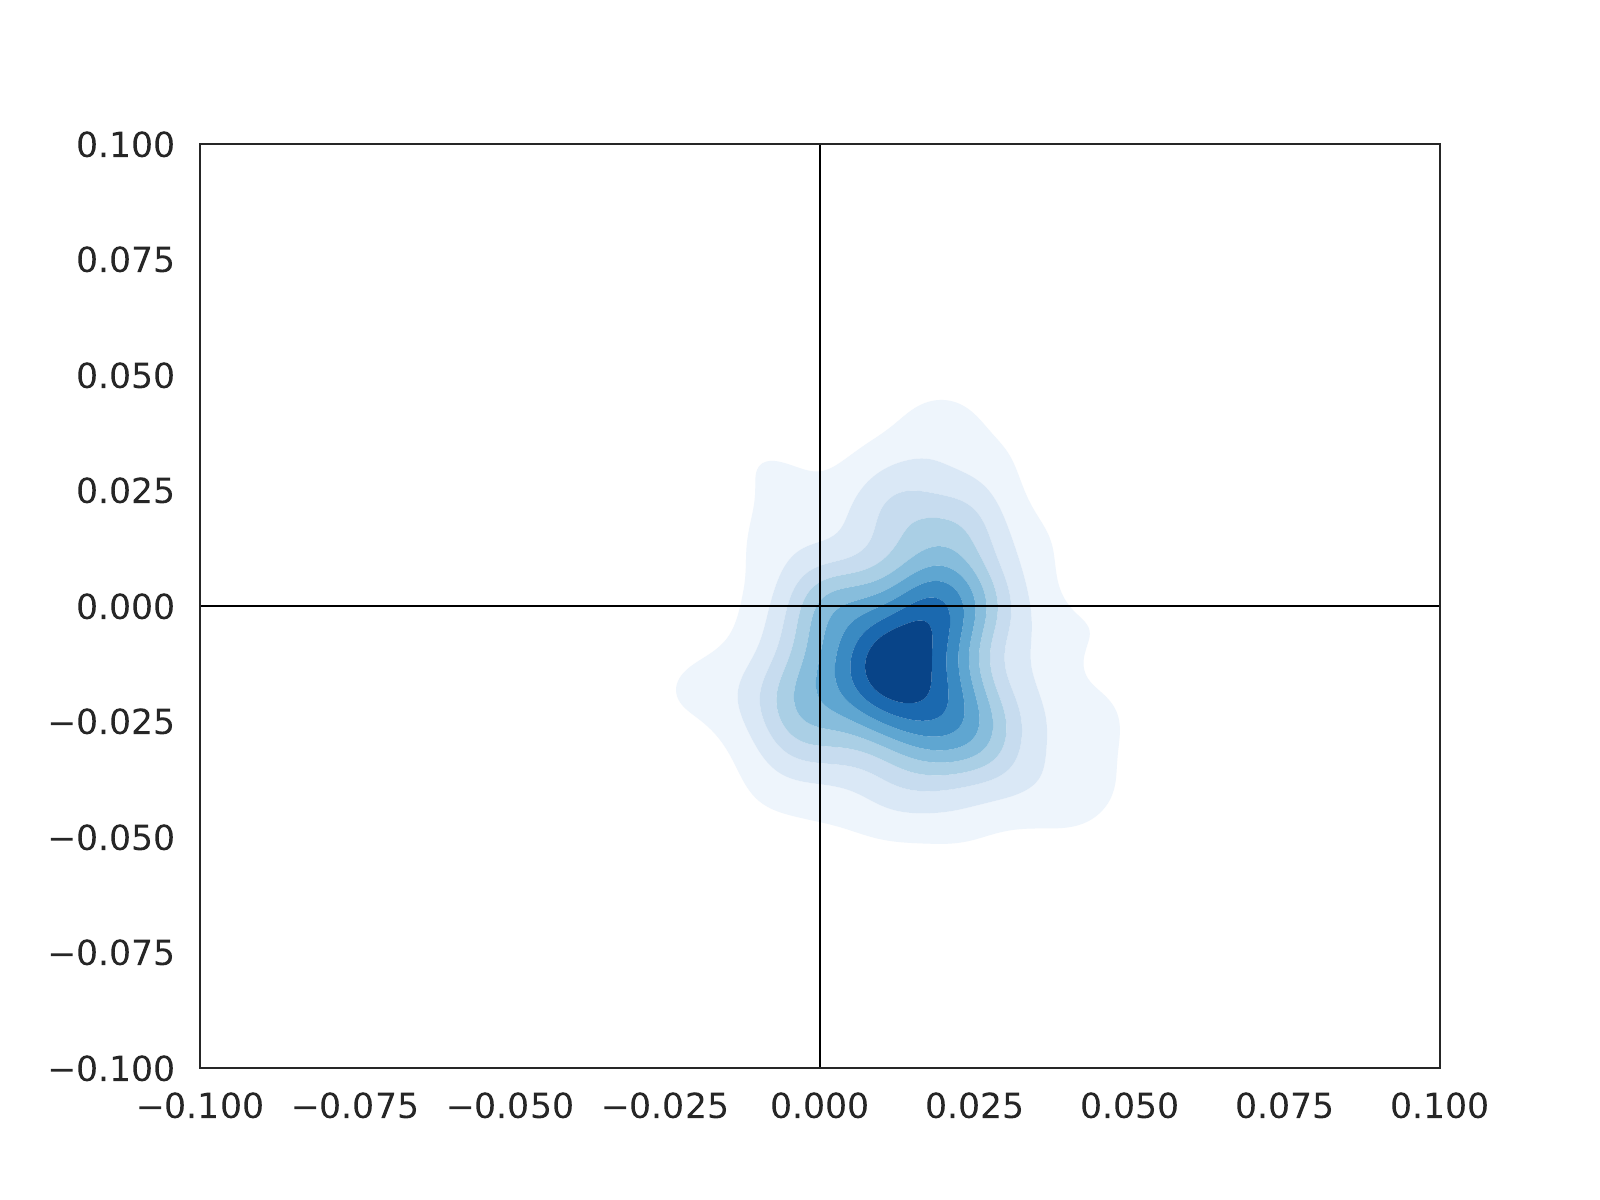} &
         \includegraphics[trim=60 80 60 80,clip,width=0.2\columnwidth]{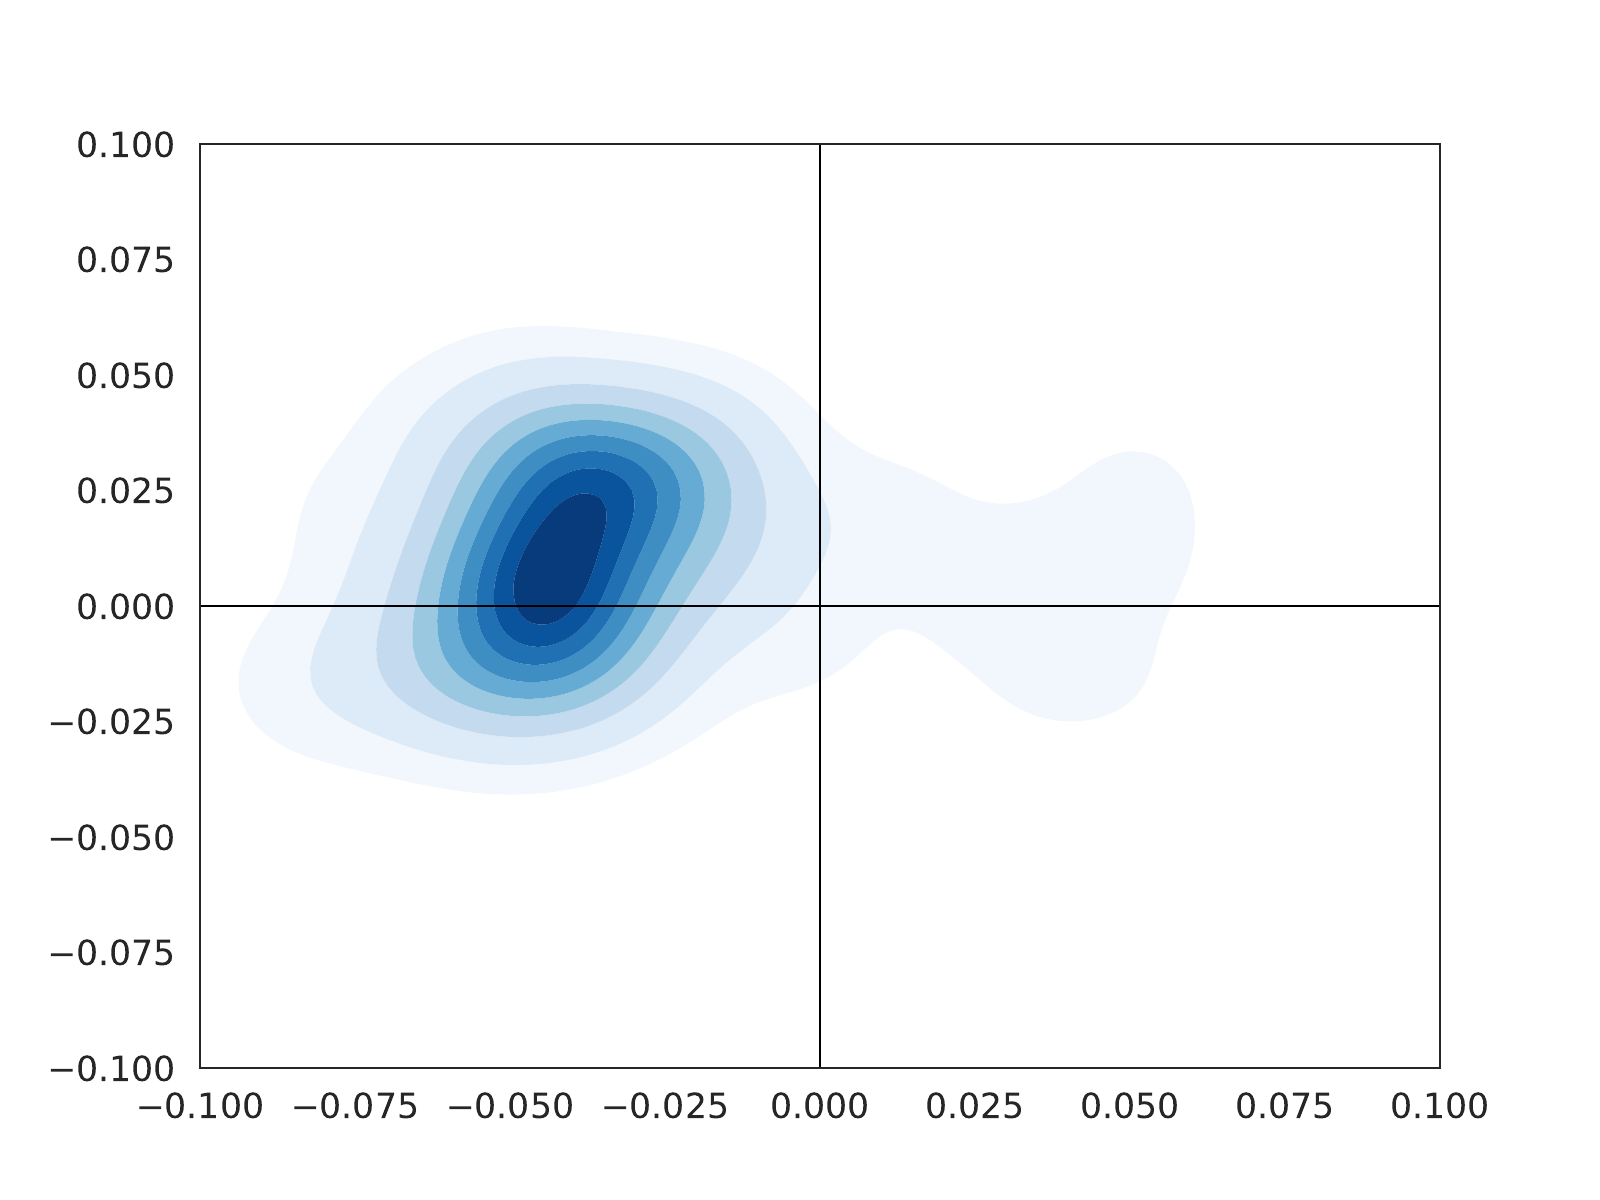} \\
         
         \rotatebox{90}{\hspace{3mm}Ours} &
         \includegraphics[trim=60 80 60 80,clip,width=0.2\columnwidth]{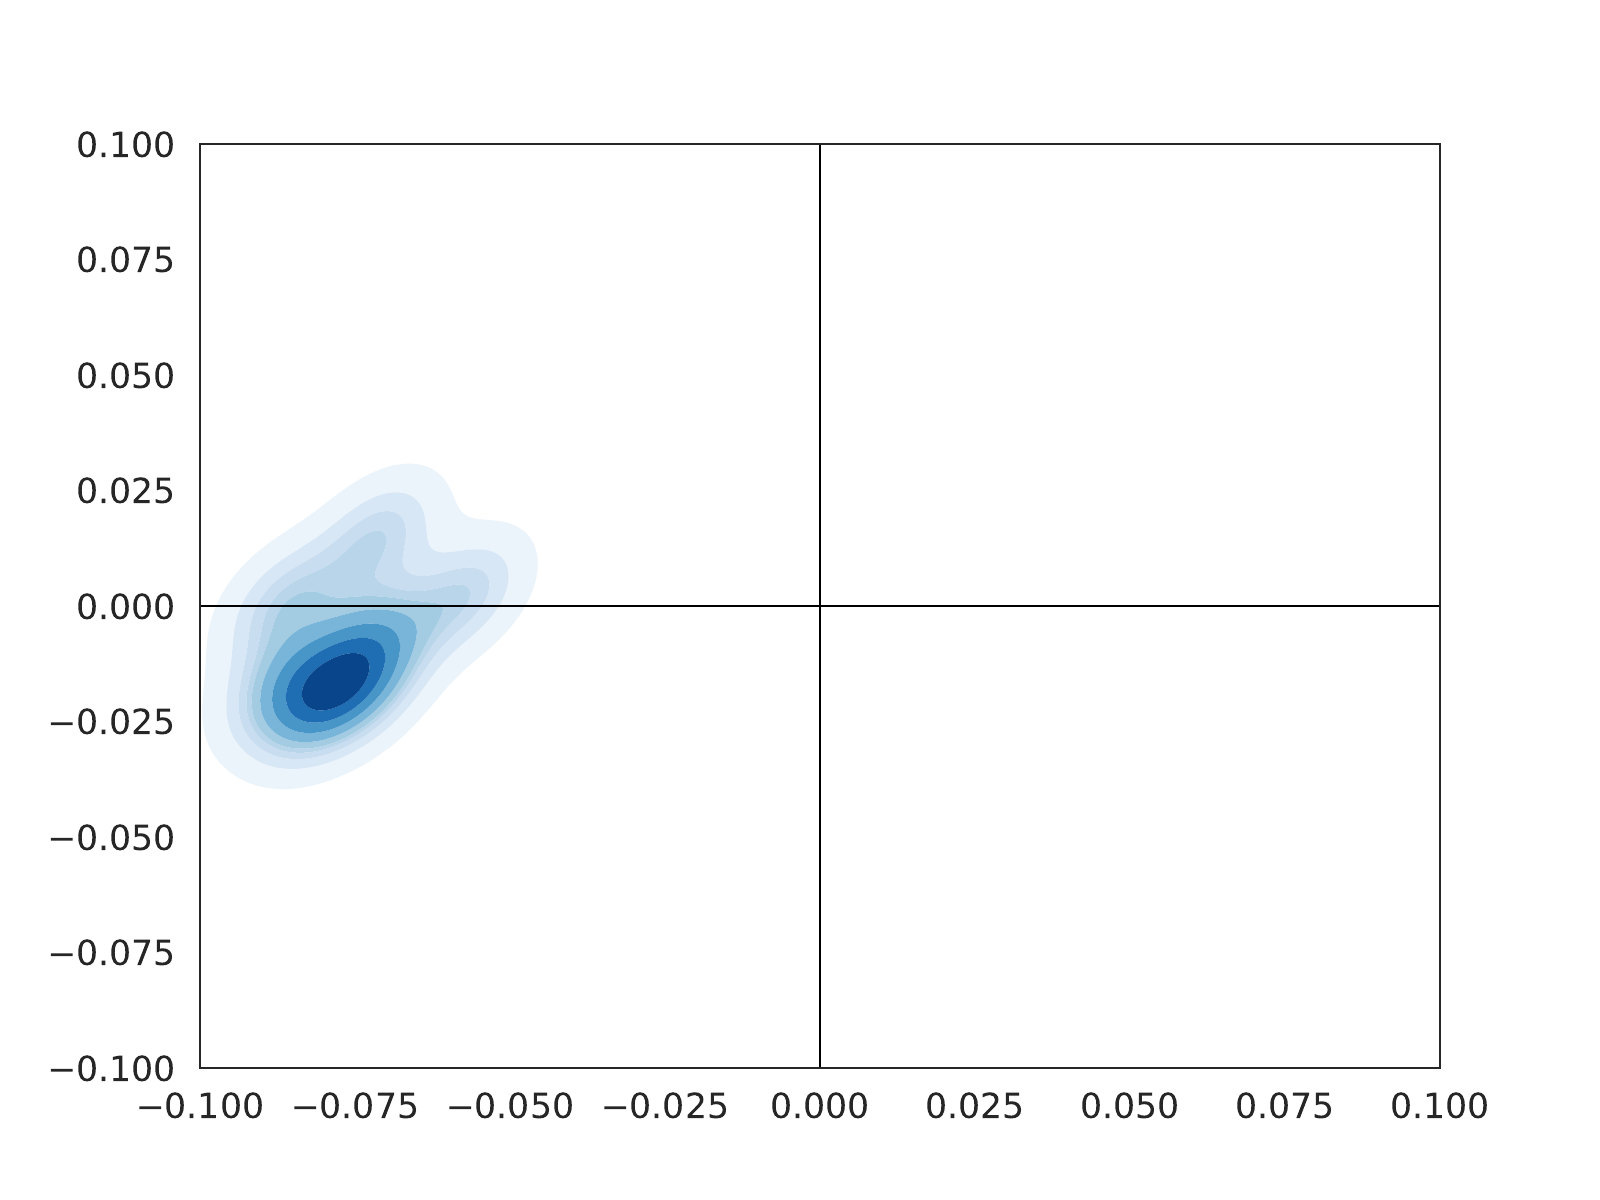} &
         \includegraphics[trim=60 80 60 80,clip,width=0.2\columnwidth]{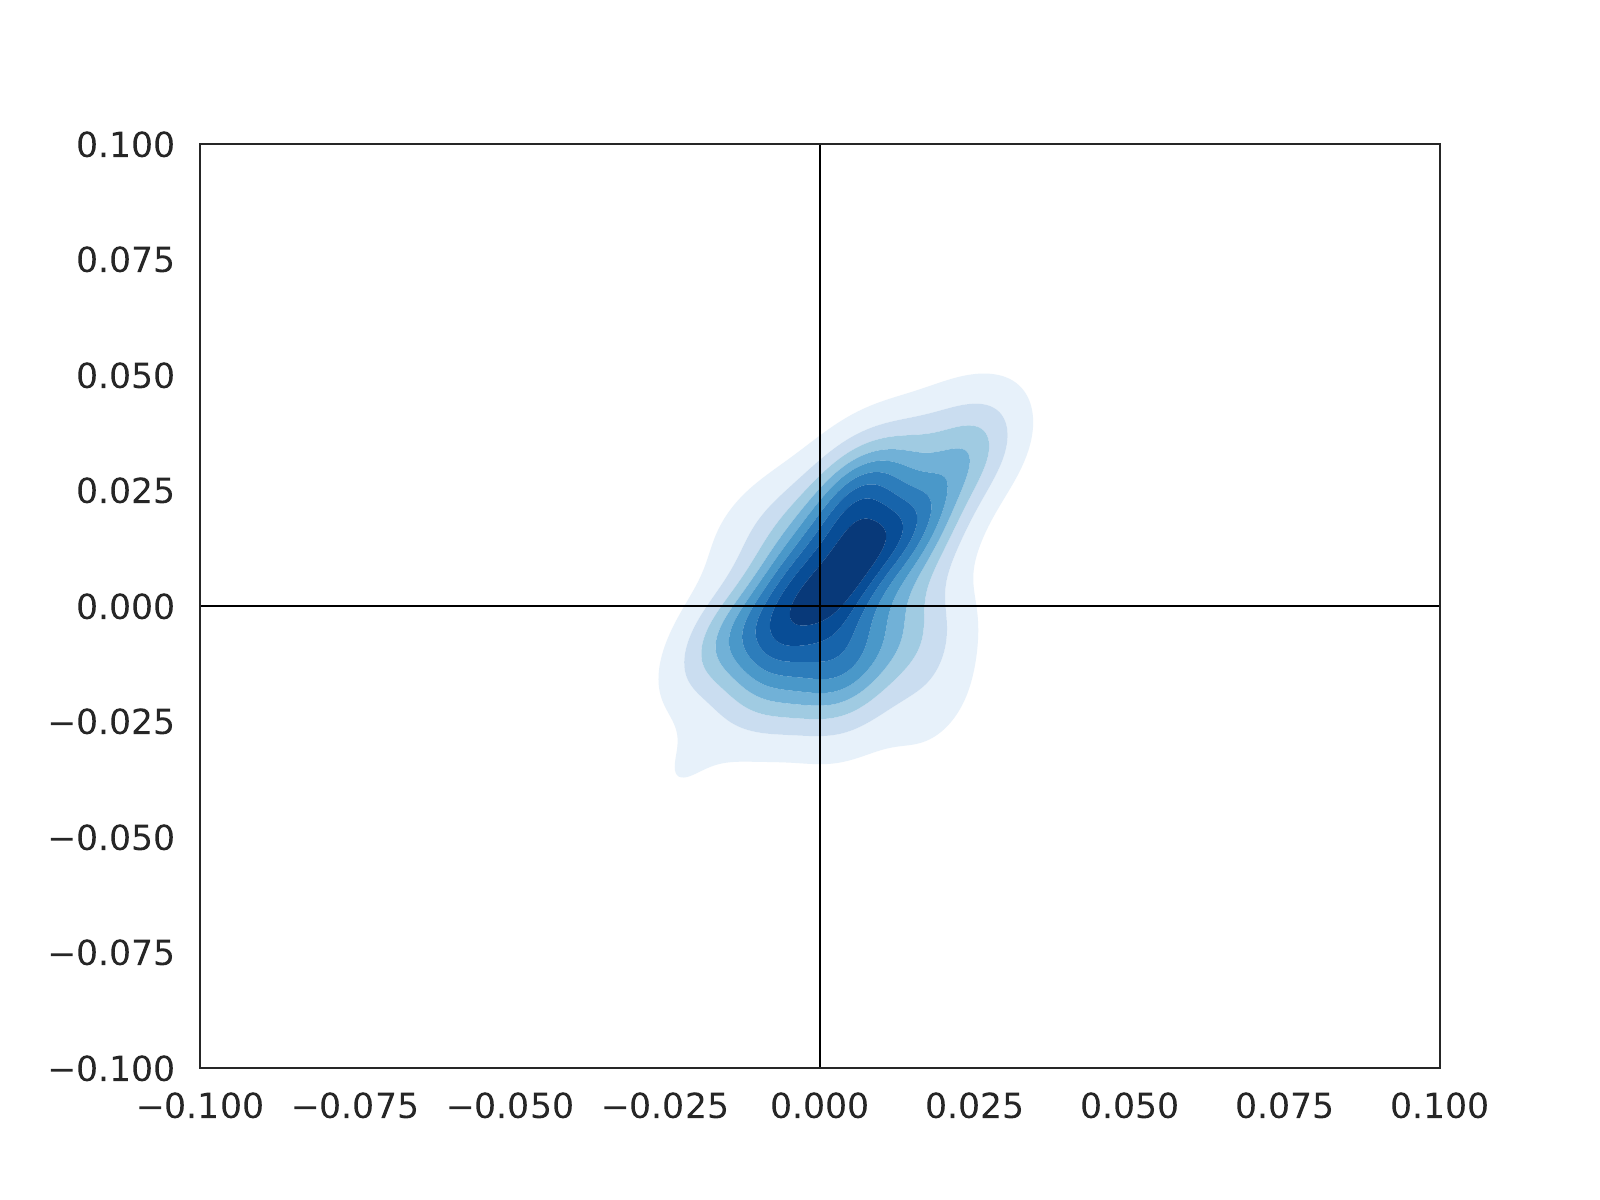} &
         \includegraphics[trim=60 80 60 80,clip,width=0.2\columnwidth]{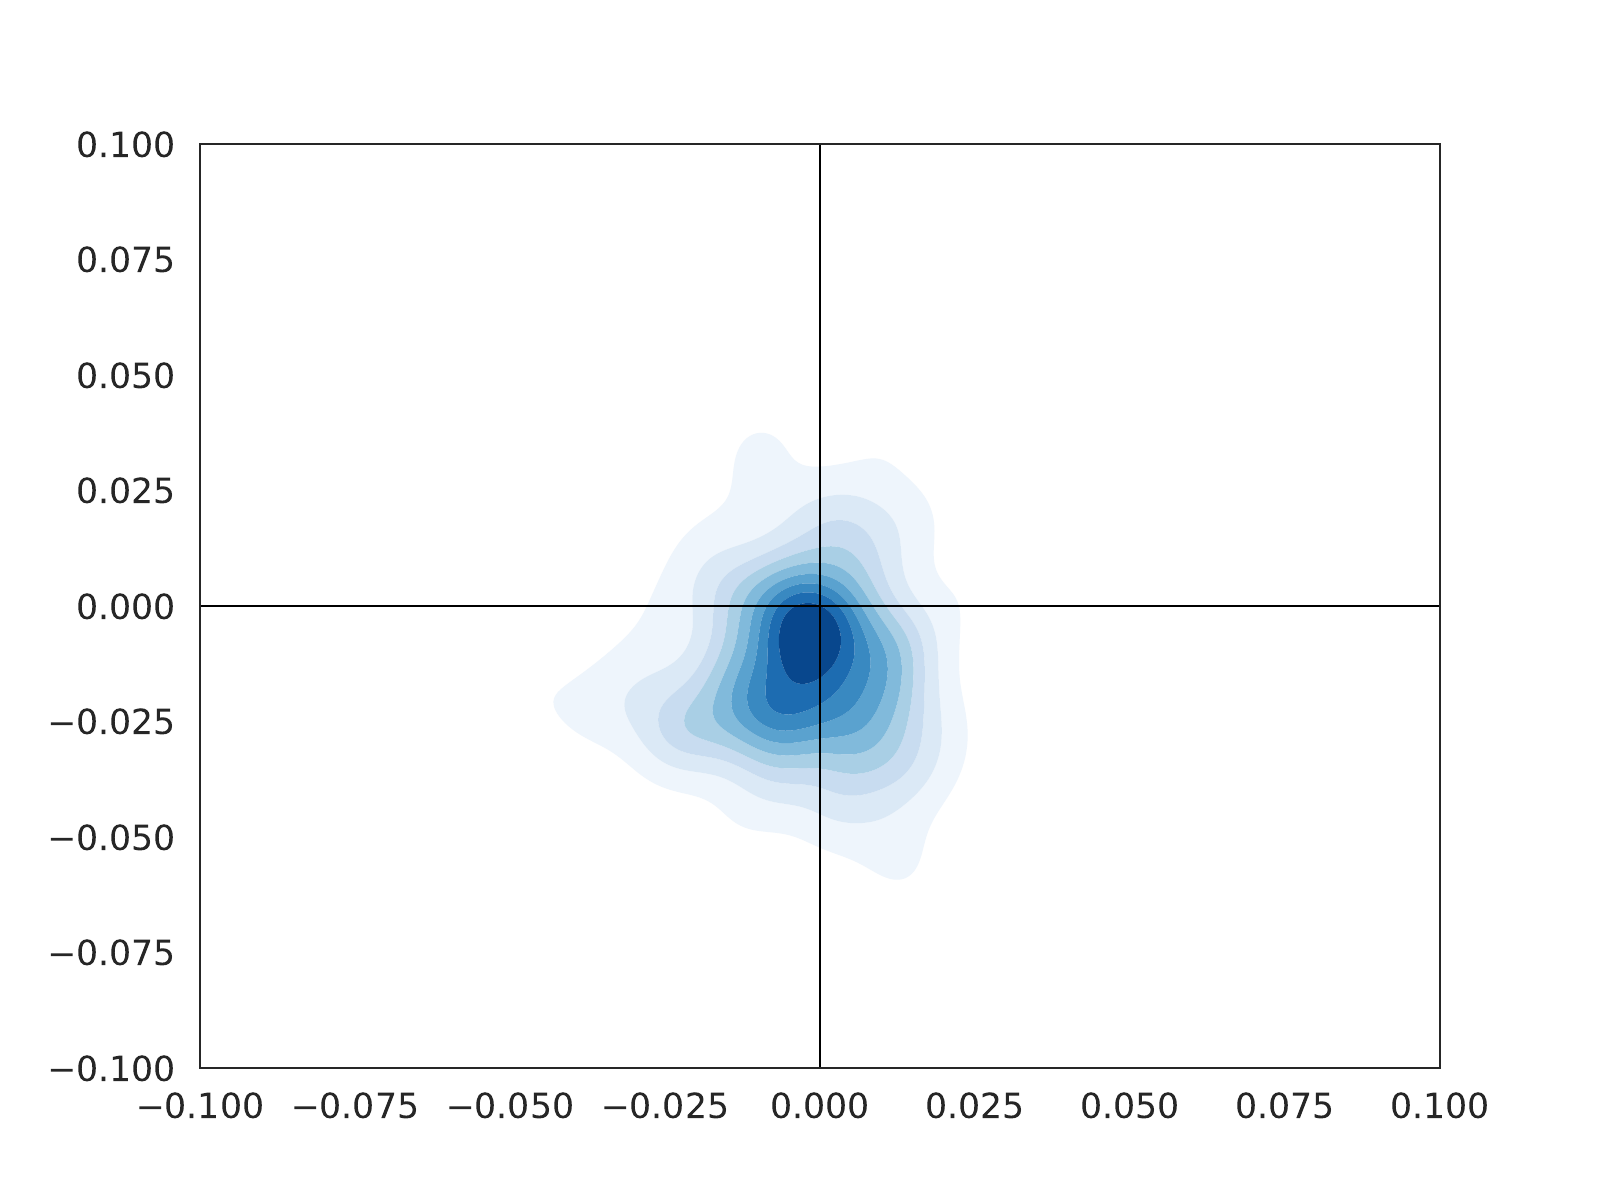} &
         \includegraphics[trim=60 80 60 80,clip,width=0.2\columnwidth]{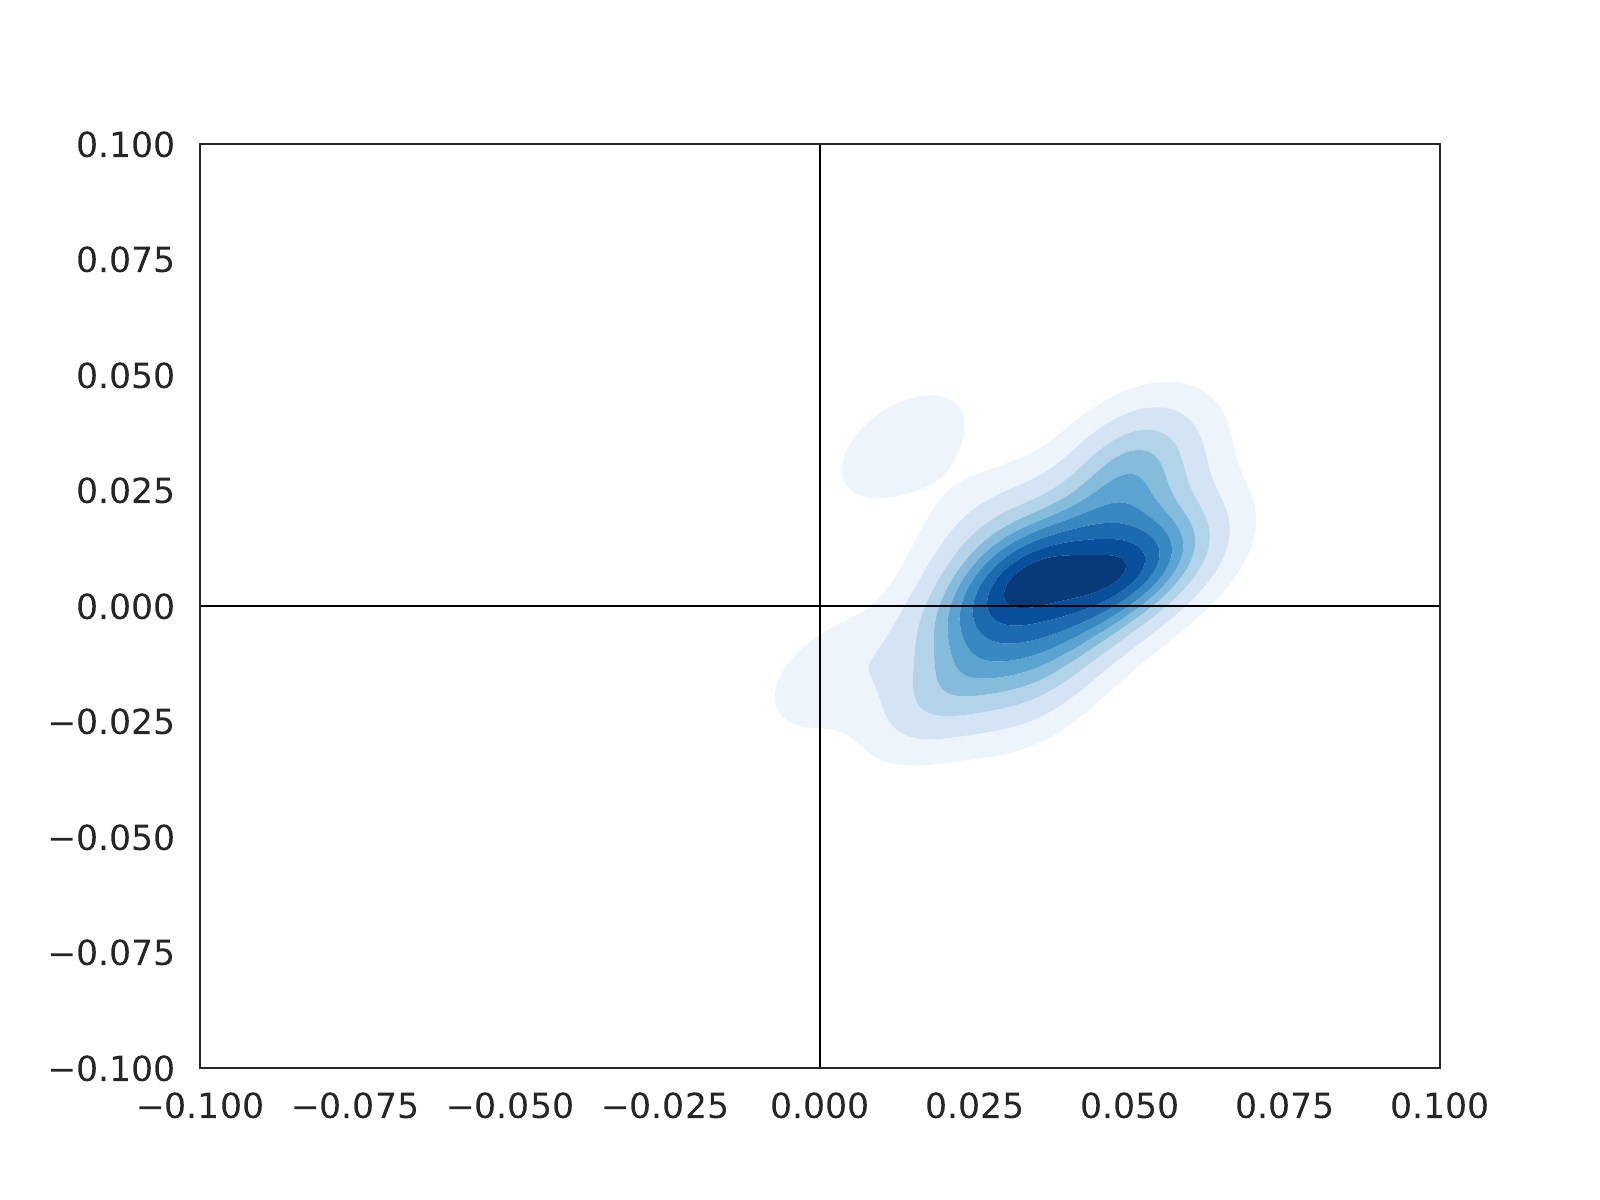} &
         \includegraphics[trim=60 80 60 80,clip,width=0.2\columnwidth]{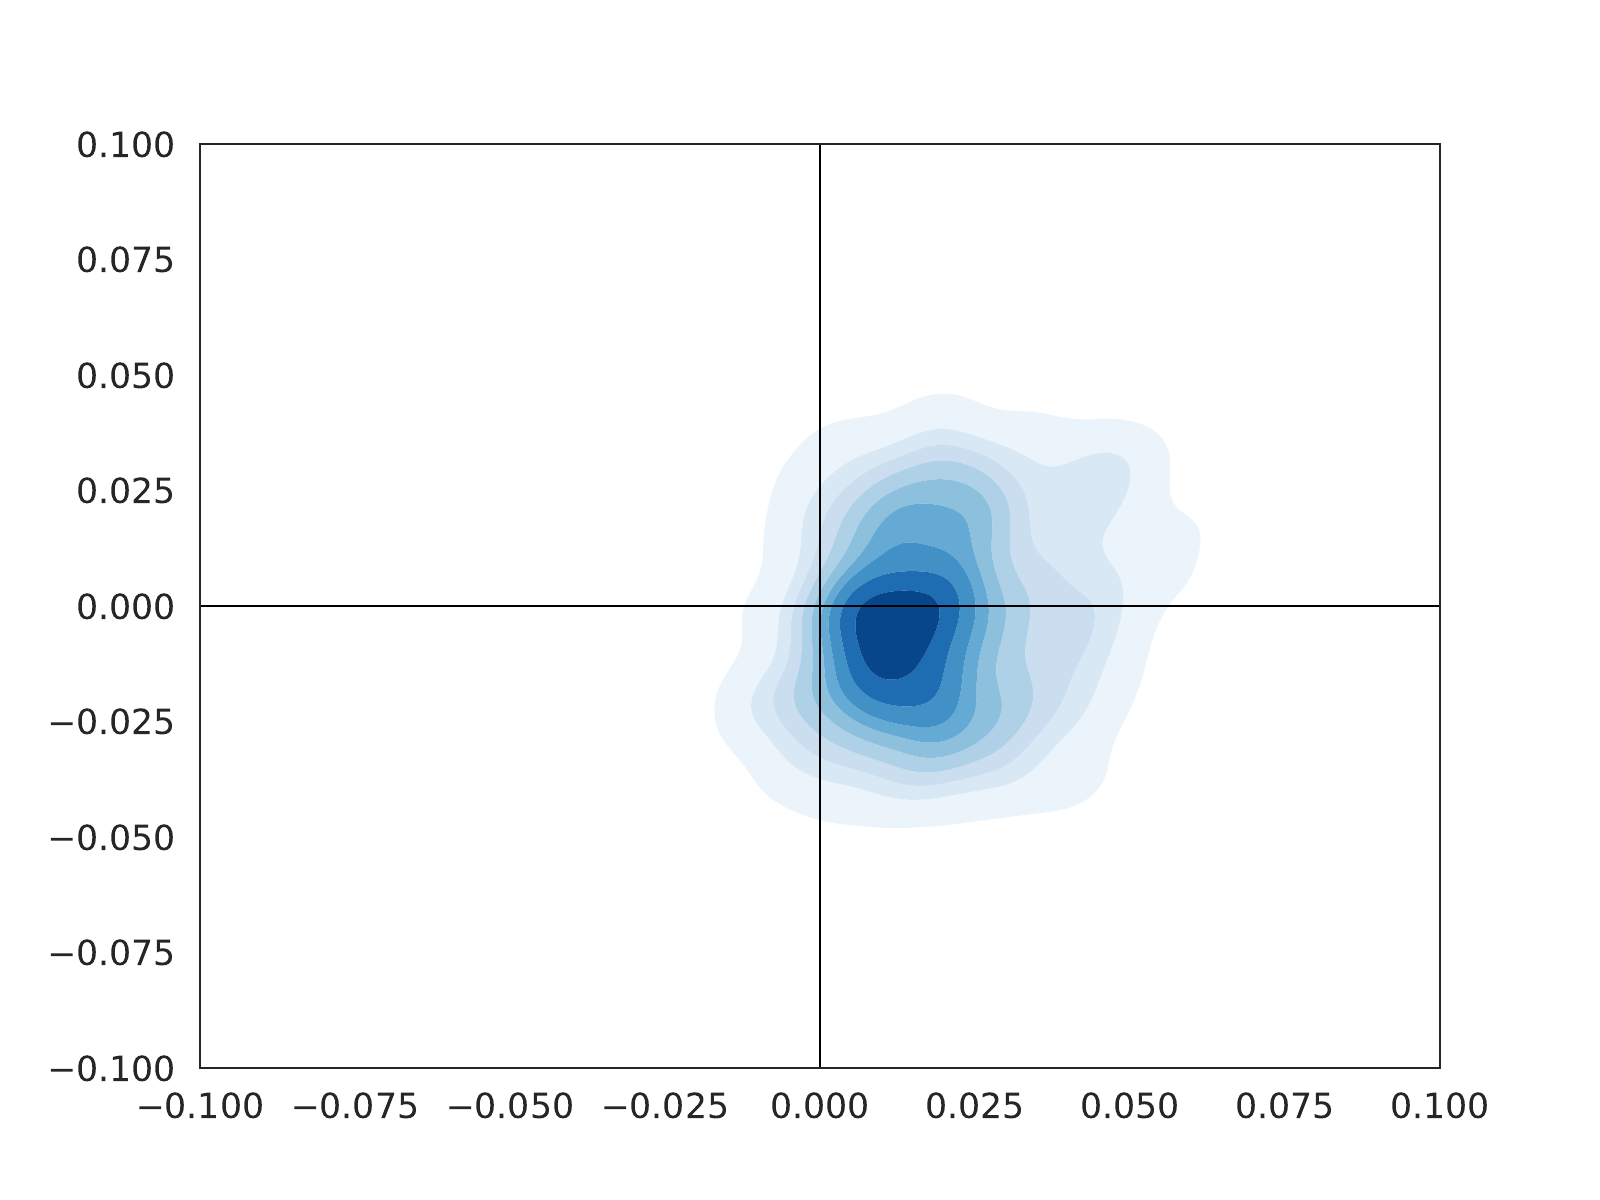} &
         \includegraphics[trim=60 80 60 80,clip,width=0.2\columnwidth]{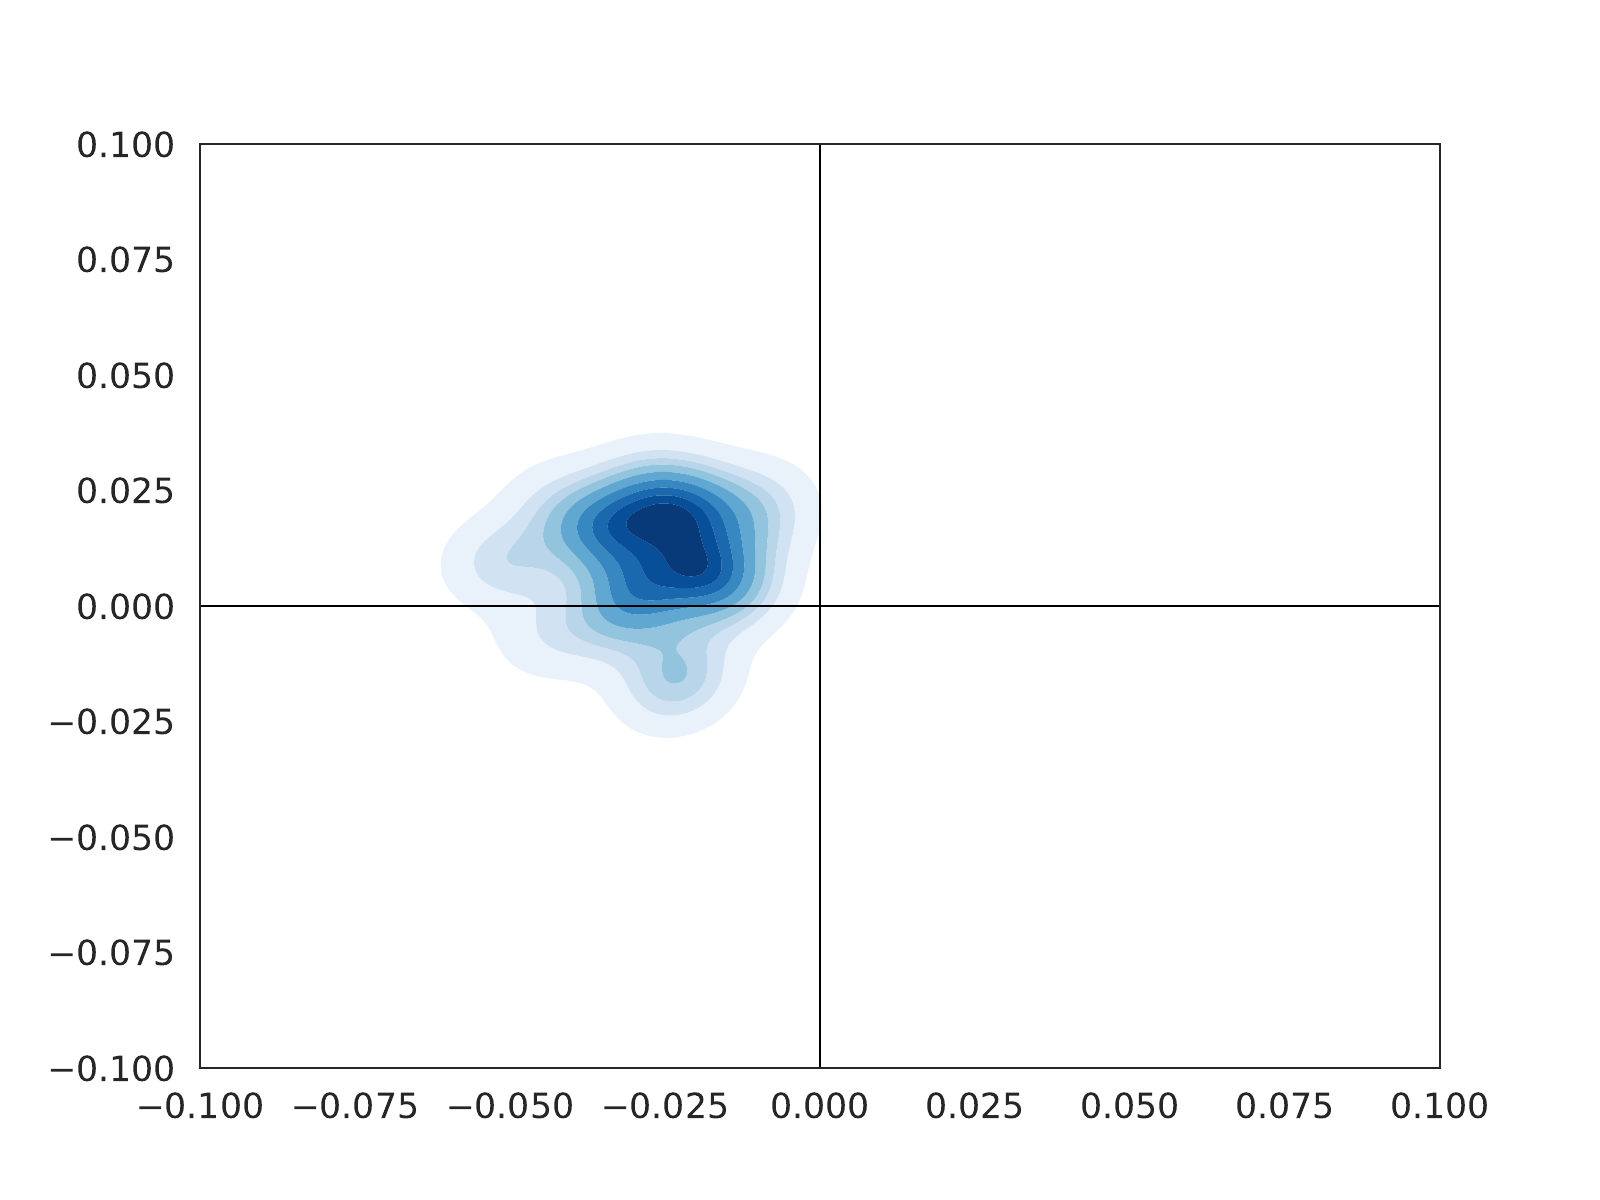} &
         \includegraphics[trim=60 80 60 80,clip,width=0.2\columnwidth]{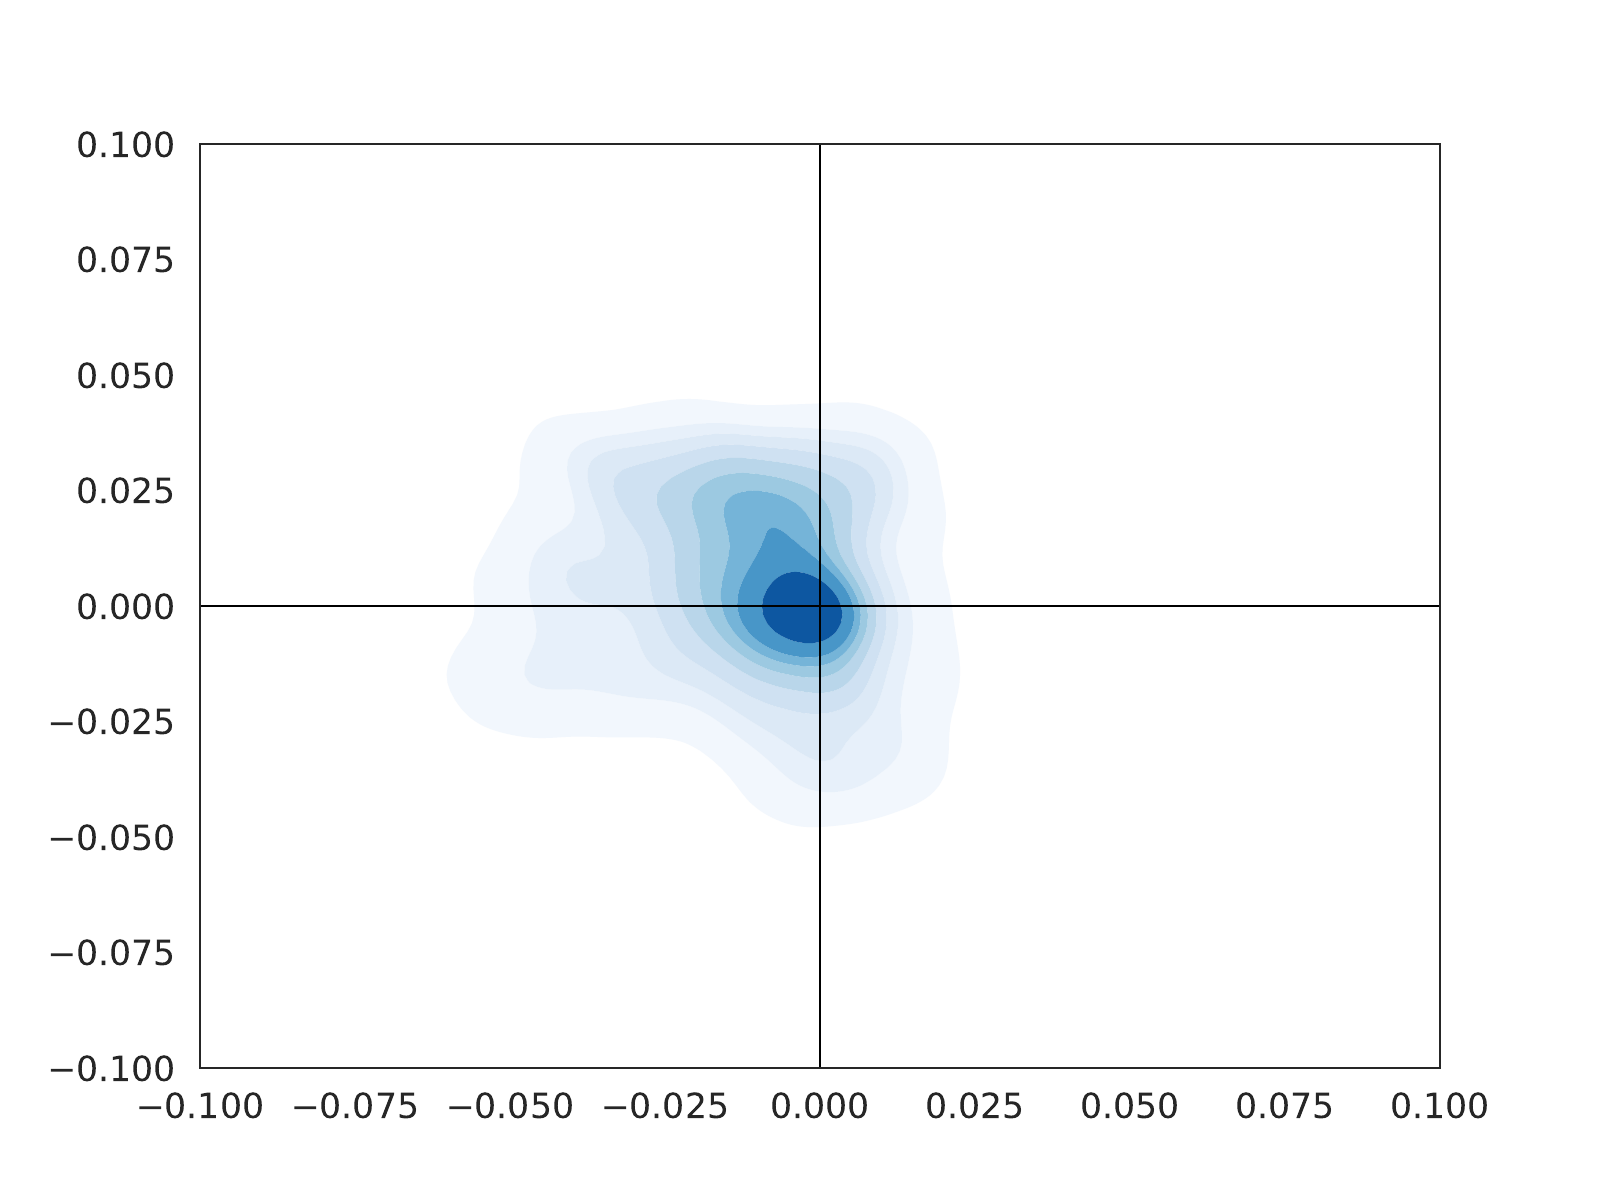} \\

    \end{tabular}
    }
    \captionof{figure}{Distribution of the displacement $\Delta$ associated with robot arm on the \emph{BAIR} dataset. Ideal distributions are different for each action and have low variance, meaning that they capture specific movements. The displacement component associated with movement on the vertical axis $z$ is not shown. While the distributions of the displacement $\Delta$ on the $x$ and $y$ axes associated with the SAVP and SAVP+ baselines are influenced by the input action, they do not successfully capture movement of the robot arm on the $z$ axis. This is reflected in the $\Delta$-\emph{MSE} score which shows that the actions learned by our model correspond to more specific movements than the ones learned by the baselines.}
    \label{fig:bair_density_plots}
\end{table*}
