# Supplementary material for: Playable Video Generation
Source: arXiv:2101.12195 source file (2021-01-28)
Supplement: Supplementary file 8 [file amt_votes_tables.tex]

\begin{table}
\begin{center}

\setlength{\tabcolsep}{5pt}
\footnotesize
\begin{tabular}{lccccccc}
\hline\noalign{\smallskip}
 & \emph{Hit} & \emph{Forward} & \emph{Backward} & \emph{Right} & \emph{Other} & \emph{Stay} & \emph{Left}  \\
\hline\noalign{\smallskip}
Act. 1 & 44 & 6 & 3 & 49 & 2 & 51 & 75 \\
Act. 2 & 40 & 6 & 4 & 57 & 6 & 47 & 70 \\
Act. 3 & 49 & 7 & 6 & 52 & 2 & 46 & 68 \\
Act. 4 & 46 & 7 & 3 & 48 & 3 & 49 & 74 \\
Act. 5 & 38 & 7 & 3 & 49 & 5 & 52 & 76 \\
Act. 6 & 34 & 6 & 6 & 51 & 5 & 50 & 78 \\
Act. 7 & 43 & 7 & 3 & 49 & 6 & 50 & 72 \\
\hline
\end{tabular}
\end{center}
\caption{AMT votes for MoCoGAN \cite{tulyakov2018moco} on the \emph{Tennis} dataset.}
\label{table:amt_votes_moco}
\end{table}

\begin{table}
\begin{center}

\setlength{\tabcolsep}{5pt}
\footnotesize
\begin{tabular}{lccccccc}
\hline\noalign{\smallskip}
 & \emph{Hit} & \emph{Forward} & \emph{Backward} & \emph{Right} & \emph{Other} & \emph{Stay} & \emph{Left}  \\
\hline\noalign{\smallskip}
Act. 1 & 20 & 6 & 2 & 94 & 61 & 12 & 35 \\
Act. 2 & 14 & 5 & 4 & 90 & 68 & 10 & 39 \\
Act. 3 & 24 & 7 & 2 & 92 & 66 & 4 & 35 \\
Act. 4 & 22 & 6 & 2 & 90 & 68 & 5 & 37 \\
Act. 5 & 26 & 3 & 2 & 86 & 67 & 9 & 37 \\
Act. 6 & 26 & 7 & 2 & 85 & 64 & 9 & 37 \\
Act. 7 & 20 & 11 & 2 & 86 & 57 & 12 & 42 \\
\hline
\end{tabular}
\end{center}
\caption{AMT votes for MoCoGAN+ on the \emph{Tennis} dataset.}
\label{table:amt_votes_moco_plus}
\end{table}

\begin{table}
\begin{center}
\setlength{\tabcolsep}{5pt}
\footnotesize
\begin{tabular}{lccccccc}
\hline\noalign{\smallskip}
 & \emph{Hit} & \emph{Forward} & \emph{Backward} & \emph{Right} & \emph{Other} & \emph{Stay} & \emph{Left}  \\
\hline\noalign{\smallskip}
Act. 1 & 50 & 15 & 27 & 25 & 10 & 45 & 58 \\
Act. 2 & 27 & 4 & 26 & 84 & 17 & 14 & 58 \\
Act. 3 & 22 & 8 & 18 & 54 & 13 & 10 & 105 \\
Act. 4 & 42 & 12 & 37 & 26 & 26 & 38 & 49 \\
Act. 5 & 19 & 7 & 26 & 81 & 25 & 20 & 52 \\
Act. 6 & 5 & 7 & 12 & 62 & 7 & 10 & 127 \\
Act. 7 & 60 & 21 & 19 & 7 & 17 & 95 & 11 \\
\hline
\end{tabular}
\end{center}
\caption{AMT votes for the SAVP \cite{lee2018savp} method on the \emph{Tennis} dataset.}
\label{table:amt_votes_savp}
\end{table}

\begin{table}
\begin{center}

\setlength{\tabcolsep}{5pt}
\footnotesize
\begin{tabular}{lccccccc}
\hline\noalign{\smallskip}
 & \emph{Hit} & \emph{Forward} & \emph{Backward} & \emph{Right} & \emph{Other} & \emph{Stay} & \emph{Left}  \\
\hline\noalign{\smallskip}
Act. 1 & 30 & 16 & 13 & 83 & 19 & 19 & 50 \\
Act. 2 & 36 & 24 & 7 & 88 & 2 & 25 & 48 \\
Act. 3 & 34 & 19 & 8 & 82 & 11 & 24 & 52 \\
Act. 4 & 36 & 17 & 10 & 88 & 13 & 22 & 44 \\
Act. 5 & 31 & 18 & 13 & 87 & 17 & 16 & 48 \\
Act. 6 & 24 & 17 & 10 & 91 & 13 & 29 & 46 \\
Act. 7 & 42 & 14 & 9 & 88 & 12 & 18 & 47 \\
\hline
\end{tabular}
\end{center}
\caption{AMT votes for the SAVP+ method on the \emph{Tennis} dataset.}
\label{table:amt_votes_savp_plus}
\end{table}

\begin{table}
\begin{center}

\setlength{\tabcolsep}{5pt}
\footnotesize
\begin{tabular}{lccccccc}
\hline\noalign{\smallskip}
 & \emph{Hit} & \emph{Forward} & \emph{Backward} & \emph{Right} & \emph{Other} & \emph{Stay} & \emph{Left}  \\
\hline\noalign{\smallskip}
Act. 1 & 21 & 62 & 1 & 122 & 4 & 15 & 5 \\
Act. 2 & 6 & 203 & 2 & 17 & 1 & 0 & 1 \\
Act. 3 & 7 & 2 & 137 & 15 & 14 & 7 & 48 \\
Act. 4 & 2 & 1 & 3 & 219 & 4 & 0 & 1 \\
Act. 5 & 20 & 8 & 52 & 19 & 2 & 27 & 102 \\
Act. 6 & 20 & 16 & 8 & 22 & 1 & 111 & 52 \\
Act. 7 & 10 & 13 & 2 & 0 & 3 & 1 & 201 \\
\hline
\end{tabular}
\end{center}
\caption{AMT votes for the our method on the \emph{Tennis} dataset.}
\label{table:amt_votes_ours}
\end{table}
