# Supplementary material for: Playable Video Generation
Source: arXiv:2101.12195 source file (2021-01-28)
Supplement: Supplementary file 10 [file tennis_reconstruction_39.tex]

\begin{table*}
    \centering
    
    \resizebox{\linewidth}{!}{
    \setlength\tabcolsep{0pt}
    \tiny
    
    \begin{tabular}{r@{\hskip 0.7mm}cccccc}
         & $t=1$ & $t=4$ & $t=7$ & $t=10$ & $t=13$ & $t=16$  \\
         \rotatebox{90}{\hspace{0mm}Original} &
         \includegraphics[width=0.2\columnwidth]{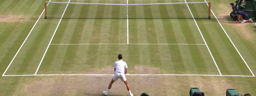} &
         \includegraphics[width=0.2\columnwidth]{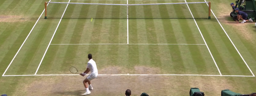} &
         \includegraphics[width=0.2\columnwidth]{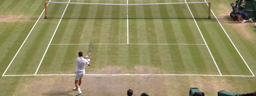} &
         \includegraphics[width=0.2\columnwidth]{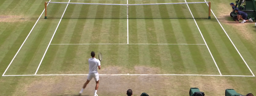} &
         \includegraphics[width=0.2\columnwidth]{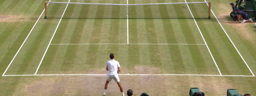} &
         \includegraphics[width=0.2\columnwidth]{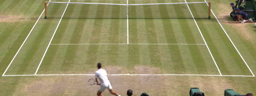} \\
         
         \rotatebox{90}{\hspace{0mm}\scalebox{0.55}{MoCoGAN \cite{tulyakov2018moco}}} &
         \includegraphics[width=0.2\columnwidth]{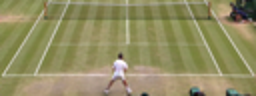} &
         \includegraphics[width=0.2\columnwidth]{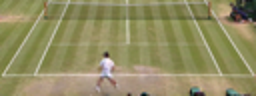} &
         \includegraphics[width=0.2\columnwidth]{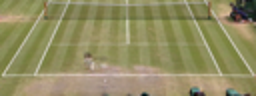} &
         \includegraphics[width=0.2\columnwidth]{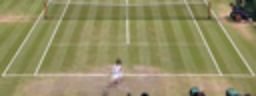} &
         \includegraphics[width=0.2\columnwidth]{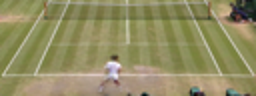} &
         \includegraphics[width=0.2\columnwidth]{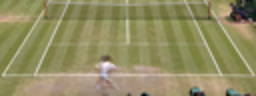} \\
         
         \rotatebox{90}{\hspace{0mm}\scalebox{0.65}{MoCoGAN+}} &
         \includegraphics[width=0.2\columnwidth]{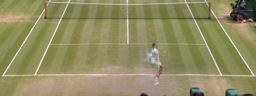} &
         \includegraphics[width=0.2\columnwidth]{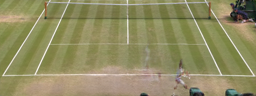} &
         \includegraphics[width=0.2\columnwidth]{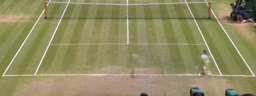} &
         \includegraphics[width=0.2\columnwidth]{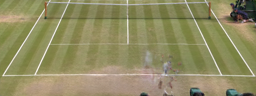} &
         \includegraphics[width=0.2\columnwidth]{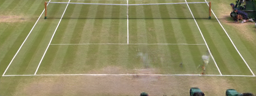} &
         \includegraphics[width=0.2\columnwidth]{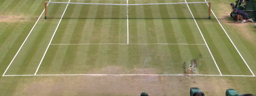} \\
         
         \rotatebox{90}{\hspace{0mm}SAVP\cite{lee2018savp}} &
         \includegraphics[width=0.2\columnwidth]{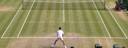} &
         \includegraphics[width=0.2\columnwidth]{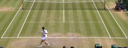} &
         \includegraphics[width=0.2\columnwidth]{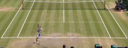} &
         \includegraphics[width=0.2\columnwidth]{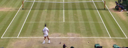} &
         \includegraphics[width=0.2\columnwidth]{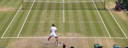} &
         \includegraphics[width=0.2\columnwidth]{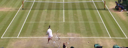} \\
         
         \rotatebox{90}{\hspace{0.5mm}SAVP+} &
         \includegraphics[width=0.2\columnwidth]{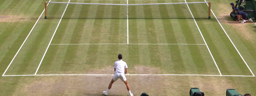} &
         \includegraphics[width=0.2\columnwidth]{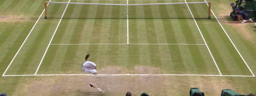} &
         \includegraphics[width=0.2\columnwidth]{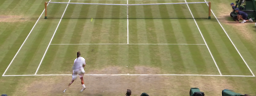} &
         \includegraphics[width=0.2\columnwidth]{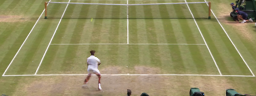} &
         \includegraphics[width=0.2\columnwidth]{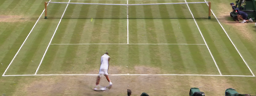} &
         \includegraphics[width=0.2\columnwidth]{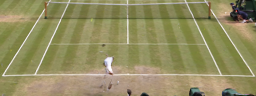} \\
         
         \rotatebox{90}{\hspace{1.5mm}Ours} &
         \includegraphics[width=0.2\columnwidth]{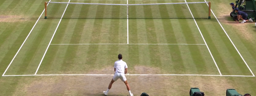} &
         \includegraphics[width=0.2\columnwidth]{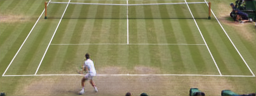} &
         \includegraphics[width=0.2\columnwidth]{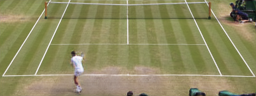} &
         \includegraphics[width=0.2\columnwidth]{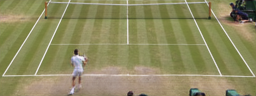} &
         \includegraphics[width=0.2\columnwidth]{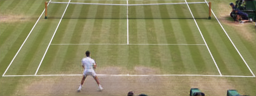} &
         \includegraphics[width=0.2\columnwidth]{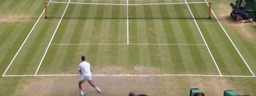} \\

    \end{tabular}
    }
    \captionof{figure}{Reconstructed sequences on the \emph{Tennis} dataset using the learned, discrete actions extracted from the original sequence as inputs.}
    \label{fig:tennis_reconstruction_39}
\end{table*}
