# Supplementary material for: Playable Video Generation
Source: arXiv:2101.12195 source file (2021-01-28)
Supplement: Supplementary file 11 [file action_space_visualizations.tex]

\begin{figure*}
\centering
\resizebox{\linewidth}{!}{
\begin{subfigure}{.33\textwidth}
  \centering
  \includegraphics[trim=60 40 130 50,clip,width=1\linewidth]{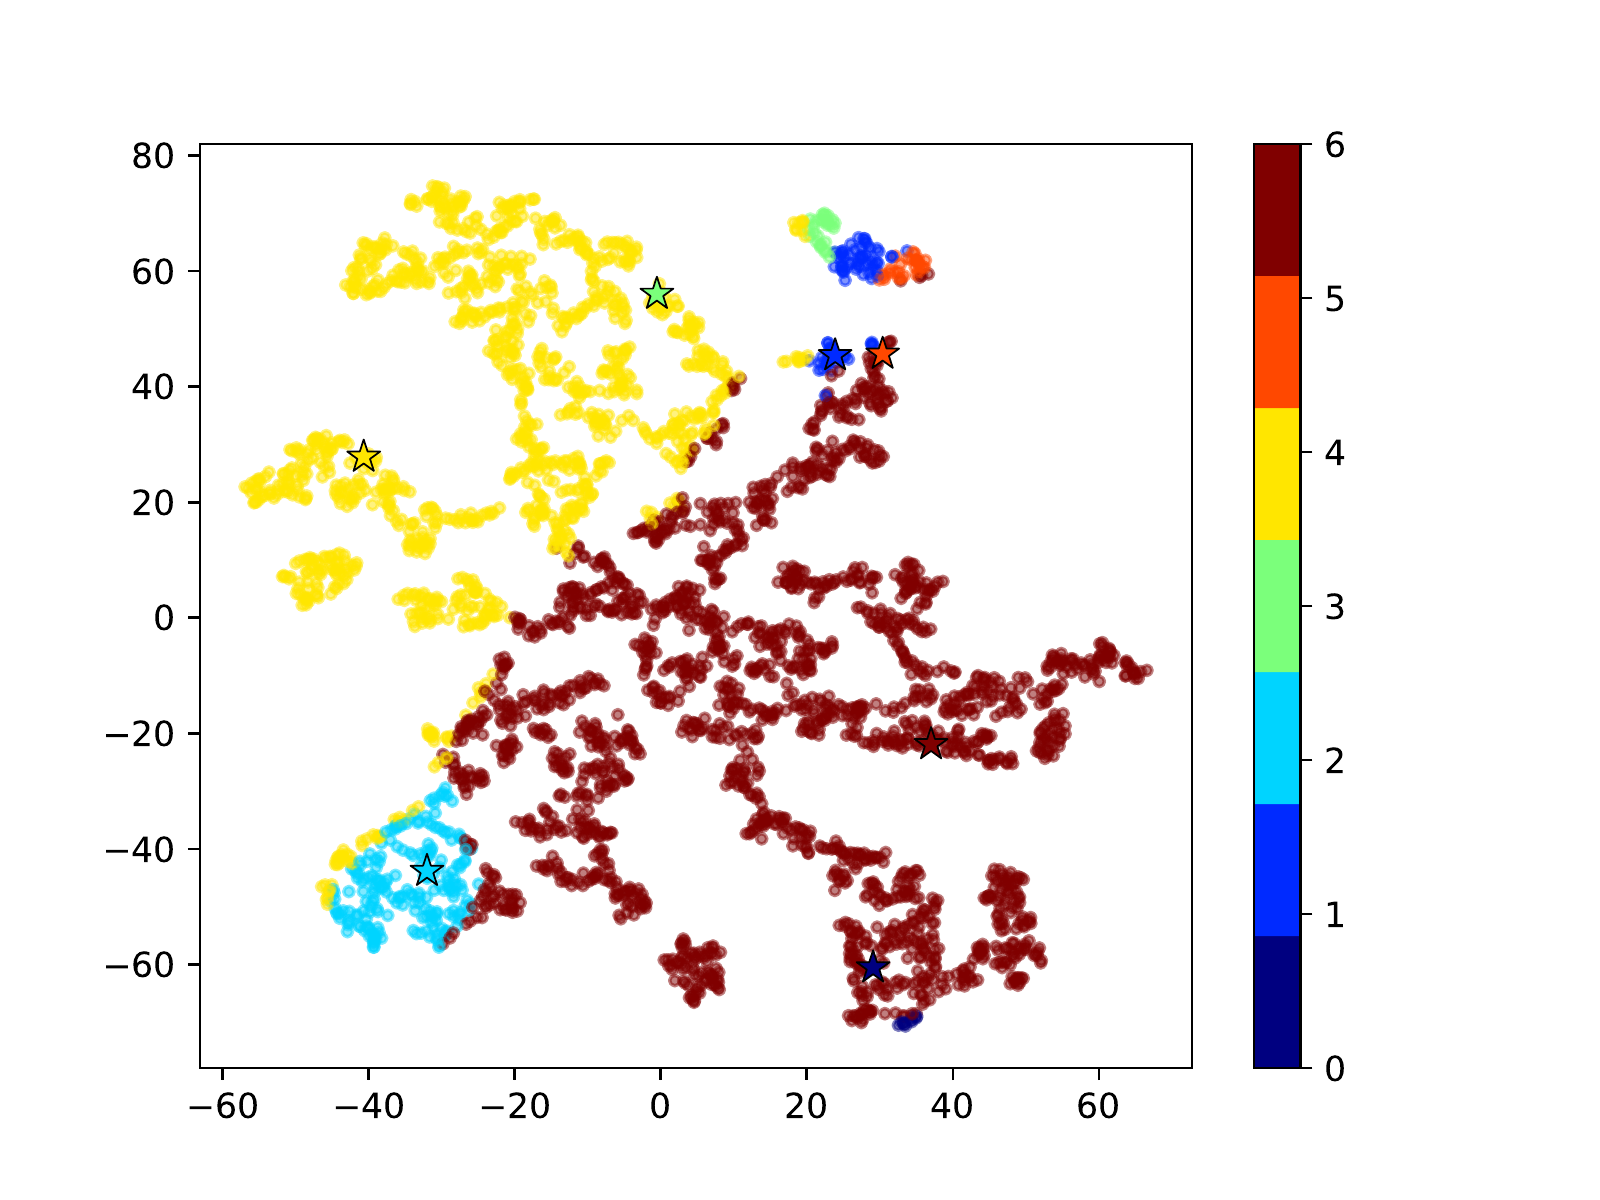}
  \caption{\emph{BAIR}}
  \label{fig:action_space_bair}
\end{subfigure}%
\begin{subfigure}{.33\textwidth}
  \centering
  \includegraphics[trim=60 40 130 50,clip,width=0.8\linewidth]{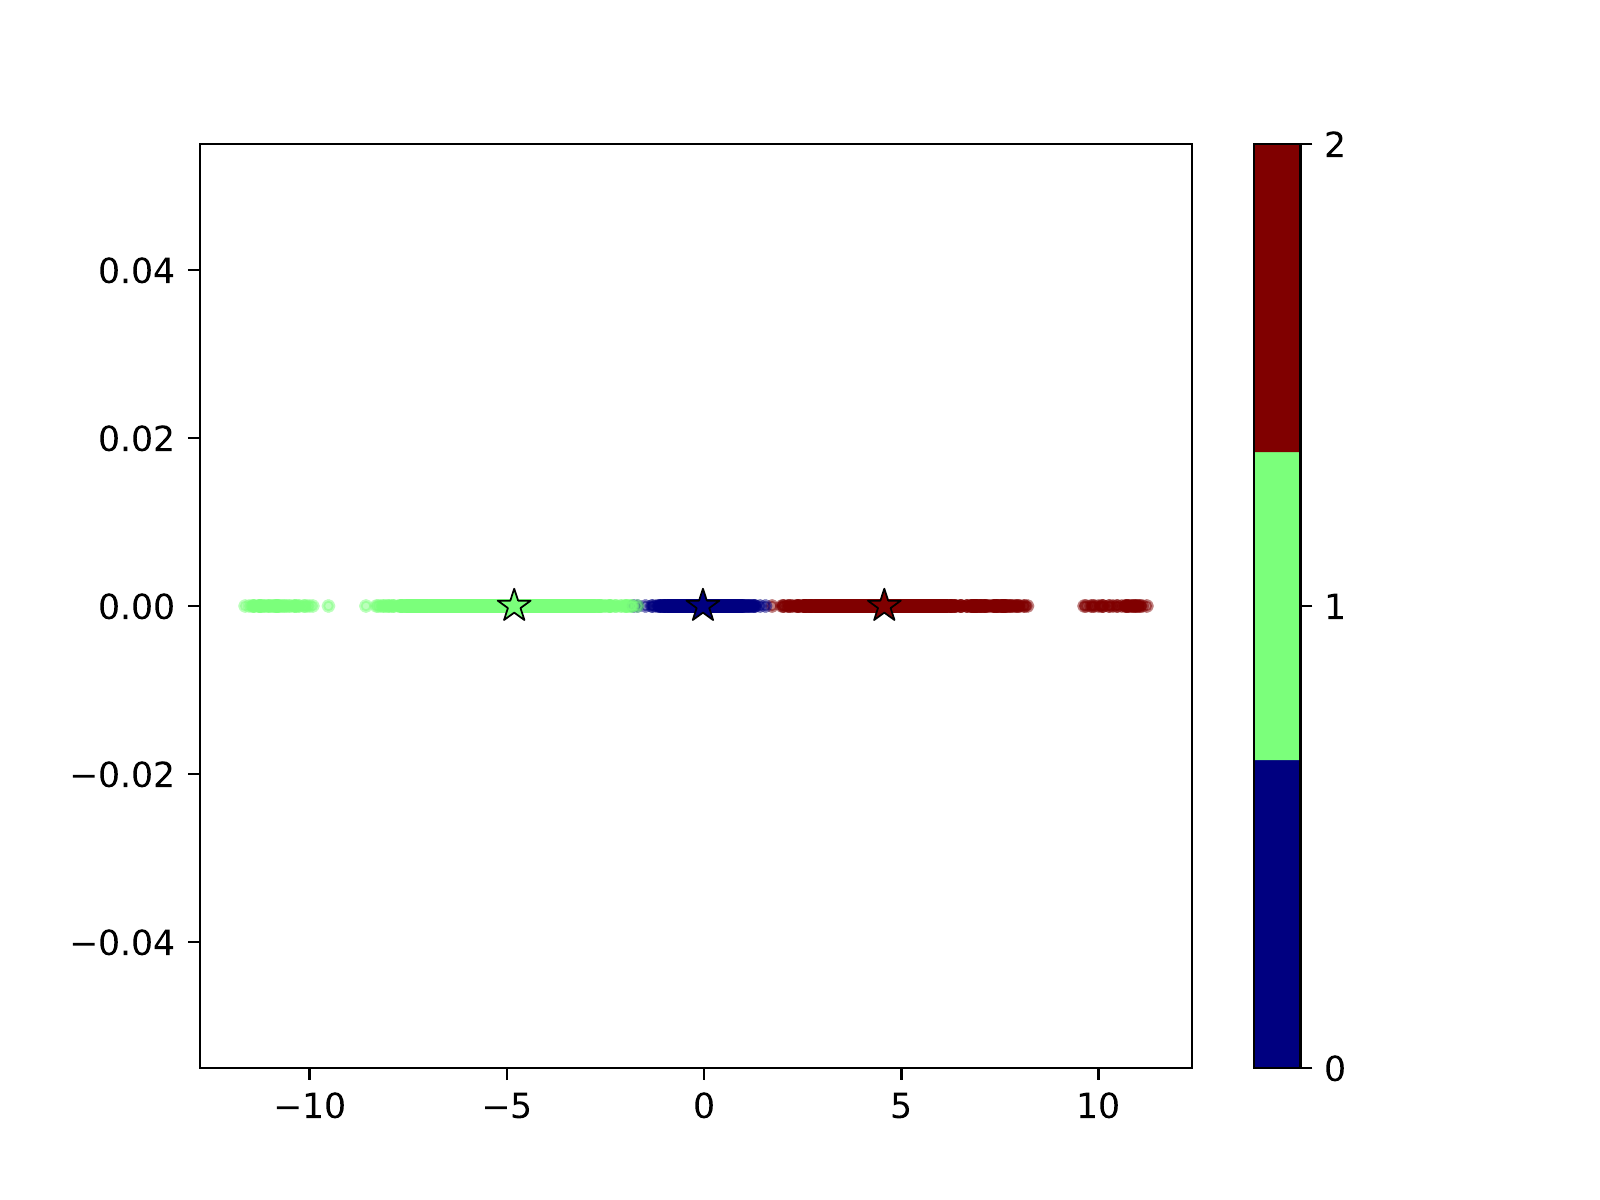}
  \caption{\emph{Atari Breakout}}
  \label{fig:action_space_breakout}
\end{subfigure}
\begin{subfigure}{.33\textwidth}
  \centering
  \includegraphics[trim=60 40 130 50,clip,width=1\linewidth]{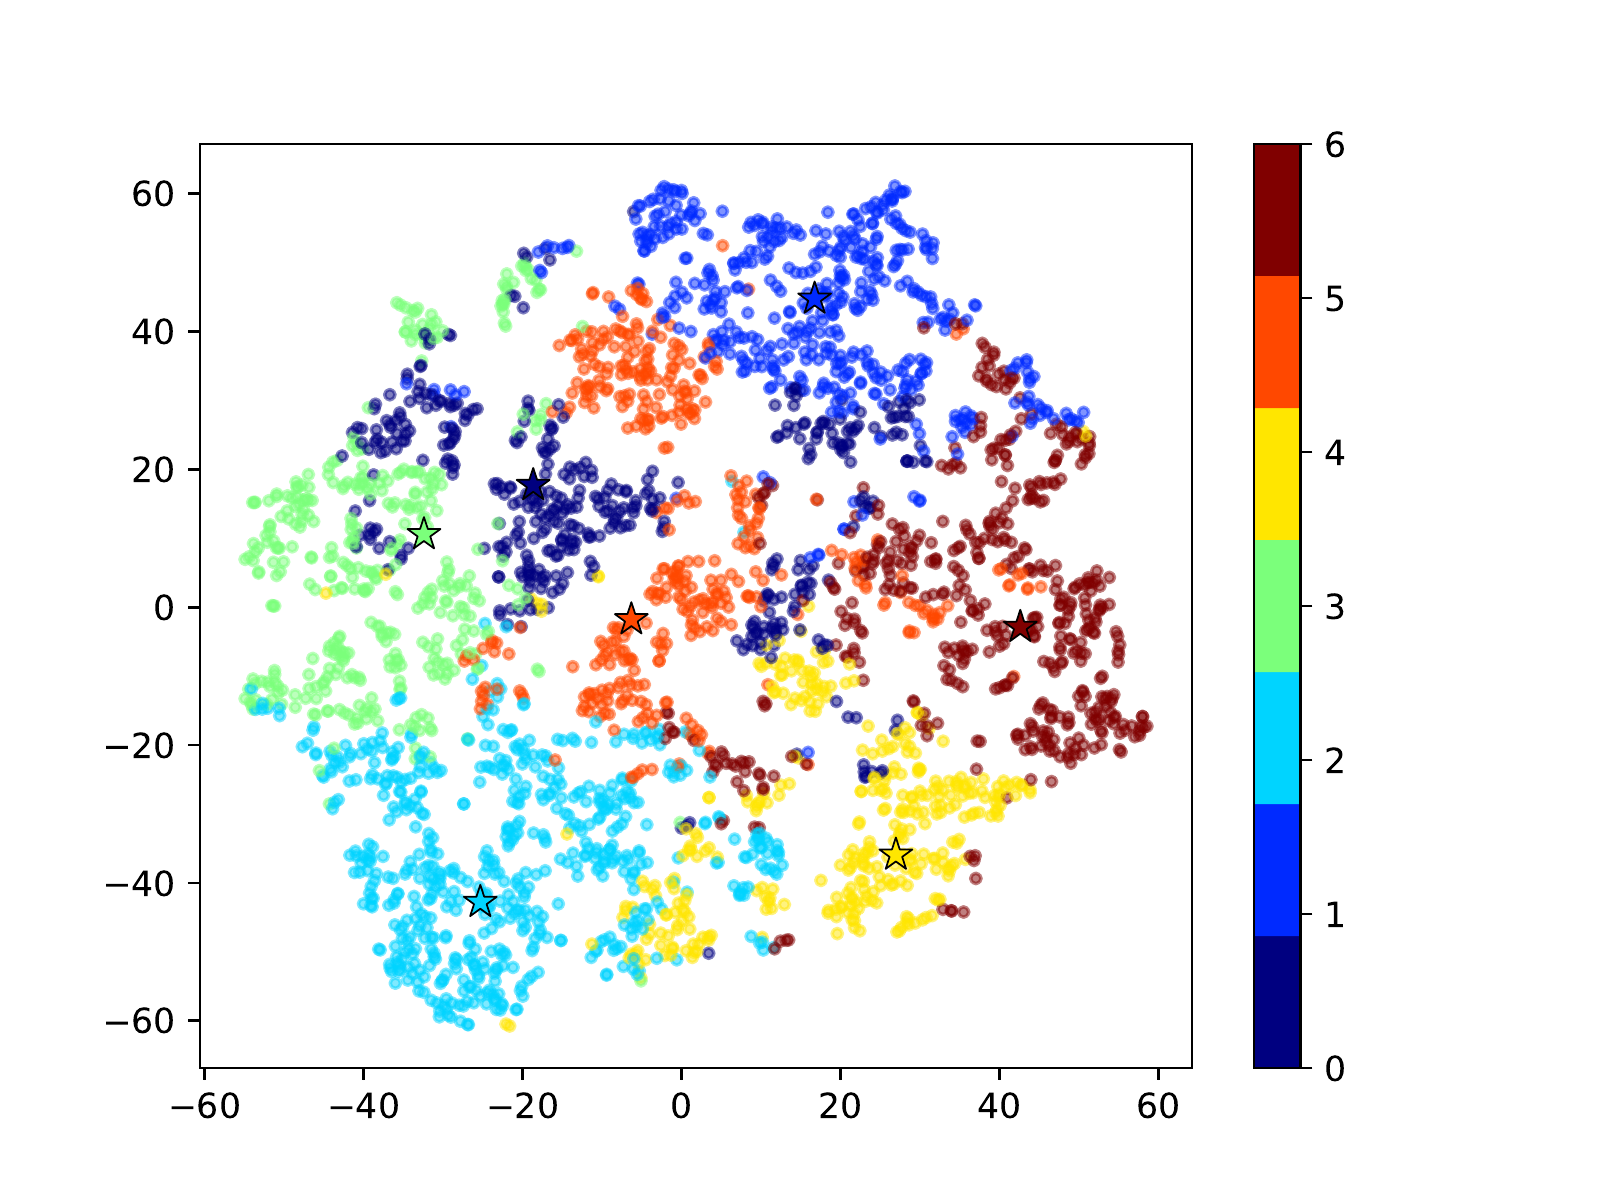}
  \caption{\emph{Tennis}}
  \label{fig:action_space_tennis}
\end{subfigure}
}
\caption{Visualizations of the learned space of \emph{action directions} $d_t$ with corresponding \textit{action direction centroids} $\{c_k\}_{k=1}^{K}$, grouped by action.}
\label{fig:action_space}
\end{figure*}
