# Supplementary material for: Playable Video Generation
Source: arXiv:2101.12195 source file (2021-01-28)
Supplement: Supplementary file 13 [file bair_reconstruction_119.tex]

\begin{table*}
    \centering
    
    \resizebox{\linewidth}{!}{
    \setlength\tabcolsep{0pt}
    \footnotesize
    
    \begin{tabular}{l@{\hskip 1mm}ccccccccccc}
         & $t=1$ & $t=4$ & $t=7$ & $t=10$ & $t=13$ & $t=16$ & $t=19$ & $t=22$ & $t=25$ & $t=28$ & $t=30$  \\
         \rotatebox{90}{\hspace{3.5mm}Original} &
         \includegraphics[trim=2 0 0 2,clip,width=0.2\columnwidth]{supplementary_resources/bair/original/119/00000.png} & 
         \includegraphics[trim=2 0 0 2,clip,width=0.2\columnwidth]{supplementary_resources/bair/original/119/00003.png} & 
         \includegraphics[trim=2 0 0 2,clip,width=0.2\columnwidth]{supplementary_resources/bair/original/119/00006.png} & 
         \includegraphics[trim=2 0 0 2,clip,width=0.2\columnwidth]{supplementary_resources/bair/original/119/00009.png} & 
         \includegraphics[trim=2 0 0 2,clip,width=0.2\columnwidth]{supplementary_resources/bair/original/119/00012.png} & 
         \includegraphics[trim=2 0 0 2,clip,width=0.2\columnwidth]{supplementary_resources/bair/original/119/00015.png} & 
         \includegraphics[trim=2 0 0 2,clip,width=0.2\columnwidth]{supplementary_resources/bair/original/119/00018.png} & 
         \includegraphics[trim=2 0 0 2,clip,width=0.2\columnwidth]{supplementary_resources/bair/original/119/00021.png} & 
         \includegraphics[trim=2 0 0 2,clip,width=0.2\columnwidth]{supplementary_resources/bair/original/119/00024.png} & 
         \includegraphics[trim=2 0 0 2,clip,width=0.2\columnwidth]{supplementary_resources/bair/original/119/00027.png} & 
         \includegraphics[trim=2 0 0 2,clip,width=0.2\columnwidth]{supplementary_resources/bair/original/119/00029.png} \\
         
         \rotatebox{90}{\hspace{0mm}\scalebox{0.94}{MoCoGAN \cite{tulyakov2018moco}}} &
         \includegraphics[trim=2 0 0 2,clip,width=0.2\columnwidth]{supplementary_resources/bair/moco/119/00000.png} & 
         \includegraphics[trim=2 0 0 2,clip,width=0.2\columnwidth]{supplementary_resources/bair/moco/119/00003.png} & 
         \includegraphics[trim=2 0 0 2,clip,width=0.2\columnwidth]{supplementary_resources/bair/moco/119/00006.png} & 
         \includegraphics[trim=2 0 0 2,clip,width=0.2\columnwidth]{supplementary_resources/bair/moco/119/00009.png} & 
         \includegraphics[trim=2 0 0 2,clip,width=0.2\columnwidth]{supplementary_resources/bair/moco/119/00012.png} & 
         \includegraphics[trim=2 0 0 2,clip,width=0.2\columnwidth]{supplementary_resources/bair/moco/119/00015.png} & 
         \includegraphics[trim=2 0 0 2,clip,width=0.2\columnwidth]{supplementary_resources/bair/moco/119/00018.png} & 
         \includegraphics[trim=2 0 0 2,clip,width=0.2\columnwidth]{supplementary_resources/bair/moco/119/00021.png} & 
         \includegraphics[trim=2 0 0 2,clip,width=0.2\columnwidth]{supplementary_resources/bair/moco/119/00024.png} & 
         \includegraphics[trim=2 0 0 2,clip,width=0.2\columnwidth]{supplementary_resources/bair/moco/119/00027.png} & 
         \includegraphics[trim=2 0 0 2,clip,width=0.2\columnwidth]{supplementary_resources/bair/moco/119/00029.png} \\
         
         \rotatebox{90}{\hspace{1mm}MoCoGAN+} &
         \includegraphics[trim=2 0 0 2,clip,width=0.2\columnwidth]{supplementary_resources/bair/moco_plus/119/00000.png} & 
         \includegraphics[trim=2 0 0 2,clip,width=0.2\columnwidth]{supplementary_resources/bair/moco_plus/119/00003.png} & 
         \includegraphics[trim=2 0 0 2,clip,width=0.2\columnwidth]{supplementary_resources/bair/moco_plus/119/00006.png} & 
         \includegraphics[trim=2 0 0 2,clip,width=0.2\columnwidth]{supplementary_resources/bair/moco_plus/119/00009.png} & 
         \includegraphics[trim=2 0 0 2,clip,width=0.2\columnwidth]{supplementary_resources/bair/moco_plus/119/00012.png} & 
         \includegraphics[trim=2 0 0 2,clip,width=0.2\columnwidth]{supplementary_resources/bair/moco_plus/119/00015.png} & 
         \includegraphics[trim=2 0 0 2,clip,width=0.2\columnwidth]{supplementary_resources/bair/moco_plus/119/00018.png} & 
         \includegraphics[trim=2 0 0 2,clip,width=0.2\columnwidth]{supplementary_resources/bair/moco_plus/119/00021.png} & 
         \includegraphics[trim=2 0 0 2,clip,width=0.2\columnwidth]{supplementary_resources/bair/moco_plus/119/00024.png} & 
         \includegraphics[trim=2 0 0 2,clip,width=0.2\columnwidth]{supplementary_resources/bair/moco_plus/119/00027.png} & 
         \includegraphics[trim=2 0 0 2,clip,width=0.2\columnwidth]{supplementary_resources/bair/moco_plus/119/00029.png} \\
         
         \rotatebox{90}{\hspace{2.5mm}SAVP \cite{lee2018savp}} &
         \includegraphics[trim=2 0 0 2,clip,width=0.2\columnwidth]{supplementary_resources/bair/savp/119/00000.png} & 
         \includegraphics[trim=2 0 0 2,clip,width=0.2\columnwidth]{supplementary_resources/bair/savp/119/00003.png} & 
         \includegraphics[trim=2 0 0 2,clip,width=0.2\columnwidth]{supplementary_resources/bair/savp/119/00006.png} & 
         \includegraphics[trim=2 0 0 2,clip,width=0.2\columnwidth]{supplementary_resources/bair/savp/119/00009.png} & 
         \includegraphics[trim=2 0 0 2,clip,width=0.2\columnwidth]{supplementary_resources/bair/savp/119/00012.png} & 
         \includegraphics[trim=2 0 0 2,clip,width=0.2\columnwidth]{supplementary_resources/bair/savp/119/00015.png} & 
         \includegraphics[trim=2 0 0 2,clip,width=0.2\columnwidth]{supplementary_resources/bair/savp/119/00018.png} & 
         \includegraphics[trim=2 0 0 2,clip,width=0.2\columnwidth]{supplementary_resources/bair/savp/119/00021.png} & 
         \includegraphics[trim=2 0 0 2,clip,width=0.2\columnwidth]{supplementary_resources/bair/savp/119/00024.png} & 
         \includegraphics[trim=2 0 0 2,clip,width=0.2\columnwidth]{supplementary_resources/bair/savp/119/00027.png} & 
         \includegraphics[trim=2 0 0 2,clip,width=0.2\columnwidth]{supplementary_resources/bair/savp/119/00029.png} \\
         
         \rotatebox{90}{\hspace{4mm}SAVP+} &
         \includegraphics[trim=2 0 0 2,clip,width=0.2\columnwidth]{supplementary_resources/bair/savp_plus/119/00000.png} & 
         \includegraphics[trim=2 0 0 2,clip,width=0.2\columnwidth]{supplementary_resources/bair/savp_plus/119/00003.png} & 
         \includegraphics[trim=2 0 0 2,clip,width=0.2\columnwidth]{supplementary_resources/bair/savp_plus/119/00006.png} & 
         \includegraphics[trim=2 0 0 2,clip,width=0.2\columnwidth]{supplementary_resources/bair/savp_plus/119/00009.png} & 
         \includegraphics[trim=2 0 0 2,clip,width=0.2\columnwidth]{supplementary_resources/bair/savp_plus/119/00012.png} & 
         \includegraphics[trim=2 0 0 2,clip,width=0.2\columnwidth]{supplementary_resources/bair/savp_plus/119/00015.png} & 
         \includegraphics[trim=2 0 0 2,clip,width=0.2\columnwidth]{supplementary_resources/bair/savp_plus/119/00018.png} & 
         \includegraphics[trim=2 0 0 2,clip,width=0.2\columnwidth]{supplementary_resources/bair/savp_plus/119/00021.png} & 
         \includegraphics[trim=2 0 0 2,clip,width=0.2\columnwidth]{supplementary_resources/bair/savp_plus/119/00024.png} & 
         \includegraphics[trim=2 0 0 2,clip,width=0.2\columnwidth]{supplementary_resources/bair/savp_plus/119/00027.png} & 
         \includegraphics[trim=2 0 0 2,clip,width=0.2\columnwidth]{supplementary_resources/bair/savp_plus/119/00029.png} \\
         
         \rotatebox{90}{\hspace{6mm}Ours} &
         \includegraphics[trim=2 0 0 2,clip,width=0.2\columnwidth]{supplementary_resources/bair/ours/119/00000.png} & 
         \includegraphics[trim=2 0 0 2,clip,width=0.2\columnwidth]{supplementary_resources/bair/ours/119/00003.png} & 
         \includegraphics[trim=2 0 0 2,clip,width=0.2\columnwidth]{supplementary_resources/bair/ours/119/00006.png} & 
         \includegraphics[trim=2 0 0 2,clip,width=0.2\columnwidth]{supplementary_resources/bair/ours/119/00009.png} & 
         \includegraphics[trim=2 0 0 2,clip,width=0.2\columnwidth]{supplementary_resources/bair/ours/119/00012.png} & 
         \includegraphics[trim=2 0 0 2,clip,width=0.2\columnwidth]{supplementary_resources/bair/ours/119/00015.png} & 
         \includegraphics[trim=2 0 0 2,clip,width=0.2\columnwidth]{supplementary_resources/bair/ours/119/00018.png} & 
         \includegraphics[trim=2 0 0 2,clip,width=0.2\columnwidth]{supplementary_resources/bair/ours/119/00021.png} & 
         \includegraphics[trim=2 0 0 2,clip,width=0.2\columnwidth]{supplementary_resources/bair/ours/119/00024.png} & 
         \includegraphics[trim=2 0 0 2,clip,width=0.2\columnwidth]{supplementary_resources/bair/ours/119/00027.png} & 
         \includegraphics[trim=2 0 0 2,clip,width=0.2\columnwidth]{supplementary_resources/bair/ours/119/00029.png} \\

    \end{tabular}
    }
    \captionof{figure}{Reconstructed sequences on the \emph{BAIR} dataset using the learned, discrete actions extracted from the original sequence as inputs.}
    \label{fig:bair_reconstruction_119}
\end{table*}
