# Supplementary material for: Playable Video Generation
Source: arXiv:2101.12195 source file (2021-01-28)
Supplement: Supplementary file 14 [file breakout_density_plots.tex]

\begin{table*}
    \centering
    
    \resizebox{0.43\linewidth}{!}{
    \setlength\tabcolsep{0pt}
    \tiny
    
    \begin{tabular}{l@{\hskip 0.7mm}ccc}
         & Action 1 & Action 2 & Action 3  \\

         \rotatebox{90}{\hspace{0mm}\scalebox{1}{MoCoGAN \cite{tulyakov2018moco}}} &
         \includegraphics[trim=60 80 60 80,clip,width=0.2\columnwidth]{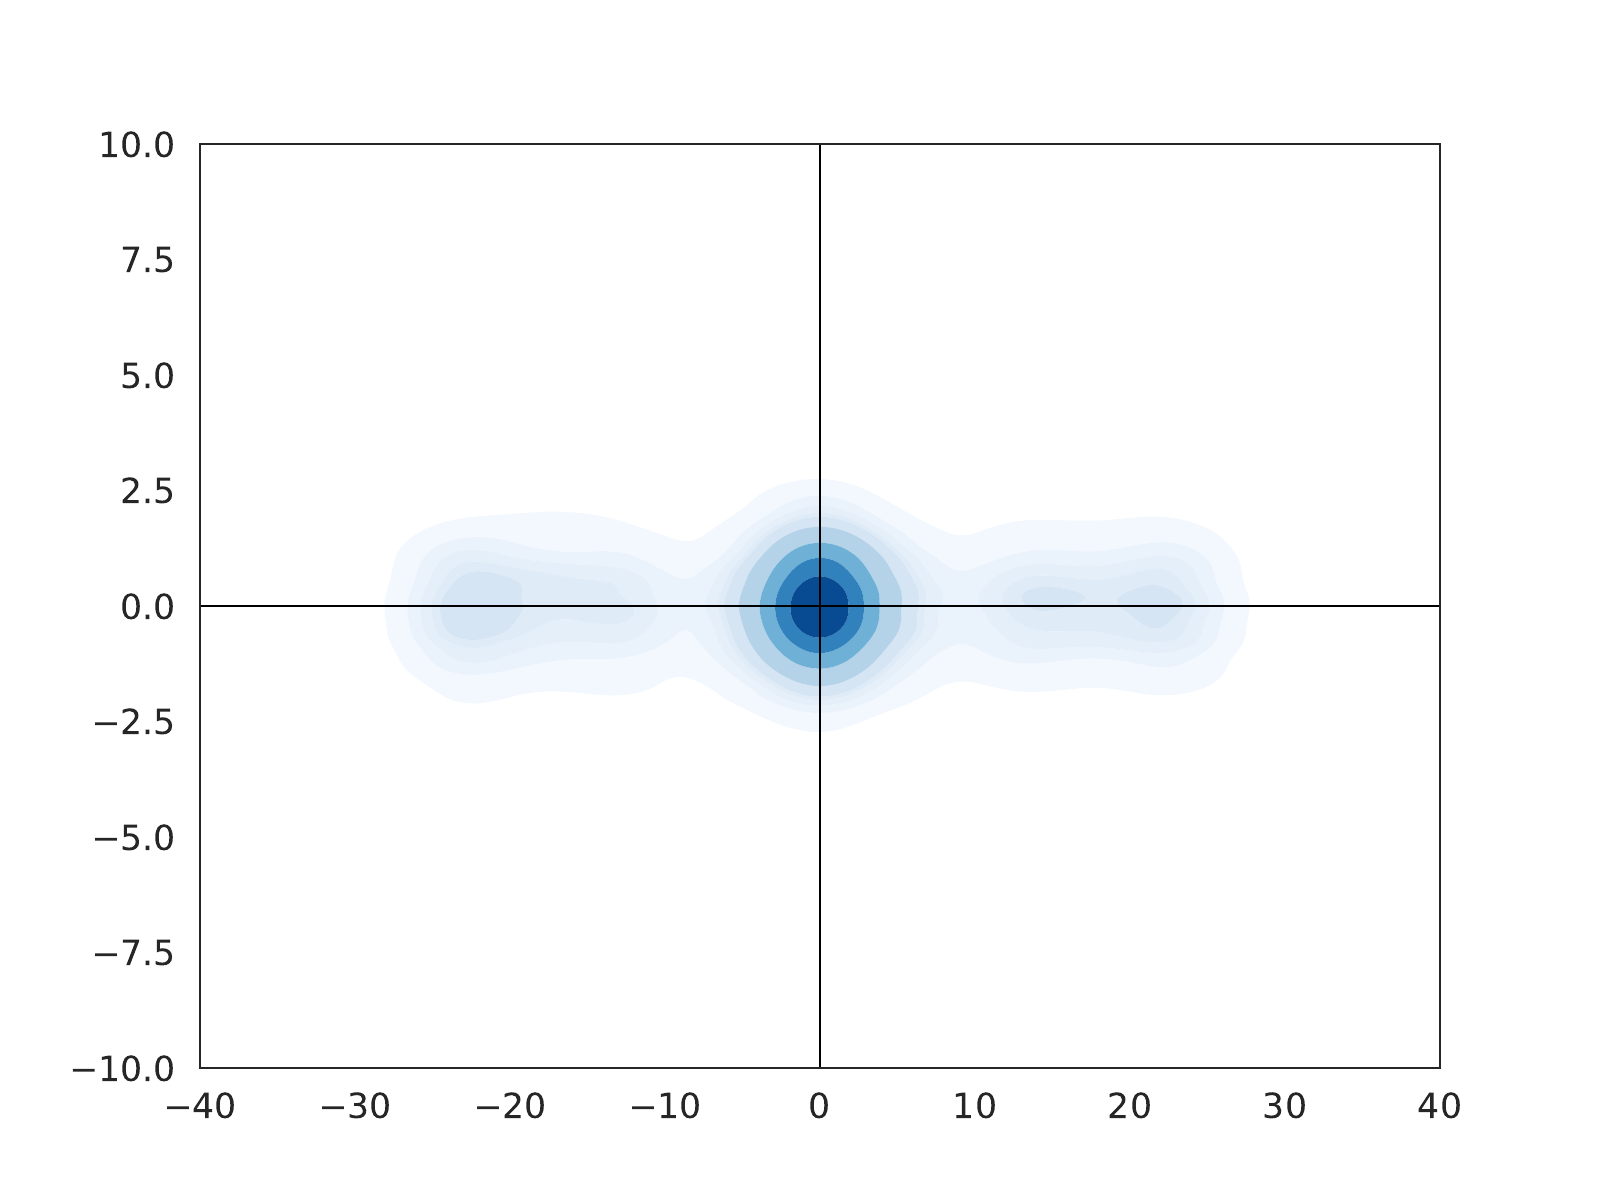} &
         \includegraphics[trim=60 80 60 80,clip,width=0.2\columnwidth]{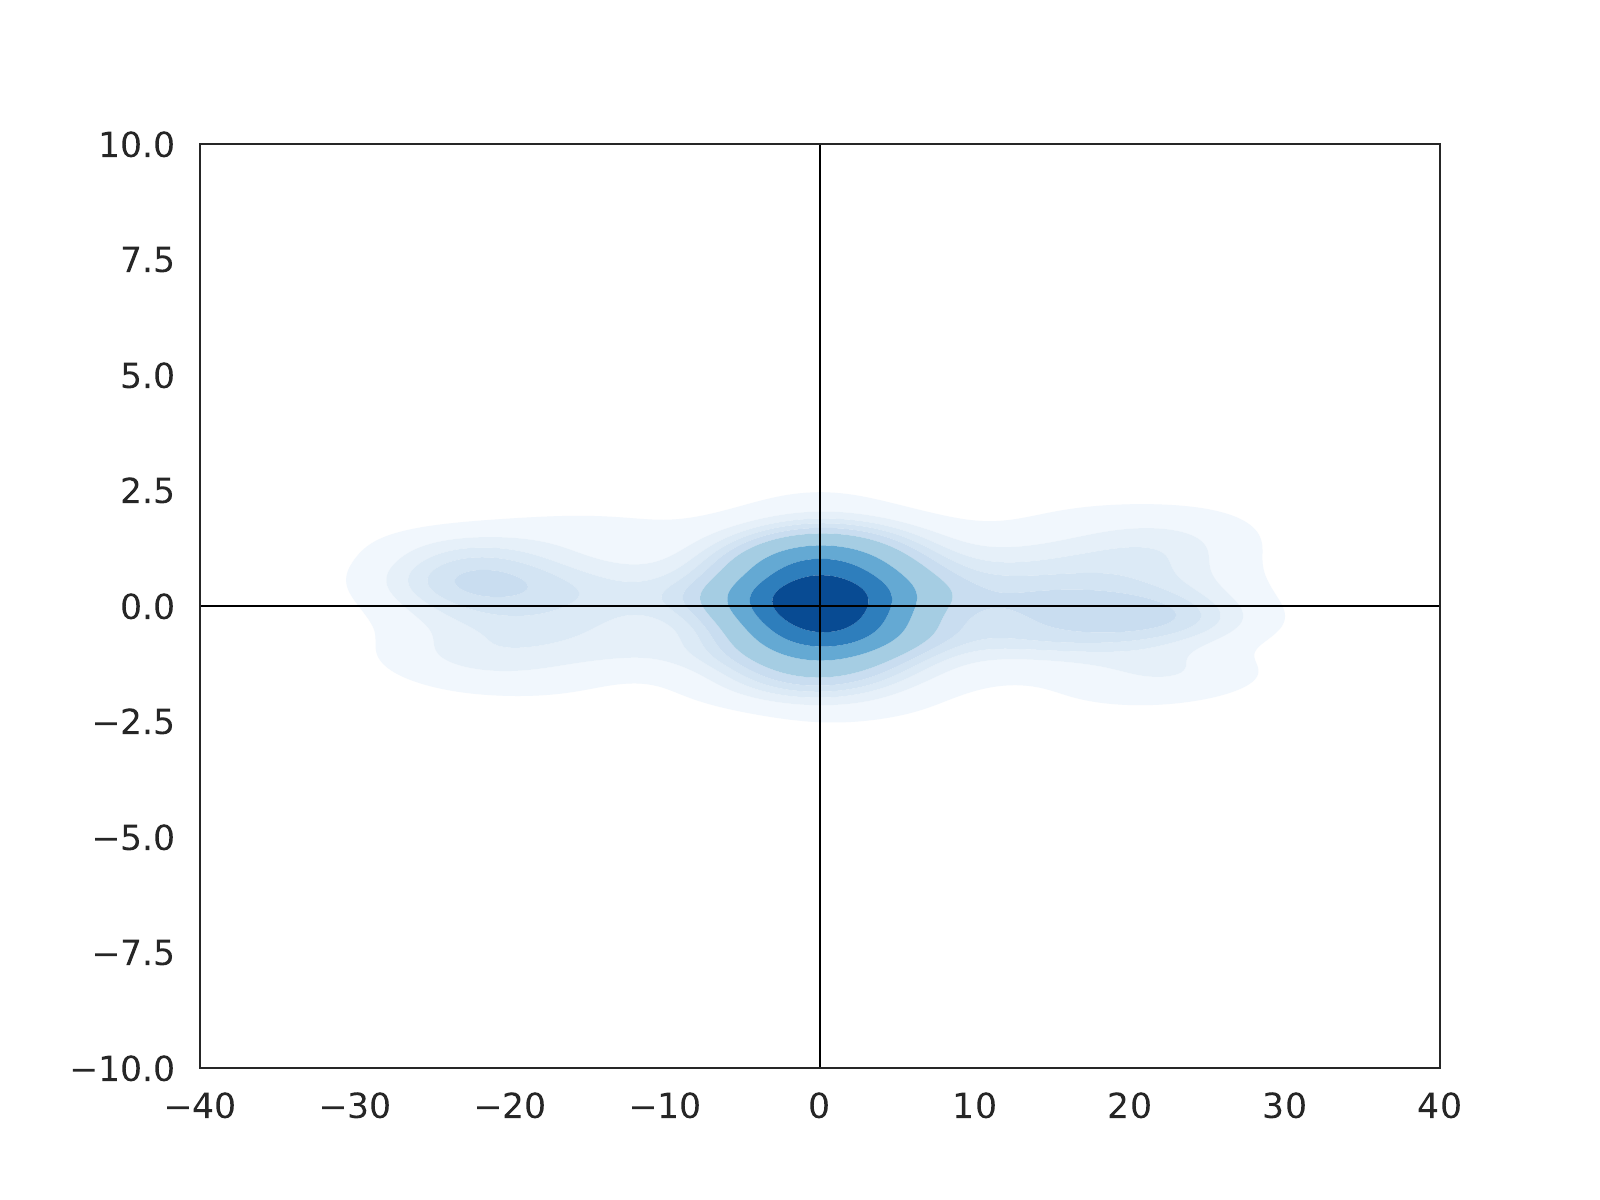} &
         \includegraphics[trim=60 80 60 80,clip,width=0.2\columnwidth]{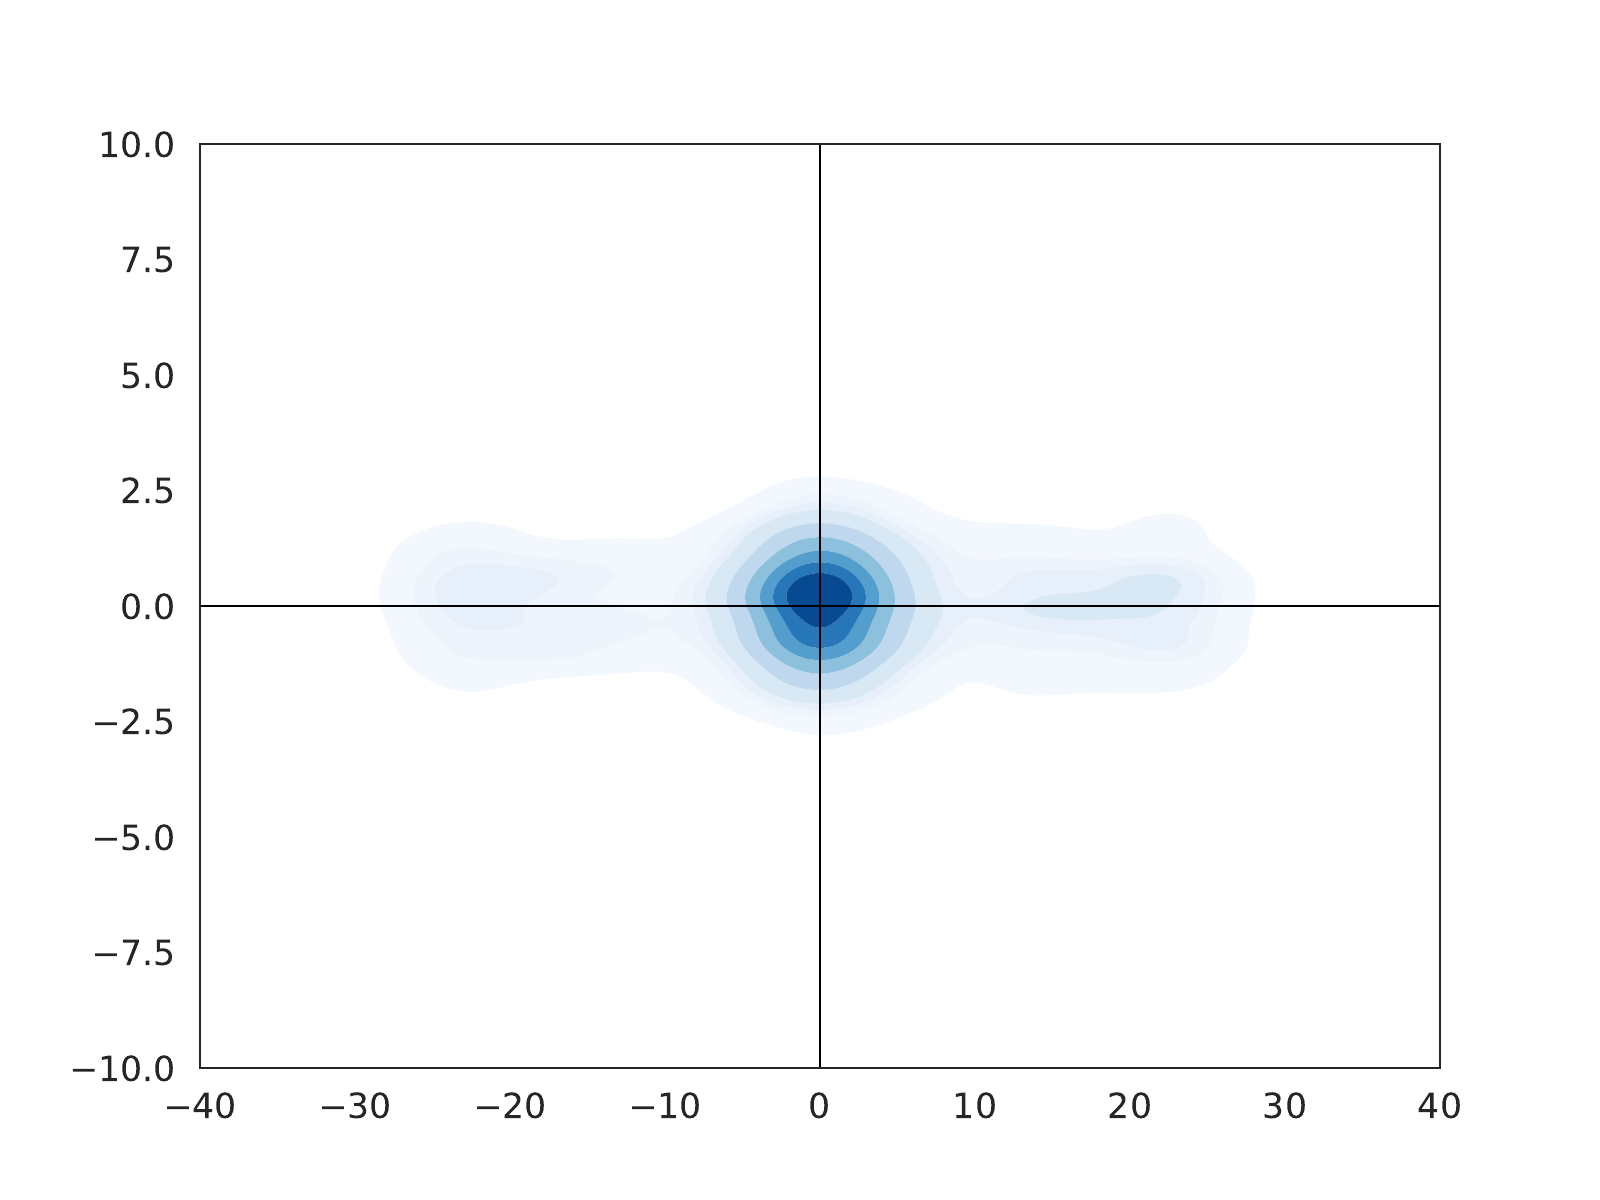} \\
         
         \rotatebox{90}{\hspace{0mm}\scalebox{1}{MoCoGAN+}} &
         \includegraphics[trim=60 80 60 80,clip,width=0.2\columnwidth]{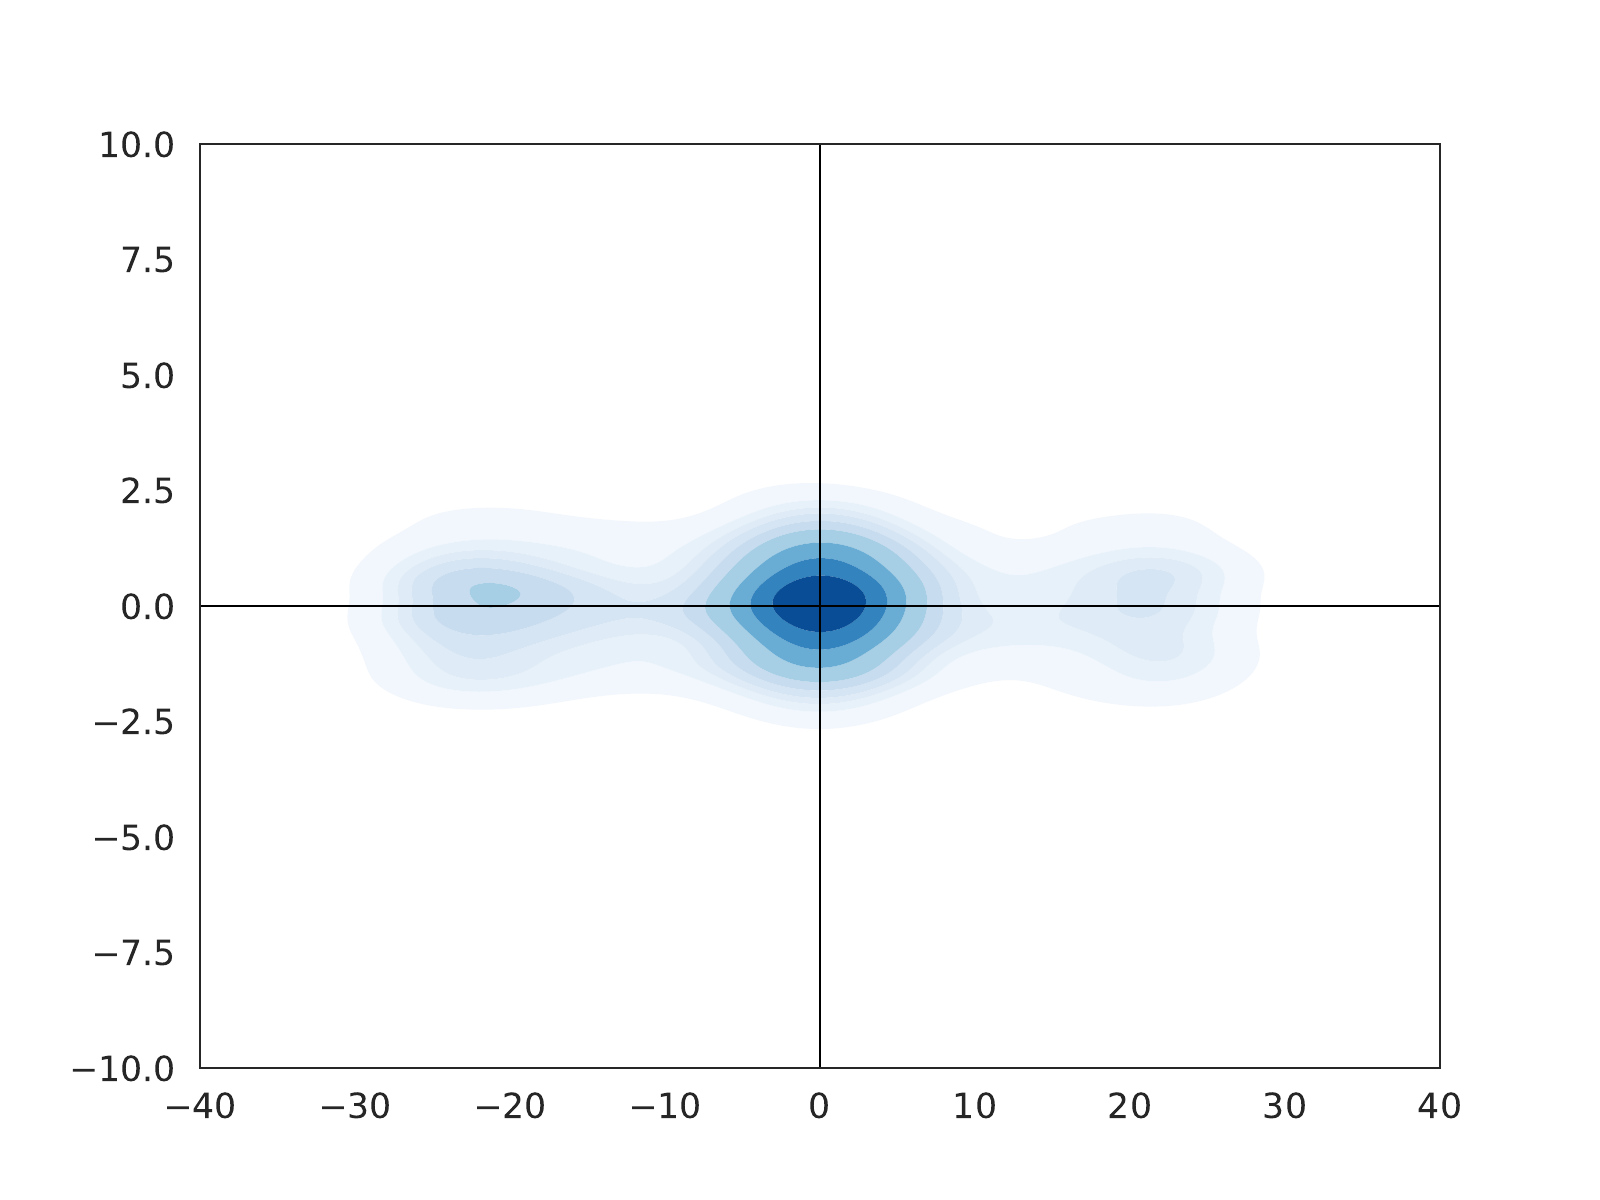} &
         \includegraphics[trim=60 80 60 80,clip,width=0.2\columnwidth]{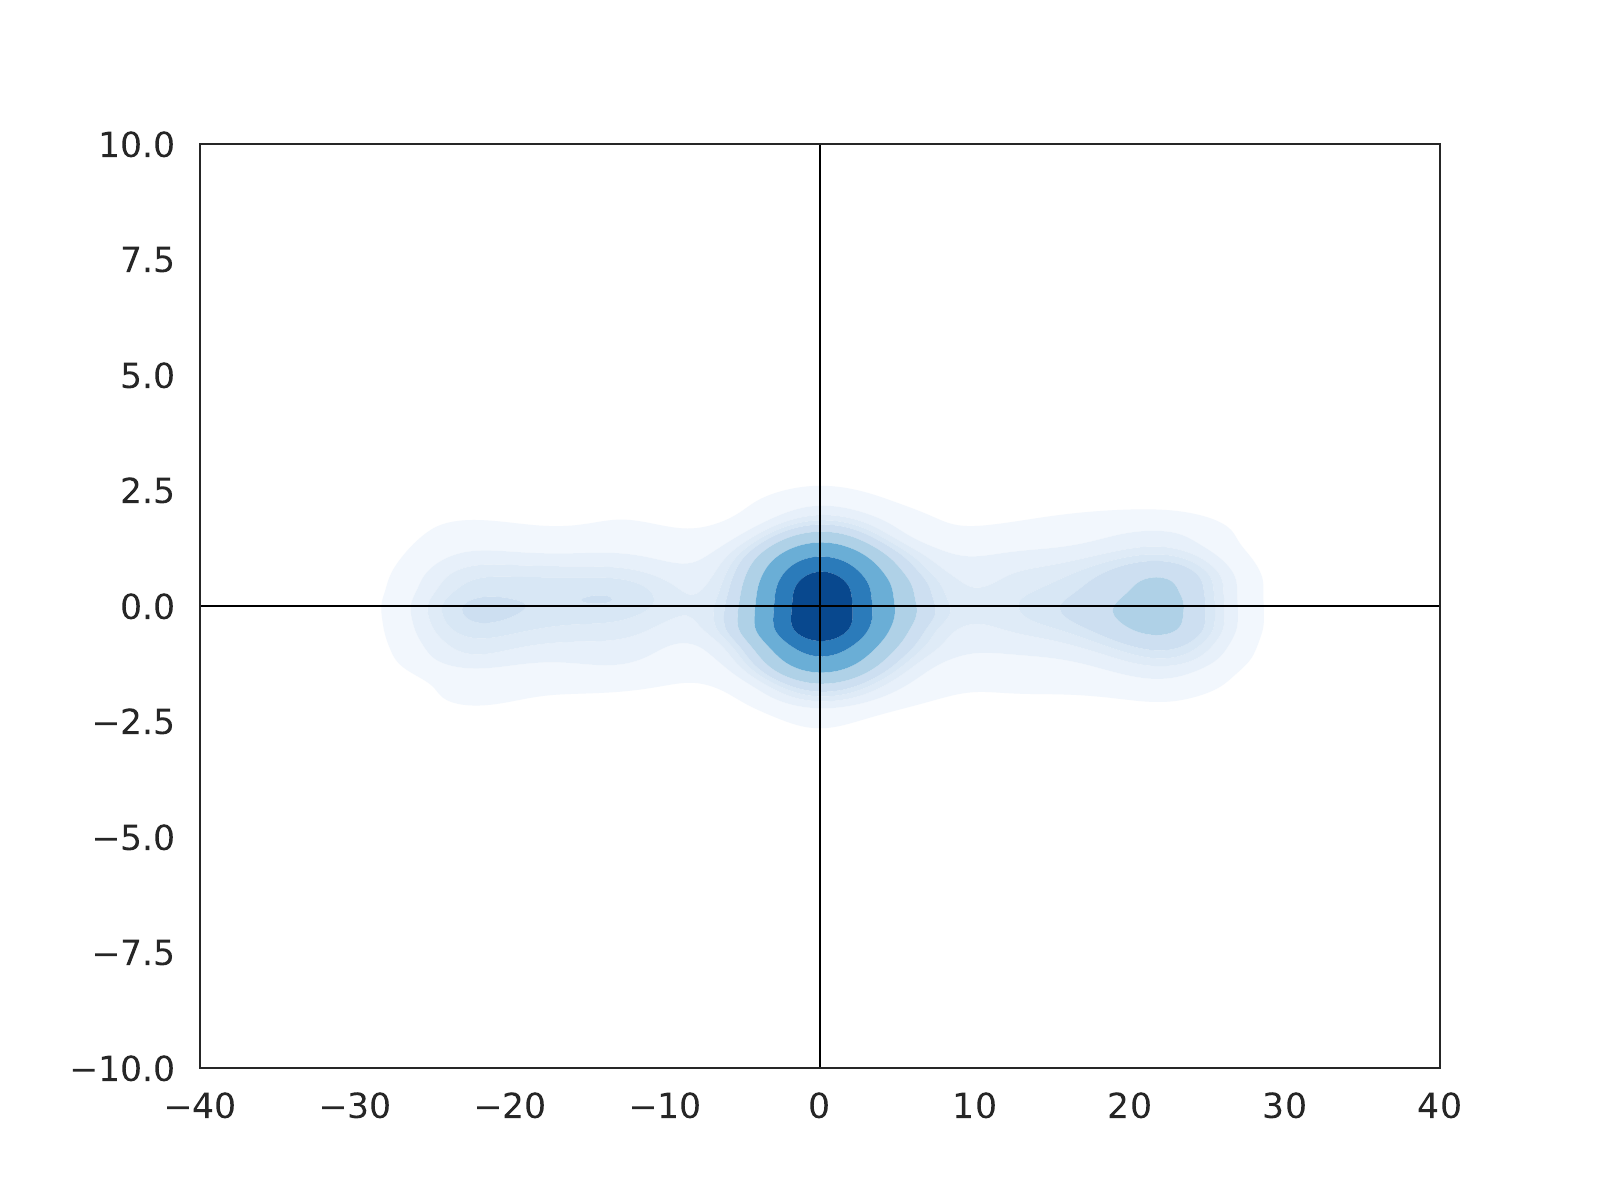} &
         \includegraphics[trim=60 80 60 80,clip,width=0.2\columnwidth]{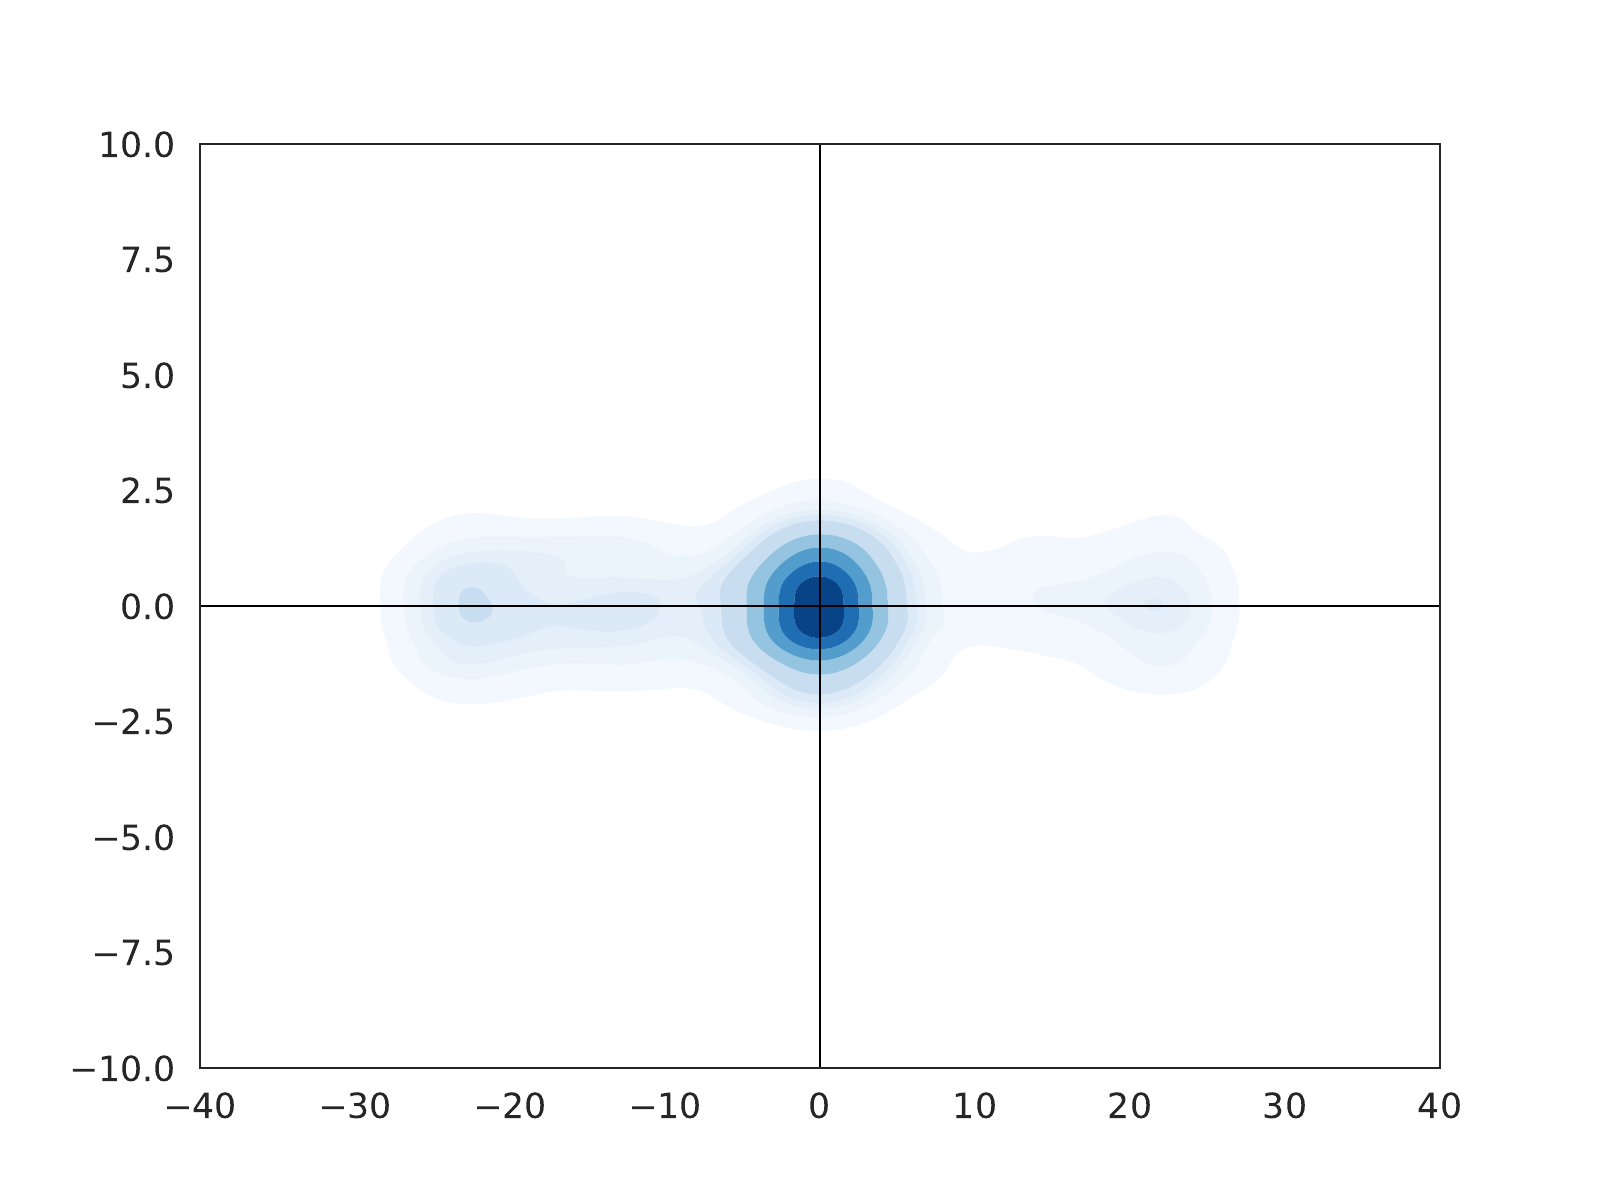} \\
         
         \rotatebox{90}{\hspace{1.8mm}SAVP\cite{lee2018savp}} &
         \includegraphics[trim=60 80 60 80,clip,width=0.2\columnwidth]{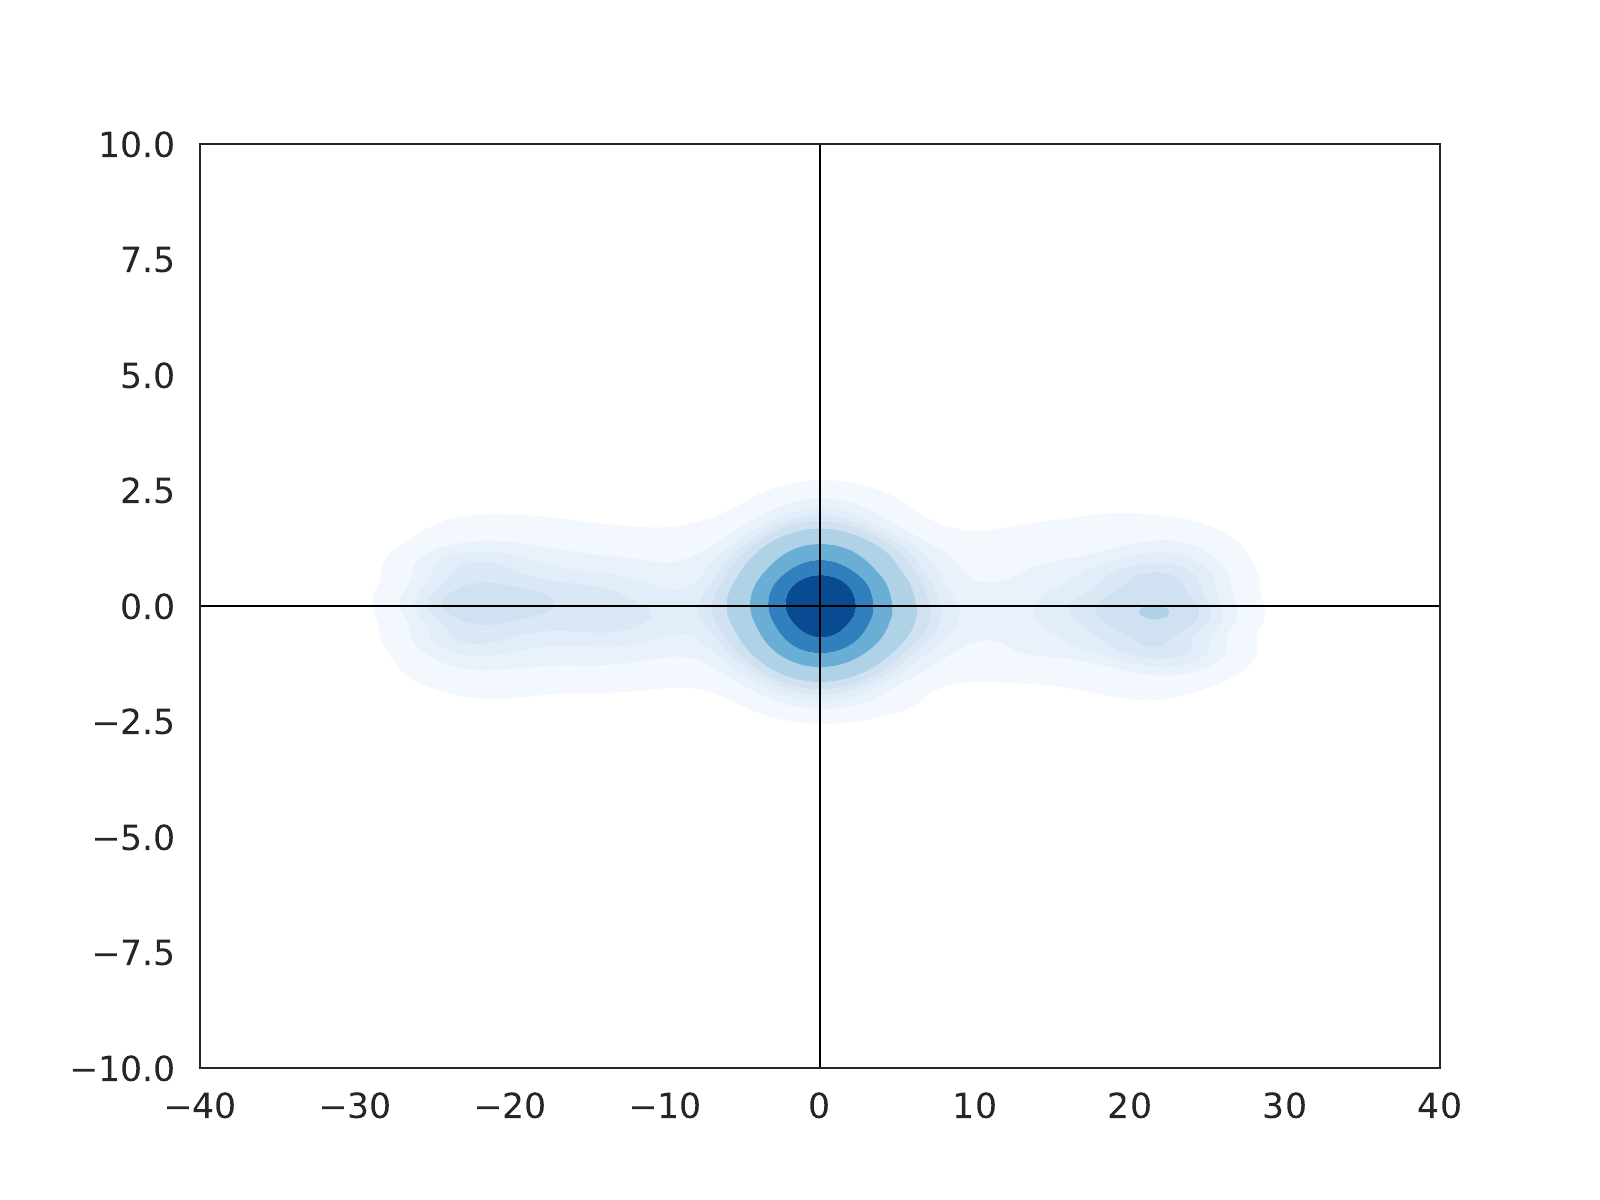} &
         \includegraphics[trim=60 80 60 80,clip,width=0.2\columnwidth]{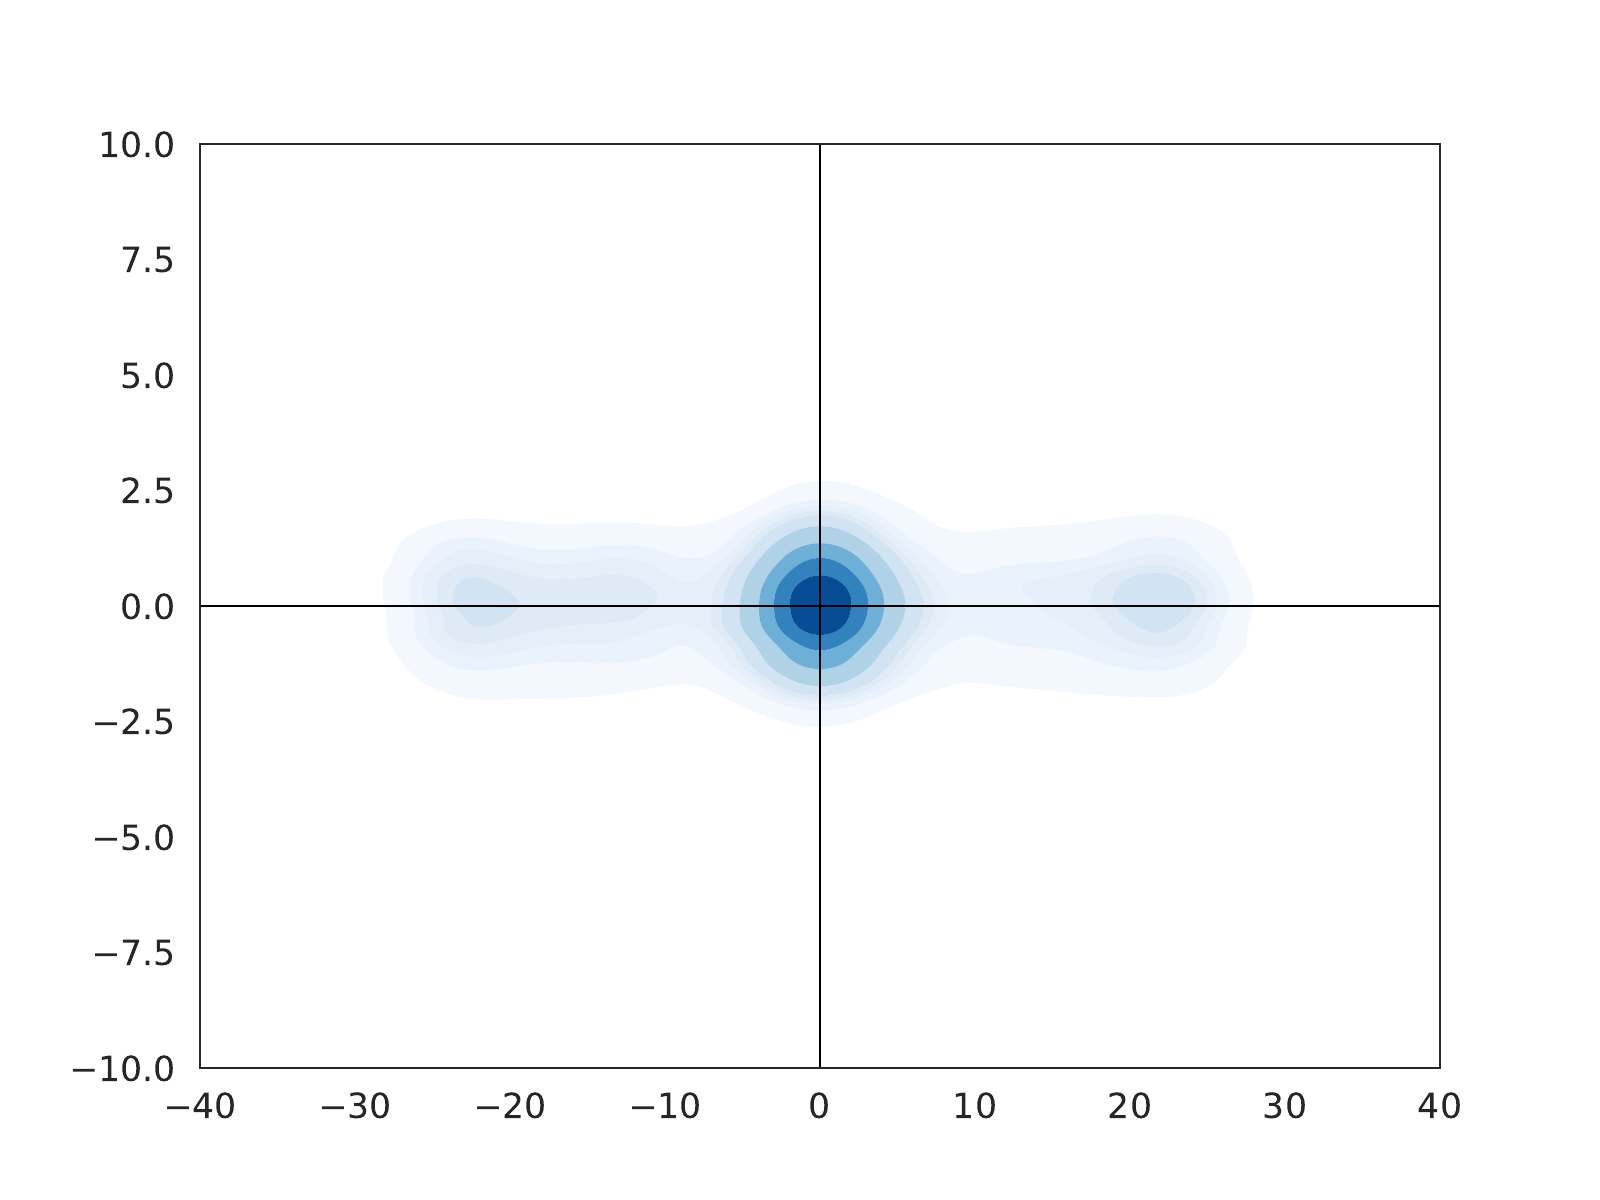} &
         \includegraphics[trim=60 80 60 80,clip,width=0.2\columnwidth]{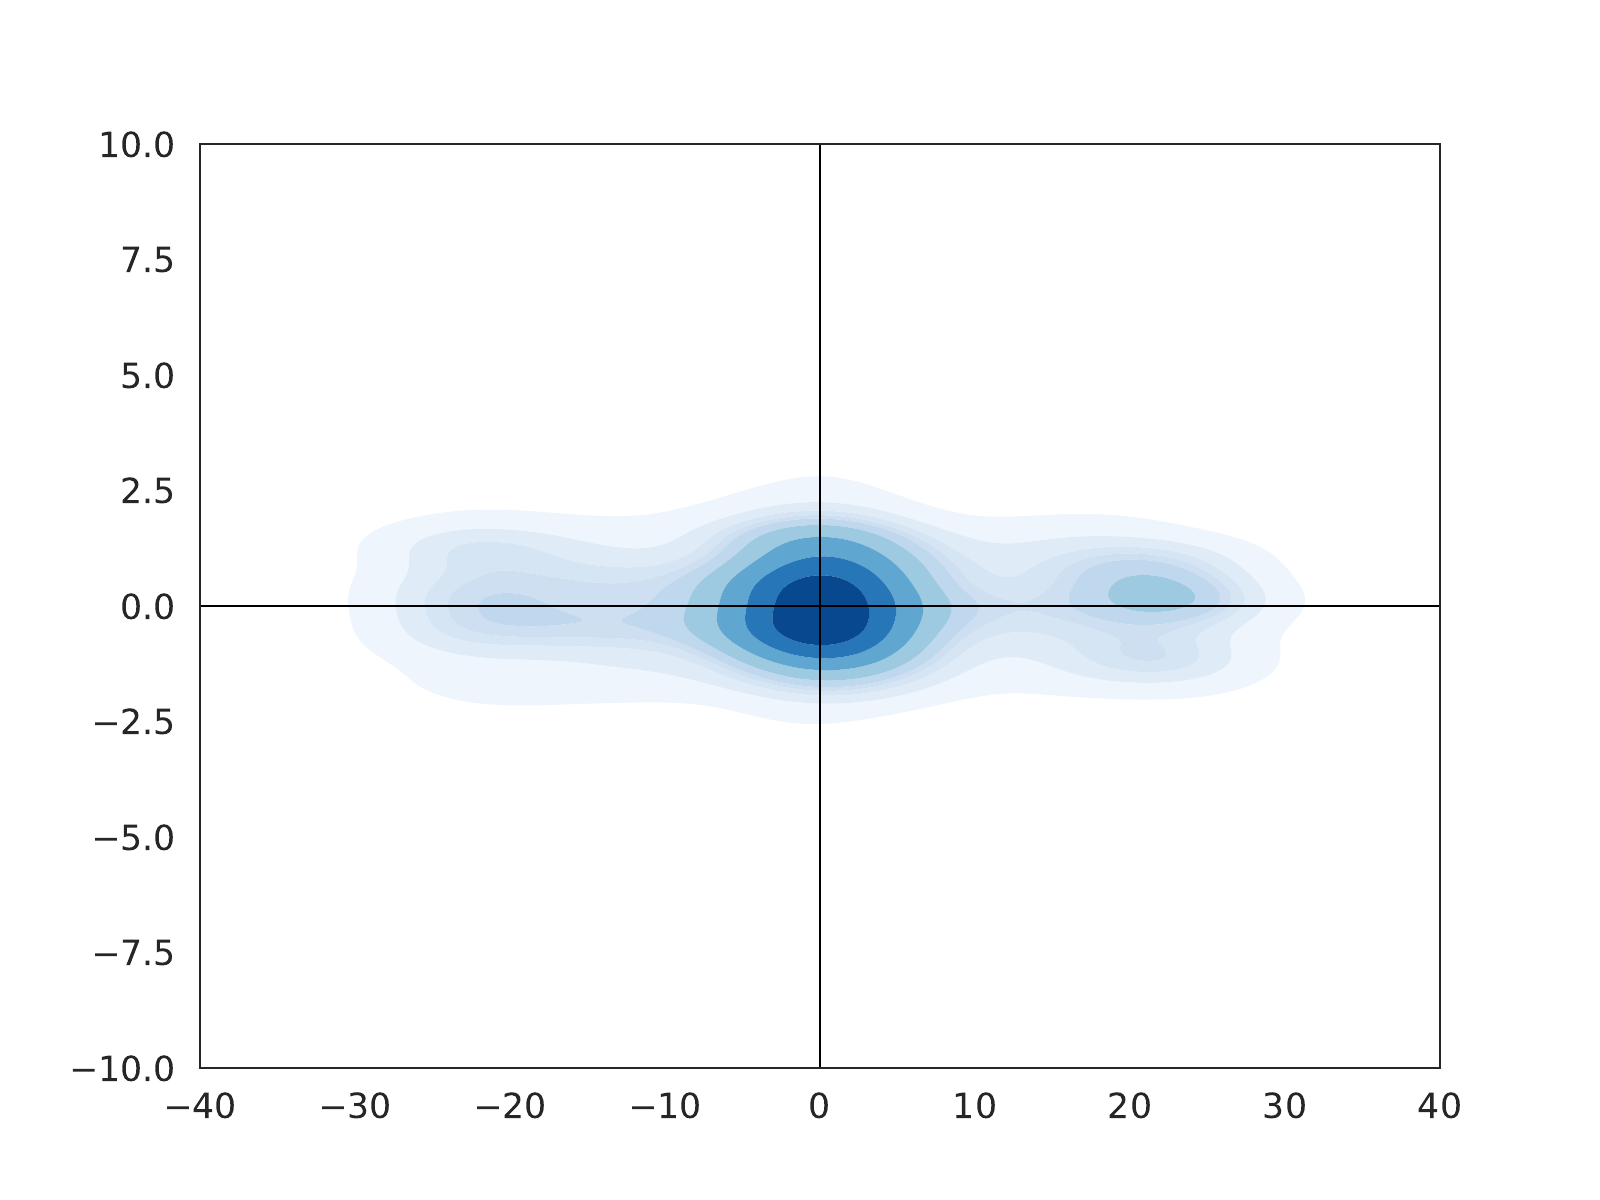} \\
         
         \rotatebox{90}{\hspace{2.5mm}SAVP+} &
         \includegraphics[trim=60 80 60 80,clip,width=0.2\columnwidth]{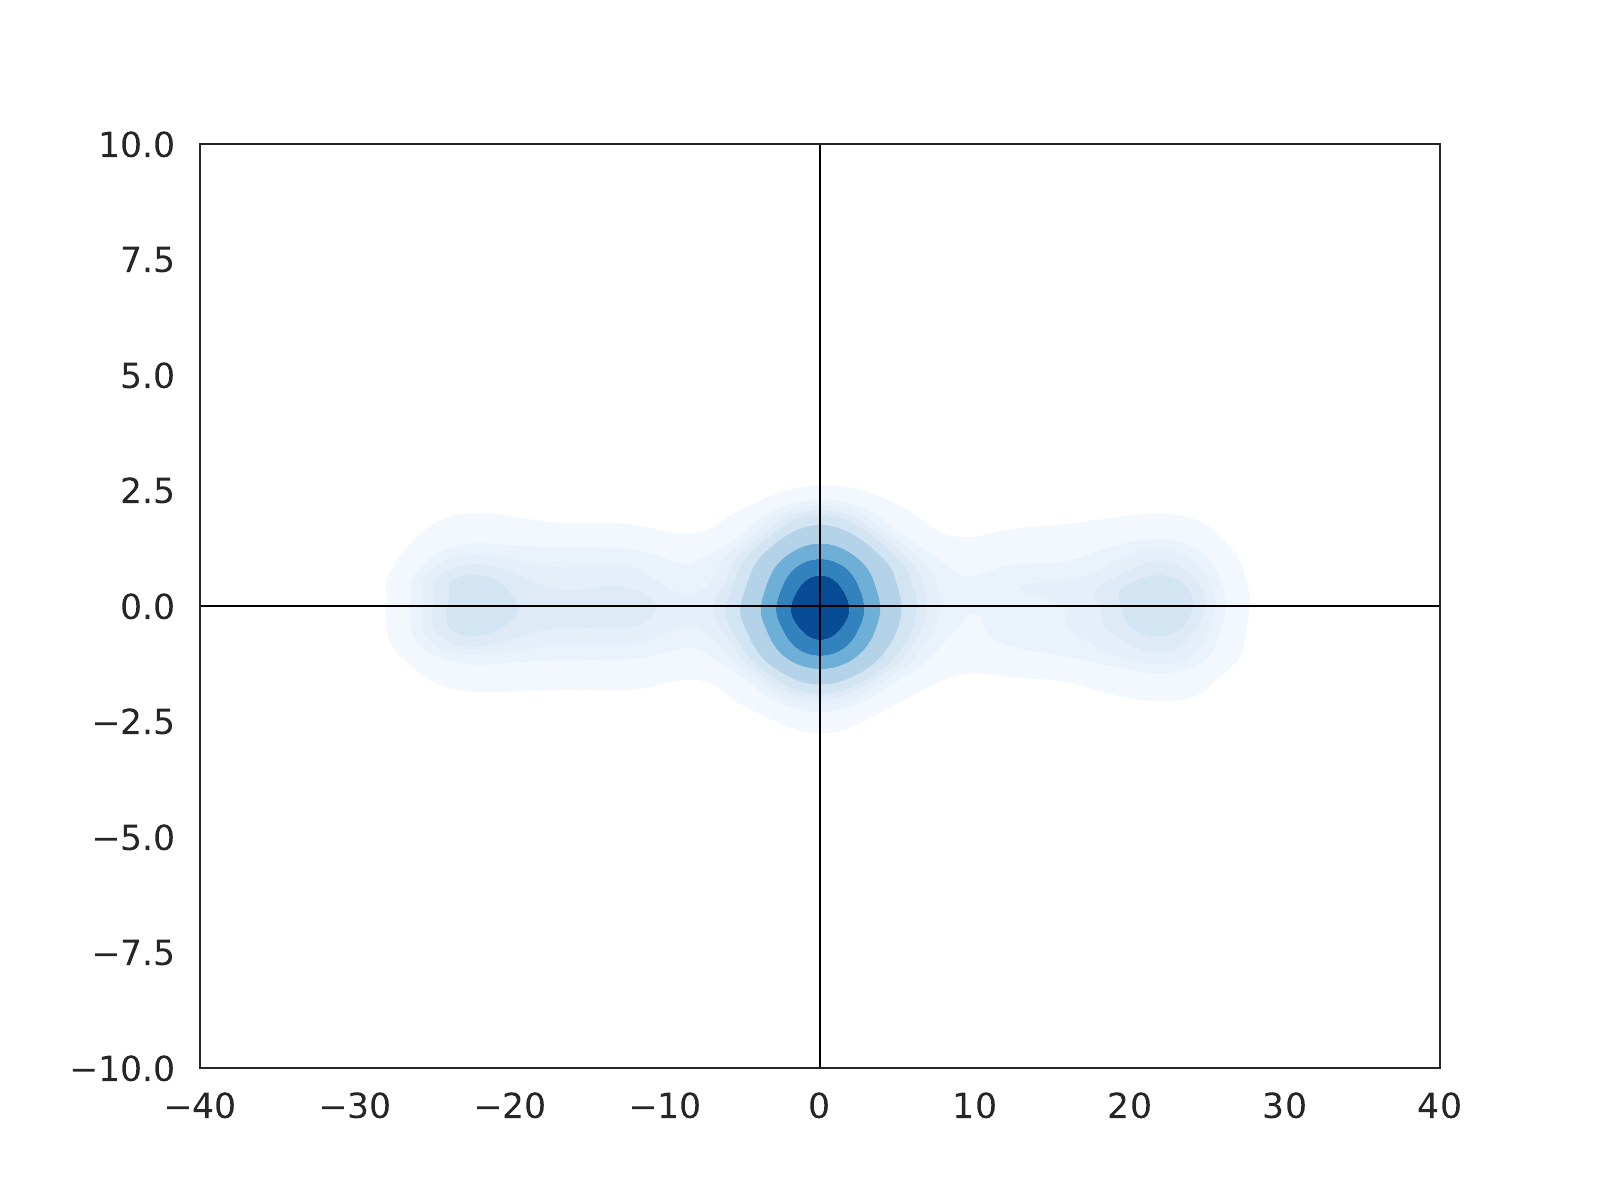} &
         \includegraphics[trim=60 80 60 80,clip,width=0.2\columnwidth]{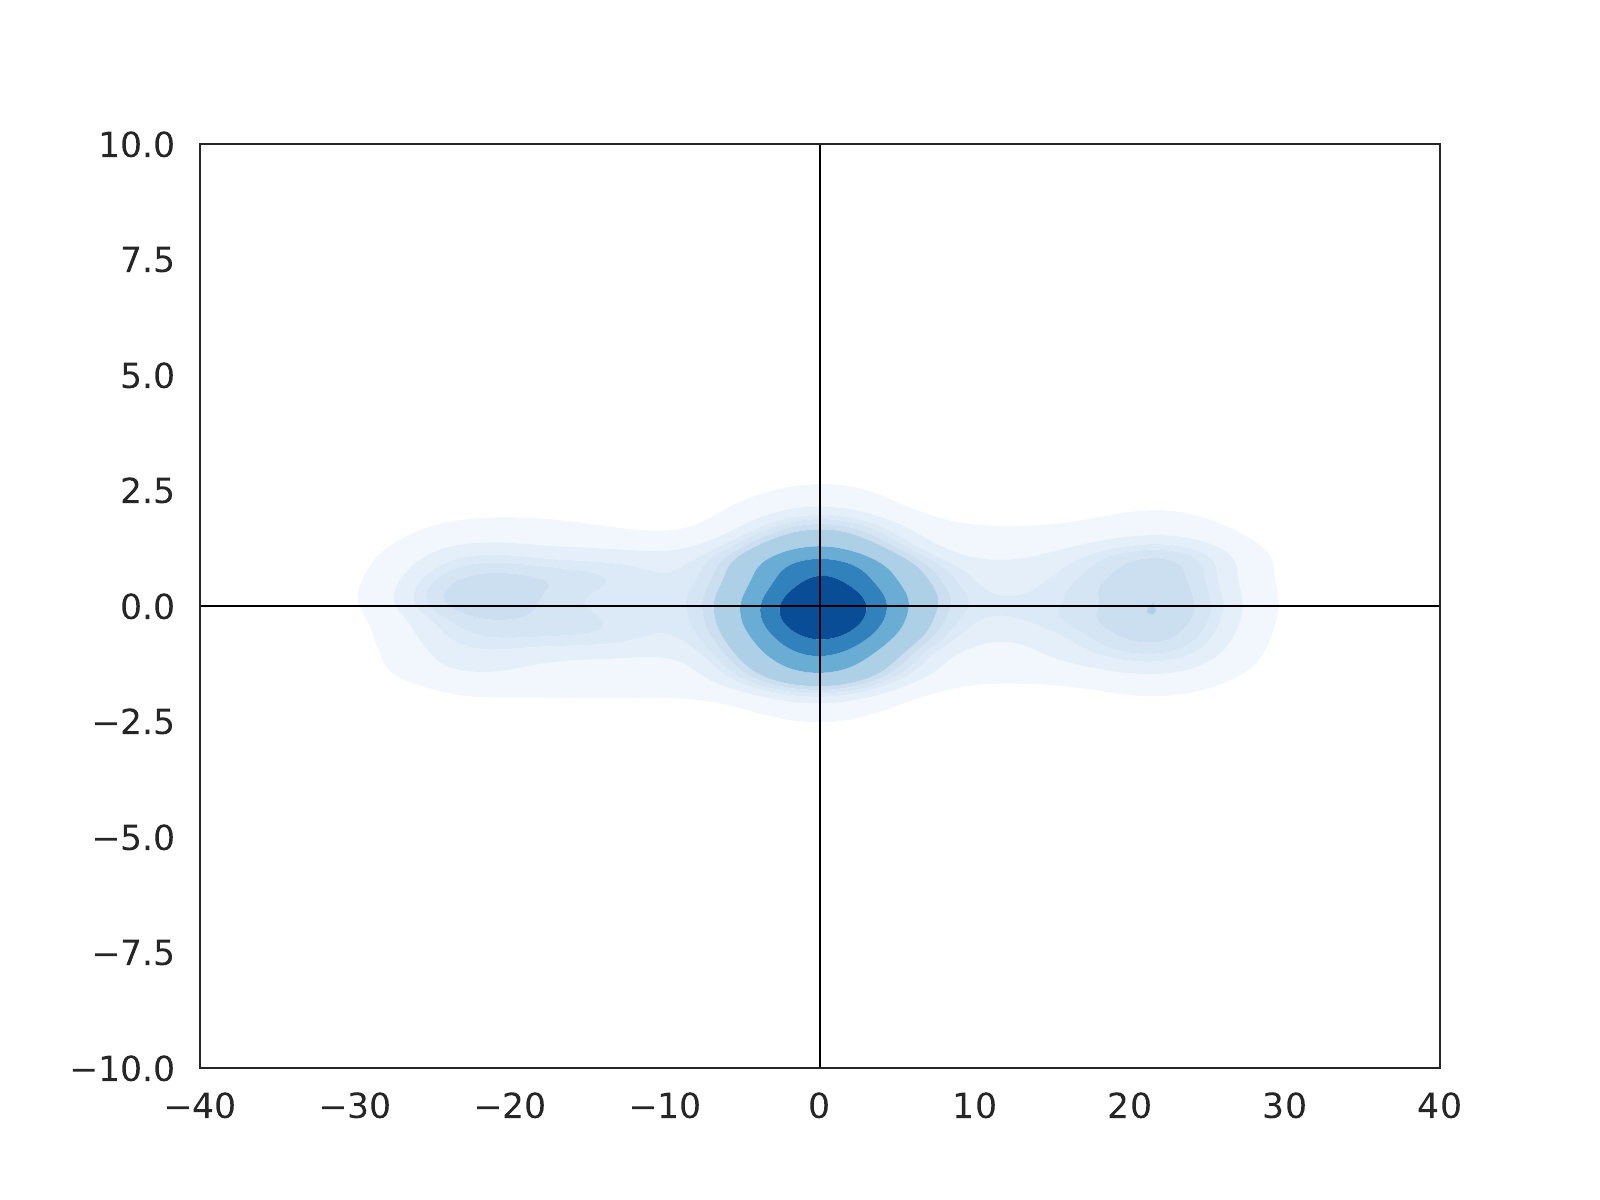} &
         \includegraphics[trim=60 80 60 80,clip,width=0.2\columnwidth]{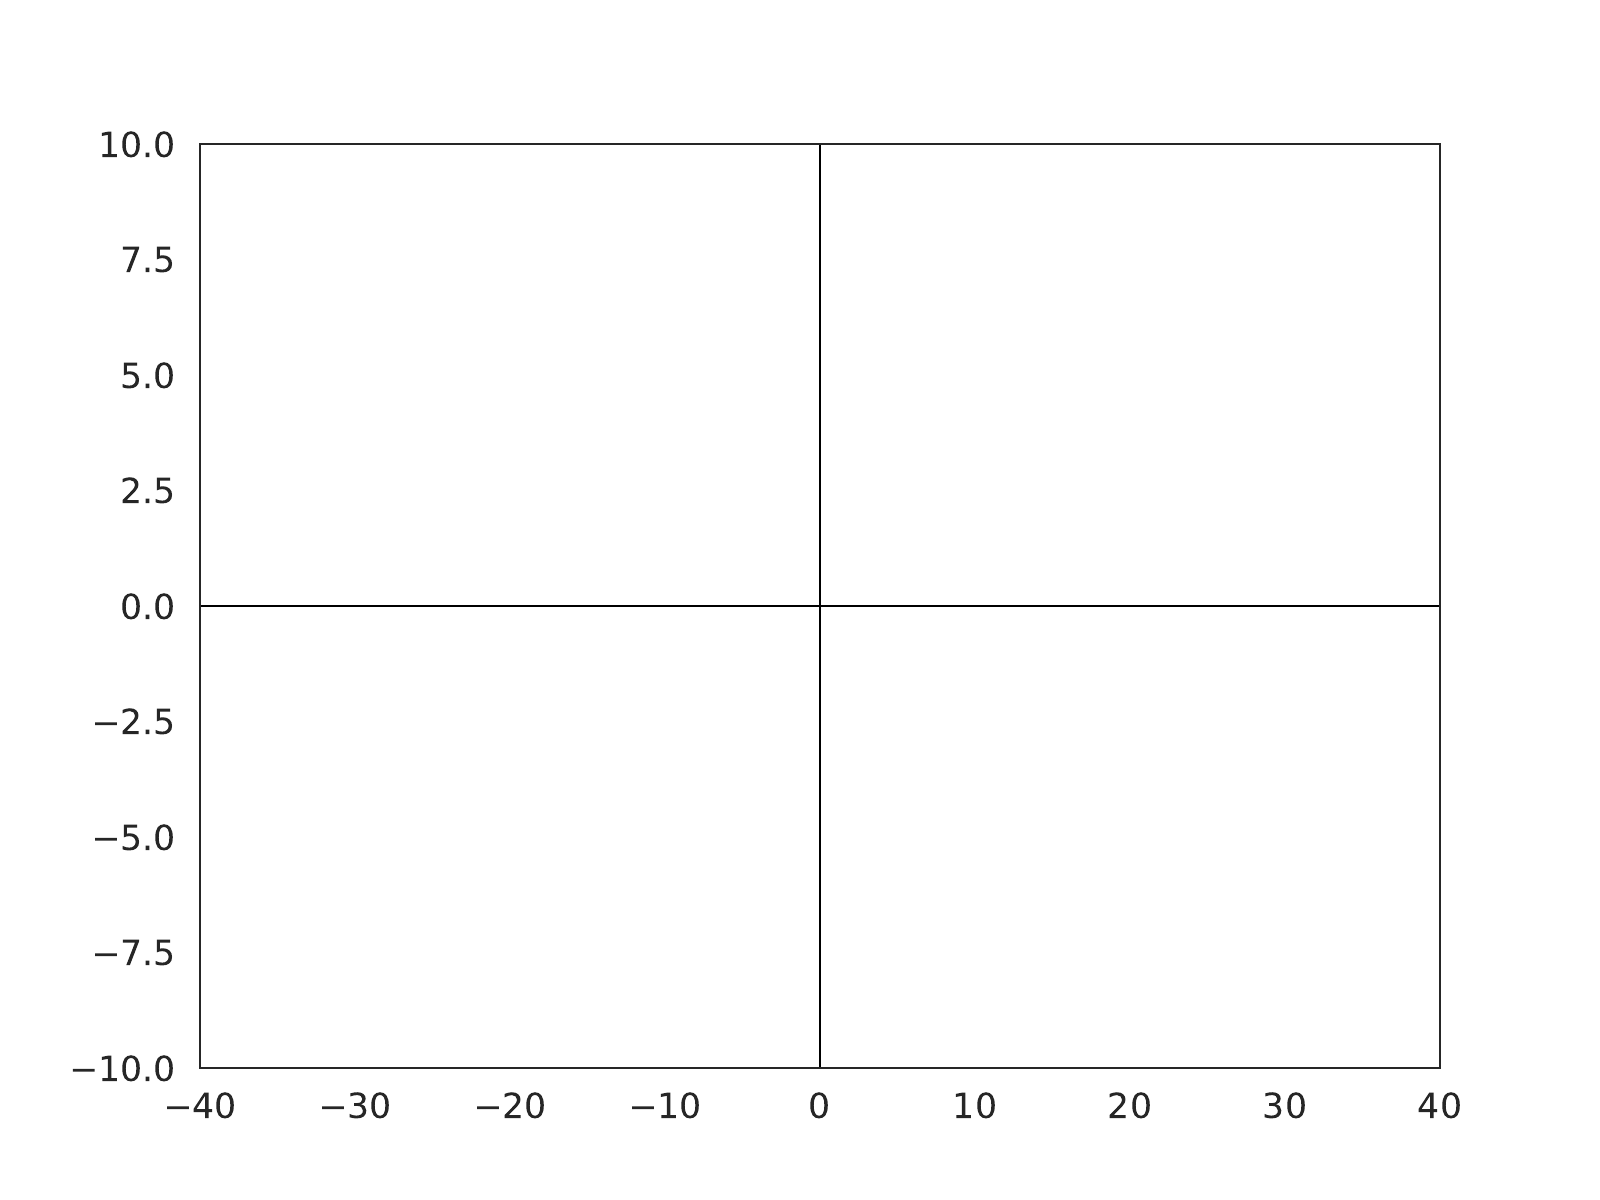} \\
         
         \rotatebox{90}{\hspace{3mm}Ours} &
         \includegraphics[trim=60 80 60 80,clip,width=0.2\columnwidth]{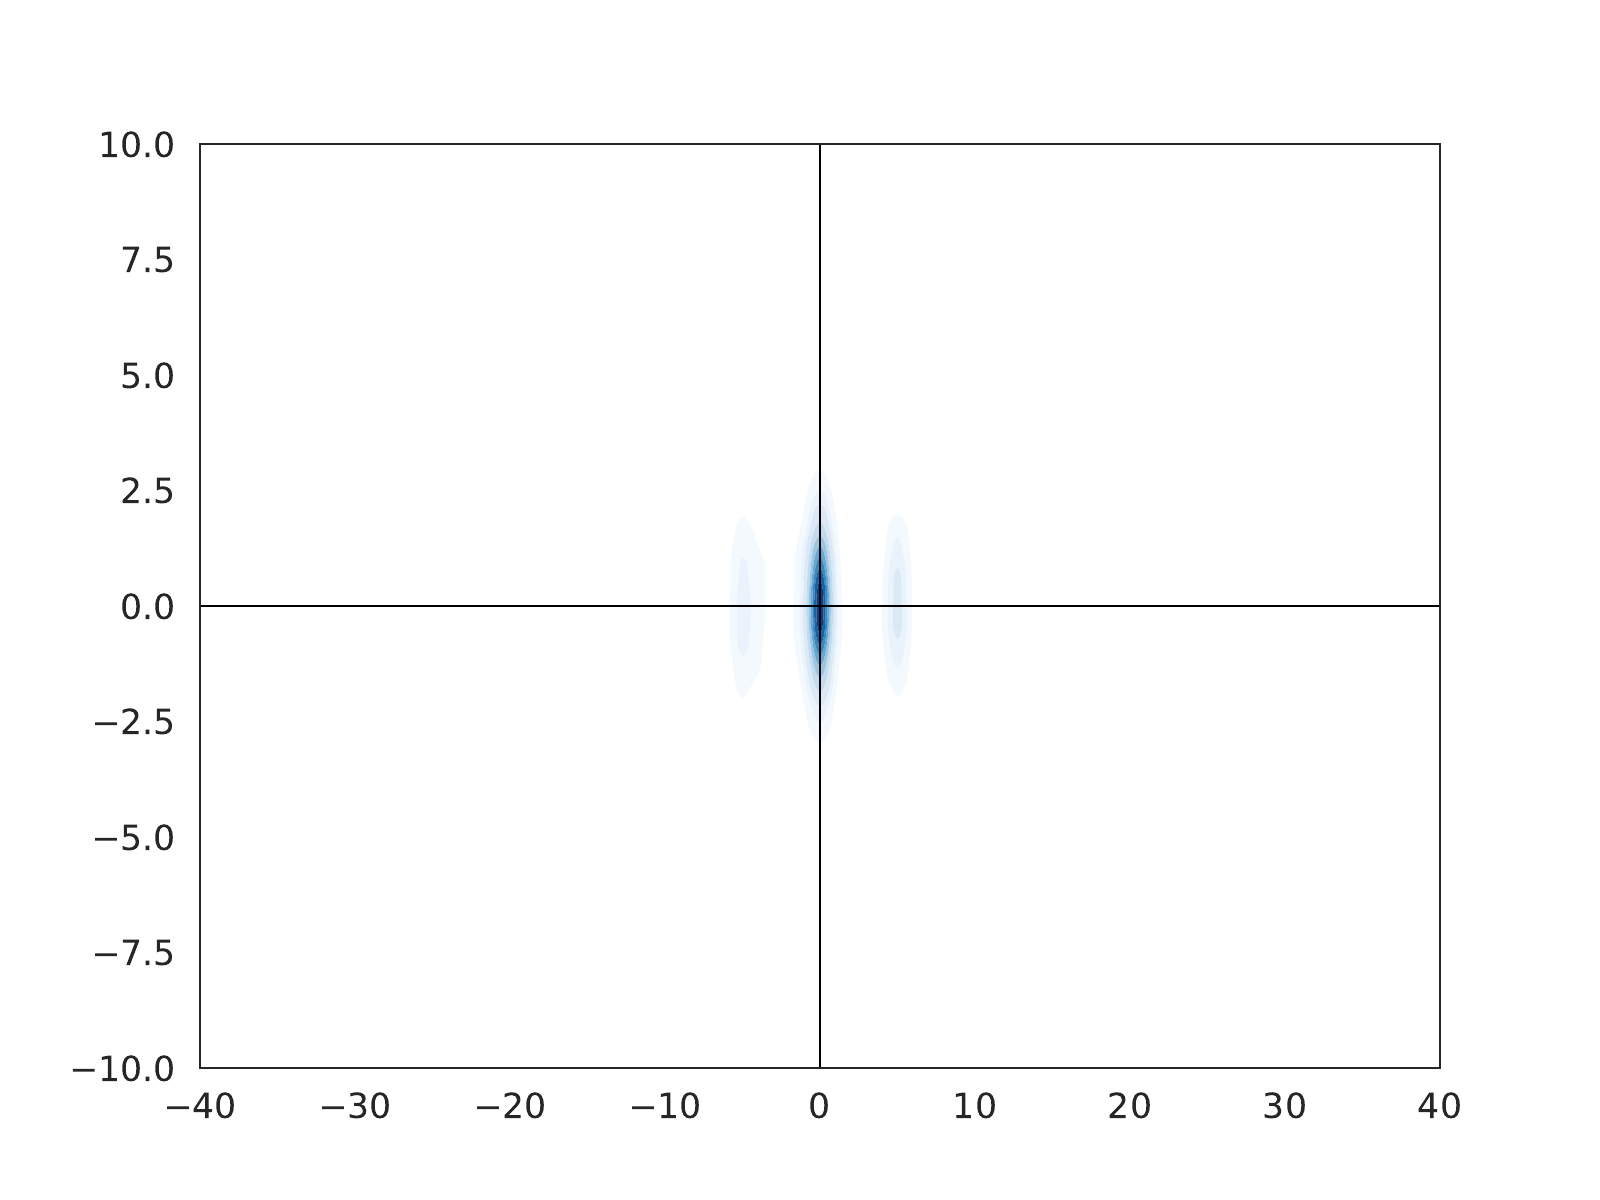} &
         \includegraphics[trim=60 80 60 80,clip,width=0.2\columnwidth]{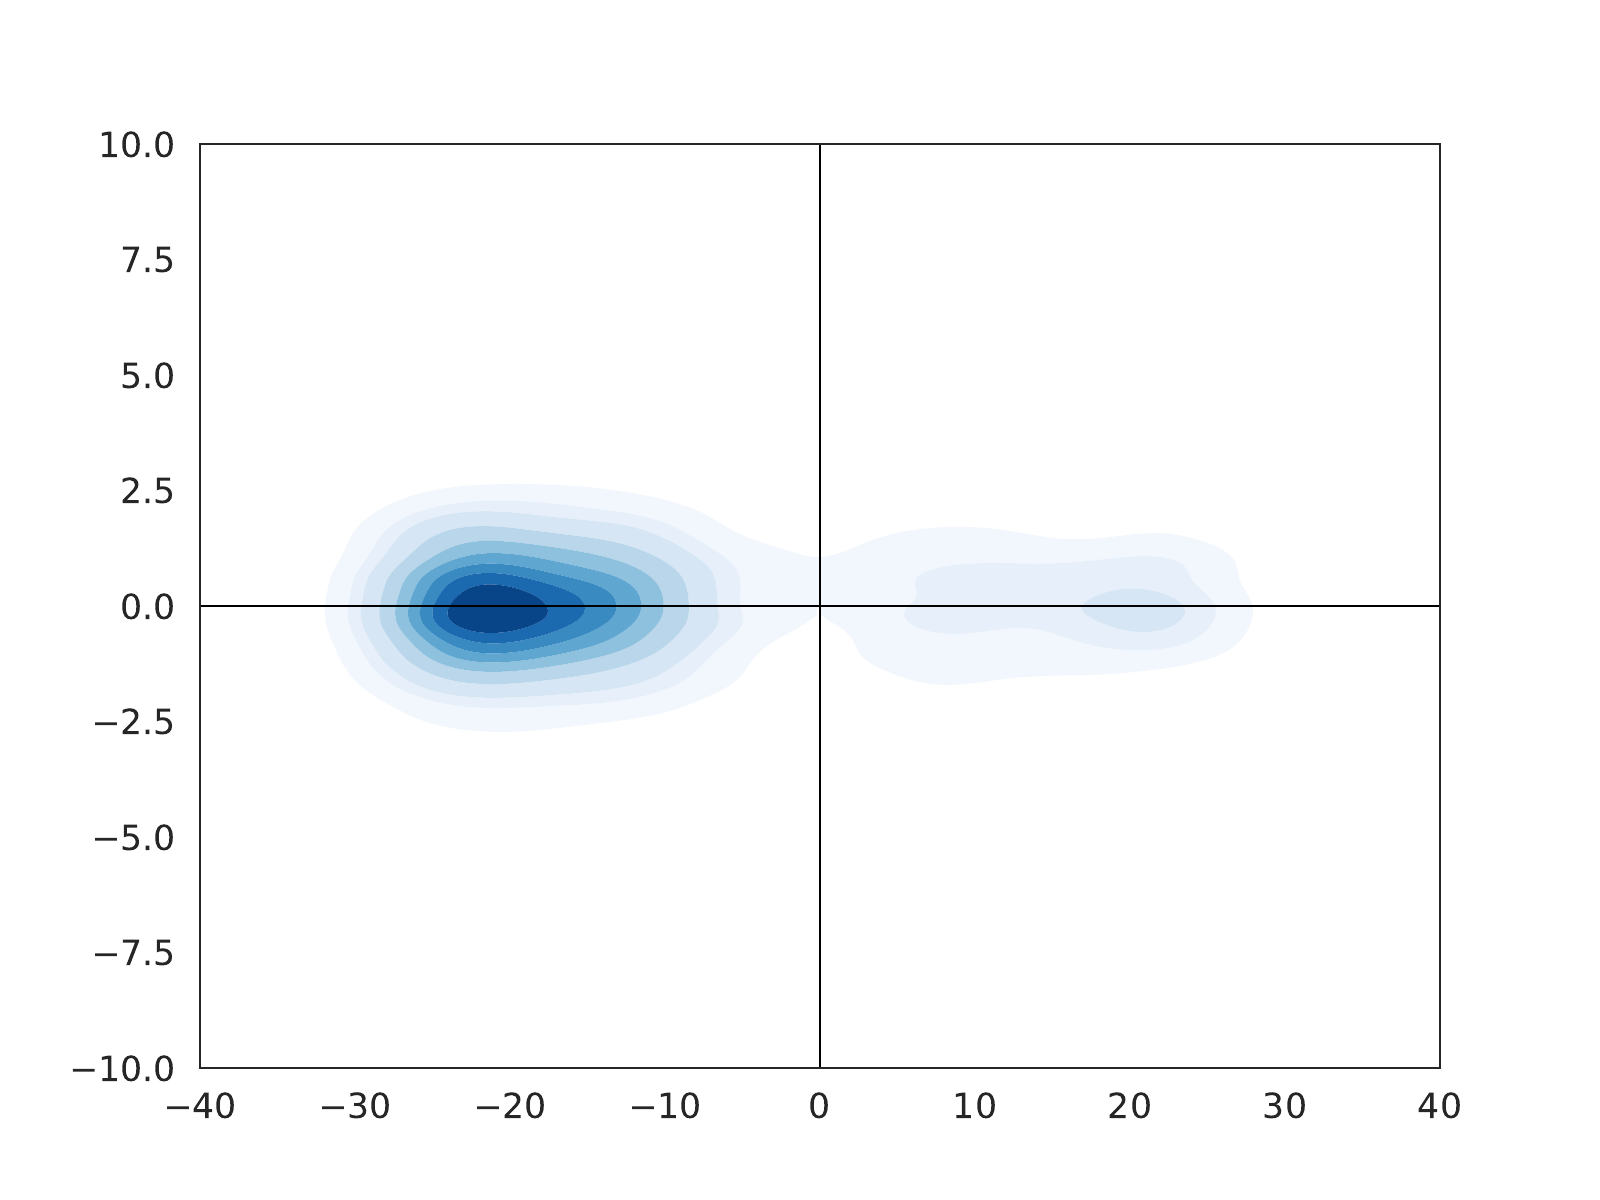} &
         \includegraphics[trim=60 80 60 80,clip,width=0.2\columnwidth]{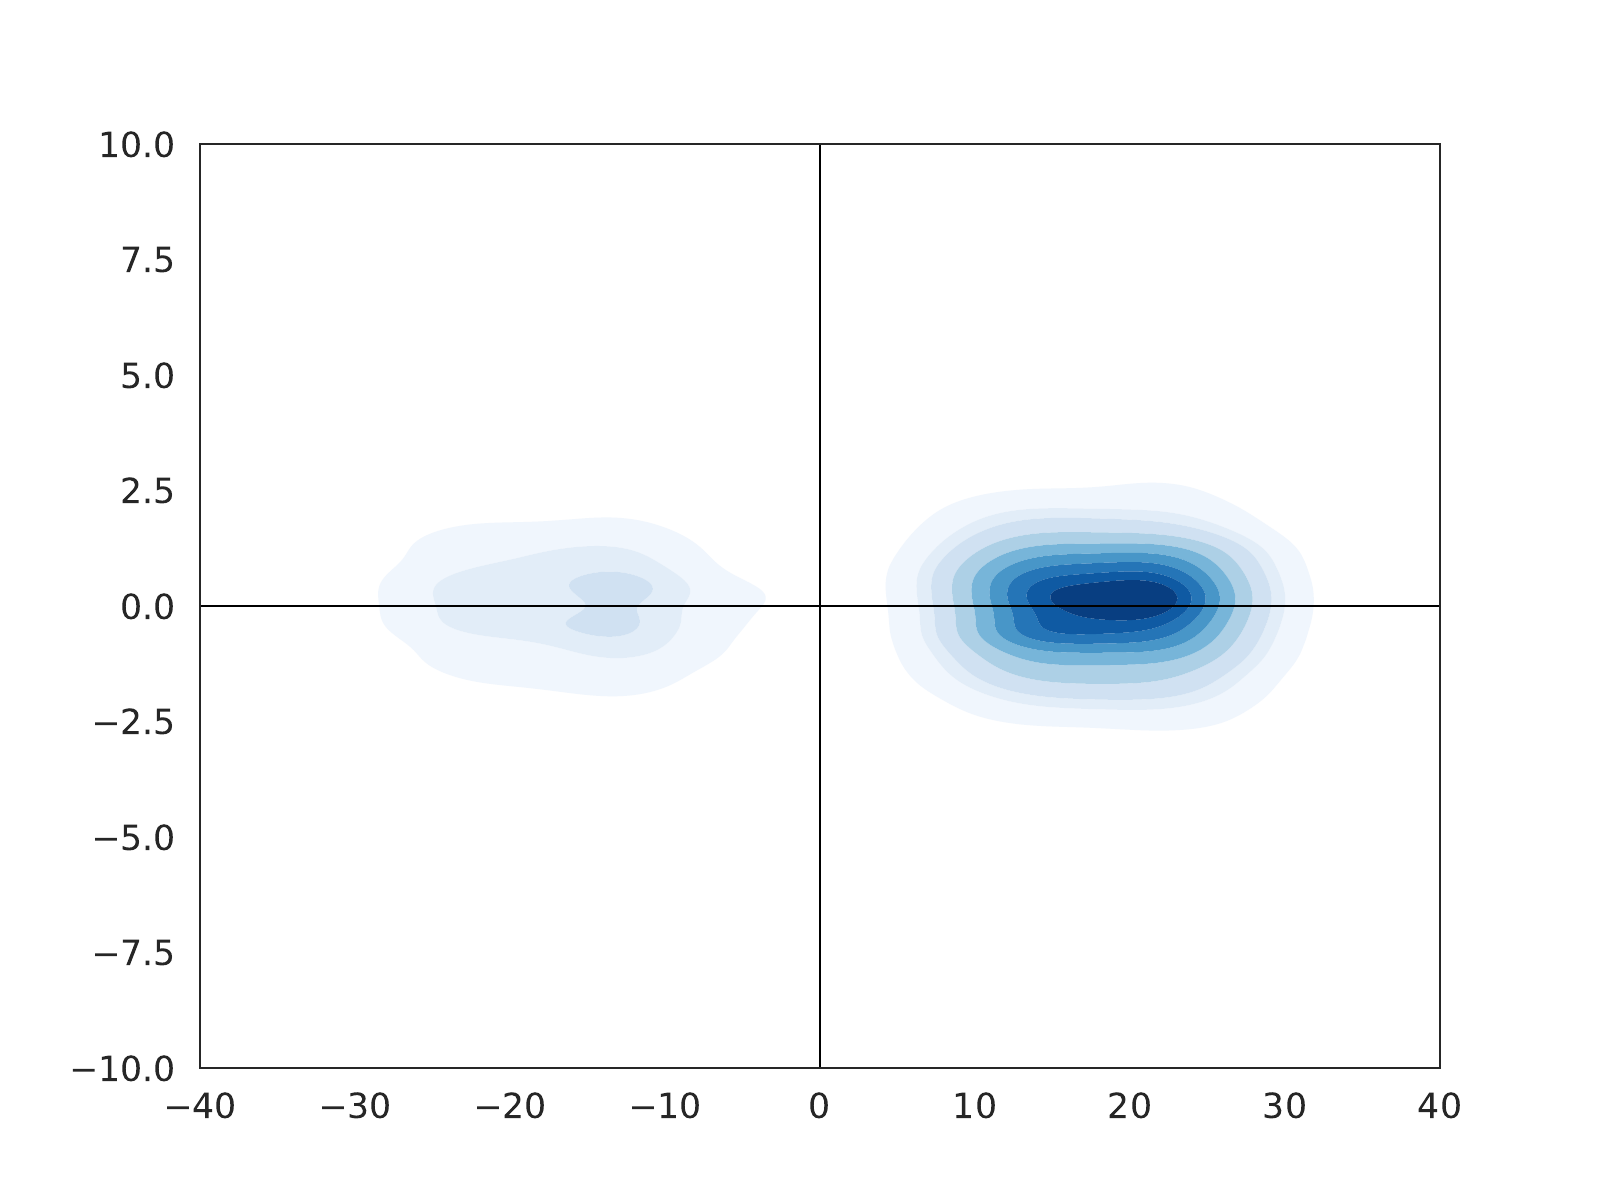} \\

    \end{tabular}
    }
    \captionof{figure}{Distribution of the displacement $\Delta$ associated with the player-controlled platform on the \emph{Atari Breakout} dataset. Ideal distributions are different for each action and have low variance, meaning that they capture specific movements. Differently from the baselines, our model learns actions that correspond to specific movements of the platform.}
    \label{fig:breakout_density_plots}
\end{table*}
