# Supplementary material for: Playable Video Generation
Source: arXiv:2101.12195 source file (2021-01-28)
Supplement: Supplementary file 15 [file tennis_density_plots.tex]

\begin{table*}
    \centering
    
    \resizebox{\linewidth}{!}{
    \setlength\tabcolsep{0pt}
    \tiny
    
    \begin{tabular}{l@{\hskip 0.7mm}ccccccc}
         & Action 1 & Action 2 & Action 3 & Action 4 & Action 5 & Action 6 & Action 7  \\

         \rotatebox{90}{\hspace{0mm}\scalebox{1}{MoCoGAN \cite{tulyakov2018moco}}} &
         \includegraphics[trim=60 80 60 80,clip,width=0.2\columnwidth]{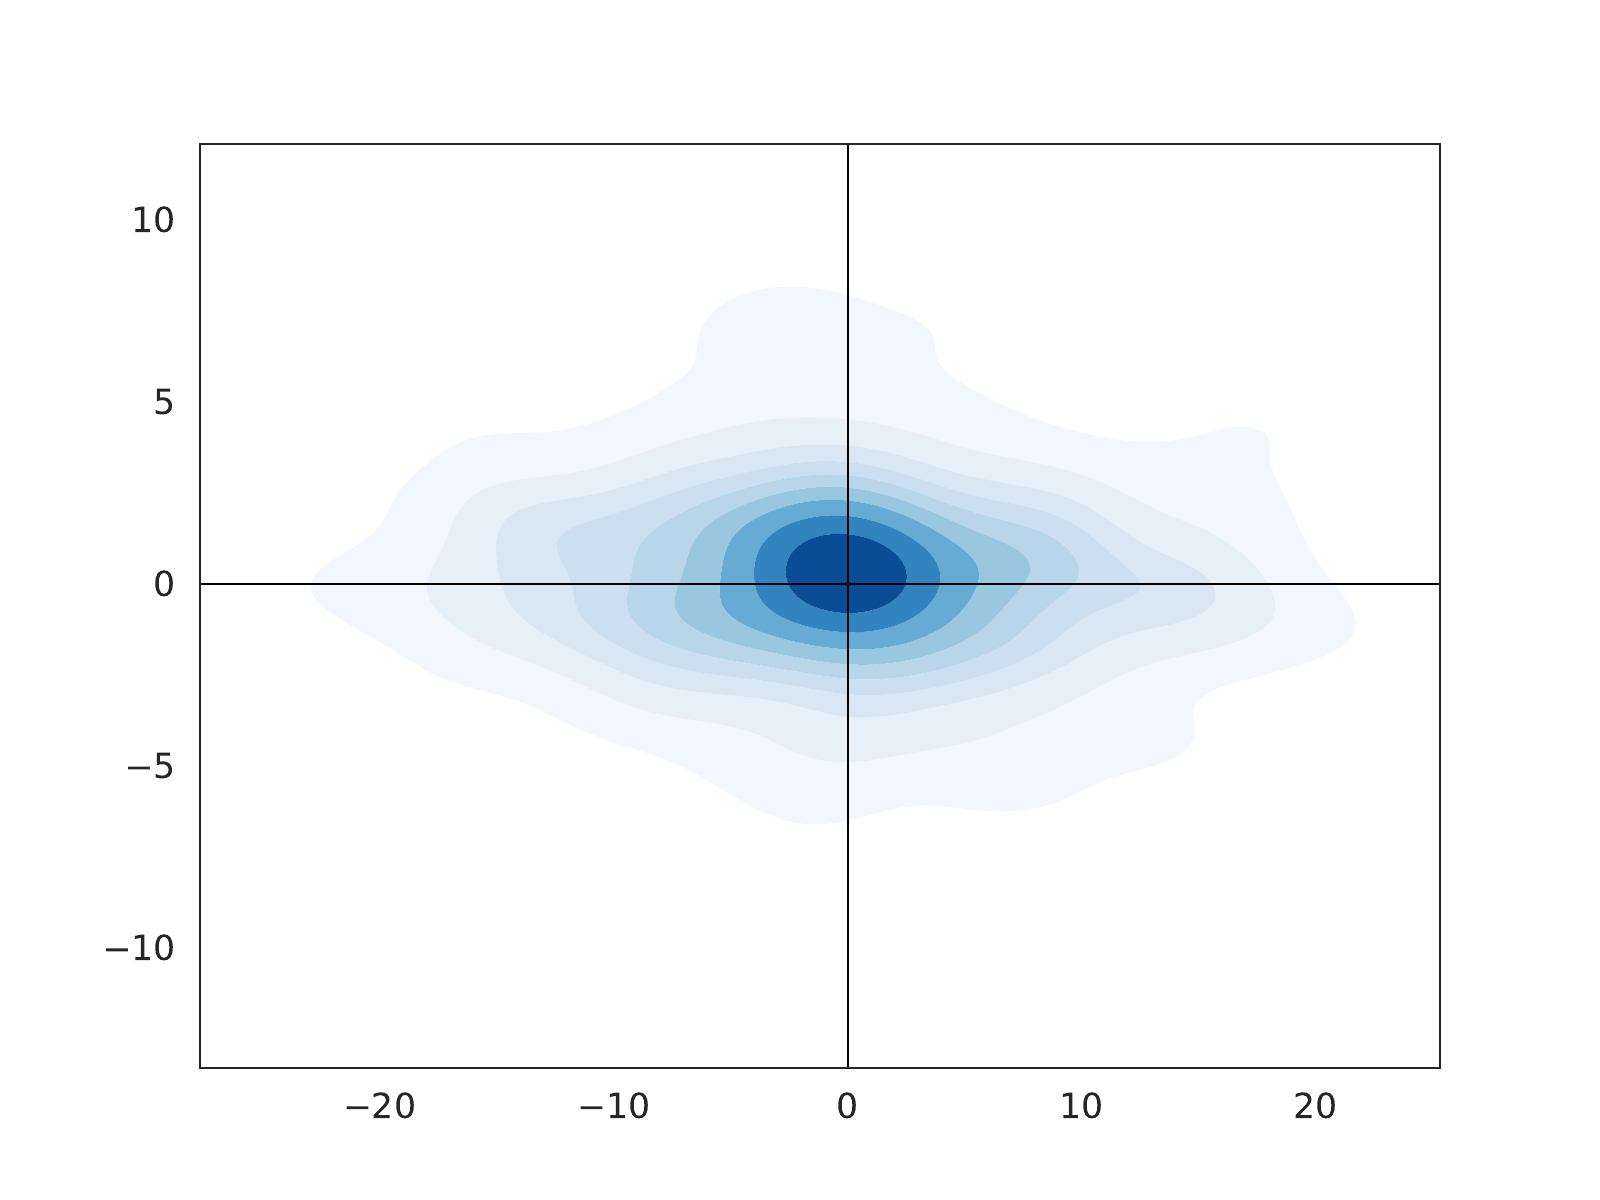} &
         \includegraphics[trim=60 80 60 80,clip,width=0.2\columnwidth]{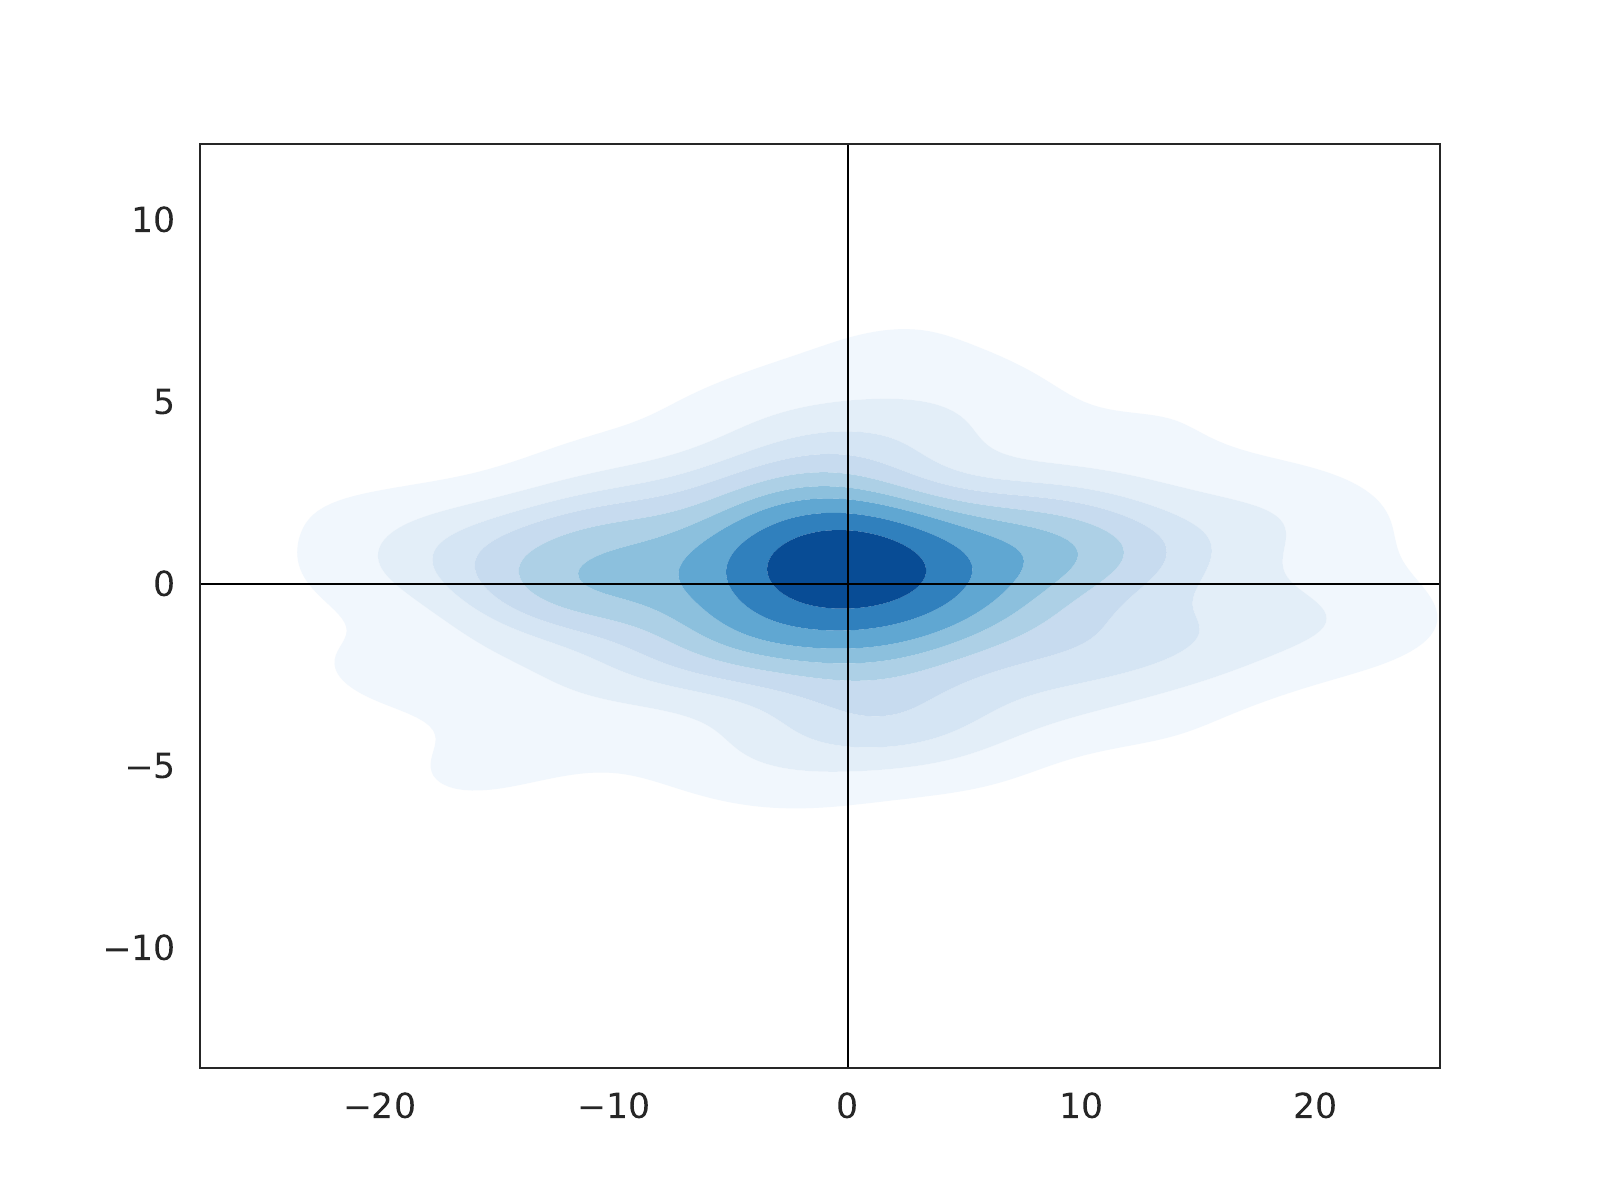} &
         \includegraphics[trim=60 80 60 80,clip,width=0.2\columnwidth]{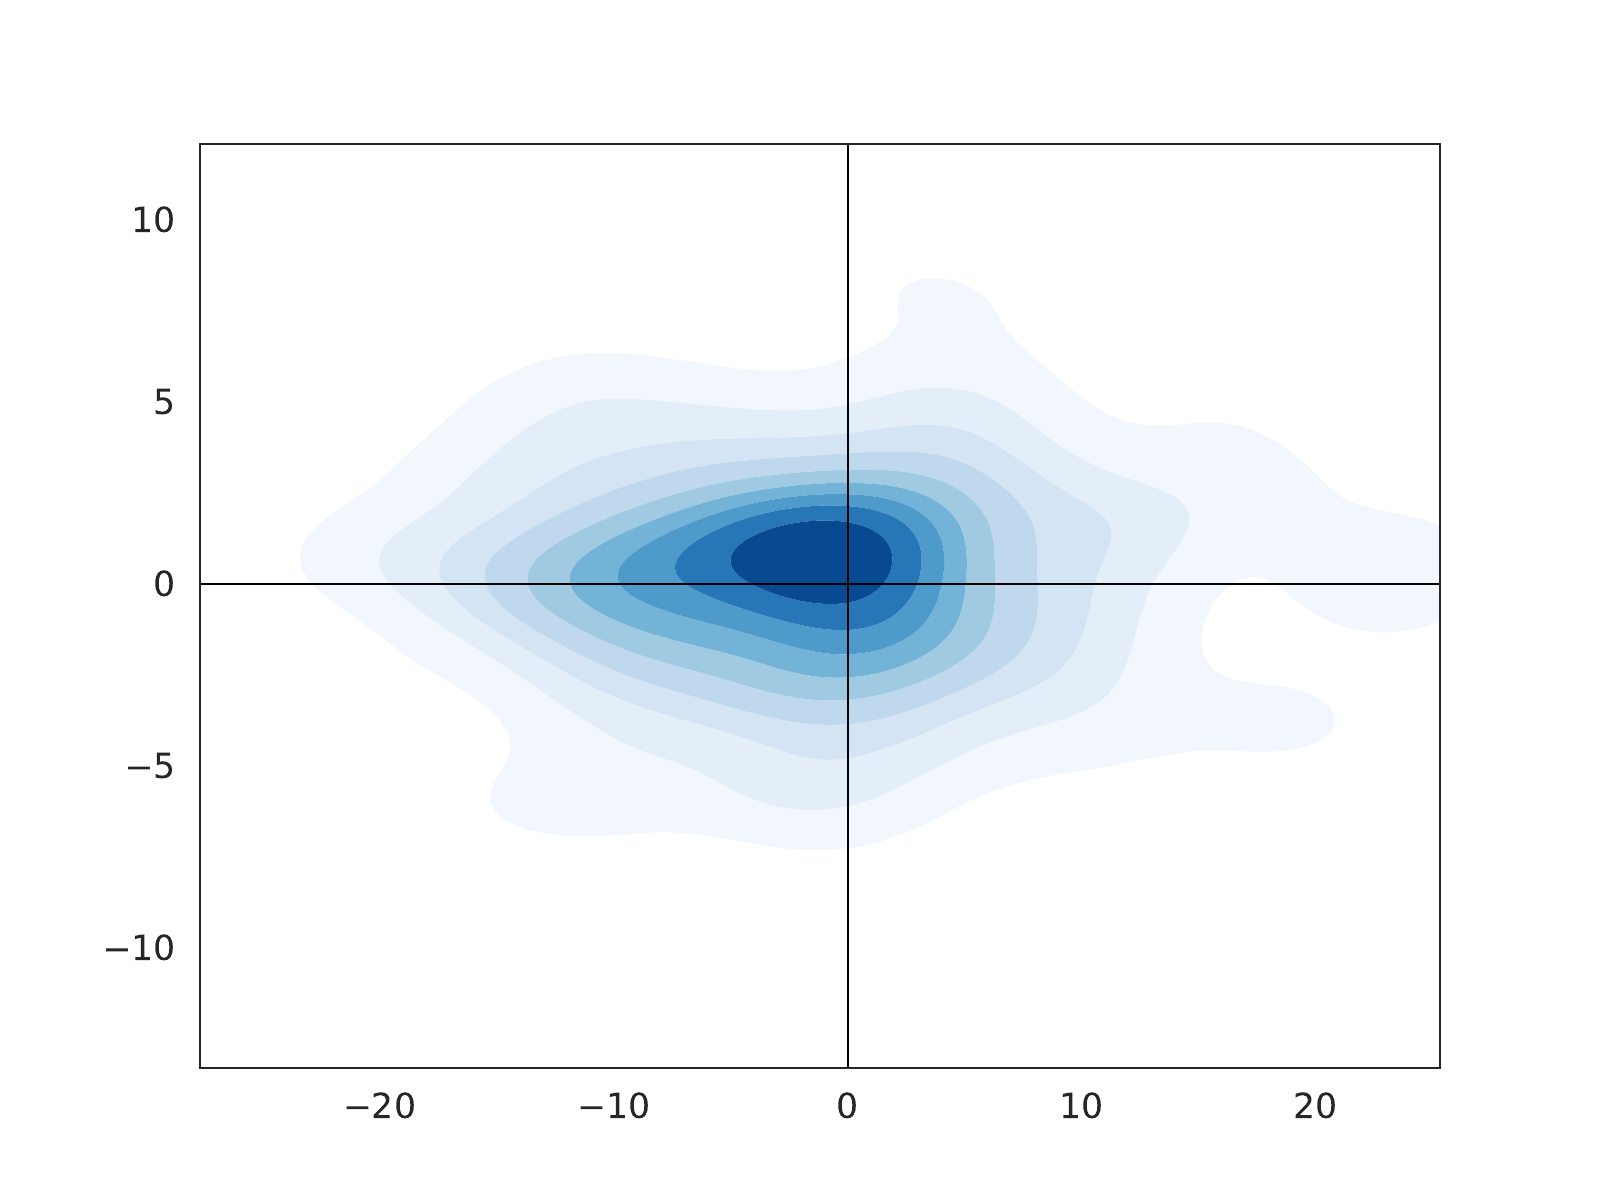} &
         \includegraphics[trim=60 80 60 80,clip,width=0.2\columnwidth]{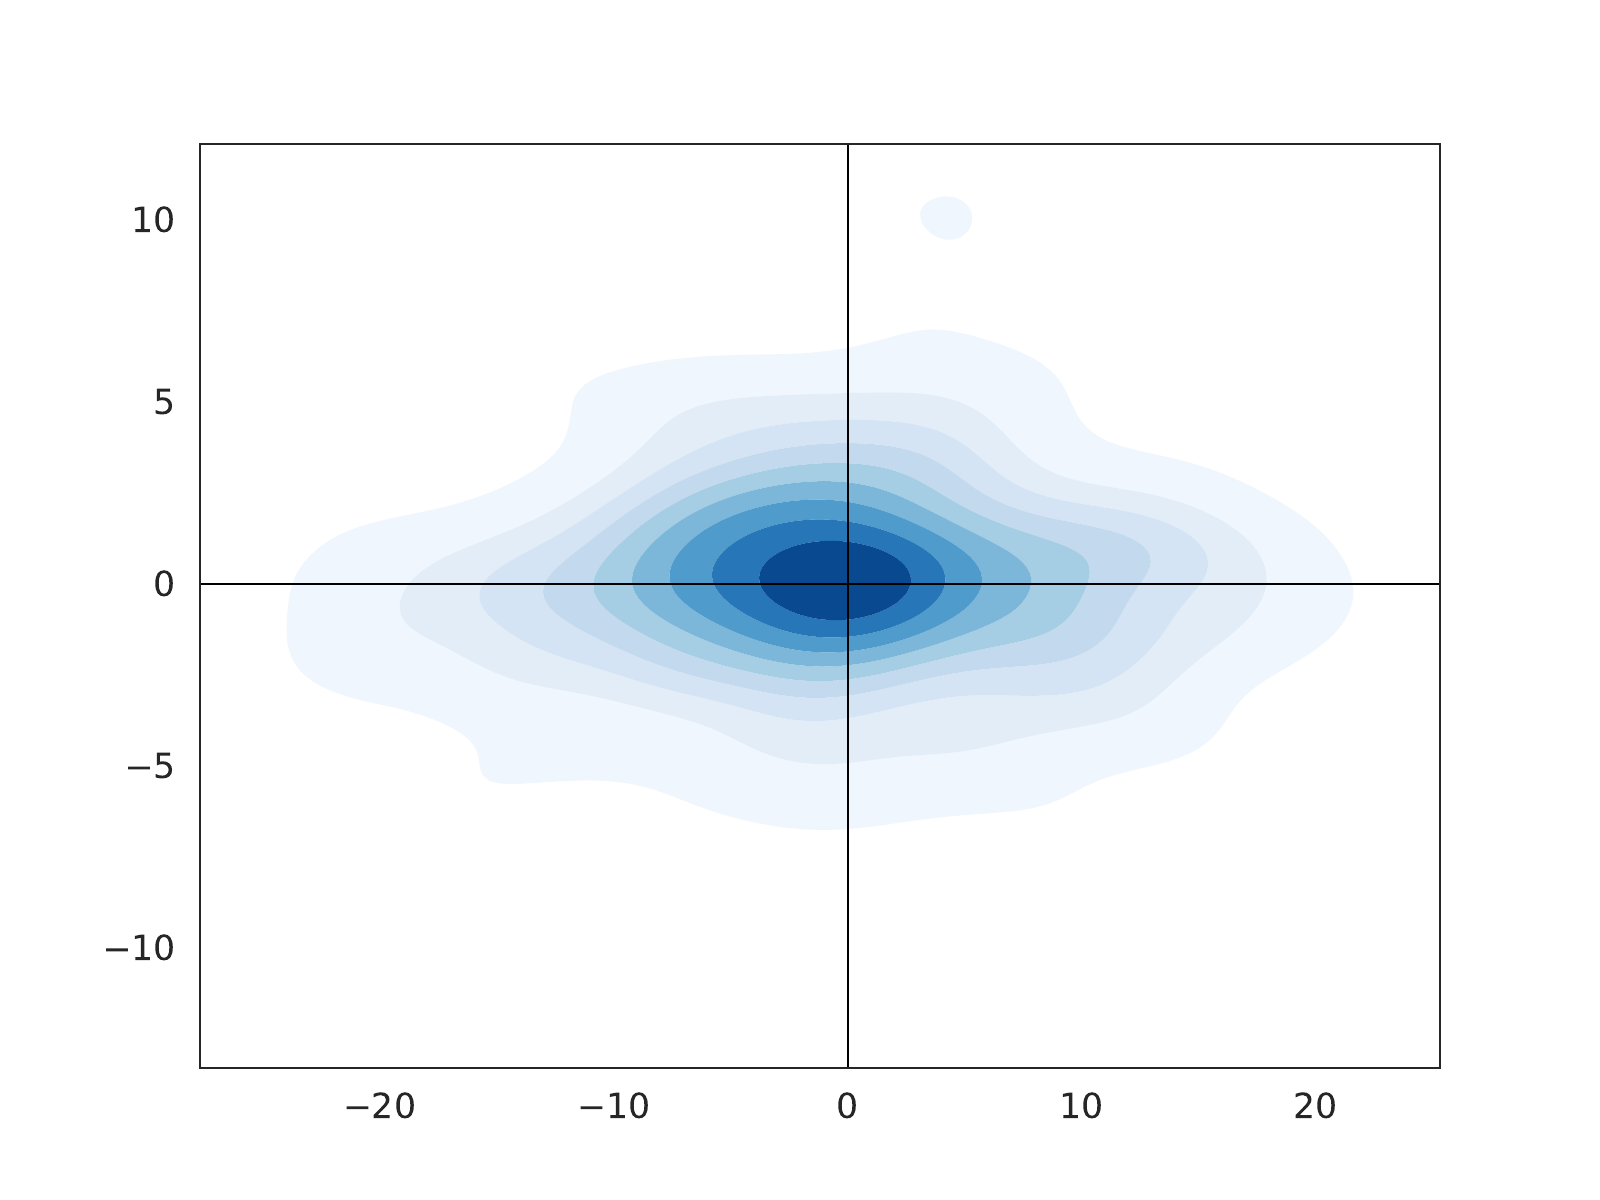} &
         \includegraphics[trim=60 80 60 80,clip,width=0.2\columnwidth]{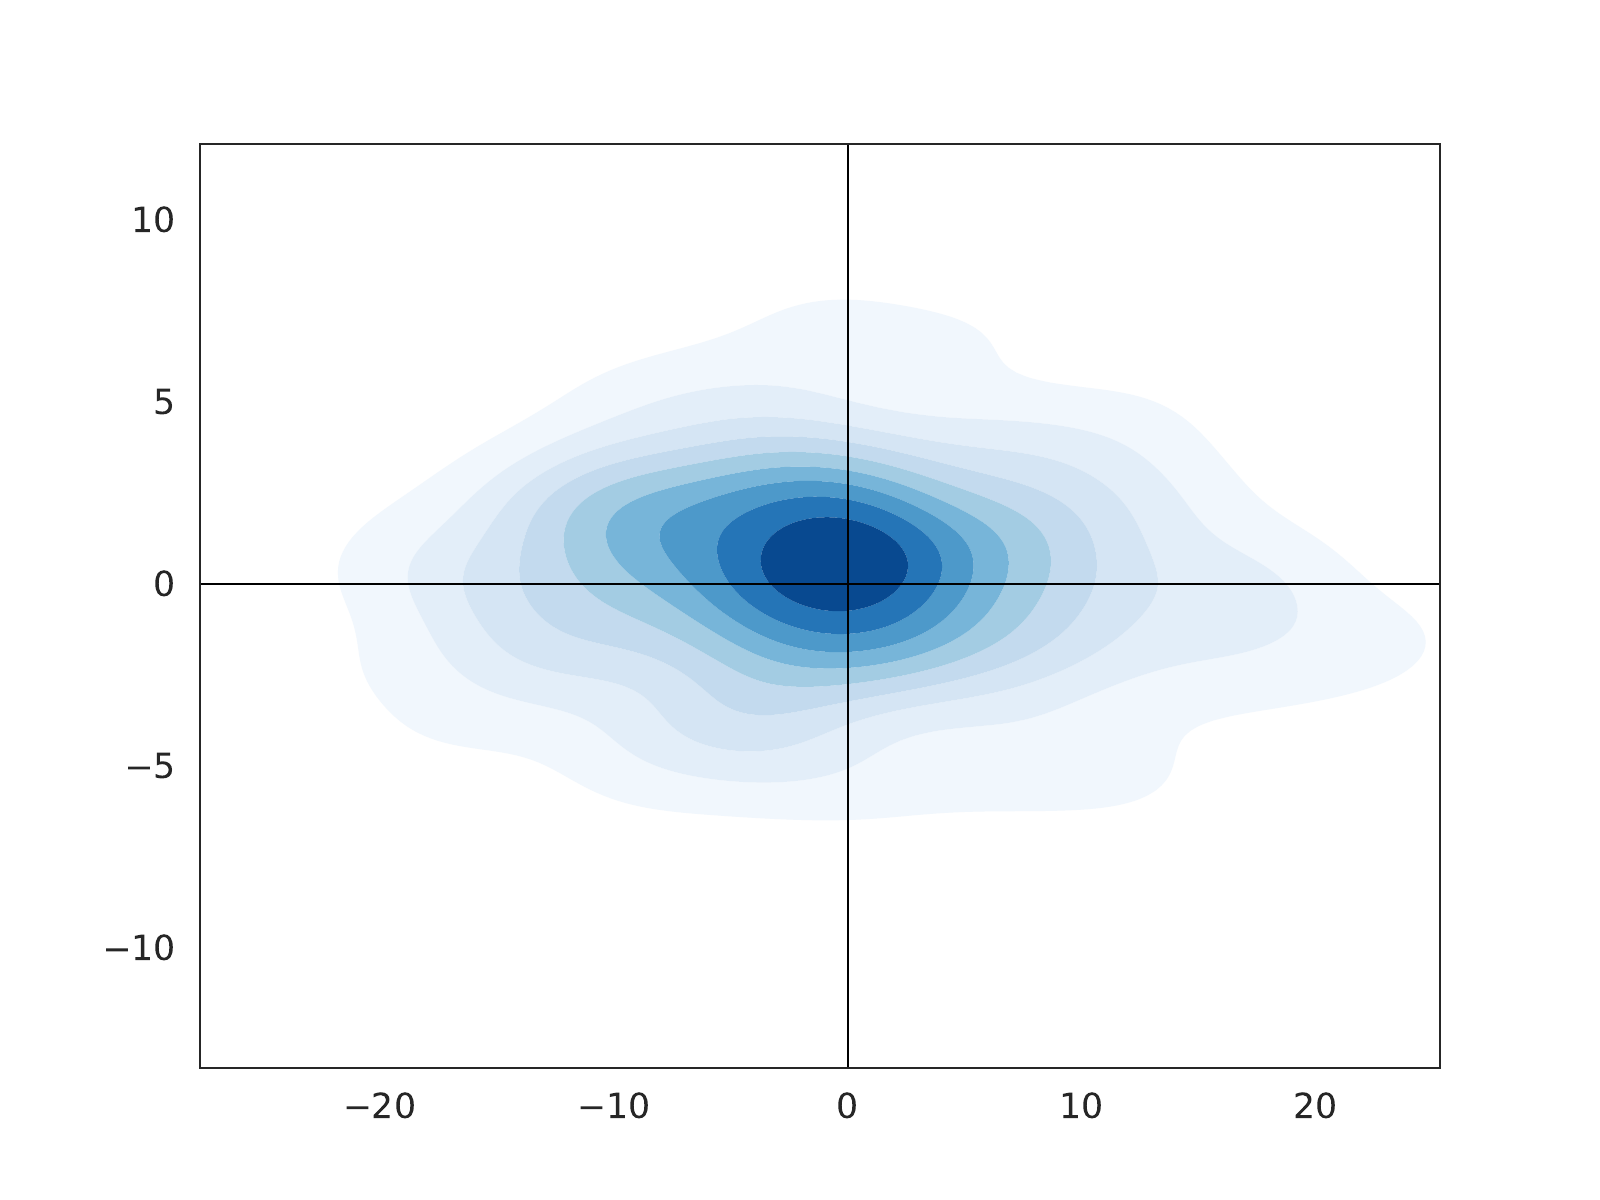} &
         \includegraphics[trim=60 80 60 80,clip,width=0.2\columnwidth]{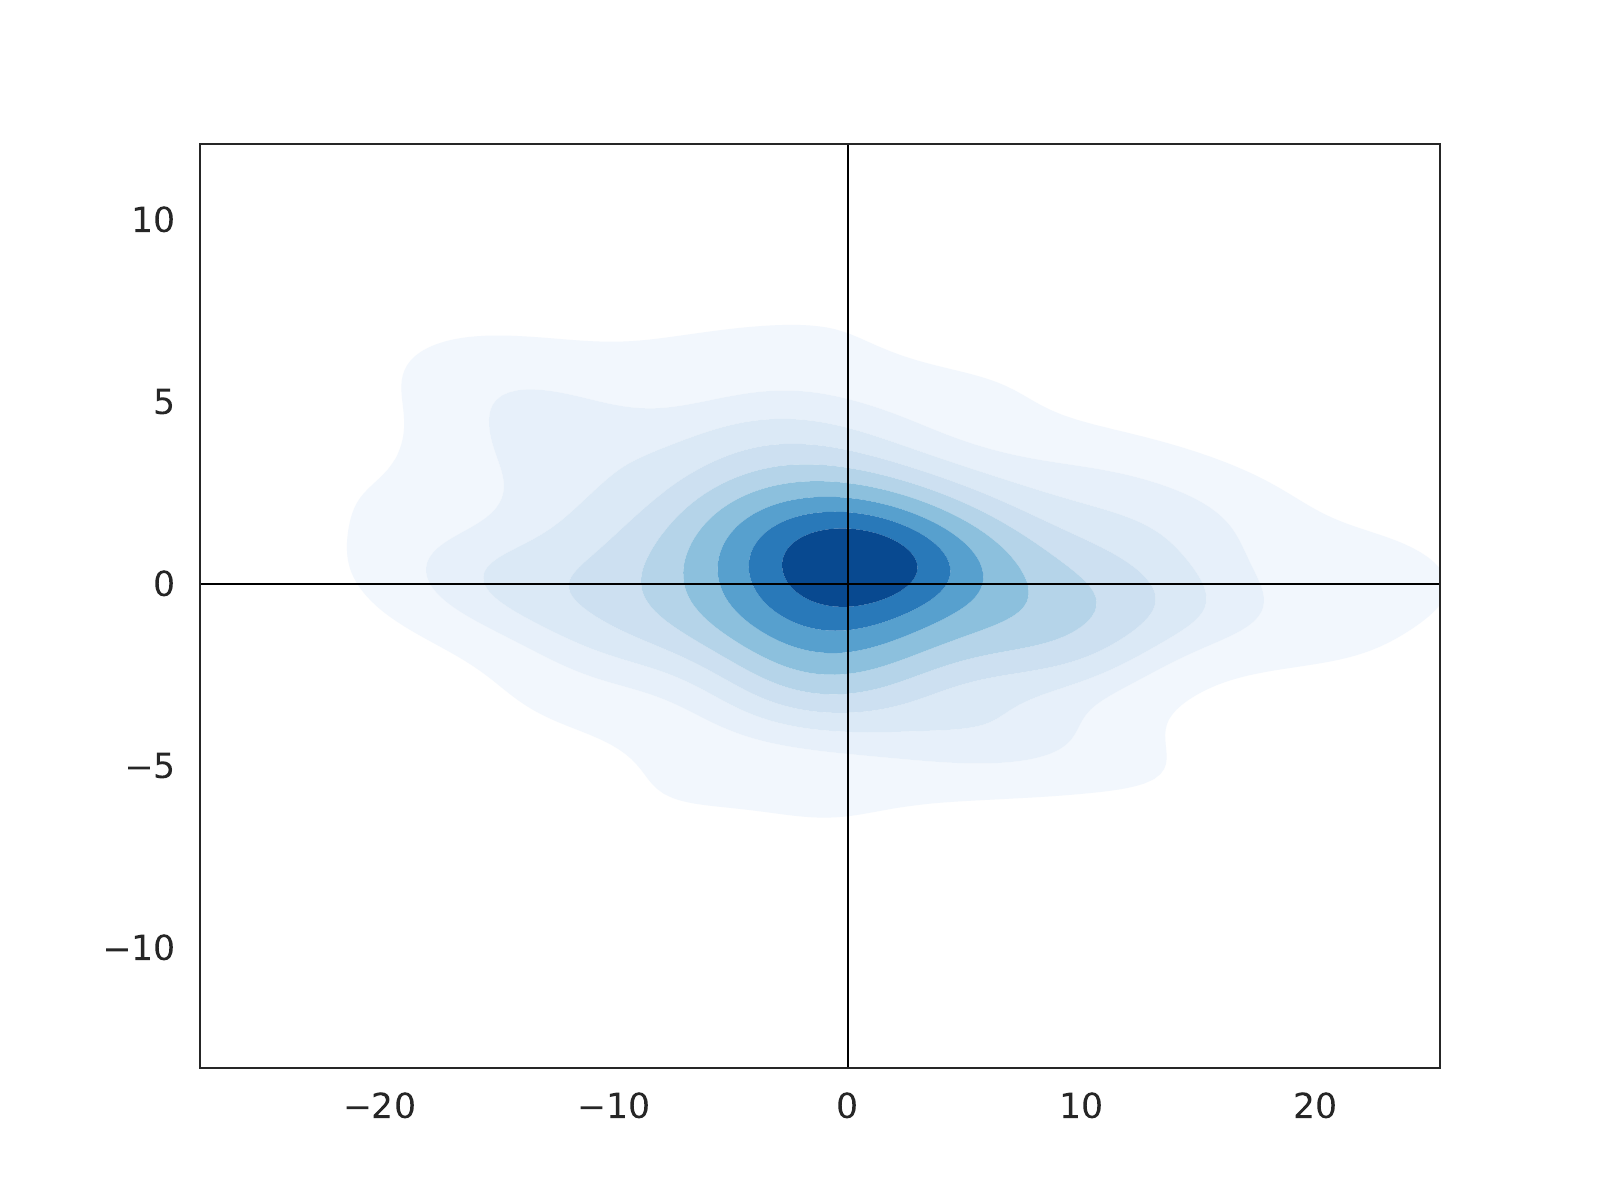} &
         \includegraphics[trim=60 80 60 80,clip,width=0.2\columnwidth]{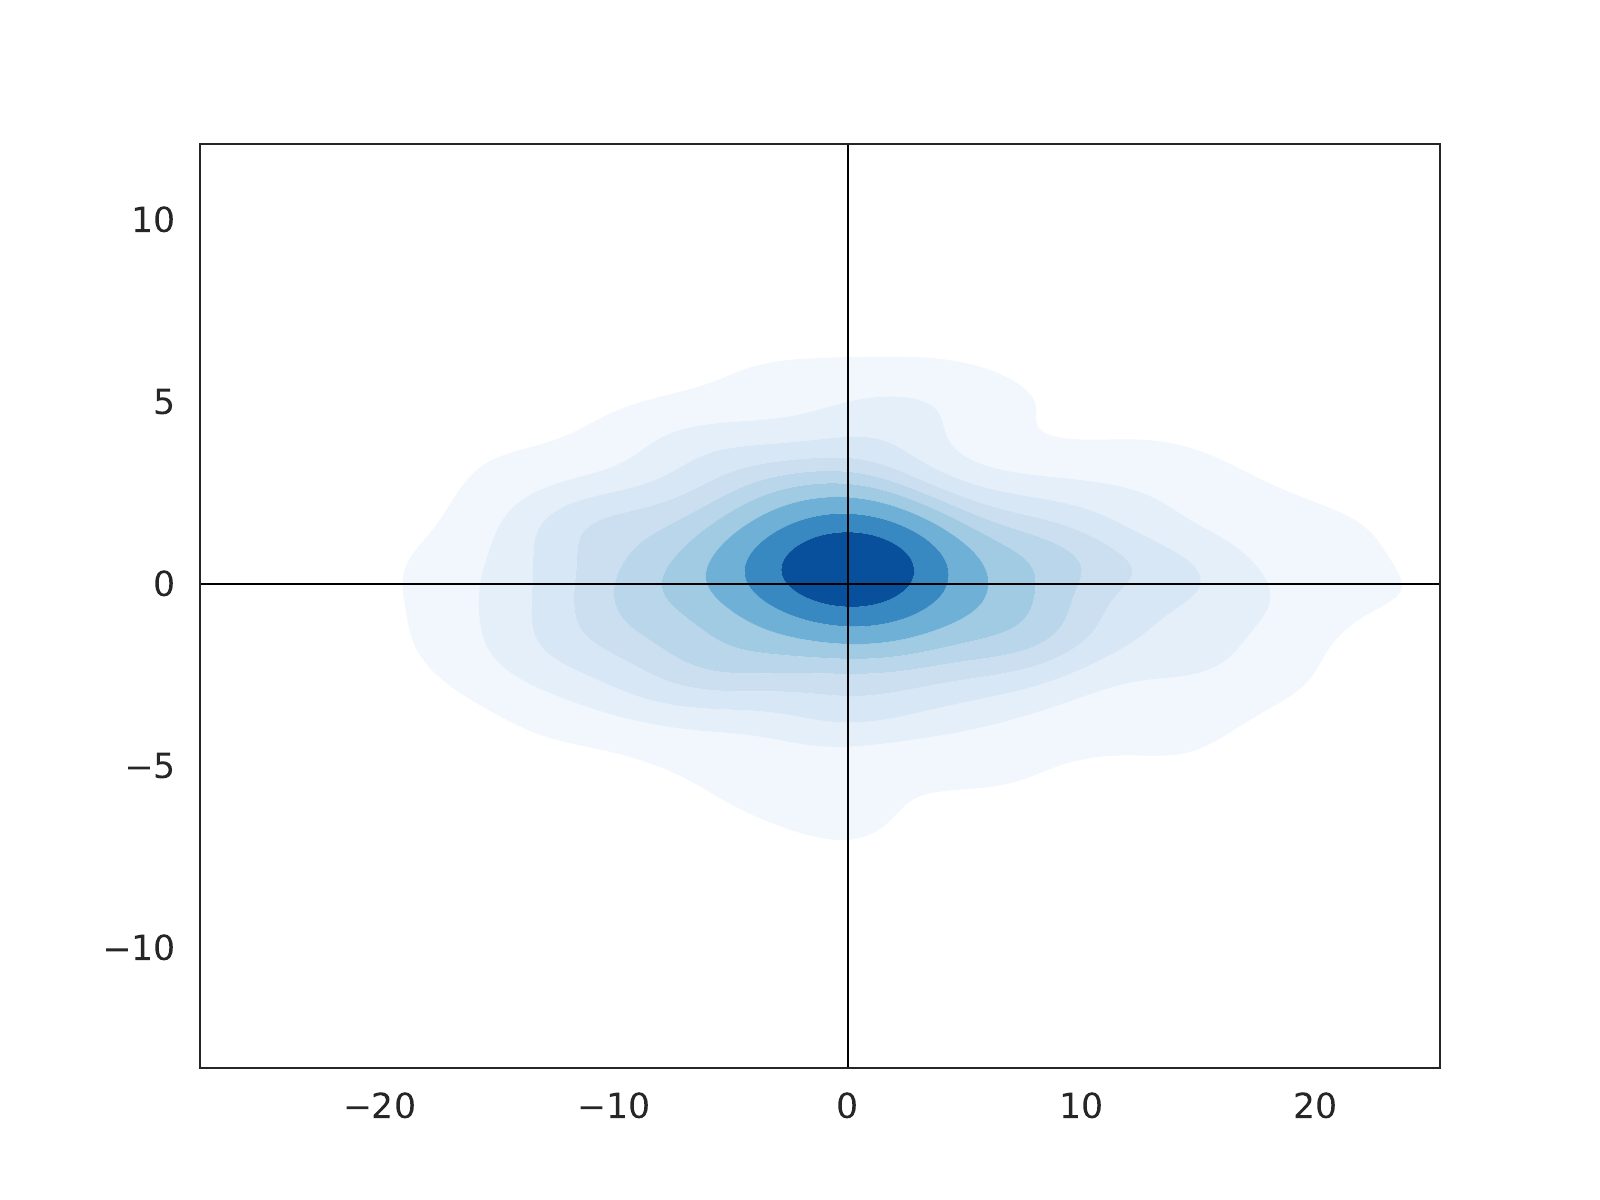} \\
         
         \rotatebox{90}{\hspace{0mm}\scalebox{1}{MoCoGAN+}} &
         \includegraphics[trim=60 80 60 80,clip,width=0.2\columnwidth]{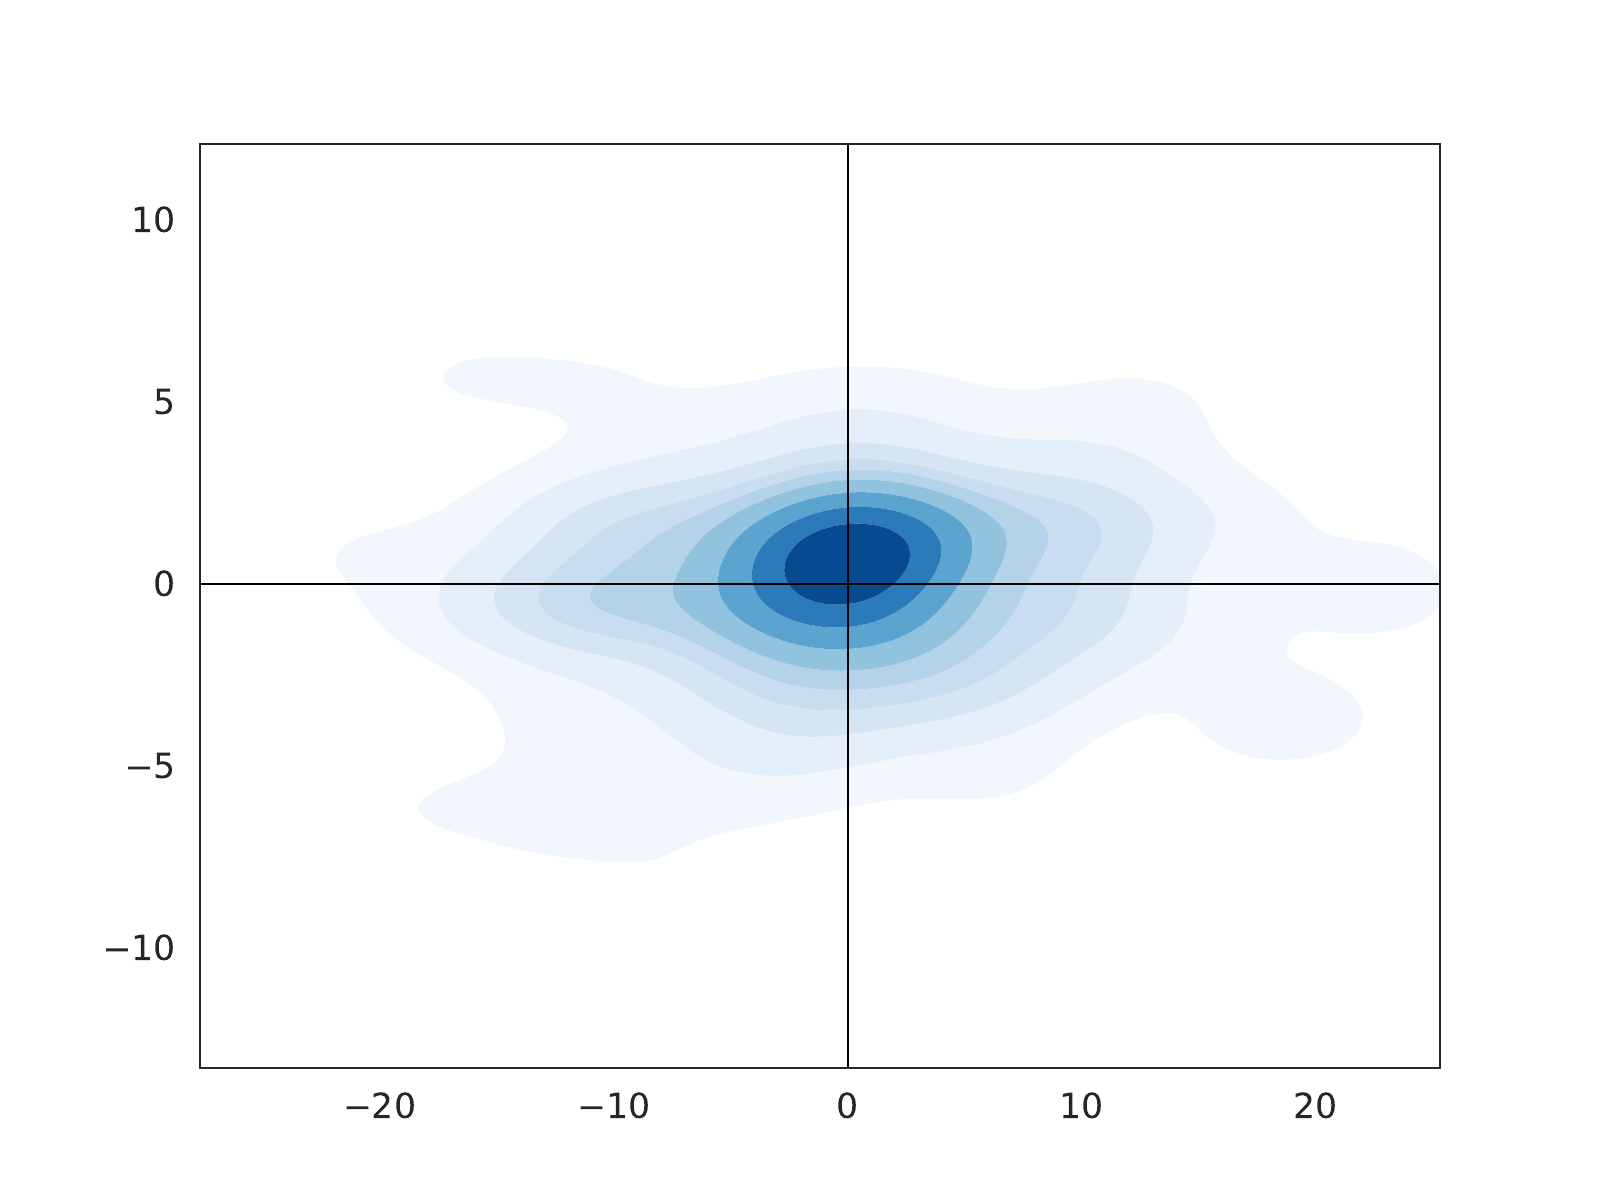} &
         \includegraphics[trim=60 80 60 80,clip,width=0.2\columnwidth]{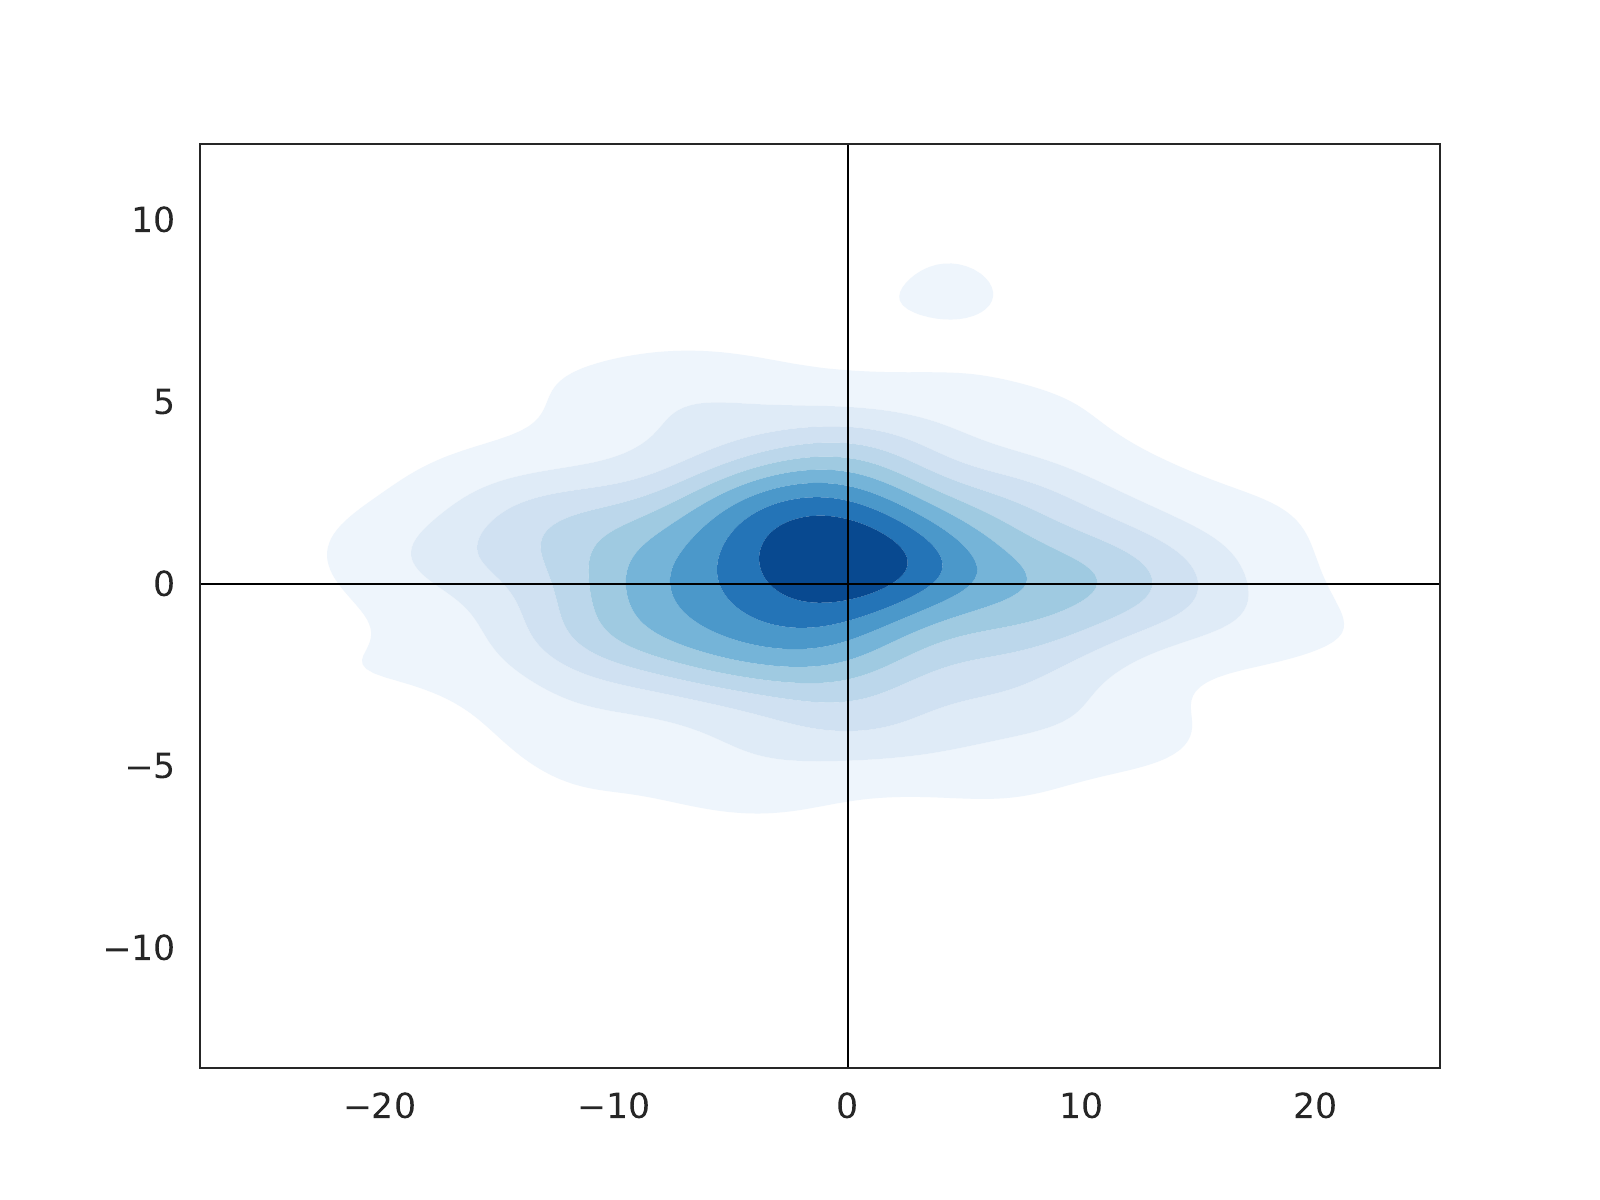} &
         \includegraphics[trim=60 80 60 80,clip,width=0.2\columnwidth]{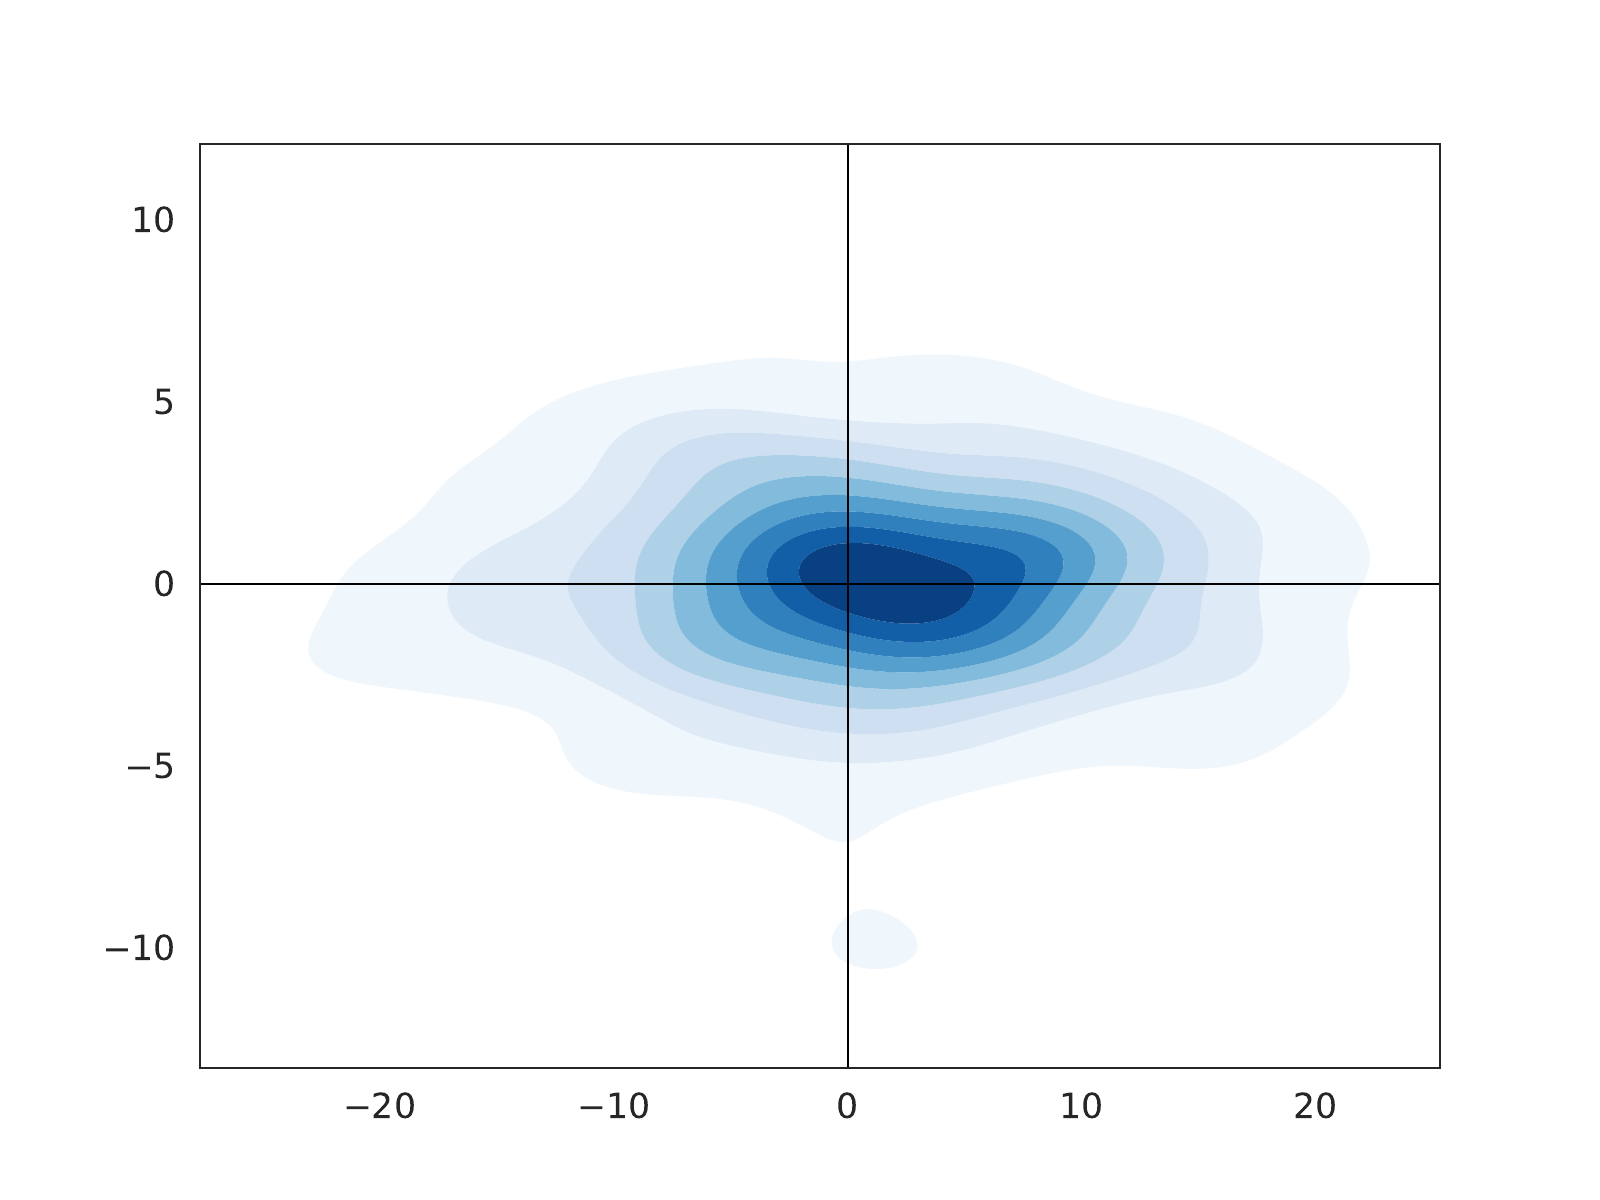} &
         \includegraphics[trim=60 80 60 80,clip,width=0.2\columnwidth]{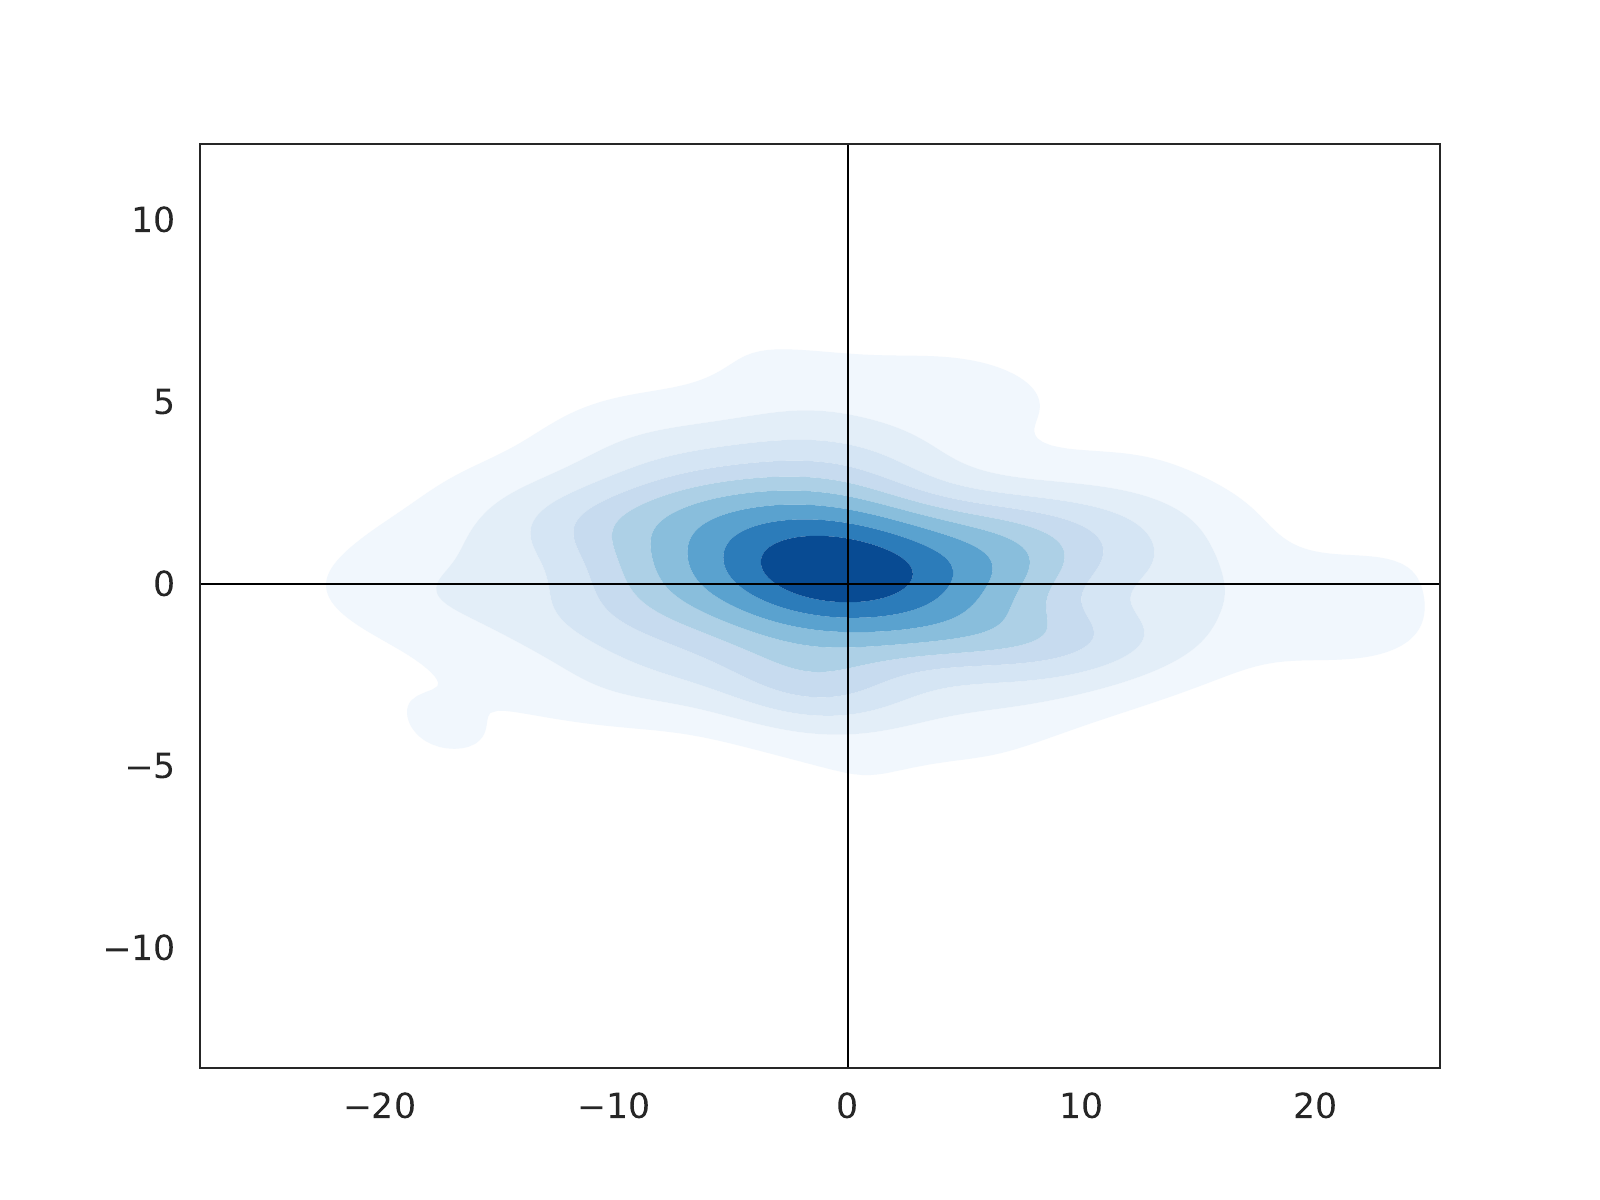} &
         \includegraphics[trim=60 80 60 80,clip,width=0.2\columnwidth]{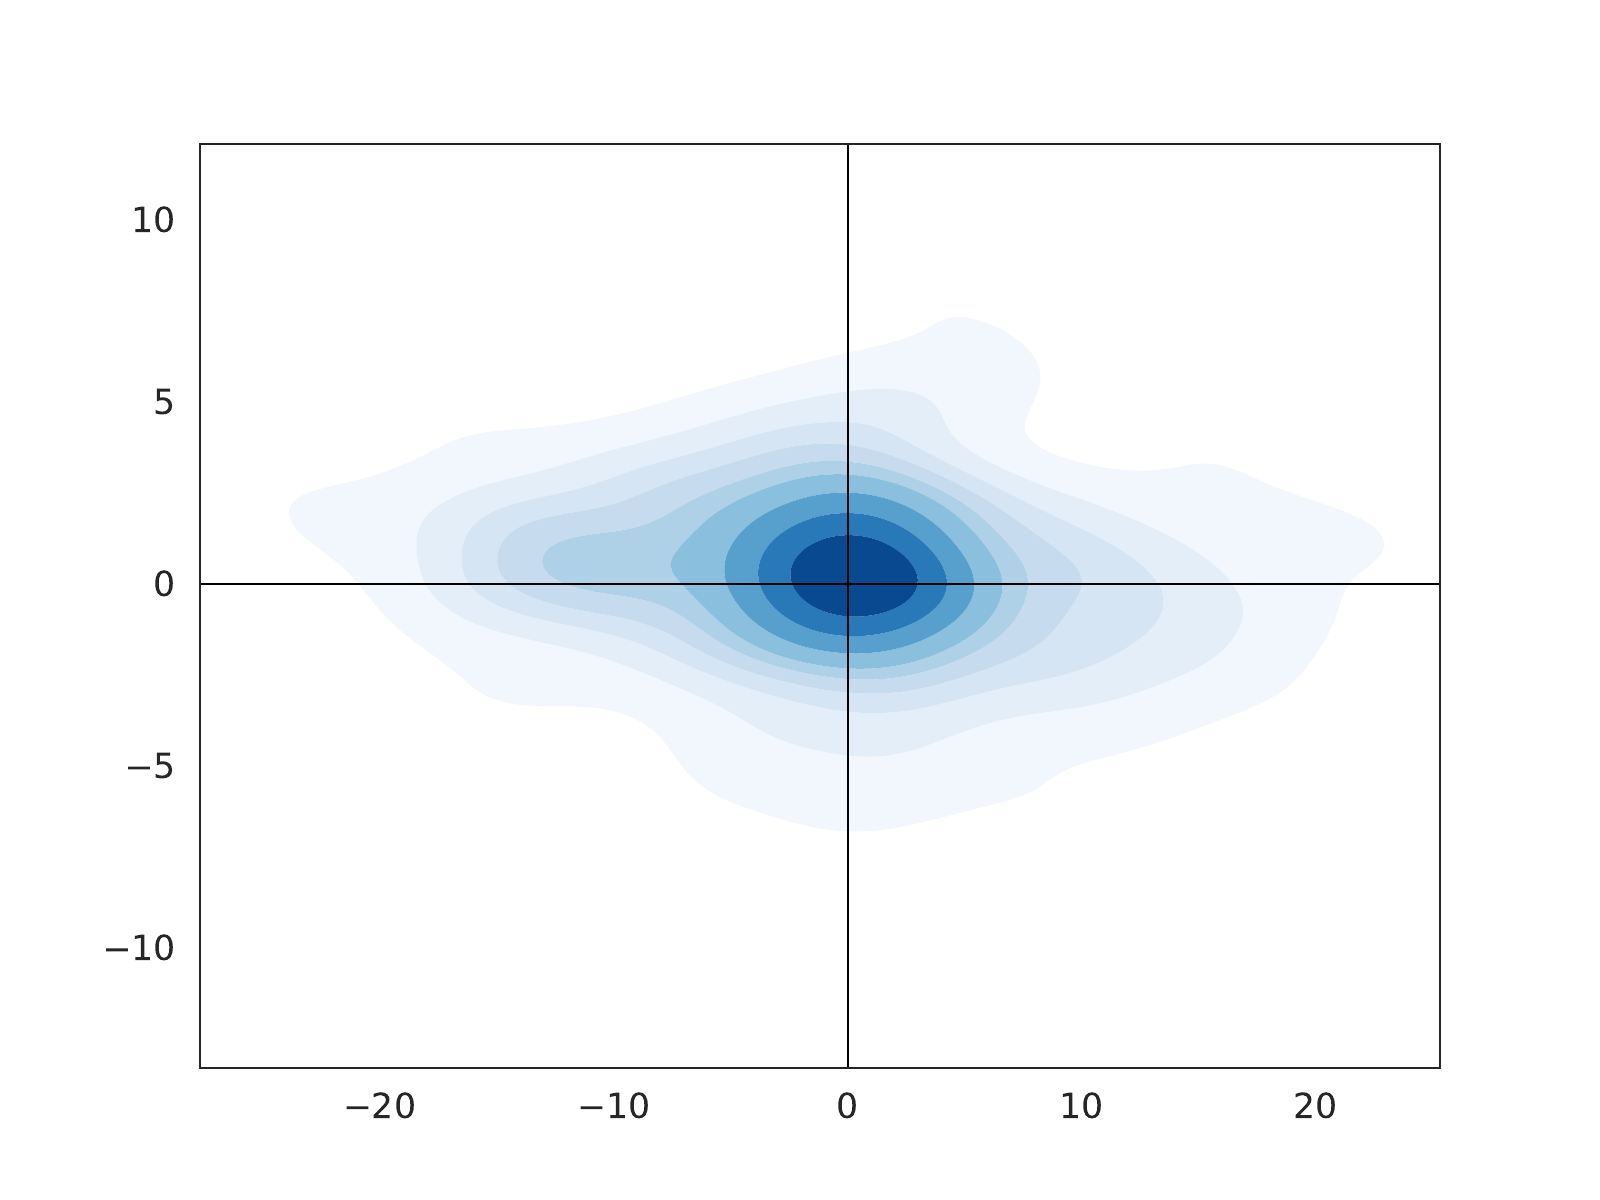} &
         \includegraphics[trim=60 80 60 80,clip,width=0.2\columnwidth]{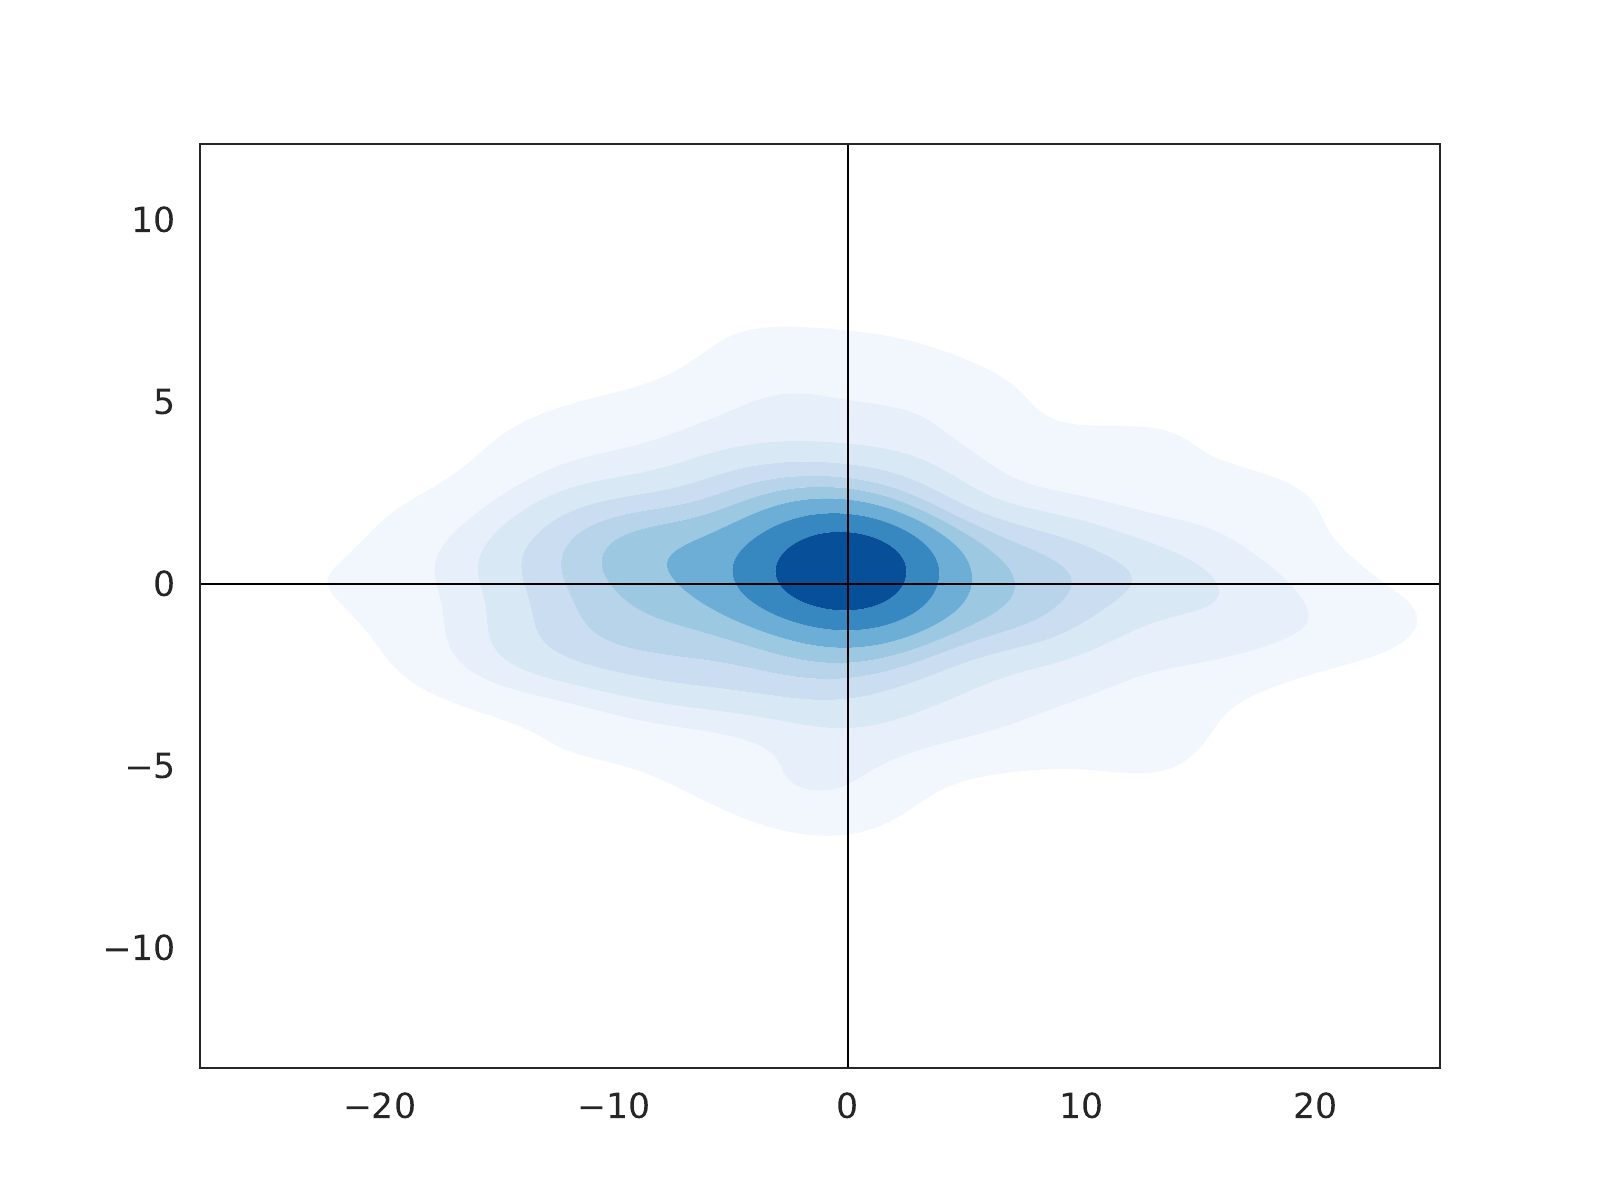} &
         \includegraphics[trim=60 80 60 80,clip,width=0.2\columnwidth]{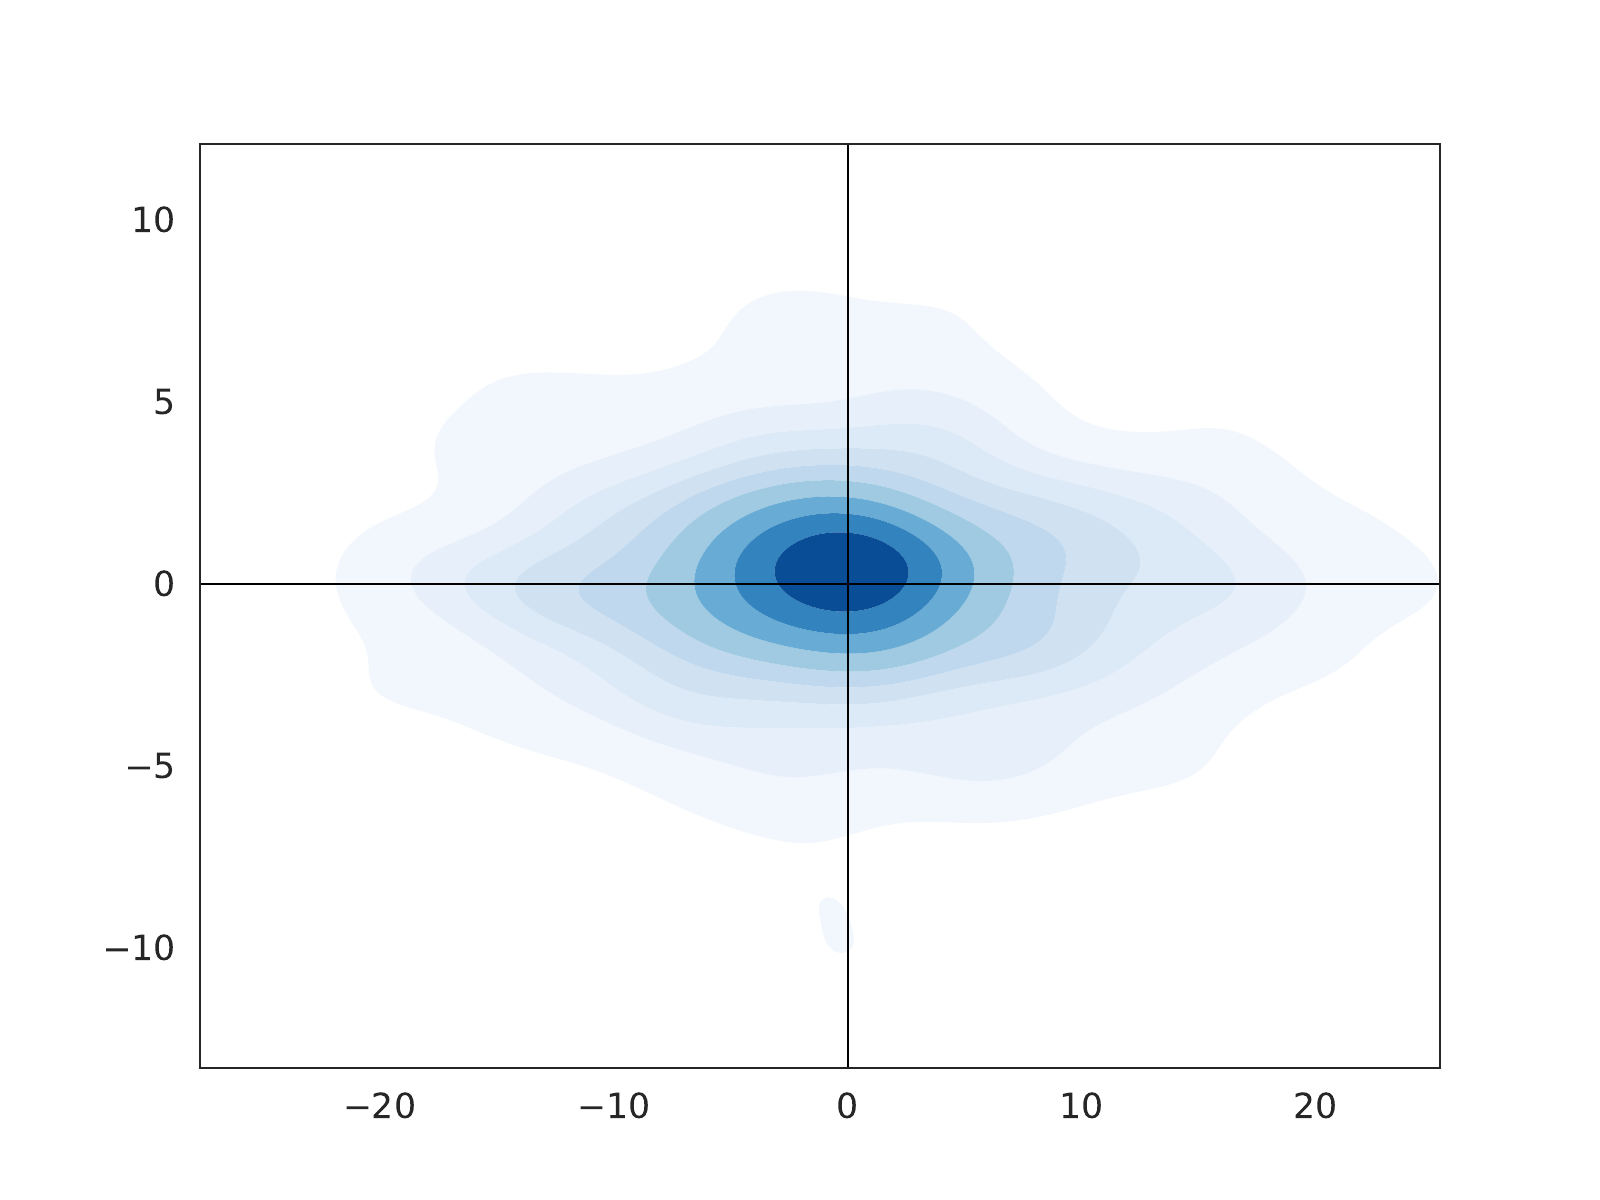} \\
         
         \rotatebox{90}{\hspace{1.8mm}SAVP\cite{lee2018savp}} &
         \includegraphics[trim=60 80 60 80,clip,width=0.2\columnwidth]{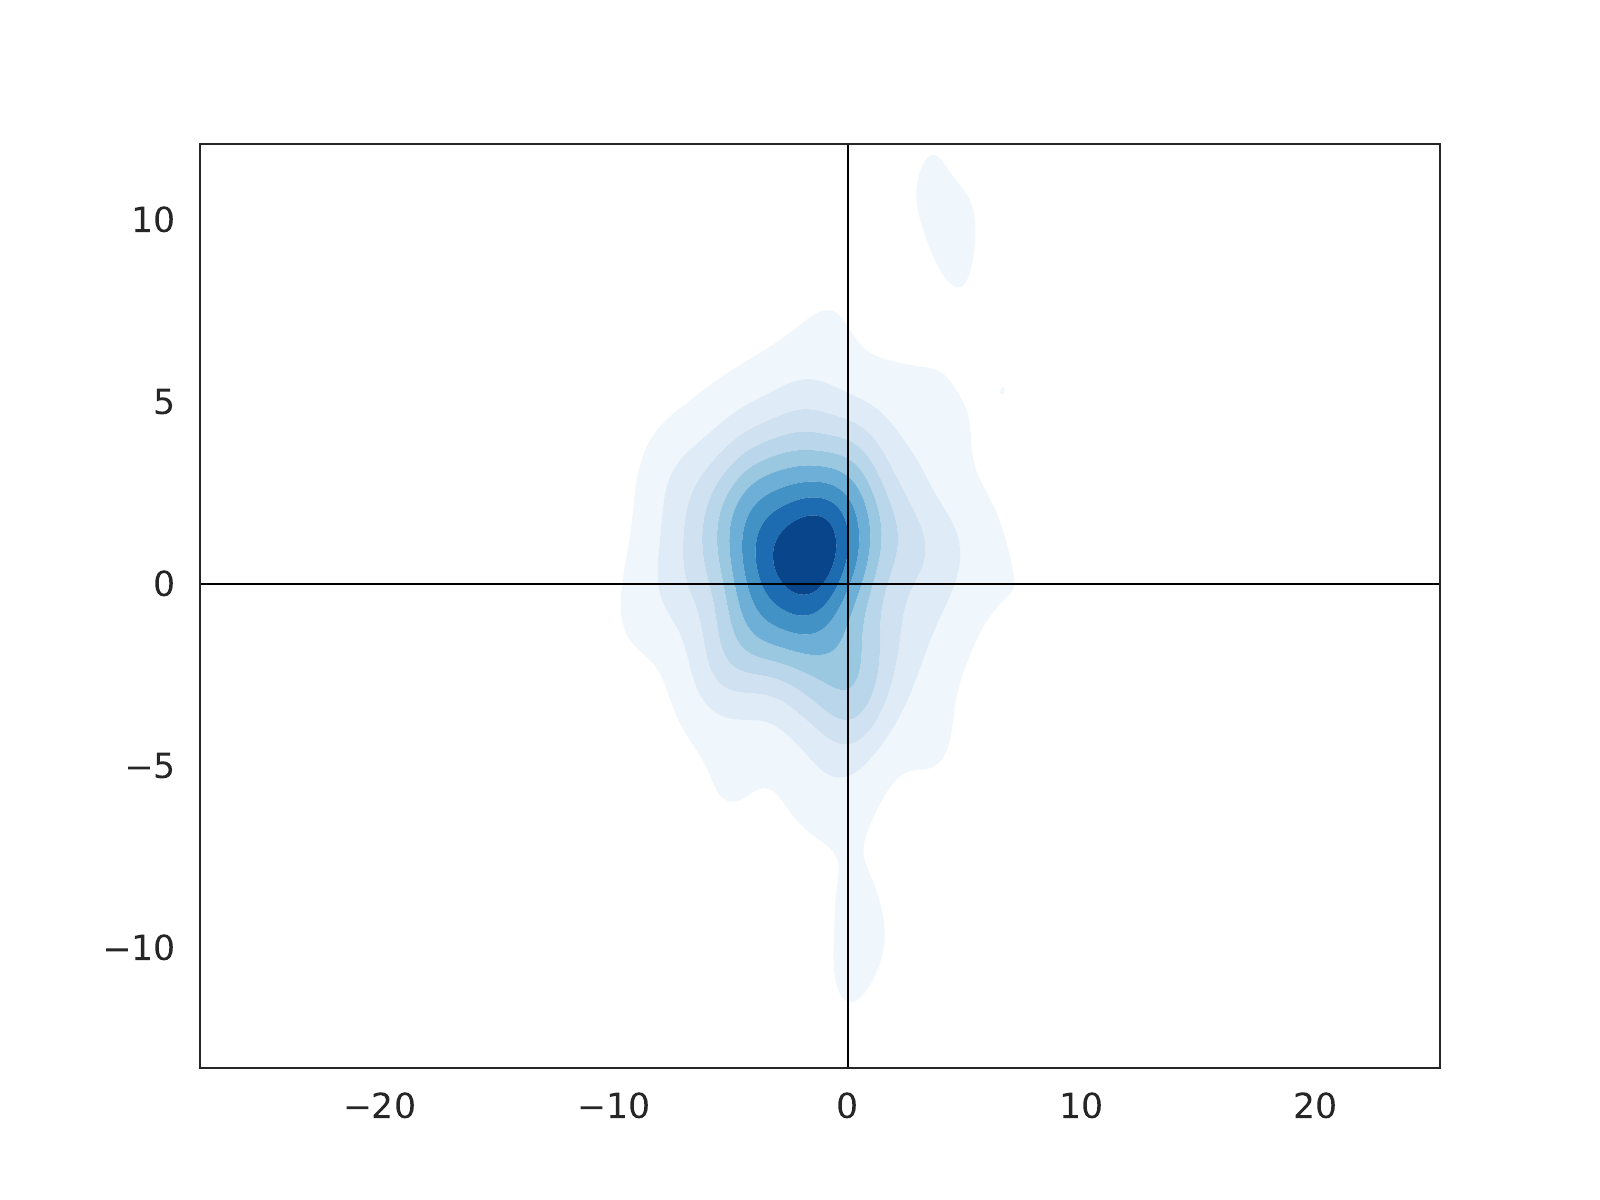} &
         \includegraphics[trim=60 80 60 80,clip,width=0.2\columnwidth]{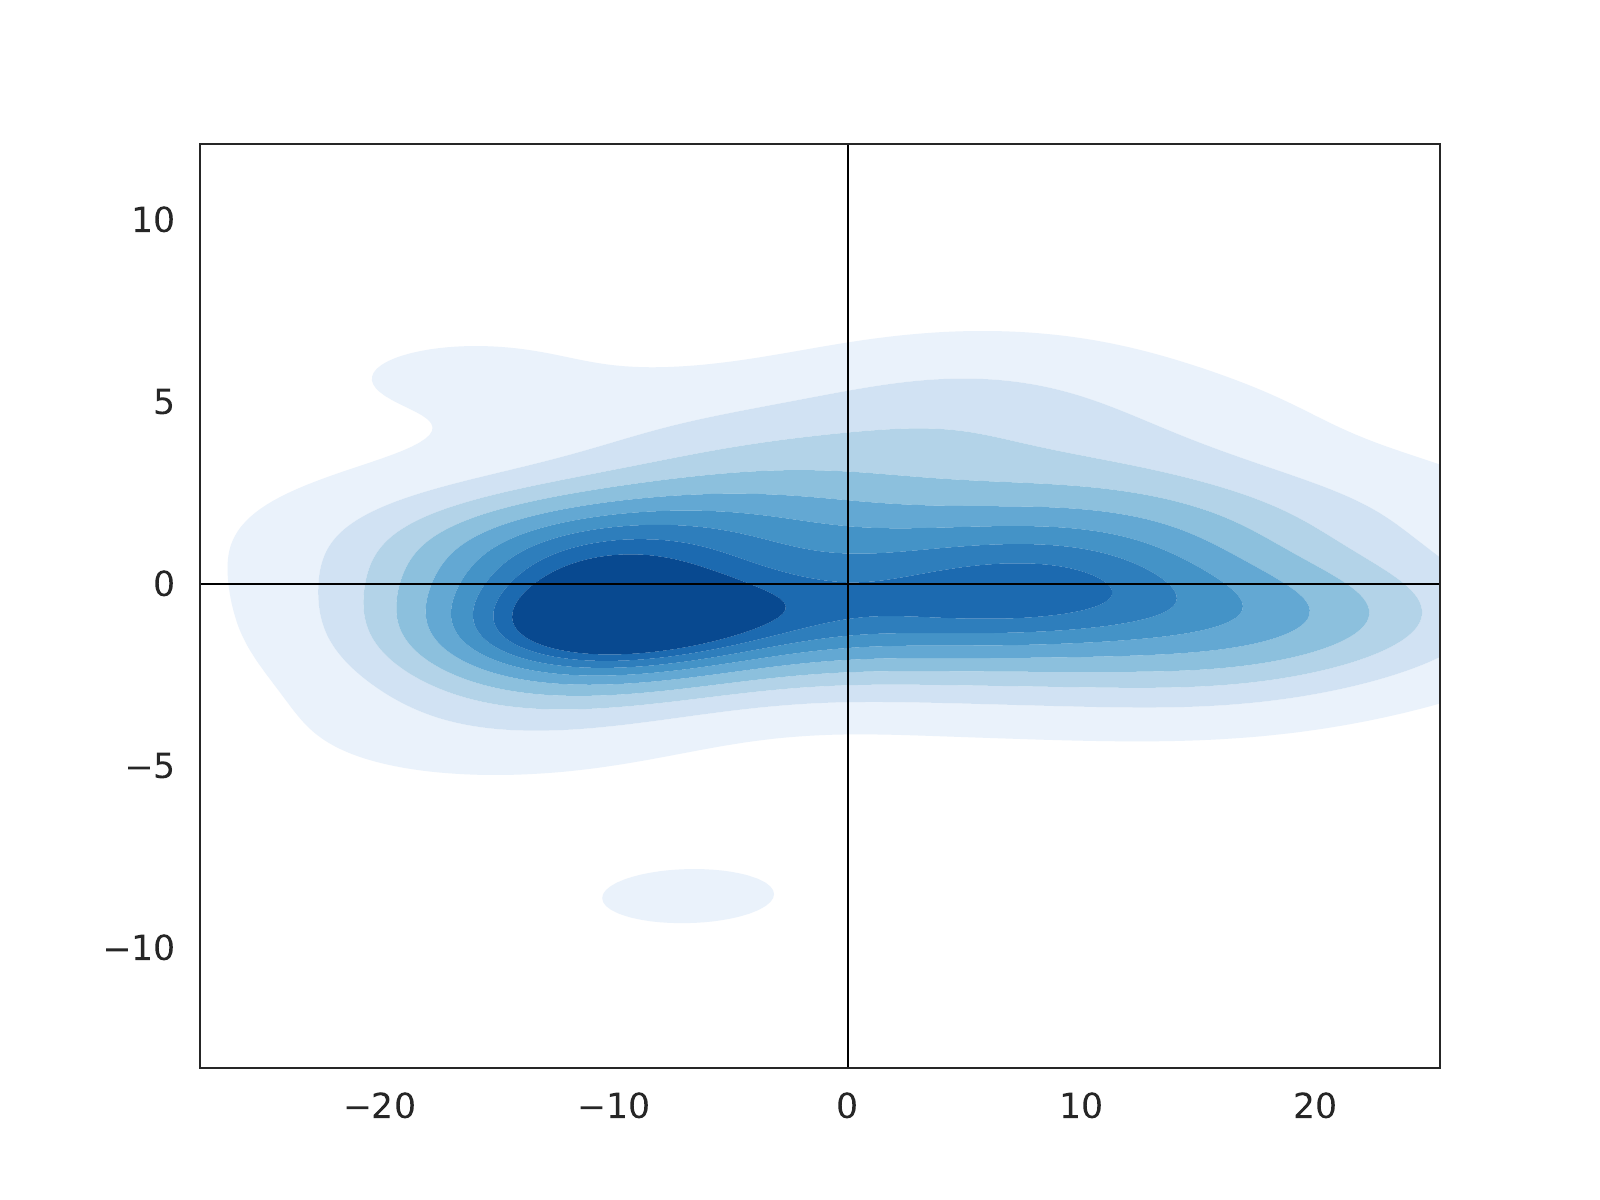} &
         \includegraphics[trim=60 80 60 80,clip,width=0.2\columnwidth]{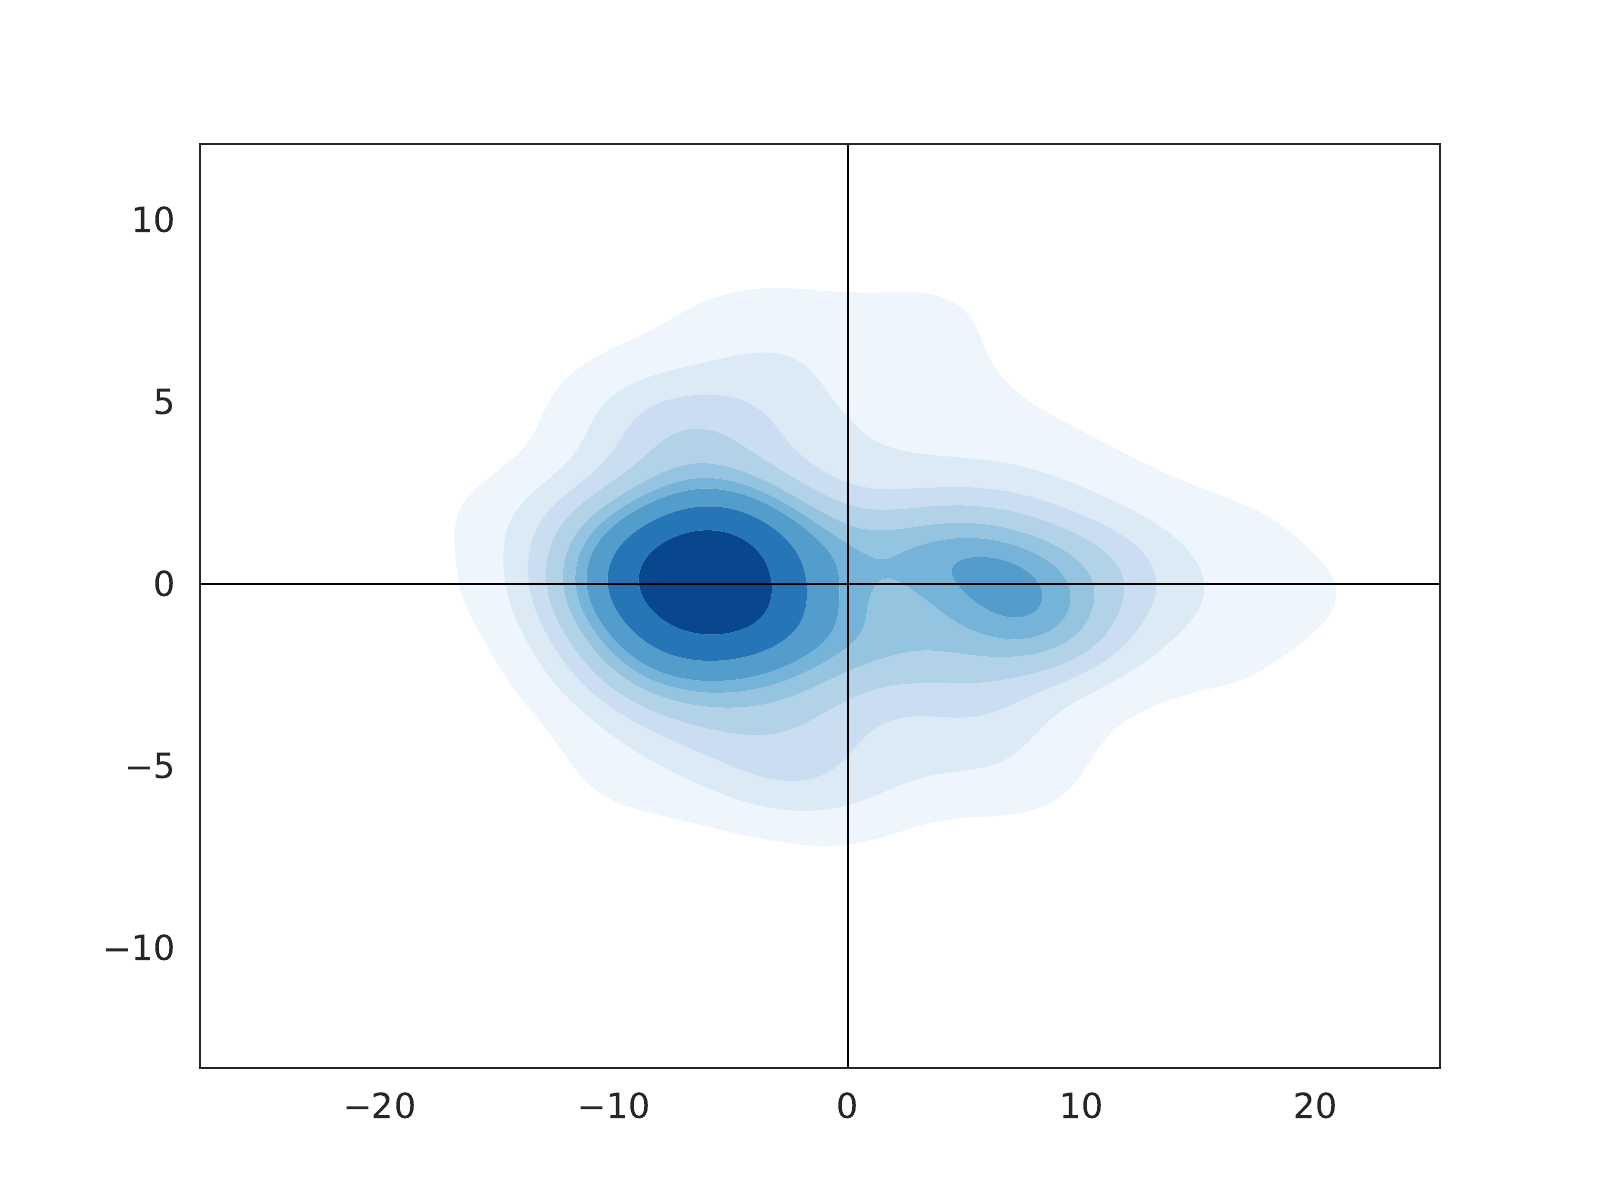} &
         \includegraphics[trim=60 80 60 80,clip,width=0.2\columnwidth]{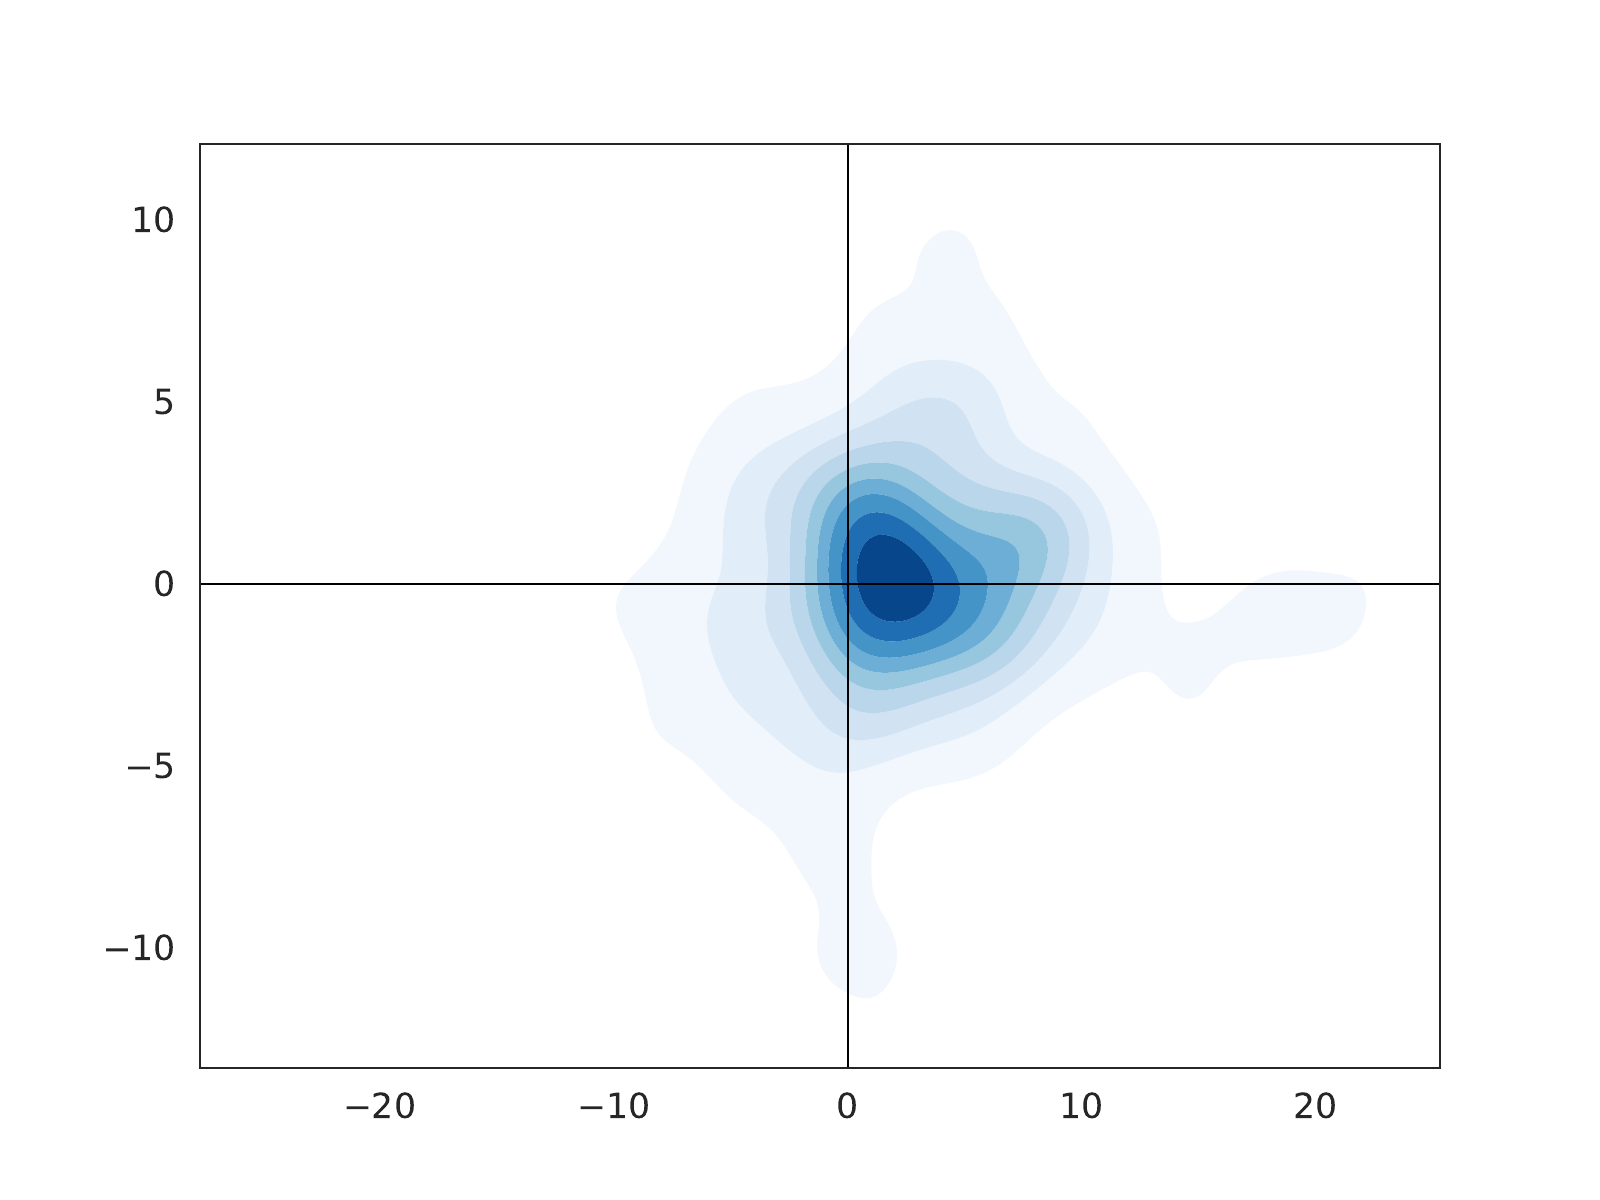} &
         \includegraphics[trim=60 80 60 80,clip,width=0.2\columnwidth]{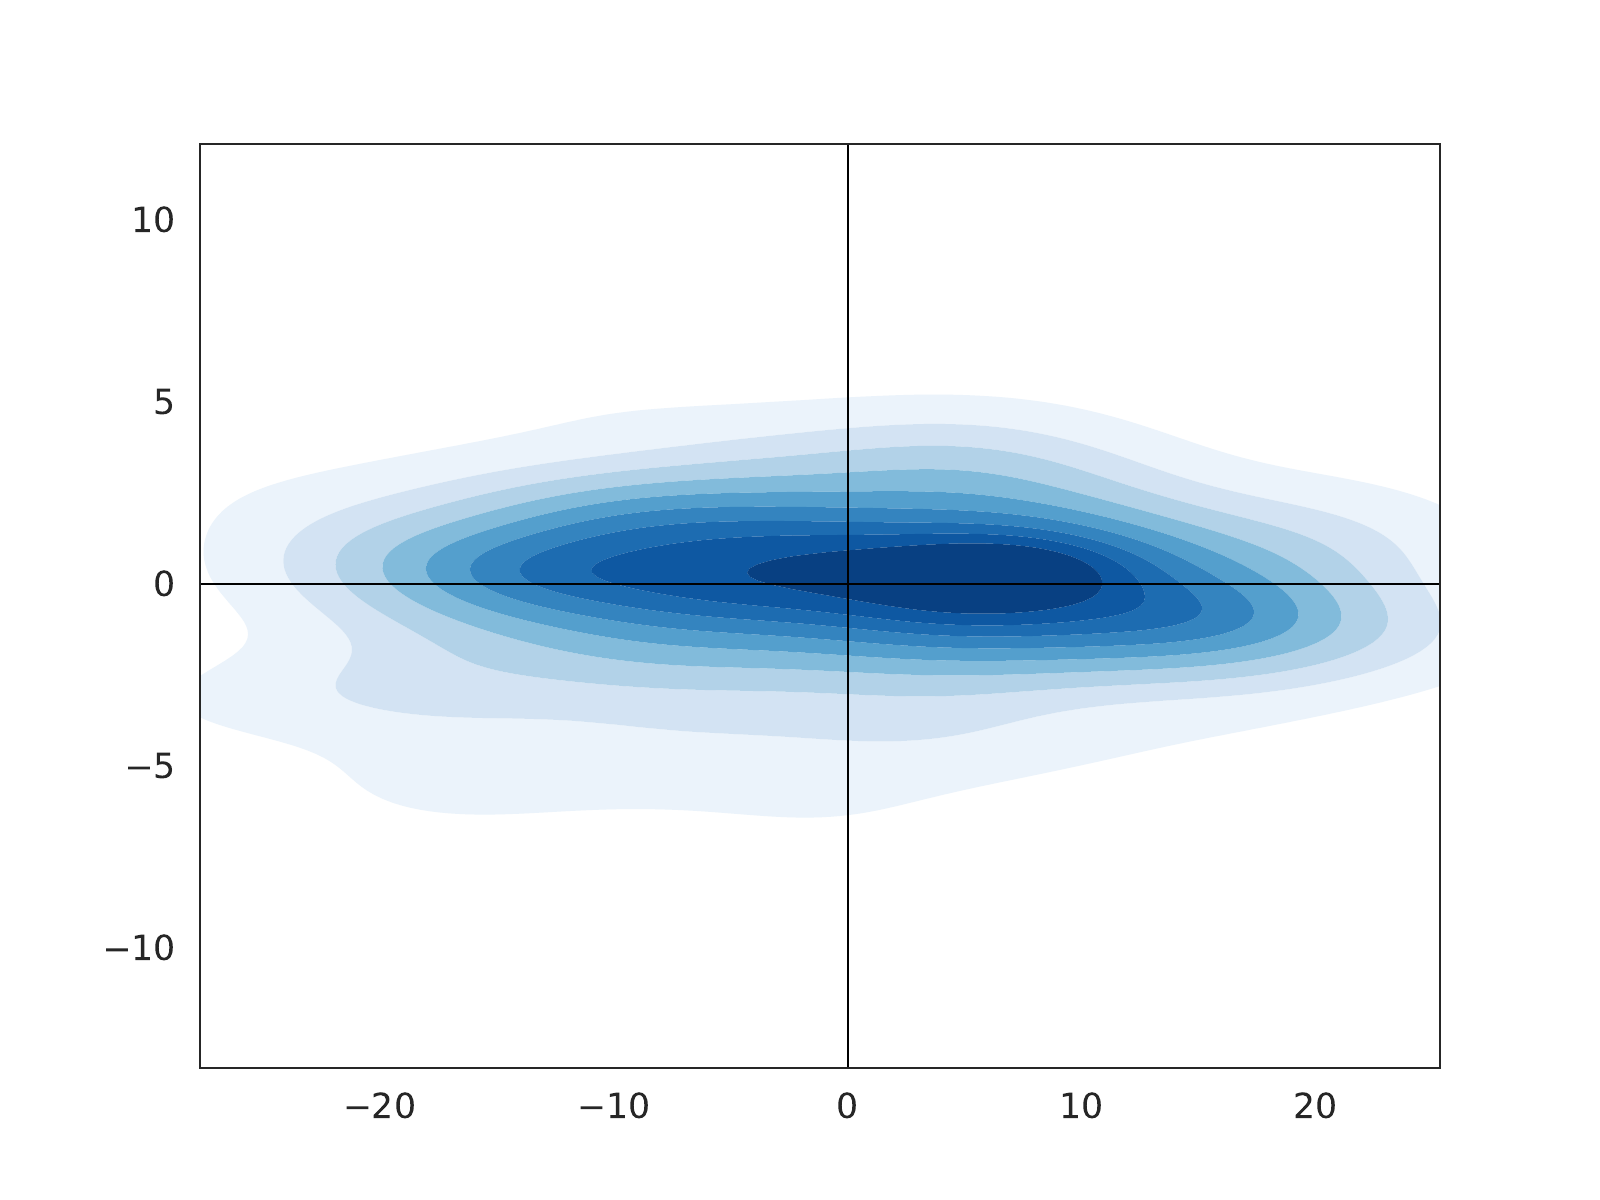} &
         \includegraphics[trim=60 80 60 80,clip,width=0.2\columnwidth]{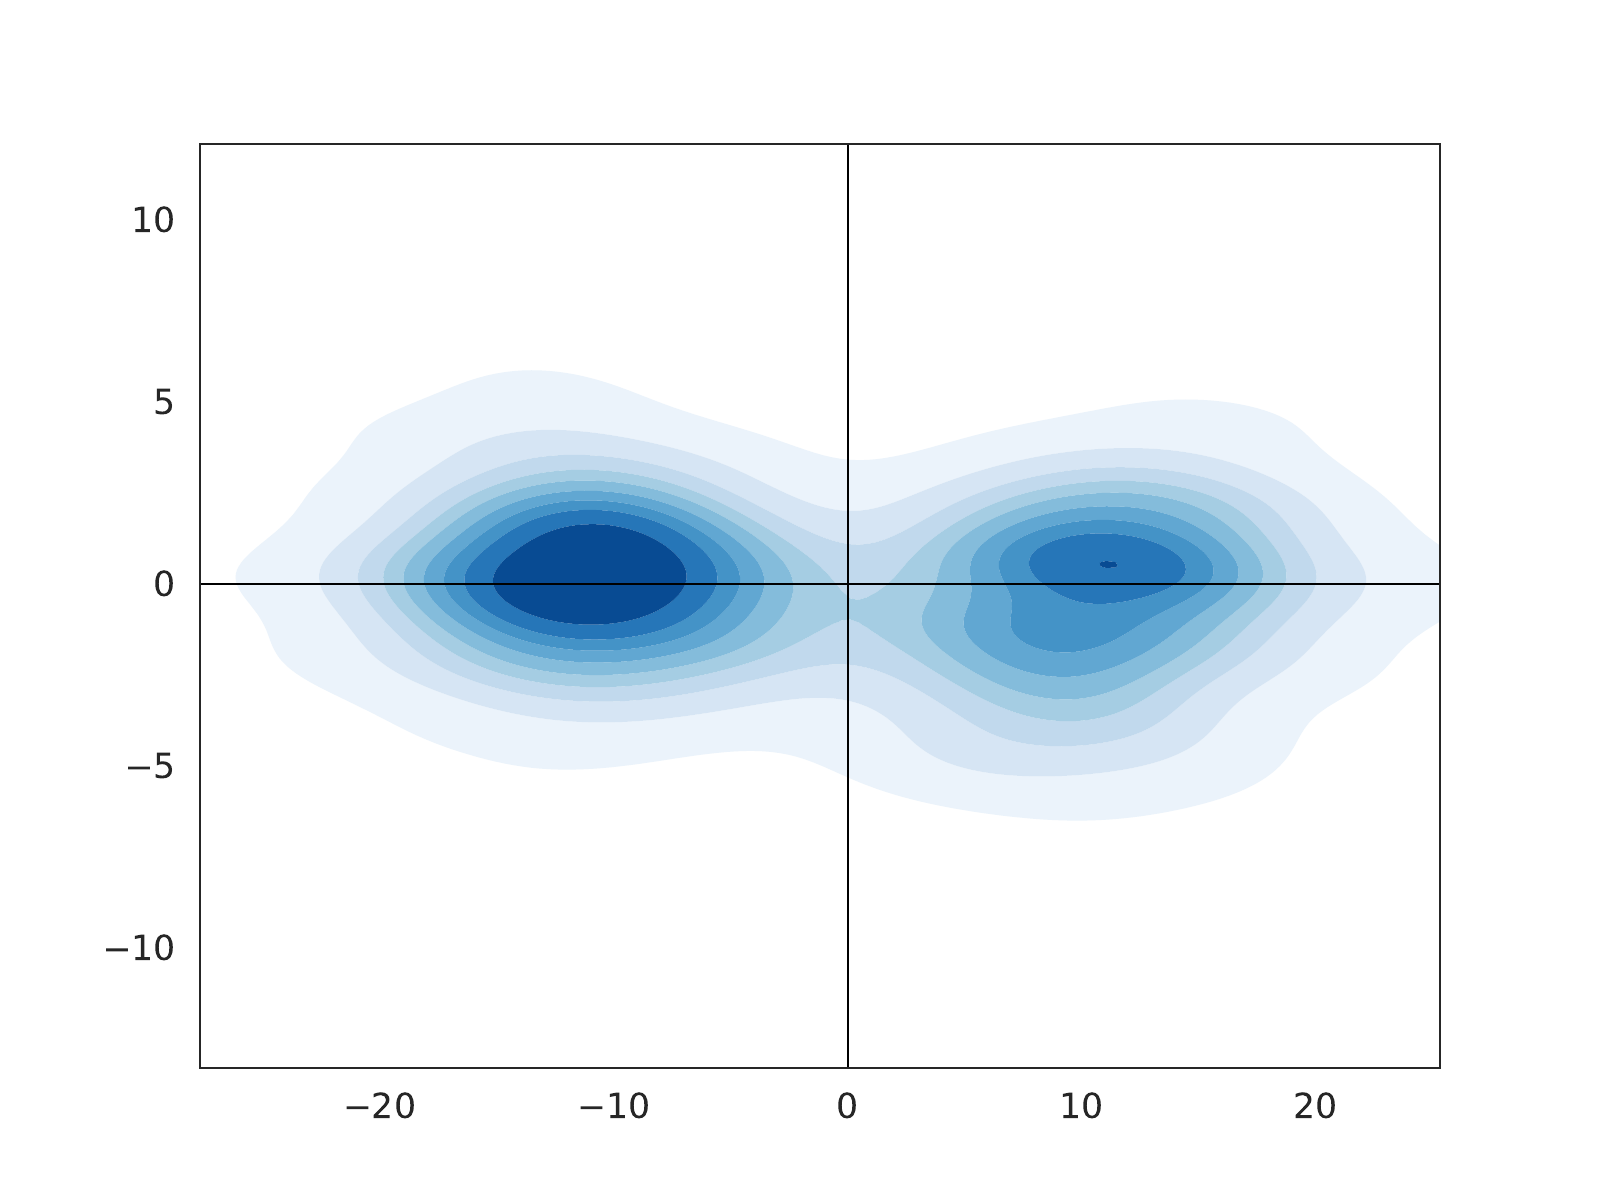} &
         \includegraphics[trim=60 80 60 80,clip,width=0.2\columnwidth]{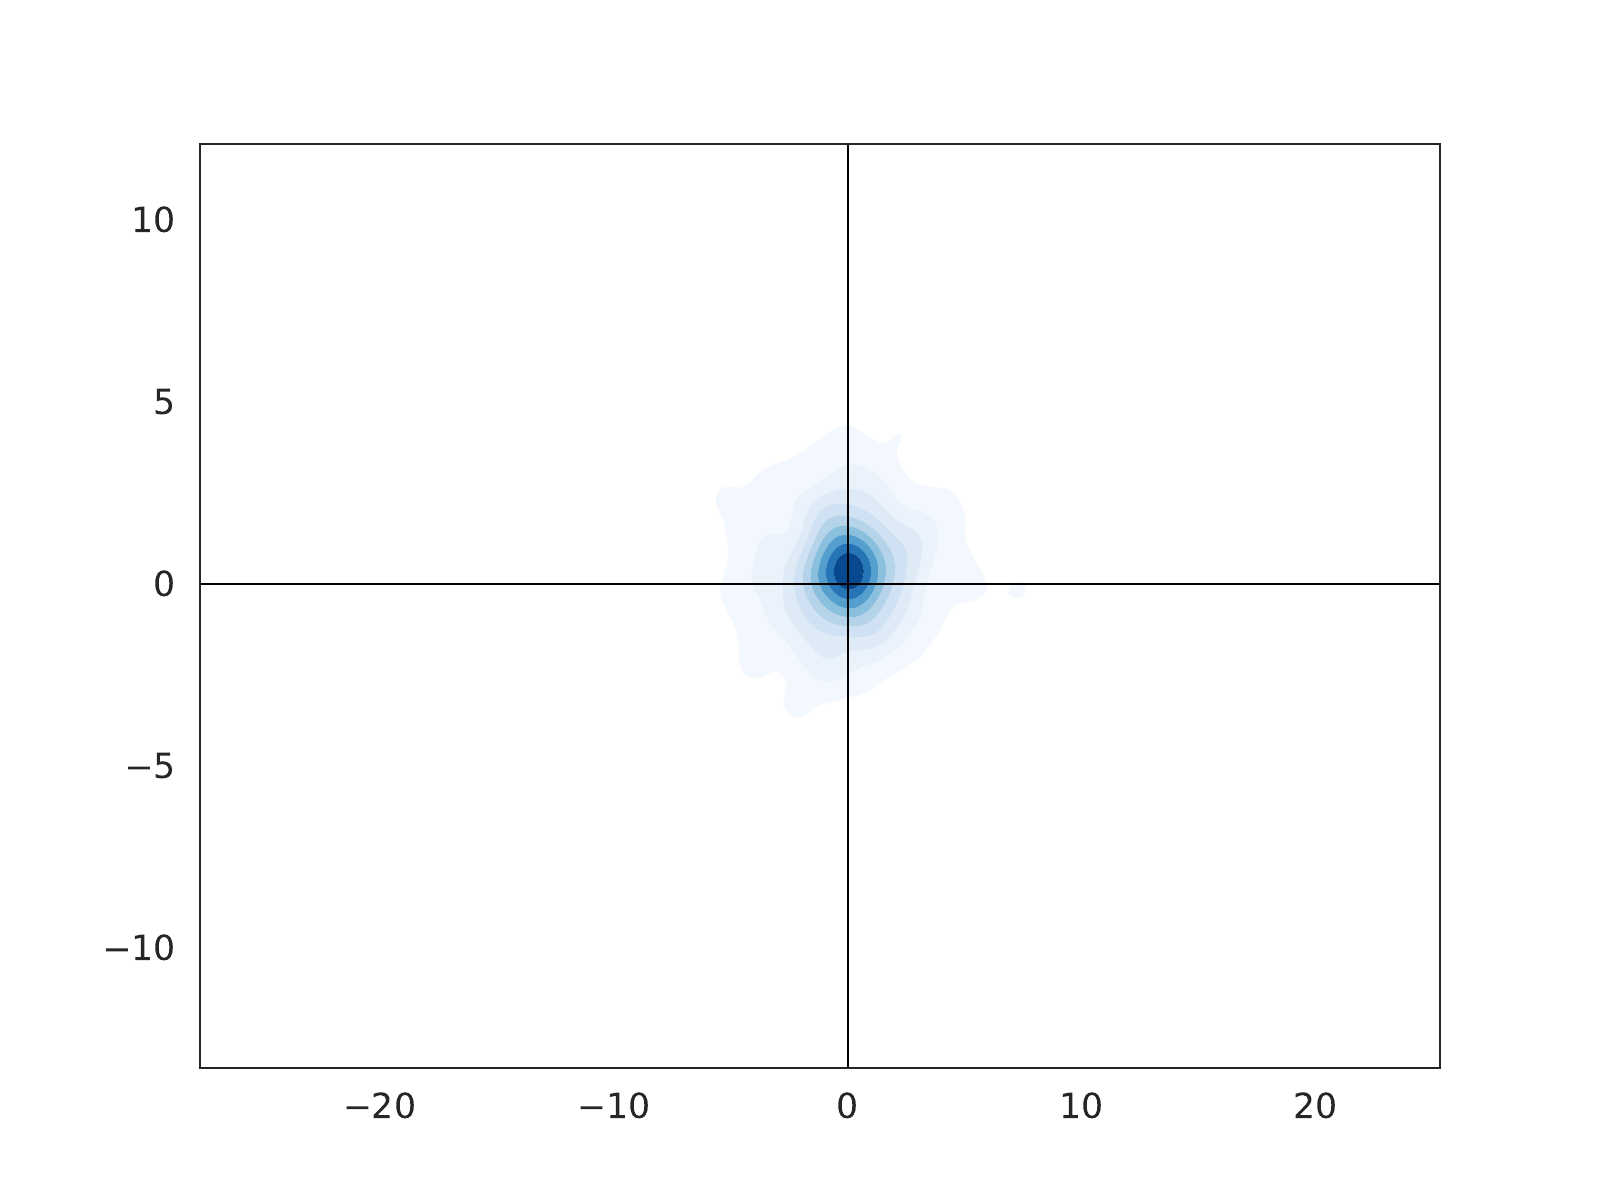} \\
         
         \rotatebox{90}{\hspace{2.5mm}SAVP+} &
         \includegraphics[trim=60 80 60 80,clip,width=0.2\columnwidth]{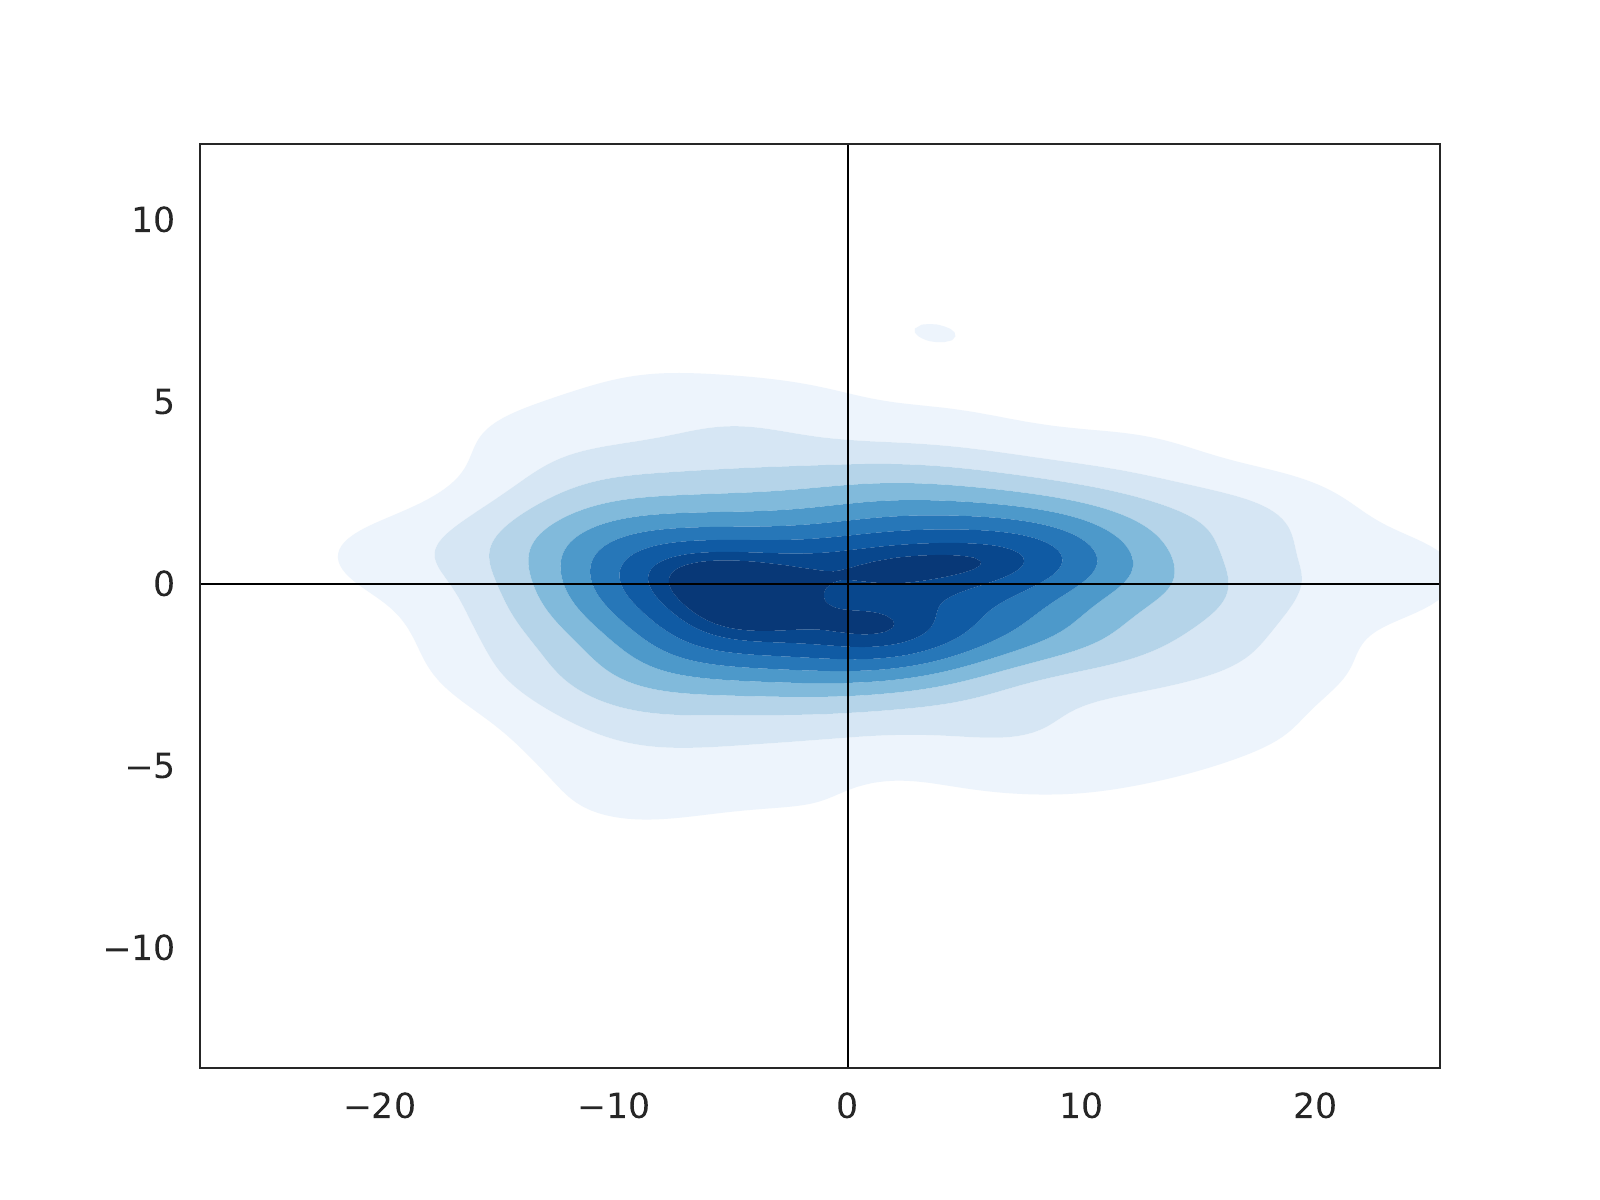} &
         \includegraphics[trim=60 80 60 80,clip,width=0.2\columnwidth]{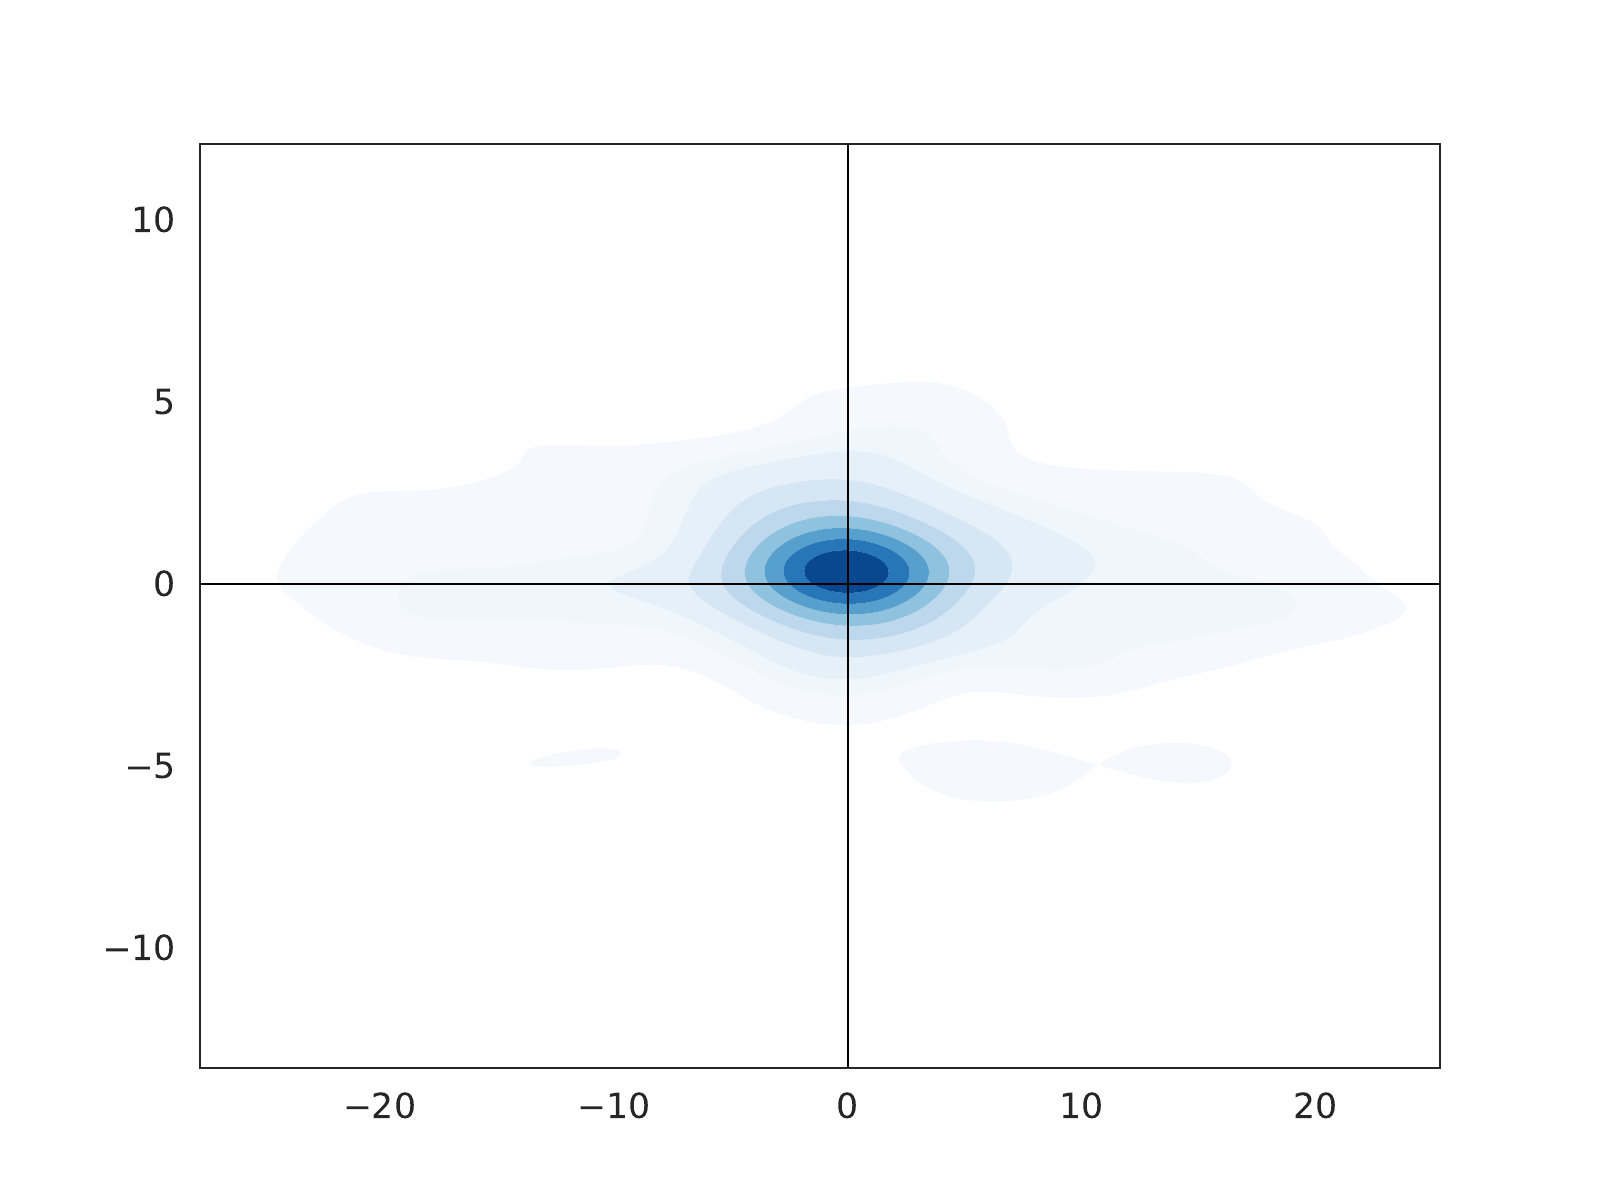} &
         \includegraphics[trim=60 80 60 80,clip,width=0.2\columnwidth]{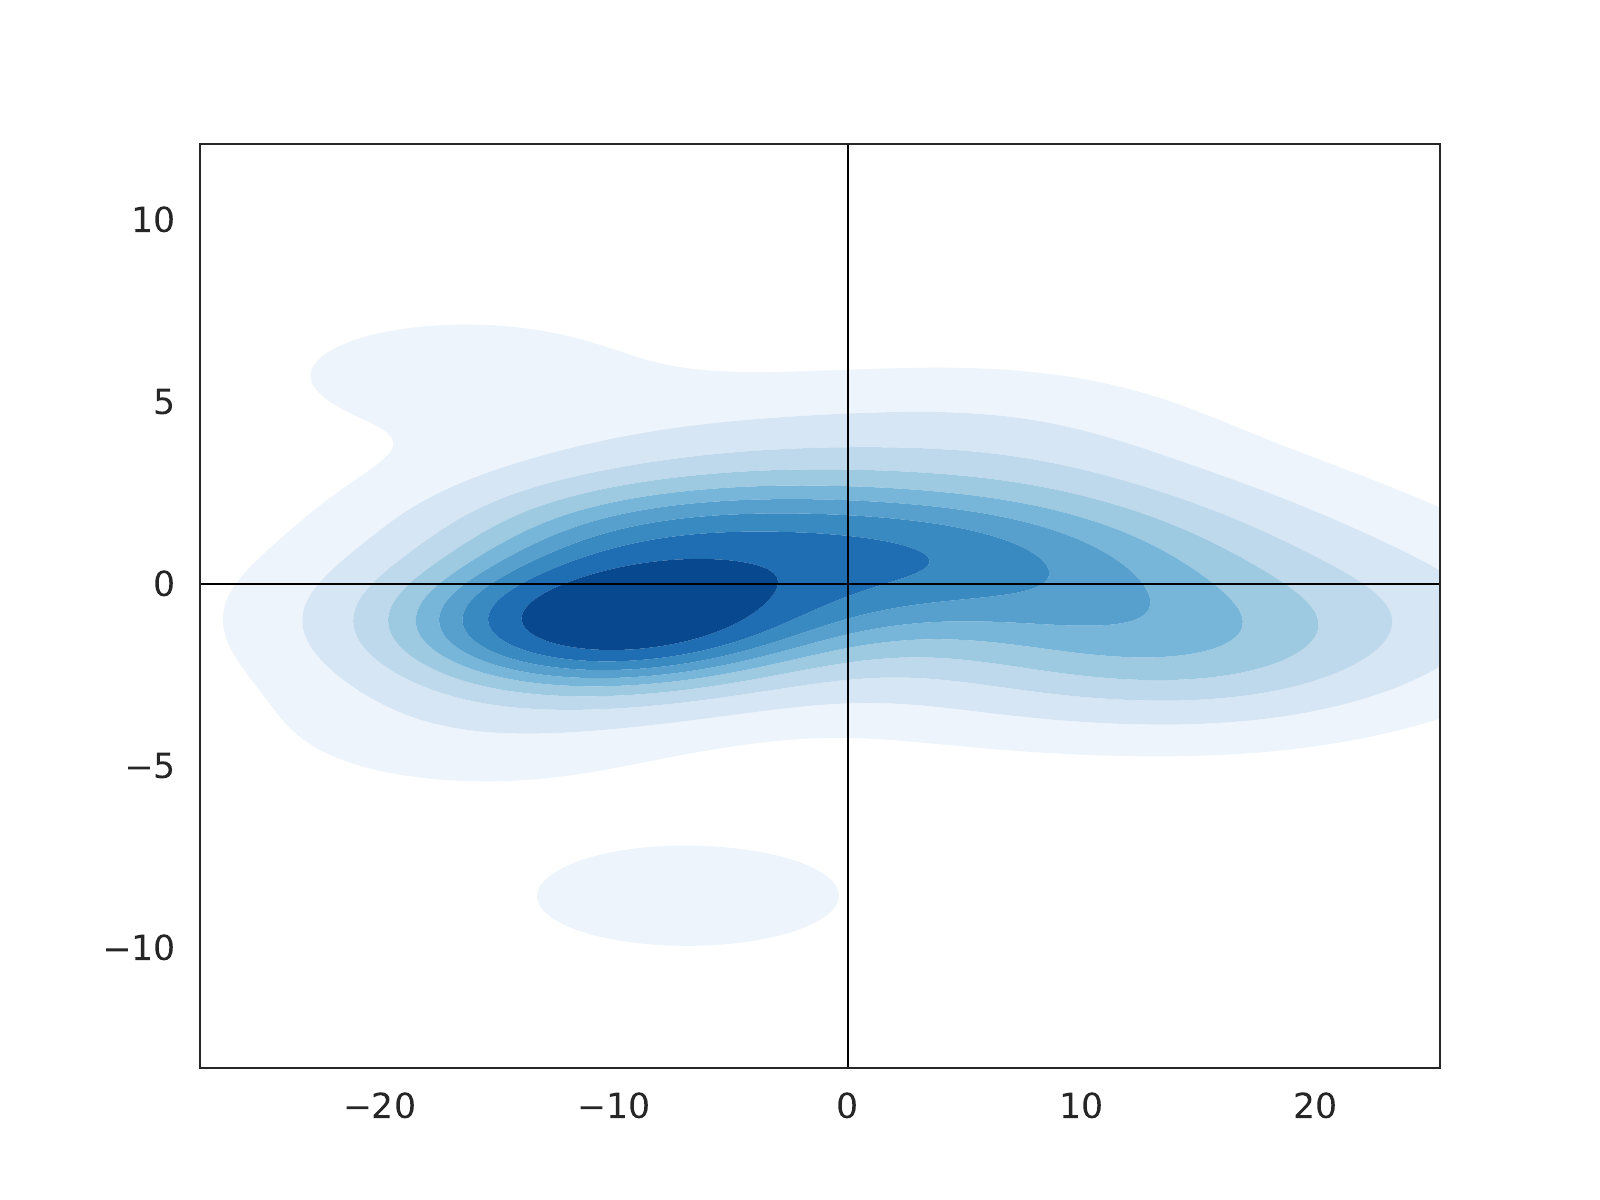} &
         \includegraphics[trim=60 80 60 80,clip,width=0.2\columnwidth]{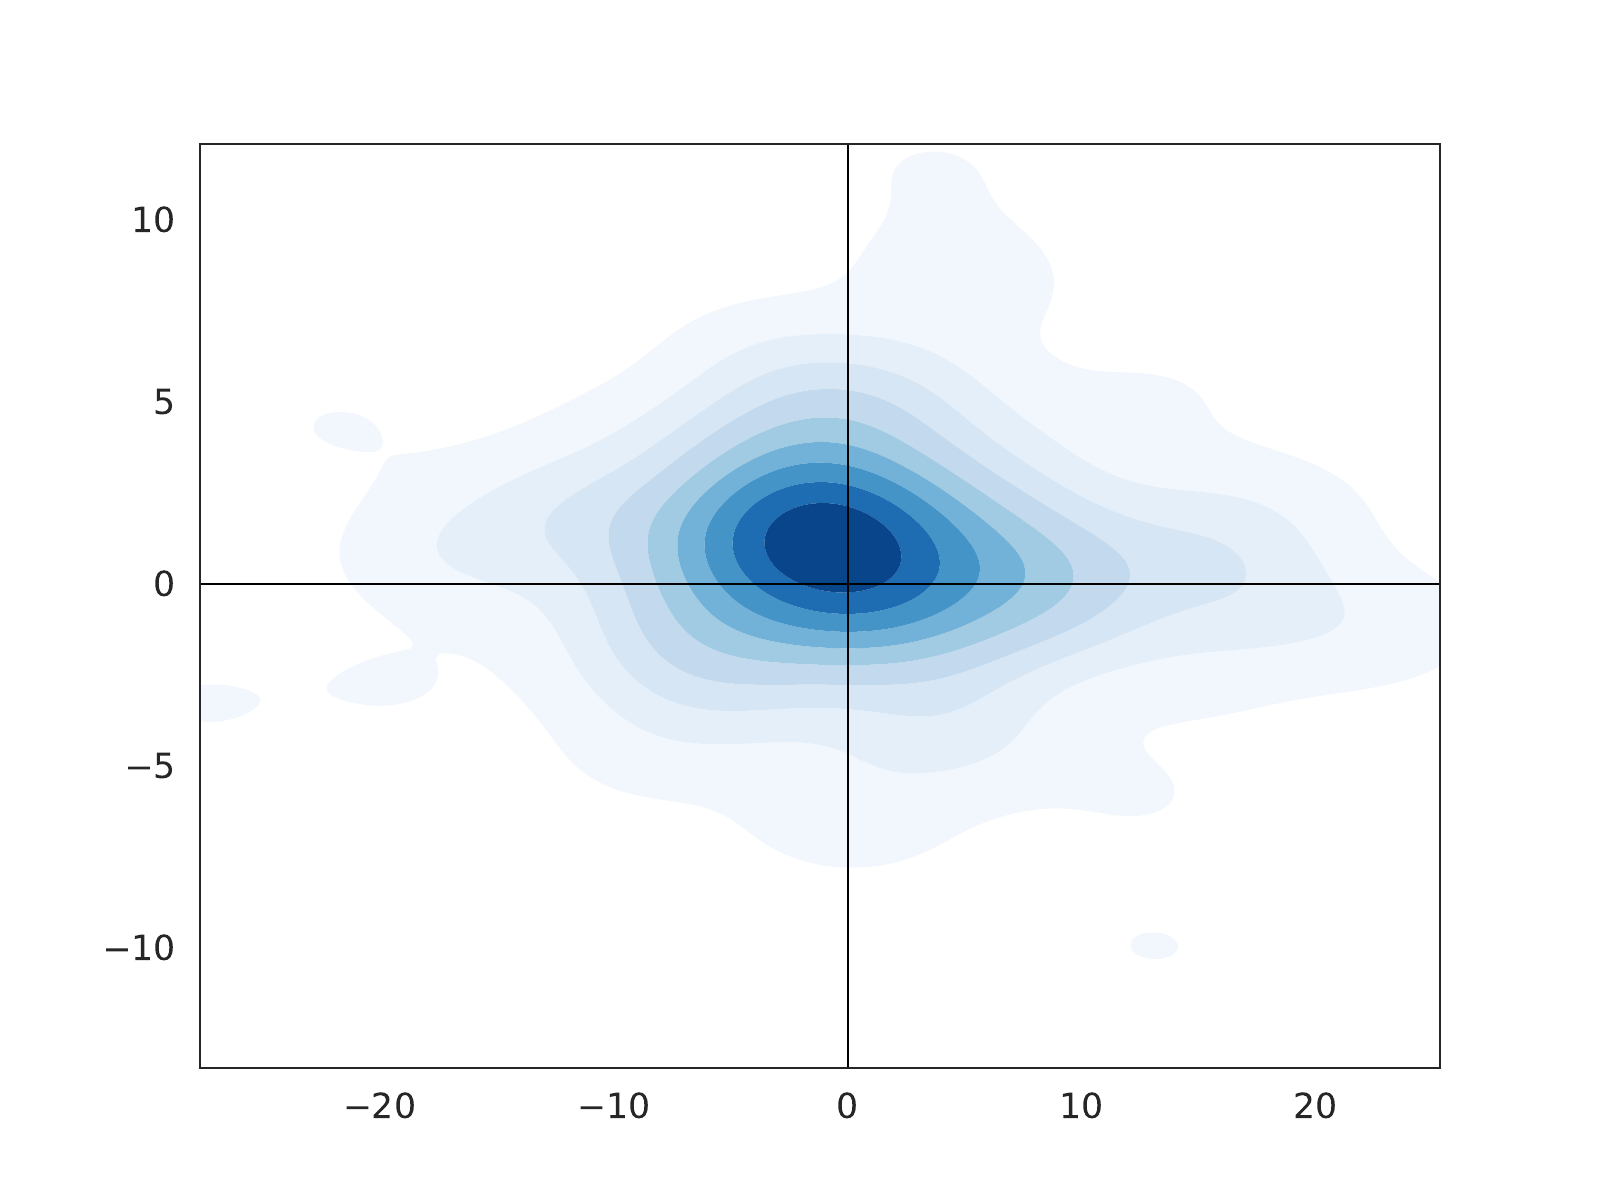} &
         \includegraphics[trim=60 80 60 80,clip,width=0.2\columnwidth]{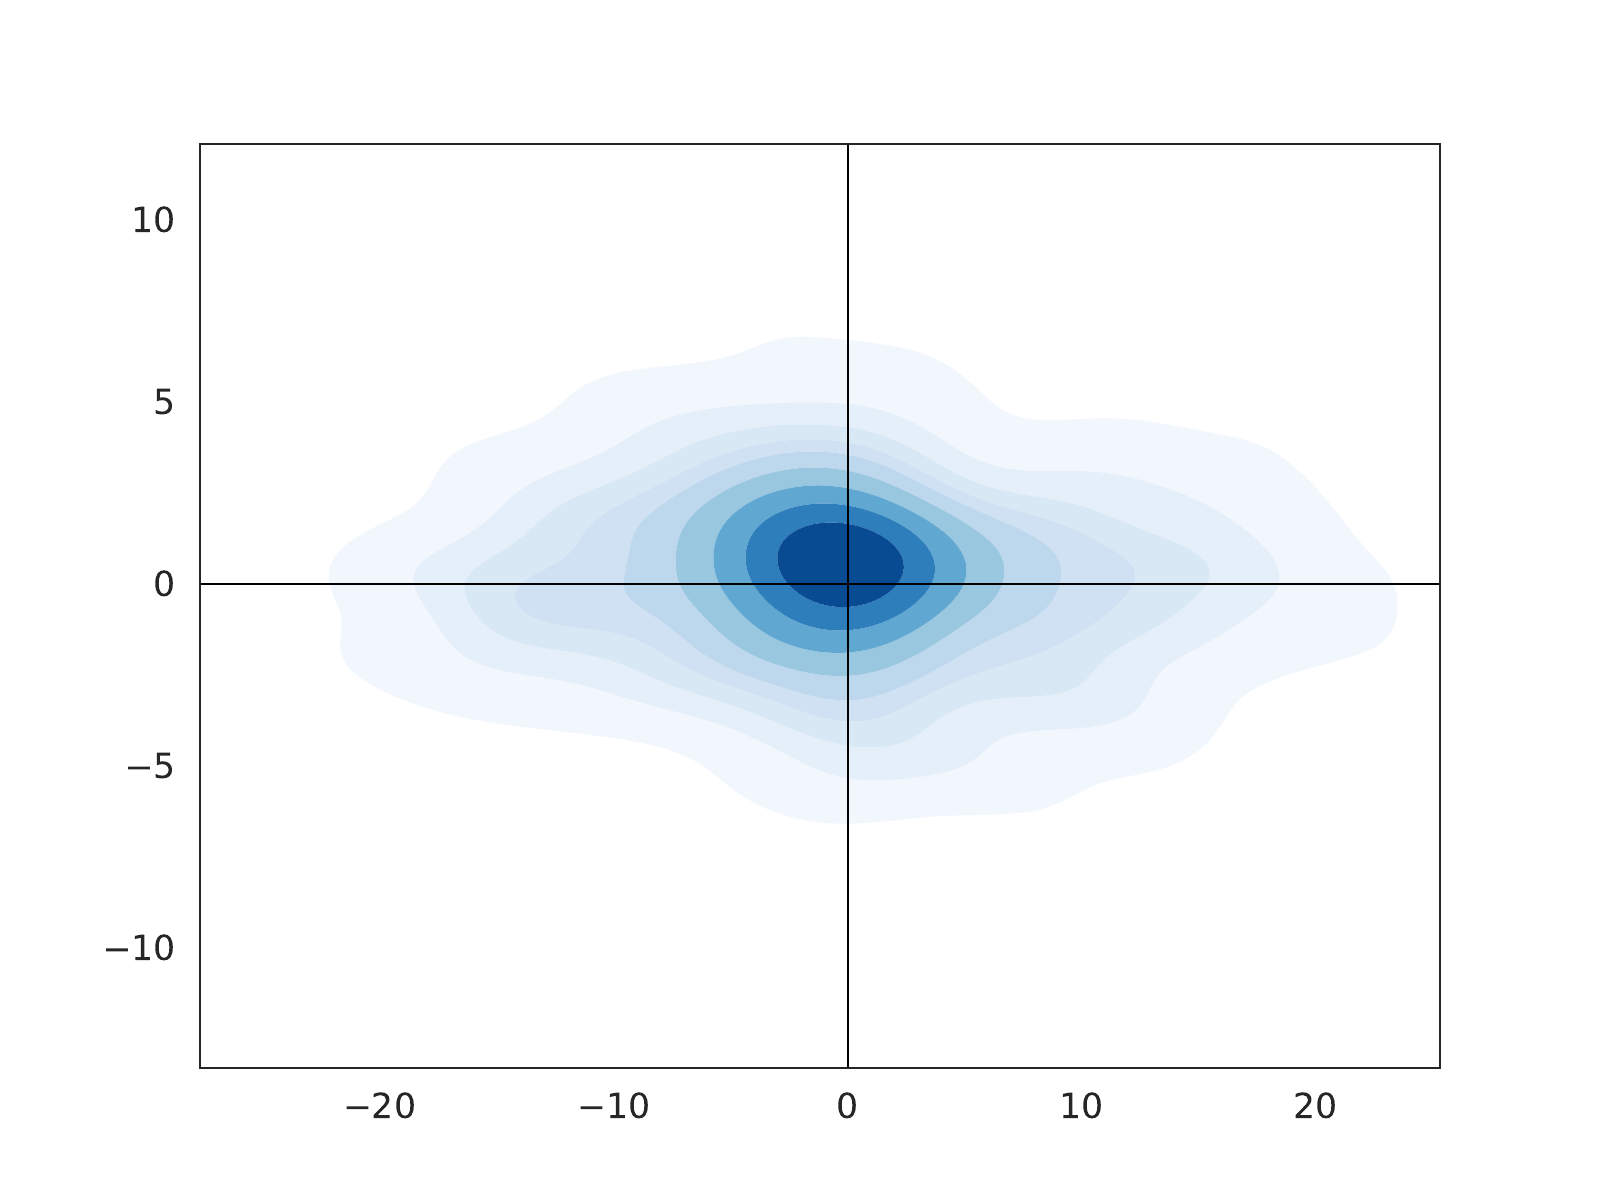} &
         \includegraphics[trim=60 80 60 80,clip,width=0.2\columnwidth]{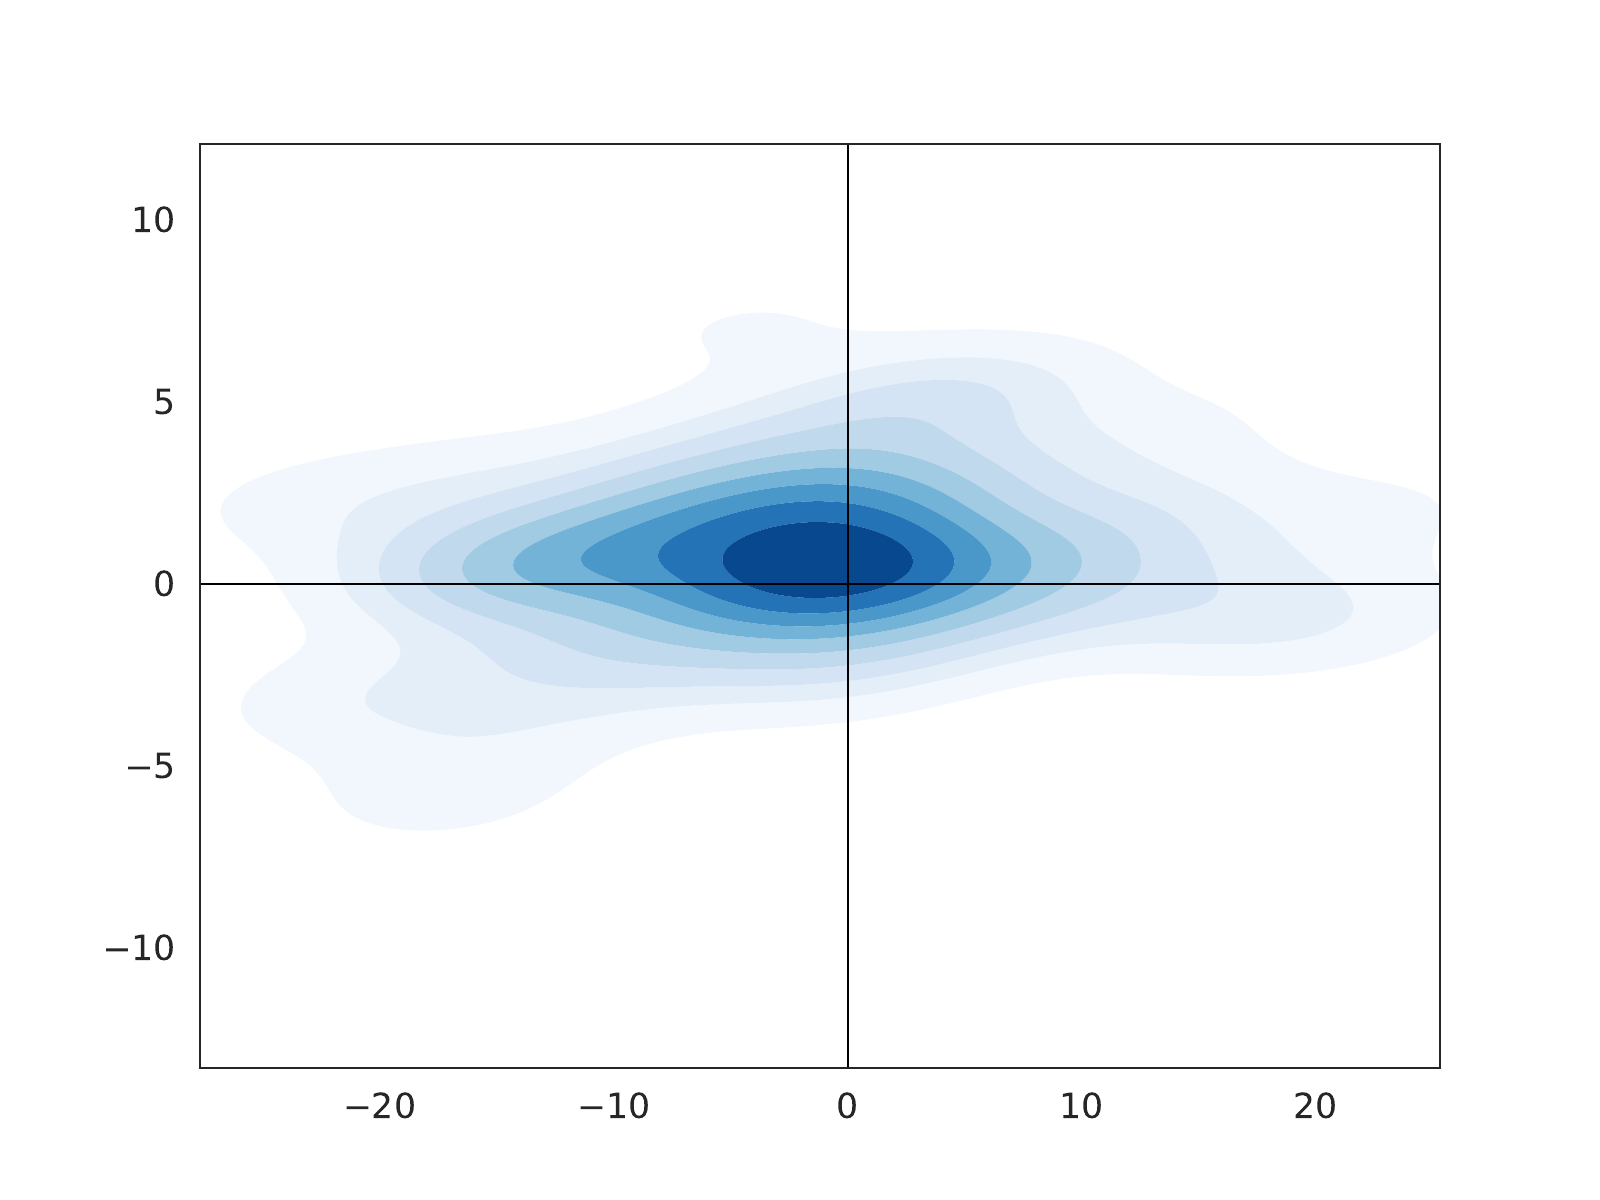} &
         \includegraphics[trim=60 80 60 80,clip,width=0.2\columnwidth]{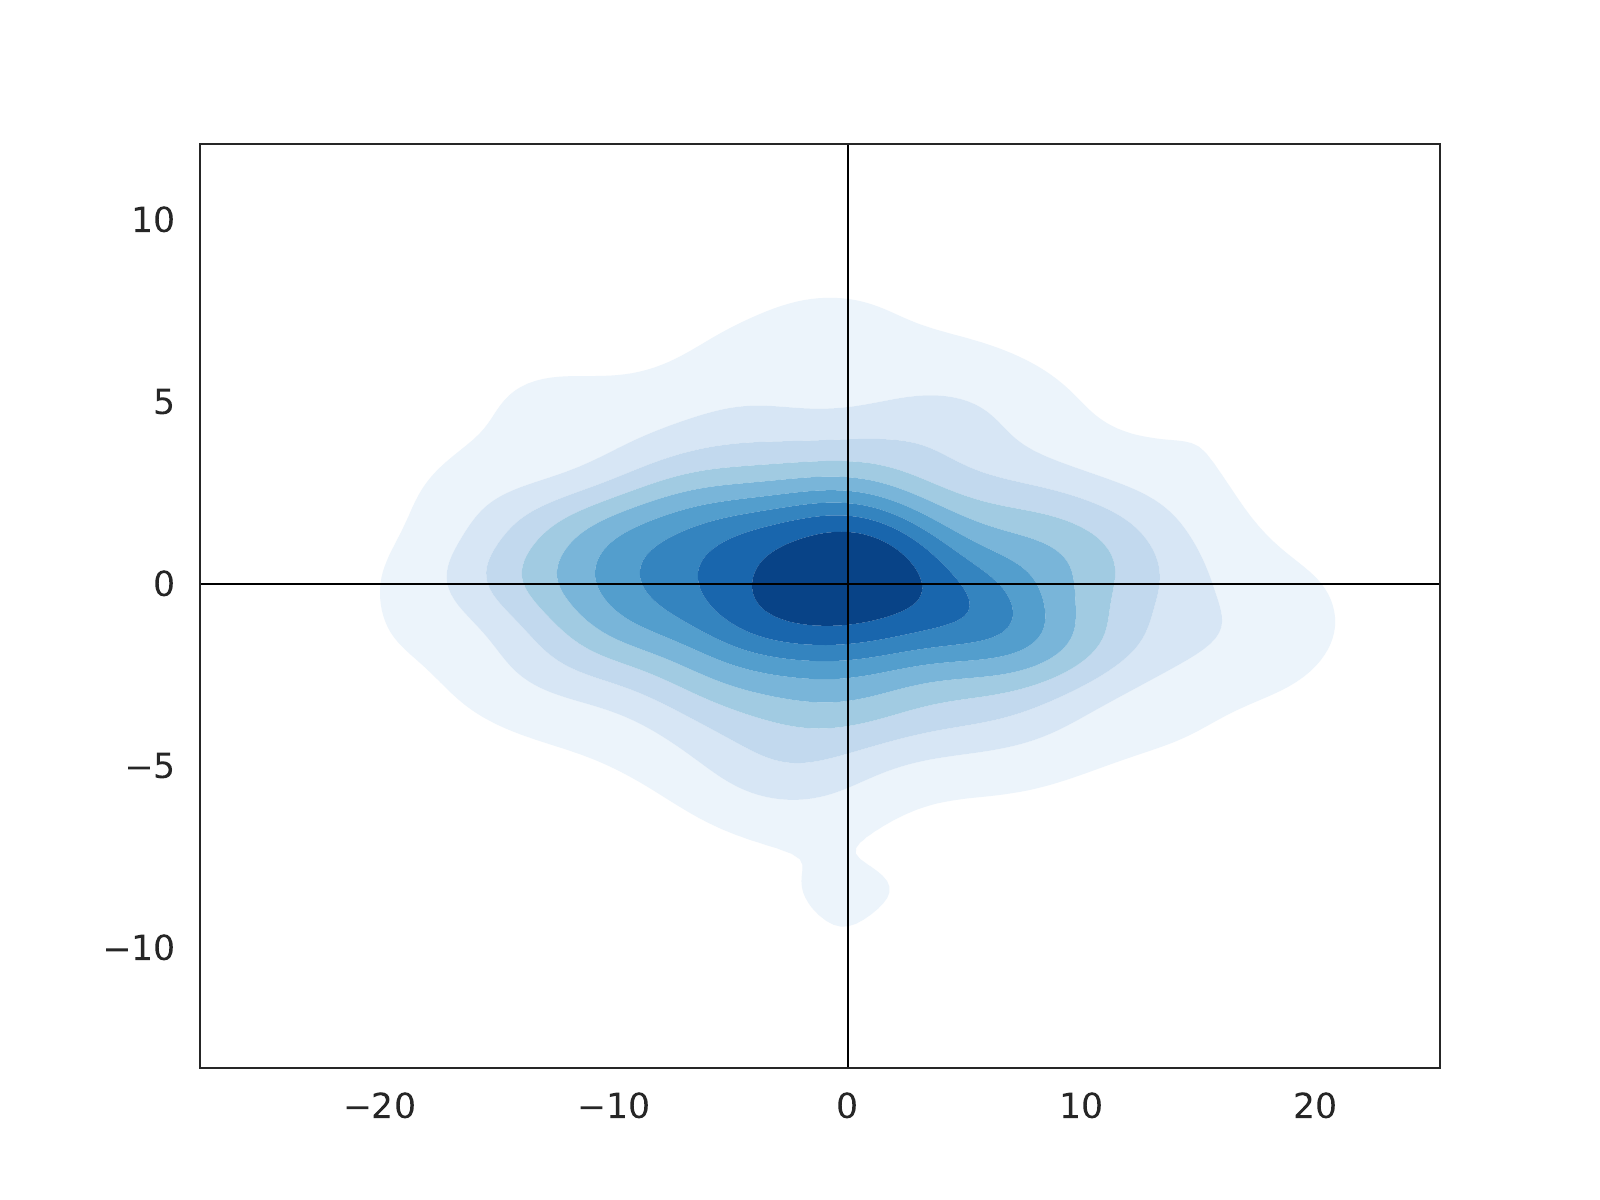} \\
         
         \rotatebox{90}{\hspace{3mm}Ours} &
         \includegraphics[trim=60 80 60 80,clip,width=0.2\columnwidth]{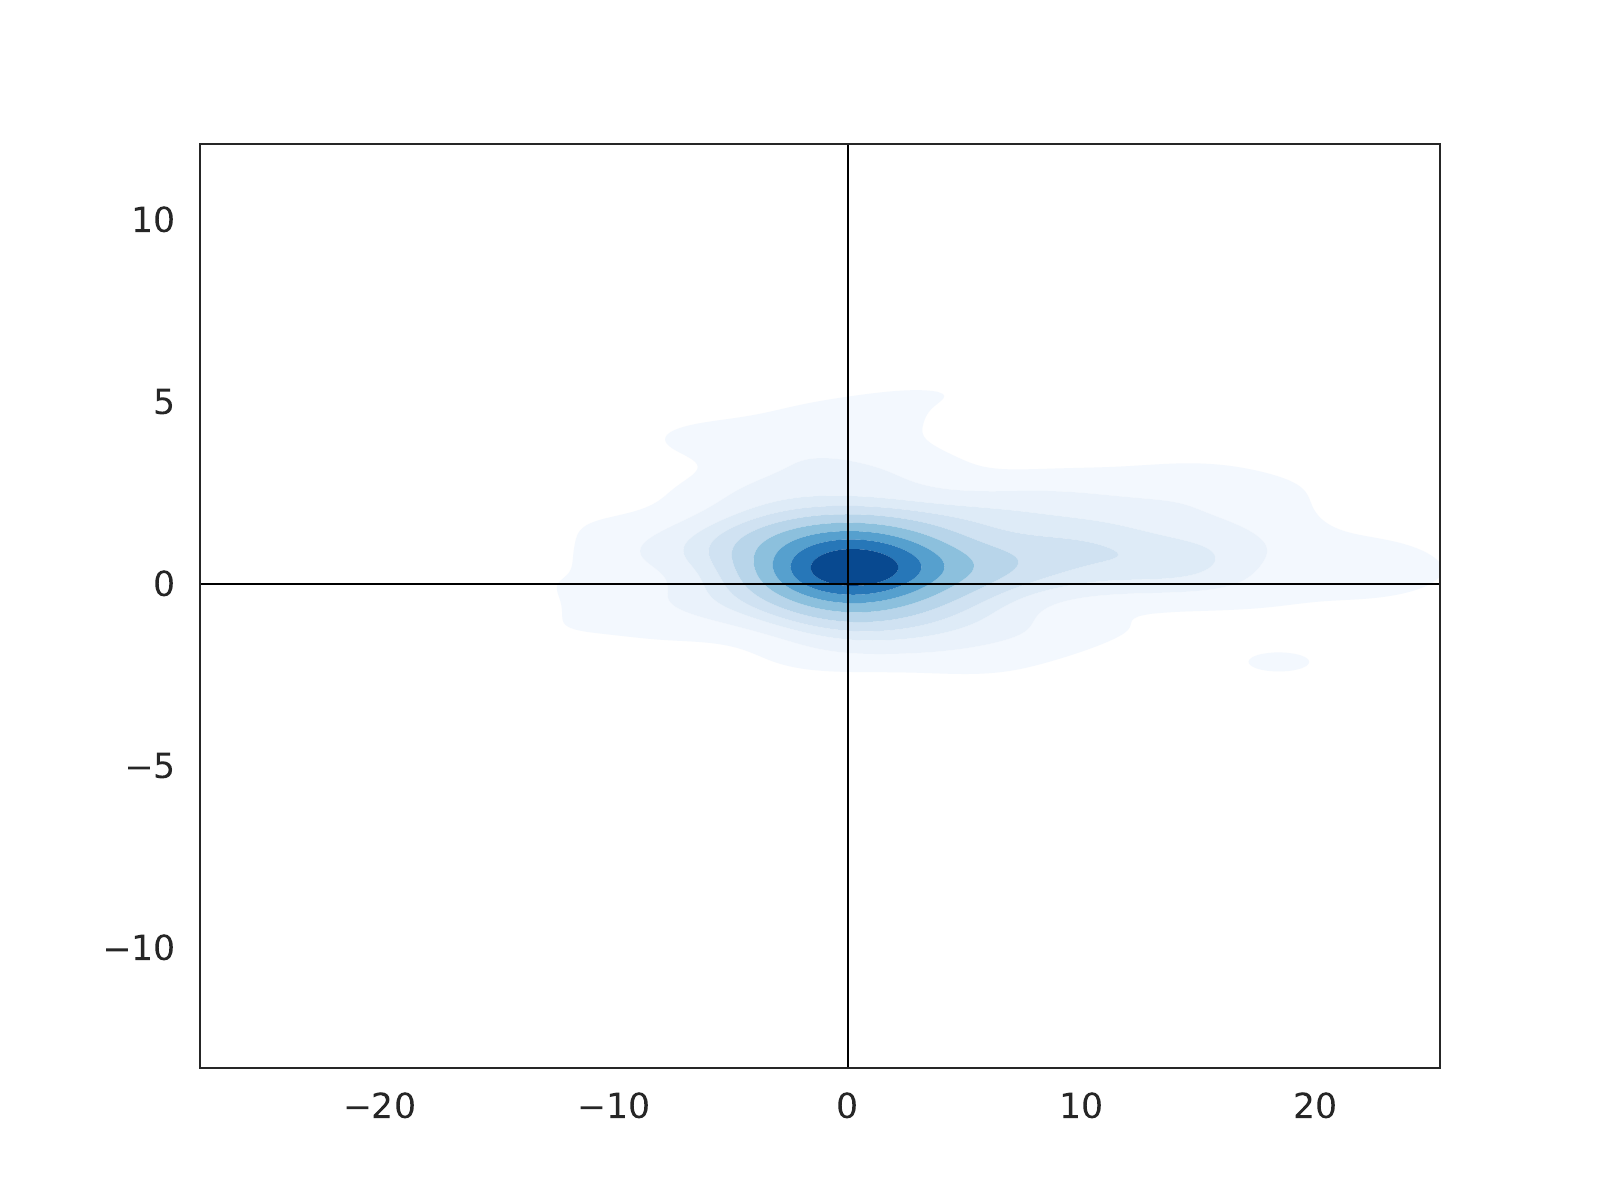} &
         \includegraphics[trim=60 80 60 80,clip,width=0.2\columnwidth]{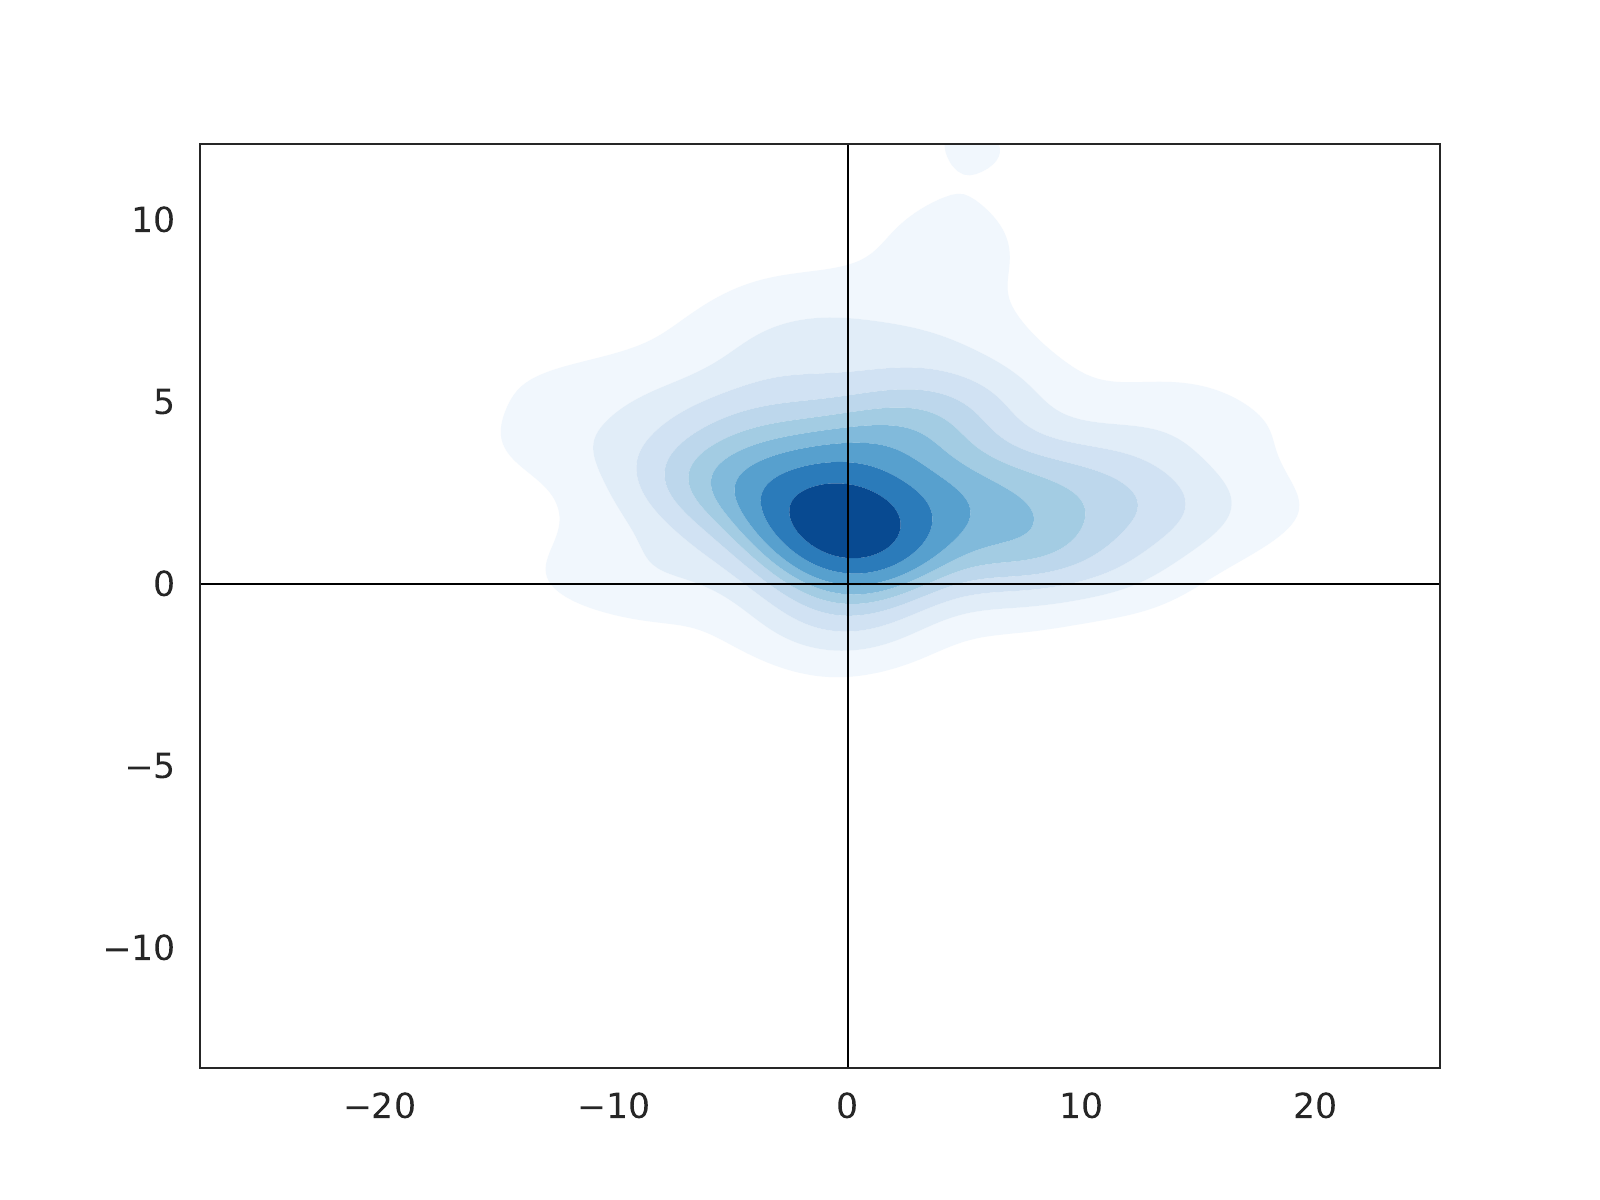} &
         \includegraphics[trim=60 80 60 80,clip,width=0.2\columnwidth]{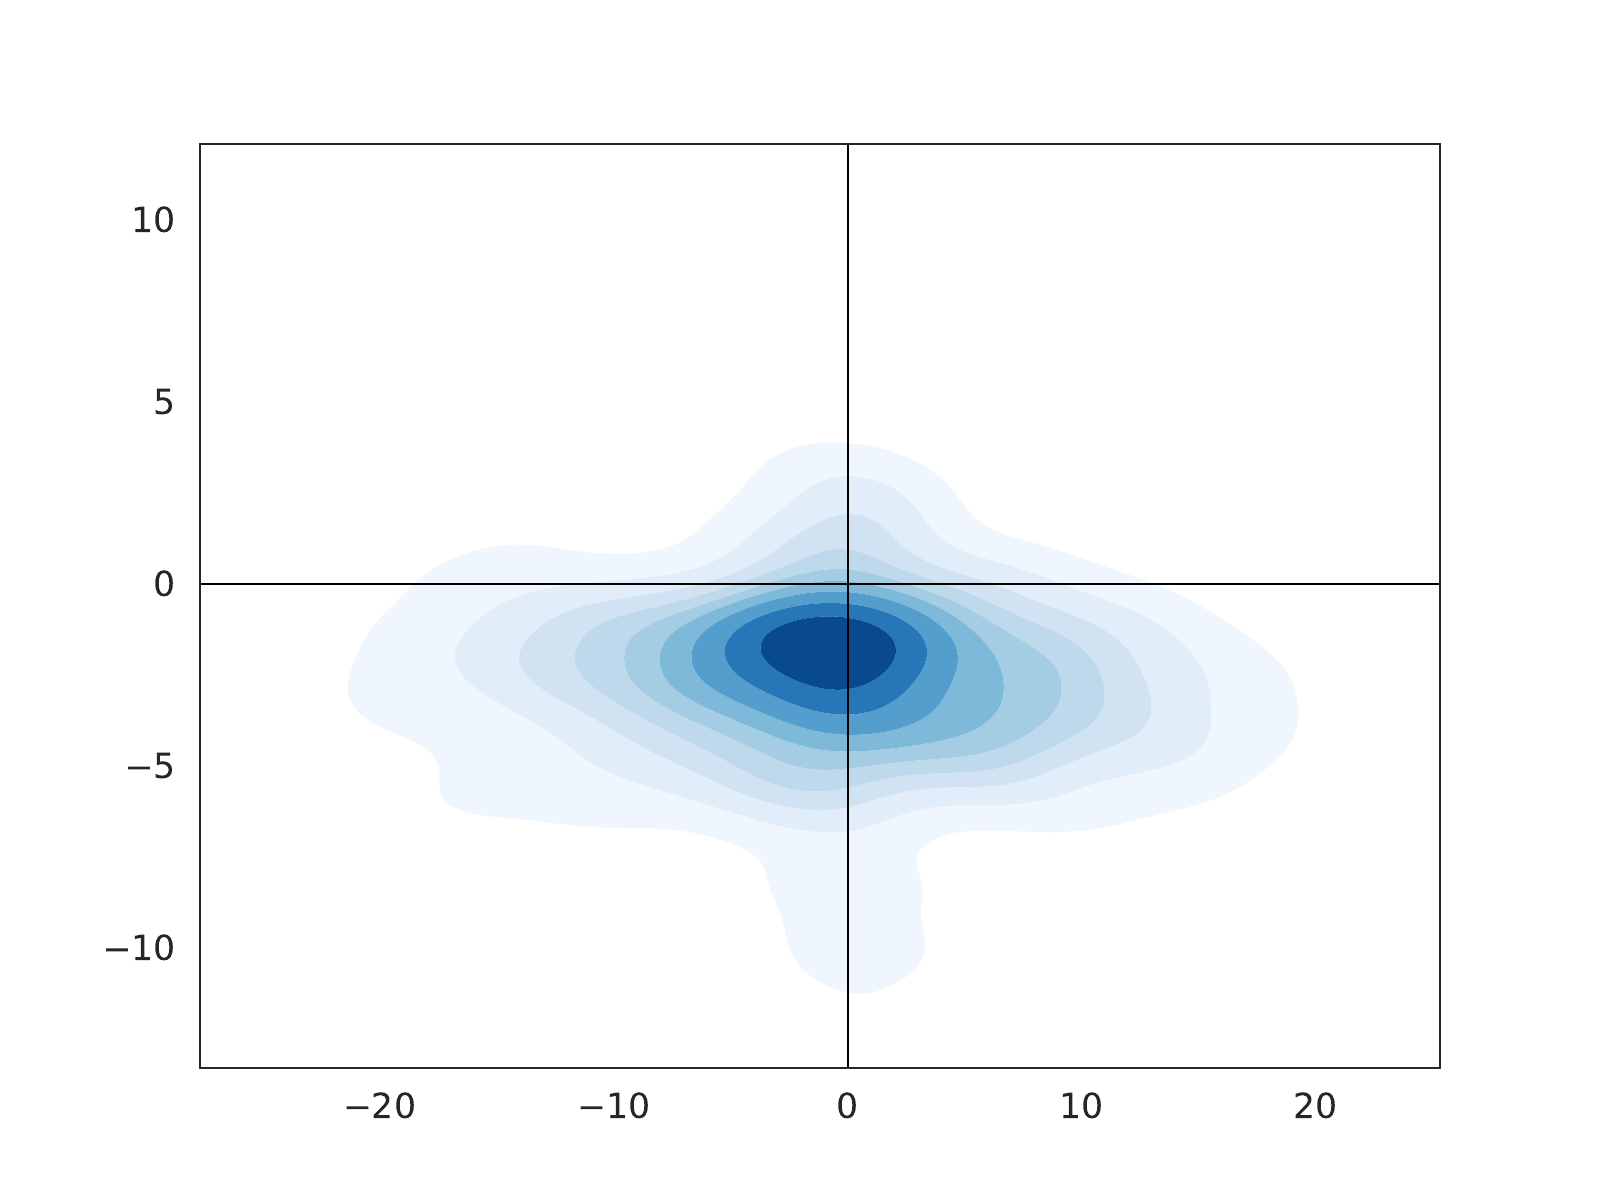} &
         \includegraphics[trim=60 80 60 80,clip,width=0.2\columnwidth]{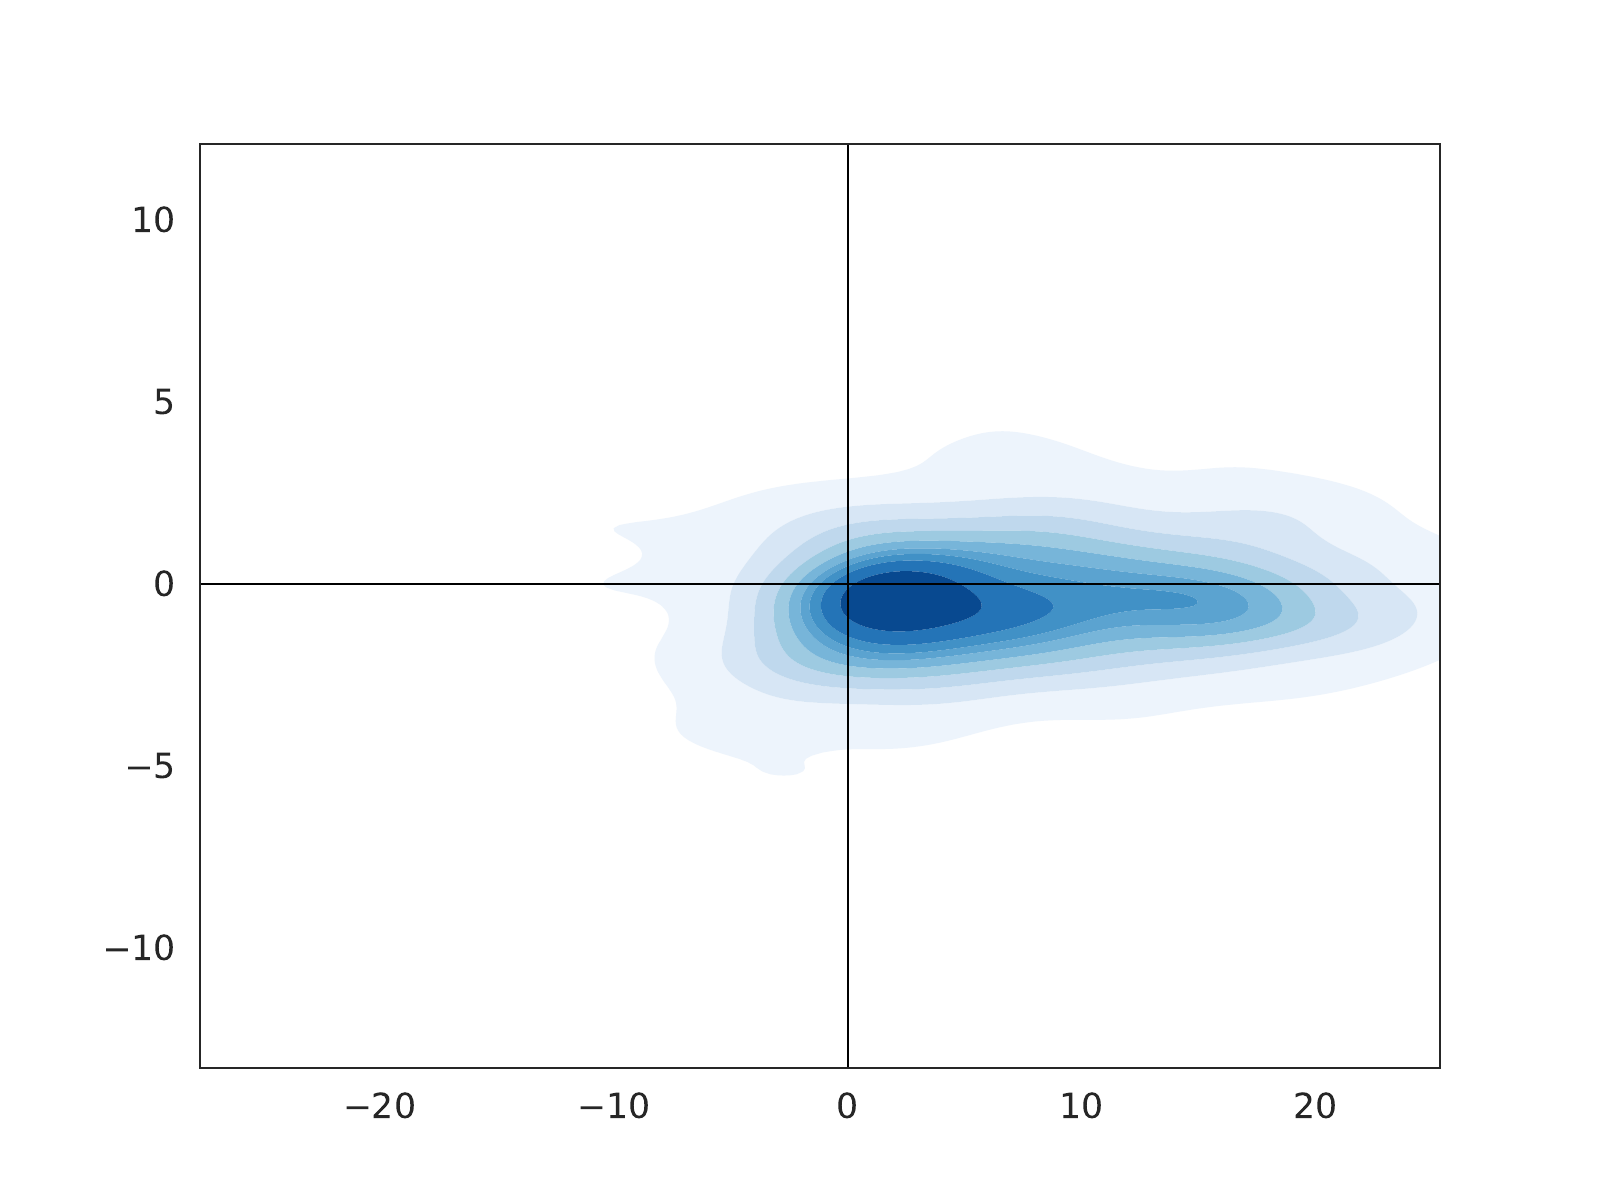} &
         \includegraphics[trim=60 80 60 80,clip,width=0.2\columnwidth]{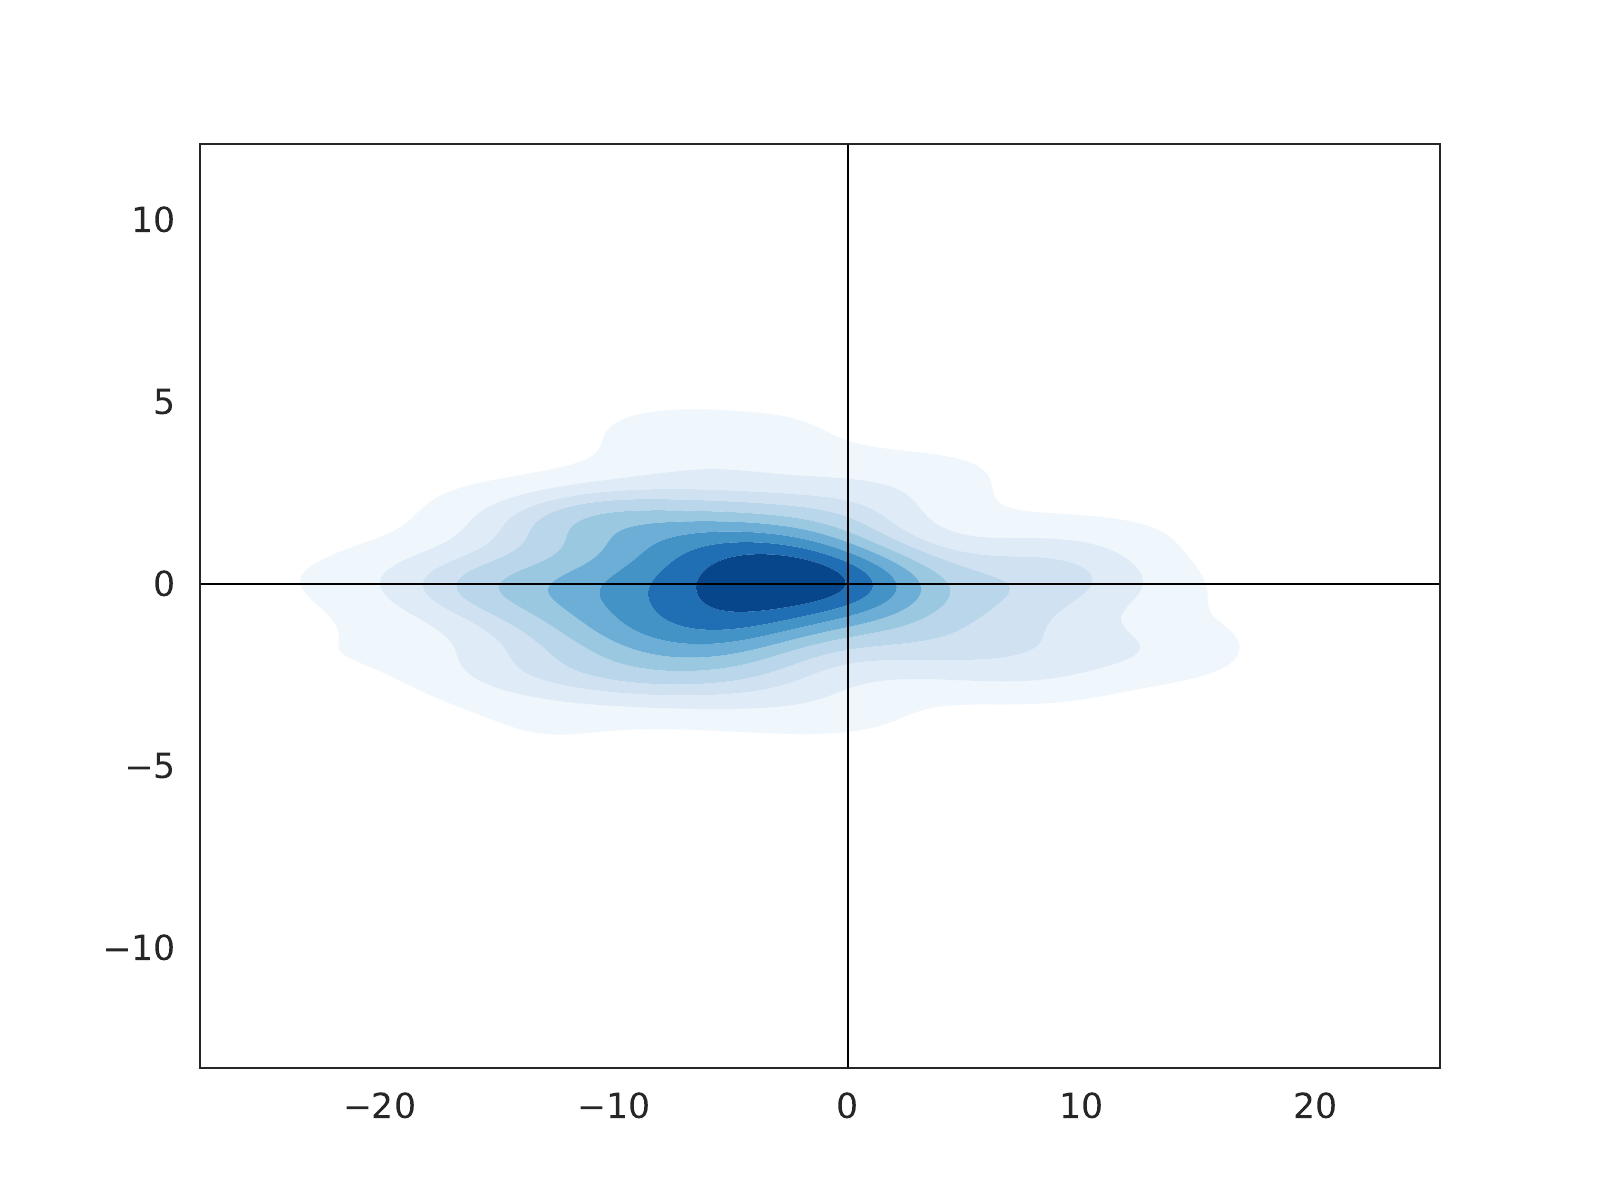} &
         \includegraphics[trim=60 80 60 80,clip,width=0.2\columnwidth]{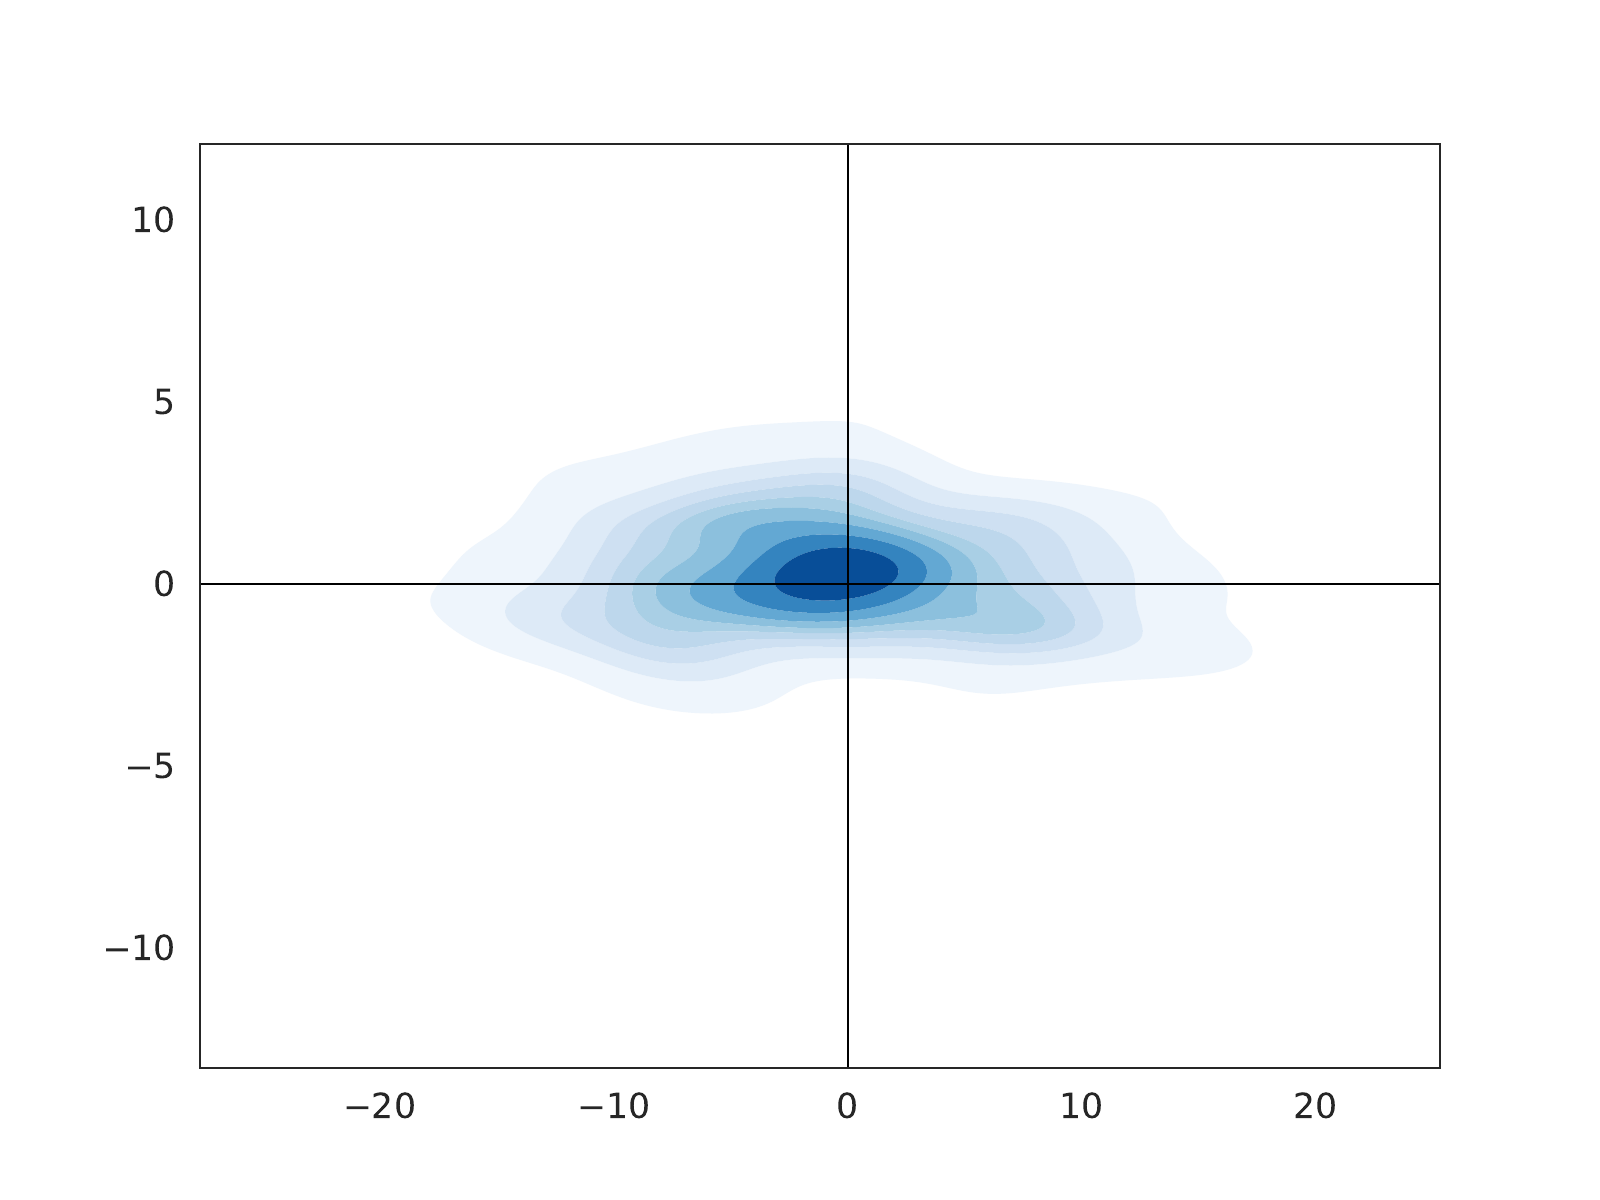} &
         \includegraphics[trim=60 80 60 80,clip,width=0.2\columnwidth]{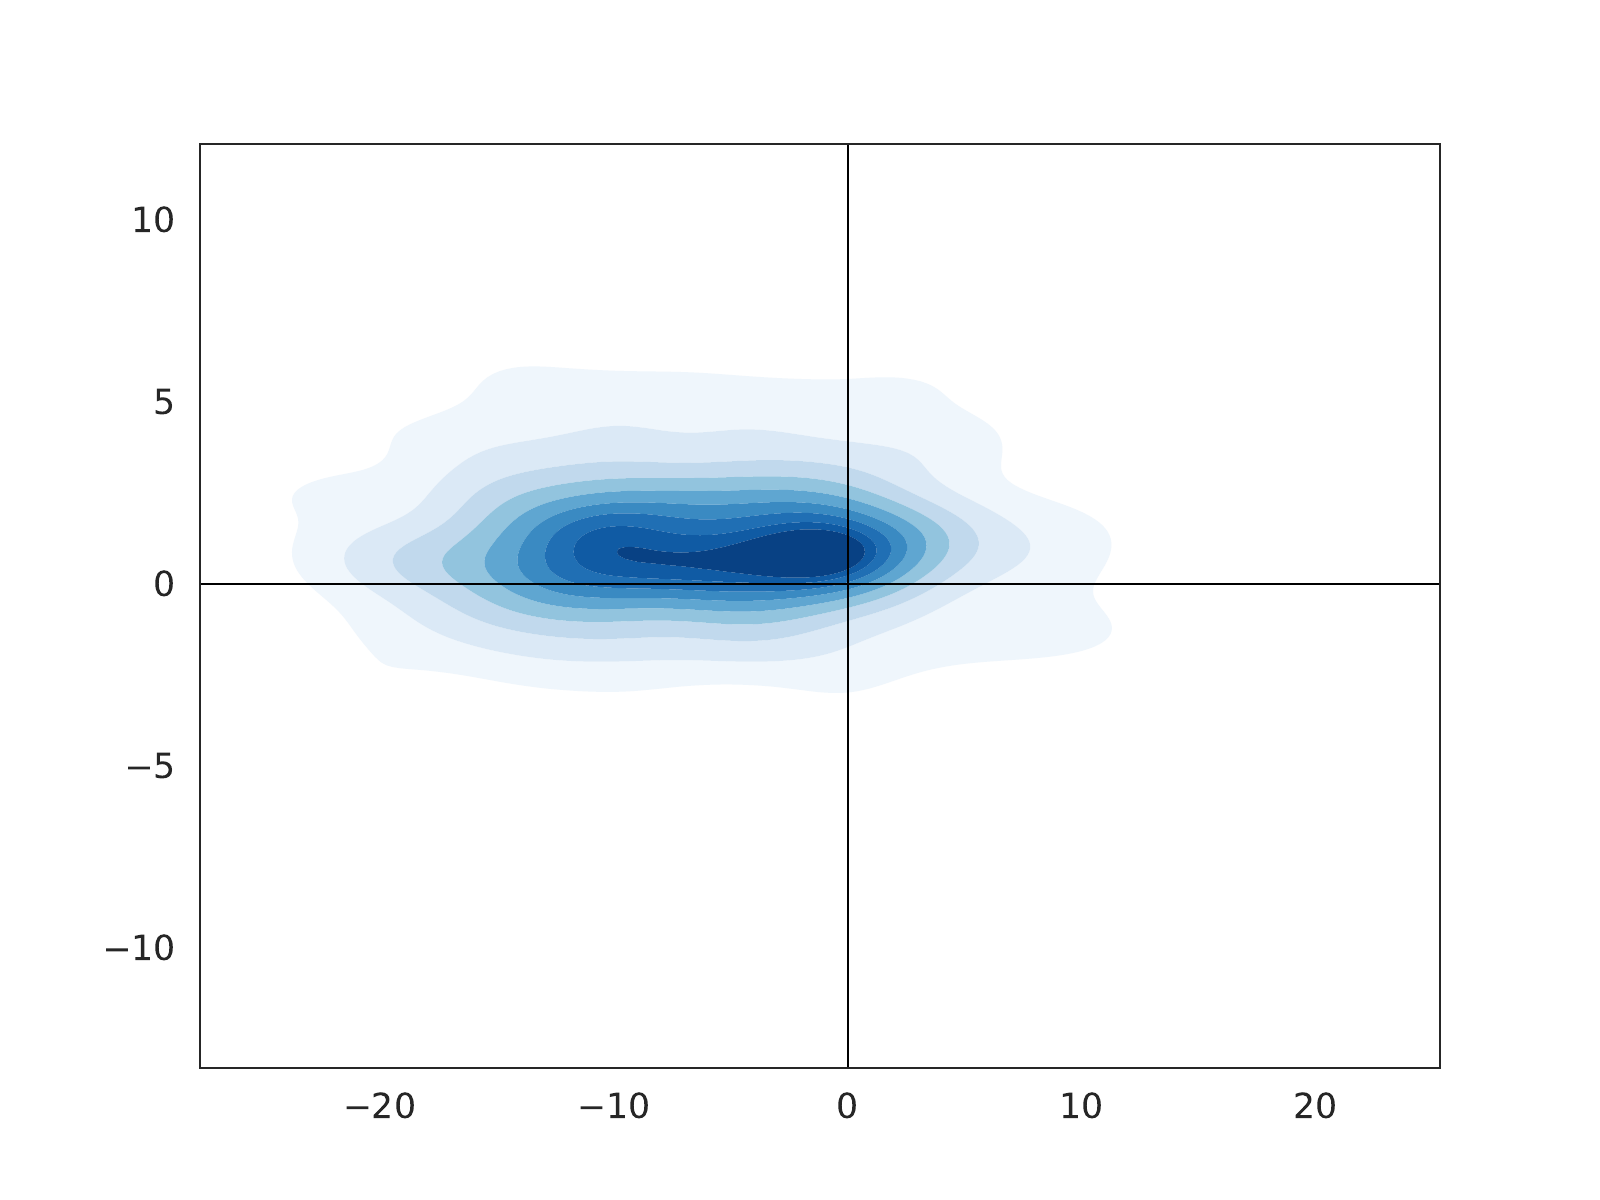} \\

    \end{tabular}
    }
    \captionof{figure}{Distribution of the displacement $\Delta$ associated with the player on the \emph{Tennis} dataset. Ideal distributions are different for each action and have low variance, meaning that they capture specific movements. Our model successfully conditions the movement of the player on the action, while the other baselines show limited conditioning capabilities.}
    \label{fig:tennis_density_plots}
\end{table*}
