# Supplementary material for: Playable Video Generation
Source: arXiv:2101.12195 source file (2021-01-28)
Supplement: Supplementary file 16 [file tennis_interpolation.tex]

\begin{figure*}
\centering
\resizebox{\linewidth}{!}{
\includegraphics[width=1\linewidth]{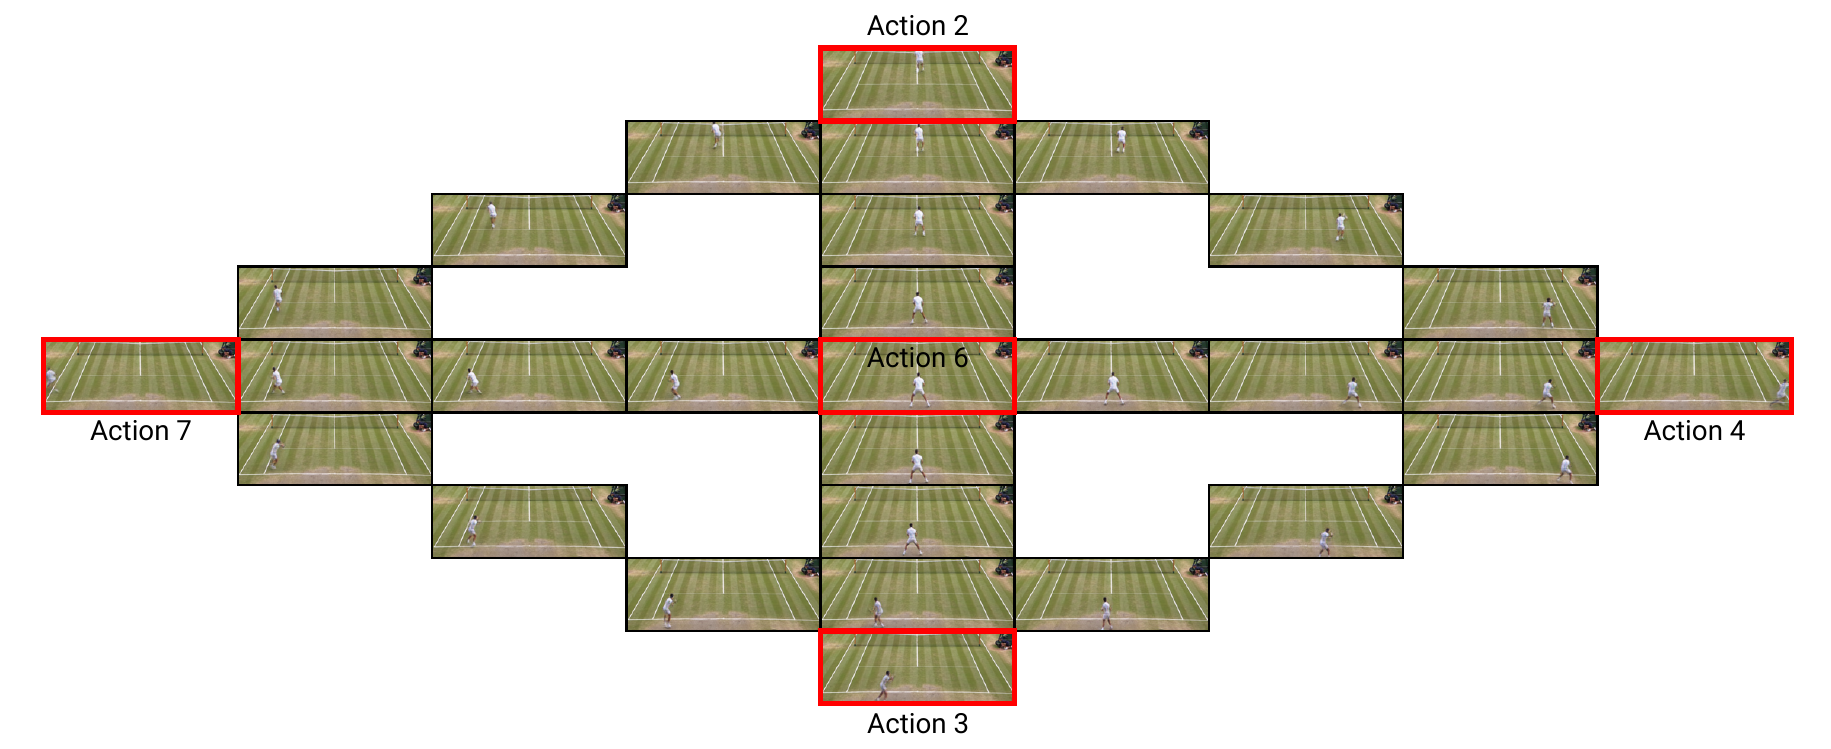}
}
\caption{Visualization of the last frame of sequences produced from the same initial frame with differing \emph{actions} and \emph{action variability embeddings}. The sequences in red represent pure discrete actions where, \emph{action variability embeddings} are posed to 0. For the sequences in black instead, \emph{actions} and \emph{action variability embeddings} are derived as described in Sec.~\ref{sec:action_variability_embeddings} to represent intermediate actions between the two closest discrete actions using values of the \emph{interpolation factor} of 0.3, 0.5 and 0.7. Note how the player positions depicted in the black sequences smoothly interpolate between the positions obtained with pure discrete actions, showing the capability of \emph{action variability embeddings} to capture variations on discrete actions.}
\label{fig:action_interpolation}
\end{figure*}
